# Supplementary material for: On the Use of Information Criteria for Subset Selection in Least Squares Regression
Source: arXiv:1911.10191 source file (2021-03-06)
Supplement: Supplementary file 1 [file Dense_n2000_rho_0.tex]

% latex table generated in R 3.6.2 by xtable 1.8-4 package
% Sat Dec 21 23:36:37 2019
\begin{table}[ht]
\centering
\caption{The performance of BOSS compared to other methods, Dense, $\rho$=0, n=2000} 
\scalebox{0.7}{
\begin{tabular}{|c|c|ccccccc|}
  \toprule 
 \multicolumn{1}{|c}{} &       & BOSS  & BS    & FS    & LASSO & Gamma LASSO & SparseNet & \multicolumn{1}{c|}{rLASSO} \\
 \multicolumn{1}{|c}{} &       & C$_p$-hdf/AICc-hdf/CV & CV    & CV    & AICc/CV & AICc/CV & CV    & \multicolumn{1}{c|}{CV}  \\
 \cmidrule{3-9}\multicolumn{1}{|c}{} &       & \multicolumn{7}{c|}{\% worse than the best possible BOSS}  \\
 \midrule\multirow{4}[2]{*}{hsnr} & p=14 & 0/0/0 & 0 & 0 & 2/2 & 1/4 & 0 & 0 \\ 
   & p=30 & 0/0/1 & 1 & 1 & 1/1 & 3/6 & 1 & 1 \\ 
   & p=60 & 5/5/7 & - & 7 & 1/0 & 0/0 & 3 & 4 \\ 
   & p=180 & 7/7/9 & - & 9 & 15/14 & 3/5 & 2 & 9 \\ 
  \midrule\multirow{4}[2]{*}{msnr} & p=14 & 0/0/0 & 0 & 0 & 0/0 & 0/2 & 0 & 0 \\ 
   & p=30 & 1/1/5 & 5 & 5 & 1/1 & 4/2 & 3 & 3 \\ 
   & p=60 & 8/8/9 & - & 9 & 1/0 & -1/0 & 3 & 4 \\ 
   & p=180 & 8/8/10 & - & 10 & 13/12 & 3/4 & 3 & 7 \\ 
  \midrule\multirow{4}[2]{*}{lsnr} & p=14 & 0/0/4 & 4 & 4 & 0/0 & 3/1 & 3 & 3 \\ 
   & p=30 & 3/3/10 & 10 & 9 & 1/0 & 7/2 & 5 & 5 \\ 
   & p=60 & 13/13/12 & - & 12 & 0/-1 & 0/1 & 3 & 3 \\ 
   & p=180 & 9/9/12 & - & 13 & 9/8 & 14/5 & 4 & 7 \\ 
   \midrule 
 \multicolumn{1}{|c}{} &       & \multicolumn{7}{c|}{Relative efficiency} \\
\midrule\multirow{4}[2]{*}{hsnr} & p=14 & 1/1/1 & 1 & 1 & 0.98/0.98 & 0.99/0.96 & 1 & 1 \\ 
   & p=30 & 1/1/0.99 & 0.99 & 0.99 & 0.99/0.99 & 0.97/0.94 & 0.99 & 0.99 \\ 
   & p=60 & 0.95/0.95/0.93 & - & 0.93 & 0.99/0.99 & 1/1 & 0.97 & 0.96 \\ 
   & p=180 & 0.95/0.96/0.94 & - & 0.94 & 0.89/0.9 & 0.99/0.98 & 1 & 0.94 \\ 
  \midrule\multirow{4}[2]{*}{msnr} & p=14 & 1/1/1 & 1 & 1 & 1/1 & 1/0.99 & 1 & 1 \\ 
   & p=30 & 1/1/0.96 & 0.96 & 0.96 & 1/1 & 0.97/0.99 & 0.97 & 0.97 \\ 
   & p=60 & 0.92/0.92/0.91 & - & 0.91 & 0.98/0.99 & 1/0.99 & 0.96 & 0.96 \\ 
   & p=180 & 0.95/0.95/0.93 & - & 0.93 & 0.91/0.92 & 1/0.99 & 1 & 0.96 \\ 
  \midrule\multirow{4}[2]{*}{lsnr} & p=14 & 1/1/0.96 & 0.96 & 0.96 & 1/1 & 0.98/0.99 & 0.98 & 0.97 \\ 
   & p=30 & 0.97/0.97/0.91 & 0.91 & 0.92 & 1/1 & 0.94/0.98 & 0.96 & 0.96 \\ 
   & p=60 & 0.88/0.88/0.88 & - & 0.88 & 0.99/1 & 0.99/0.99 & 0.96 & 0.96 \\ 
   & p=180 & 0.95/0.96/0.93 & - & 0.93 & 0.96/0.97 & 0.91/1 & 1 & 0.97 \\ 
   \midrule 
 \multicolumn{1}{|c}{} &       & \multicolumn{7}{c|}{Sparsistency (number of extra variables)} \\
\midrule\multirow{4}[2]{*}{hsnr} & p=14 & 14/14/14 & 14 & 14 & 14/14 & 14/14 & 14 & 14 \\ 
   & p=30 & 30/30/29.8 & 29.8 & 29.8 & 30/30 & 30/30 & 29.9 & 29.9 \\ 
   & p=60 & 50.1/49.6/39.8 & - & 39.7 & 53.1/54.3 & 46.4/50.2 & 44.8 & 42.6 \\ 
   & p=180 & 32.5/31.6/32.3 & - & 32.1 & 88.1/88.8 & 62.2/60.9 & 46.4 & 38.7 \\ 
  \midrule\multirow{4}[2]{*}{msnr} & p=14 & 14/14/14 & 14 & 14 & 14/14 & 14/14 & 14 & 14 \\ 
   & p=30 & 29.8/29.8/28.1 & 28.2 & 28.1 & 29.6/29.8 & 28.9/29.7 & 28.7 & 28.7 \\ 
   & p=60 & 42/41.1/31.3 & - & 31.1 & 48.1/49.1 & 37.1/43.5 & 37.5 & 34.2 \\ 
   & p=180 & 23.9/23.2/24.1 & - & 24.1 & 75.1/74.9 & 51.3/44.6 & 38.9 & 29.6 \\ 
  \midrule\multirow{4}[2]{*}{lsnr} & p=14 & 14/14/13.7 & 13.7 & 13.7 & 14/14 & 13.8/14 & 13.8 & 13.8 \\ 
   & p=30 & 27.8/27.8/22.1 & 21.9 & 22.1 & 26.8/27.5 & 21/26.2 & 24.6 & 23.4 \\ 
   & p=60 & 30/28.5/19.9 & - & 19.5 & 38.5/38.9 & 25.4/31.4 & 29.1 & 25.3 \\ 
   & p=180 & 14.1/13.5/14.1 & - & 14 & 55.3/53.9 & 42/31.8 & 29.7 & 23.4 \\ 
   \bottomrule 
\end{tabular}
}
\end{table}
