# Supplementary material for: On the Use of Information Criteria for Subset Selection in Least Squares Regression
Source: arXiv:1911.10191 source file (2021-03-06)
Supplement: Supplementary file 2 [file Dense_n2000_rho_05.tex]

% latex table generated in R 3.6.2 by xtable 1.8-4 package
% Sat Dec 21 23:36:43 2019
\begin{table}[ht]
\centering
\caption{The performance of BOSS compared to other methods, Dense, $\rho$=0.5, n=2000} 
\scalebox{0.7}{
\begin{tabular}{|c|c|ccccccc|}
  \toprule 
 \multicolumn{1}{|c}{} &       & BOSS  & BS    & FS    & LASSO & Gamma LASSO & SparseNet & \multicolumn{1}{c|}{rLASSO} \\
 \multicolumn{1}{|c}{} &       & C$_p$-hdf/AICc-hdf/CV & CV    & CV    & AICc/CV & AICc/CV & CV    & \multicolumn{1}{c|}{CV}  \\
 \cmidrule{3-9}\multicolumn{1}{|c}{} &       & \multicolumn{7}{c|}{\% worse than the best possible BOSS}  \\
 \midrule\multirow{4}[2]{*}{hsnr} & p=14 & 0/0/0 & 0 & 0 & 2/2 & 2/5 & 0 & 0 \\ 
   & p=30 & 0/0/3 & 0 & 0 & 1/1 & 9/10 & 0 & -1 \\ 
   & p=60 & 6/6/7 & - & 7 & 4/3 & 4/5 & 5 & 6 \\ 
   & p=180 & 8/8/9 & - & 12 & 37/36 & 20/20 & 8 & 34 \\ 
  \midrule\multirow{4}[2]{*}{msnr} & p=14 & 0/0/2 & 0 & 0 & 0/0 & 1/4 & 0 & 0 \\ 
   & p=30 & 0/0/5 & 6 & 5 & 1/0 & 3/5 & 3 & 1 \\ 
   & p=60 & 10/10/10 & - & 10 & 7/6 & 4/5 & 7 & 9 \\ 
   & p=180 & 9/9/11 & - & 14 & 36/34 & 16/18 & 9 & 33 \\ 
  \midrule\multirow{4}[2]{*}{lsnr} & p=14 & 0/0/5 & 2 & 2 & 0/0 & 1/1 & 1 & 1 \\ 
   & p=30 & 2/2/9 & 10 & 10 & 2/1 & 7/2 & 7 & 3 \\ 
   & p=60 & 17/16/13 & - & 14 & 11/10 & 6/8 & 8 & 13 \\ 
   & p=180 & 11/11/13 & - & 16 & 32/30 & 19/18 & 10 & 30 \\ 
   \midrule 
 \multicolumn{1}{|c}{} &       & \multicolumn{7}{c|}{Relative efficiency} \\
\midrule\multirow{4}[2]{*}{hsnr} & p=14 & 1/1/1 & 1 & 1 & 0.98/0.98 & 0.98/0.95 & 1 & 1 \\ 
   & p=30 & 0.98/0.98/0.96 & 0.98 & 0.98 & 0.97/0.97 & 0.9/0.89 & 0.98 & 0.99 \\ 
   & p=60 & 0.98/0.98/0.96 & - & 0.96 & 1/1 & 0.99/0.98 & 0.98 & 0.98 \\ 
   & p=180 & 1/1/0.99 & - & 0.96 & 0.79/0.79 & 0.9/0.89 & 1 & 0.81 \\ 
  \midrule\multirow{4}[2]{*}{msnr} & p=14 & 1/1/0.98 & 1 & 1 & 1/1 & 0.99/0.96 & 1 & 1 \\ 
   & p=30 & 0.98/0.98/0.94 & 0.93 & 0.94 & 0.98/0.98 & 0.95/0.94 & 0.96 & 0.97 \\ 
   & p=60 & 0.95/0.95/0.95 & - & 0.95 & 0.98/0.98 & 1/1 & 0.98 & 0.96 \\ 
   & p=180 & 0.99/1/0.98 & - & 0.95 & 0.8/0.81 & 0.93/0.92 & 1 & 0.81 \\ 
  \midrule\multirow{4}[2]{*}{lsnr} & p=14 & 1/1/0.95 & 0.98 & 0.98 & 1/1 & 0.99/0.99 & 0.99 & 0.99 \\ 
   & p=30 & 0.98/0.98/0.91 & 0.9 & 0.91 & 0.98/0.98 & 0.93/0.97 & 0.93 & 0.96 \\ 
   & p=60 & 0.91/0.91/0.93 & - & 0.93 & 0.95/0.96 & 1/0.98 & 0.98 & 0.94 \\ 
   & p=180 & 0.99/1/0.97 & - & 0.95 & 0.83/0.85 & 0.93/0.93 & 1 & 0.85 \\ 
   \midrule 
 \multicolumn{1}{|c}{} &       & \multicolumn{7}{c|}{Sparsistency (number of extra variables)} \\
\midrule\multirow{4}[2]{*}{hsnr} & p=14 & 14/14/14 & 14 & 14 & 14/14 & 14/14 & 14 & 14 \\ 
   & p=30 & 30/30/30 & 30 & 30 & 30/30 & 30/30 & 30 & 30 \\ 
   & p=60 & 53.6/53.3/40.3 & - & 40 & 55.4/56.9 & 48.4/49.4 & 43.8 & 49 \\ 
   & p=180 & 36/34.5/35.1 & - & 32.6 & 106.5/113.5 & 76.5/77.1 & 43 & 66.3 \\ 
  \midrule\multirow{4}[2]{*}{msnr} & p=14 & 14/14/14 & 14 & 14 & 14/14 & 14/14 & 14 & 14 \\ 
   & p=30 & 30/30/28.6 & 28.3 & 28.5 & 29.8/29.9 & 29.4/29.7 & 29.1 & 29.2 \\ 
   & p=60 & 47.5/46.6/31.6 & - & 31.2 & 51.5/53.4 & 42.1/48.1 & 36.3 & 43.6 \\ 
   & p=180 & 27.3/26.2/27.1 & - & 24.1 & 90.5/98.9 & 60/54.4 & 35.2 & 54.9 \\ 
  \midrule\multirow{4}[2]{*}{lsnr} & p=14 & 14/14/13.9 & 13.9 & 13.9 & 14/14 & 14/14 & 13.9 & 13.9 \\ 
   & p=30 & 29.1/29/22.7 & 21.2 & 22.1 & 28/28.9 & 23/27.6 & 24.1 & 26.2 \\ 
   & p=60 & 36.1/34.7/21.1 & - & 19.8 & 42.2/45.5 & 28.3/34.9 & 26.5 & 35.2 \\ 
   & p=180 & 17/16/17 & - & 14.3 & 61.8/72 & 43.7/33.1 & 25.3 & 46.9 \\ 
   \bottomrule 
\end{tabular}
}
\end{table}
