# Supplementary material for: On the Use of Information Criteria for Subset Selection in Least Squares Regression
Source: arXiv:1911.10191 source file (2021-03-06)
Supplement: Supplementary file 3 [file Dense_n2000_rho_09.tex]

% latex table generated in R 3.6.2 by xtable 1.8-4 package
% Sat Dec 21 23:36:50 2019
\begin{table}[ht]
\centering
\caption{The performance of BOSS compared to other methods, Dense, $\rho$=0.9, n=2000} 
\scalebox{0.7}{
\begin{tabular}{|c|c|ccccccc|}
  \toprule 
 \multicolumn{1}{|c}{} &       & BOSS  & BS    & FS    & LASSO & Gamma LASSO & SparseNet & \multicolumn{1}{c|}{rLASSO} \\
 \multicolumn{1}{|c}{} &       & C$_p$-hdf/AICc-hdf/CV & CV    & CV    & AICc/CV & AICc/CV & CV    & \multicolumn{1}{c|}{CV}  \\
 \cmidrule{3-9}\multicolumn{1}{|c}{} &       & \multicolumn{7}{c|}{\% worse than the best possible BOSS}  \\
 \midrule\multirow{4}[2]{*}{hsnr} & p=14 & 0/0/0 & 0 & 0 & 3/4 & 27/27 & 2 & 0 \\ 
   & p=30 & 0/0/3 & 1 & 1 & 2/2 & 106/106 & 1 & 3 \\ 
   & p=60 & 7/8/9 & - & 6 & 6/6 & 74/74 & 8 & 7 \\ 
   & p=180 & 10/10/10 & - & 9 & 39/38 & 56/56 & 17 & 35 \\ 
  \midrule\multirow{4}[2]{*}{msnr} & p=14 & 0/0/3 & 0 & 0 & 1/1 & 8/8 & 1 & 0 \\ 
   & p=30 & 0/0/5 & 7 & 5 & 1/1 & 25/25 & 3 & 6 \\ 
   & p=60 & 12/12/10 & - & 8 & 9/8 & 11/11 & 9 & 10 \\ 
   & p=180 & 10/11/12 & - & 9 & 41/39 & 22/23 & 16 & 38 \\ 
  \midrule\multirow{4}[2]{*}{lsnr} & p=14 & 1/1/7 & 5 & 4 & 1/1 & 5/8 & 3 & 3 \\ 
   & p=30 & 3/3/11 & 11 & 9 & 3/2 & 7/6 & 8 & 8 \\ 
   & p=60 & 19/18/14 & - & 10 & 14/13 & 8/11 & 12 & 15 \\ 
   & p=180 & 12/12/13 & - & 11 & 40/38 & 27/26 & 18 & 37 \\ 
   \midrule 
 \multicolumn{1}{|c}{} &       & \multicolumn{7}{c|}{Relative efficiency} \\
\midrule\multirow{4}[2]{*}{hsnr} & p=14 & 1/1/1 & 1 & 1 & 0.97/0.97 & 0.79/0.79 & 0.98 & 1 \\ 
   & p=30 & 1/1/0.97 & 0.99 & 0.99 & 0.98/0.98 & 0.49/0.49 & 0.99 & 0.98 \\ 
   & p=60 & 0.98/0.98/0.97 & - & 1 & 1/1 & 0.61/0.61 & 0.97 & 0.99 \\ 
   & p=180 & 0.99/0.99/0.99 & - & 1 & 0.78/0.79 & 0.7/0.7 & 0.93 & 0.8 \\ 
  \midrule\multirow{4}[2]{*}{msnr} & p=14 & 1/1/0.97 & 1 & 1 & 0.99/0.99 & 0.92/0.92 & 0.99 & 1 \\ 
   & p=30 & 1/1/0.96 & 0.94 & 0.95 & 1/1 & 0.8/0.8 & 0.97 & 0.95 \\ 
   & p=60 & 0.96/0.96/0.98 & - & 1 & 0.99/0.99 & 0.97/0.97 & 0.99 & 0.98 \\ 
   & p=180 & 0.98/0.98/0.98 & - & 1 & 0.77/0.78 & 0.89/0.88 & 0.94 & 0.79 \\ 
  \midrule\multirow{4}[2]{*}{lsnr} & p=14 & 1/1/0.94 & 0.95 & 0.97 & 1/1 & 0.96/0.93 & 0.98 & 0.98 \\ 
   & p=30 & 0.99/0.99/0.92 & 0.92 & 0.94 & 1/1 & 0.96/0.96 & 0.94 & 0.95 \\ 
   & p=60 & 0.91/0.92/0.95 & - & 0.99 & 0.95/0.96 & 1/0.98 & 0.97 & 0.95 \\ 
   & p=180 & 1/0.99/0.99 & - & 1 & 0.8/0.81 & 0.88/0.88 & 0.94 & 0.81 \\ 
   \midrule 
 \multicolumn{1}{|c}{} &       & \multicolumn{7}{c|}{Sparsistency (number of extra variables)} \\
\midrule\multirow{4}[2]{*}{hsnr} & p=14 & 14/14/14 & 14 & 14 & 14/14 & 14/14 & 14 & 14 \\ 
   & p=30 & 30/30/29.9 & 29.9 & 29.9 & 30/30 & 26.1/26.1 & 30 & 29.9 \\ 
   & p=60 & 53.2/52.7/39.2 & - & 36.3 & 55.5/57.2 & 29.4/29.4 & 46 & 49.5 \\ 
   & p=180 & 37/35/38.6 & - & 30.2 & 109.6/118.6 & 43.1/43.1 & 52.4 & 74.3 \\ 
  \midrule\multirow{4}[2]{*}{msnr} & p=14 & 14/14/14 & 14 & 14 & 14/14 & 14/14 & 14 & 14 \\ 
   & p=30 & 29.9/29.9/28.2 & 27.3 & 27.9 & 29.7/29.9 & 26.3/26.3 & 28.8 & 28.7 \\ 
   & p=60 & 47.5/46.6/31.3 & - & 27.4 & 51.1/53.4 & 35.5/35.6 & 37.2 & 44 \\ 
   & p=180 & 30.8/28.4/32 & - & 23 & 95.1/104.1 & 62.7/59 & 44.6 & 71.3 \\ 
  \midrule\multirow{4}[2]{*}{lsnr} & p=14 & 14/14/13.8 & 13.6 & 13.7 & 14/14 & 13.8/13.9 & 13.8 & 13.8 \\ 
   & p=30 & 28.8/28.8/21.2 & 18.5 & 20.2 & 27.6/28.4 & 21.7/24.8 & 23.5 & 24.8 \\ 
   & p=60 & 35.3/33.6/20.6 & - & 16.3 & 41/43.9 & 28.5/33.1 & 26.4 & 35.4 \\ 
   & p=180 & 18.5/16.6/21.4 & - & 11.8 & 65.3/76.1 & 49.6/41.2 & 32.3 & 60.8 \\ 
   \bottomrule 
\end{tabular}
}
\end{table}
