# Supplementary material for: On the Use of Information Criteria for Subset Selection in Least Squares Regression
Source: arXiv:1911.10191 source file (2021-03-06)
Supplement: Supplementary file 4 [file Dense_n200_rho_0.tex]

% latex table generated in R 3.6.2 by xtable 1.8-4 package
% Sat Dec 21 23:36:31 2019
\begin{table}[ht]
\centering
\caption{The performance of BOSS compared to other methods, Dense, $\rho$=0, n=200} 
\scalebox{0.7}{
\begin{tabular}{|c|c|ccccccc|}
  \toprule 
 \multicolumn{1}{|c}{} &       & BOSS  & BS    & FS    & LASSO & Gamma LASSO & SparseNet & \multicolumn{1}{c|}{rLASSO} \\
 \multicolumn{1}{|c}{} &       & C$_p$-hdf/AICc-hdf/CV & CV    & CV    & AICc/CV & AICc/CV & CV    & \multicolumn{1}{c|}{CV}  \\
 \cmidrule{3-9}\multicolumn{1}{|c}{} &       & \multicolumn{7}{c|}{\% worse than the best possible BOSS}  \\
 \midrule\multirow{4}[2]{*}{hsnr} & p=14 & 0/0/0 & 0 & 0 & 0/0 & 0/1 & 0 & 0 \\ 
   & p=30 & 2/2/7 & 8 & 7 & 1/1 & 8/2 & 4 & 4 \\ 
   & p=60 & 9/11/11 & - & 11 & 0/-2 & -1/-1 & 1 & 2 \\ 
   & p=180 & 18/13/11 & - & 12 & 18/12 & 5/5 & 3 & 13 \\ 
  \midrule\multirow{4}[2]{*}{msnr} & p=14 & 0/0/6 & 6 & 6 & 1/1 & 7/1 & 3 & 3 \\ 
   & p=30 & 4/5/10 & 10 & 10 & 0/-1 & 8/2 & 4 & 3 \\ 
   & p=60 & 11/12/12 & - & 12 & -3/-5 & -1/-2 & -1 & -1 \\ 
   & p=180 & 19/14/13 & - & 12 & 3/0 & 13/1 & 2 & 5 \\ 
  \midrule\multirow{4}[2]{*}{lsnr} & p=14 & 7/9/20 & 19 & 20 & 3/3 & 17/8 & 10 & 10 \\ 
   & p=30 & 15/19/16 & 16 & 16 & -8/-8 & 5/-1 & -3 & -3 \\ 
   & p=60 & 16/14/14 & - & 14 & -9/-8 & 11/-4 & -4 & -4 \\ 
   & p=180 & 22/7/8 & - & 9 & -5/-3 & 65/0 & -1 & 0 \\ 
   \midrule 
 \multicolumn{1}{|c}{} &       & \multicolumn{7}{c|}{Relative efficiency} \\
\midrule\multirow{4}[2]{*}{hsnr} & p=14 & 1/1/1 & 1 & 1 & 1/1 & 1/0.99 & 1 & 1 \\ 
   & p=30 & 0.99/0.99/0.95 & 0.94 & 0.94 & 1/1 & 0.93/0.99 & 0.97 & 0.98 \\ 
   & p=60 & 0.9/0.88/0.89 & - & 0.89 & 0.98/1 & 1/0.99 & 0.98 & 0.96 \\ 
   & p=180 & 0.88/0.91/0.93 & - & 0.93 & 0.88/0.93 & 0.99/0.99 & 1 & 0.92 \\ 
  \midrule\multirow{4}[2]{*}{msnr} & p=14 & 1/1/0.95 & 0.95 & 0.95 & 1/1 & 0.94/0.99 & 0.97 & 0.98 \\ 
   & p=30 & 0.96/0.95/0.91 & 0.9 & 0.91 & 0.99/1 & 0.92/0.98 & 0.96 & 0.96 \\ 
   & p=60 & 0.86/0.85/0.85 & - & 0.85 & 0.98/1 & 0.96/0.97 & 0.96 & 0.96 \\ 
   & p=180 & 0.84/0.88/0.89 & - & 0.89 & 0.97/1 & 0.88/0.98 & 0.98 & 0.95 \\ 
  \midrule\multirow{4}[2]{*}{lsnr} & p=14 & 0.96/0.94/0.86 & 0.86 & 0.85 & 0.99/1 & 0.88/0.95 & 0.93 & 0.93 \\ 
   & p=30 & 0.8/0.77/0.79 & 0.79 & 0.79 & 1/1 & 0.88/0.93 & 0.94 & 0.94 \\ 
   & p=60 & 0.79/0.8/0.8 & - & 0.8 & 1/1 & 0.83/0.95 & 0.96 & 0.96 \\ 
   & p=180 & 0.78/0.89/0.88 & - & 0.88 & 1/0.98 & 0.58/0.95 & 0.96 & 0.95 \\ 
   \midrule 
 \multicolumn{1}{|c}{} &       & \multicolumn{7}{c|}{Sparsistency (number of extra variables)} \\
\midrule\multirow{4}[2]{*}{hsnr} & p=14 & 14/14/14 & 14 & 14 & 14/14 & 14/14 & 14 & 14 \\ 
   & p=30 & 29.2/29/26 & 25.7 & 25.9 & 28.6/29.2 & 25.3/28.6 & 27.2 & 26.8 \\ 
   & p=60 & 35.8/24.3/28 & - & 27.6 & 40.5/44.9 & 29.8/38.4 & 36.8 & 32.8 \\ 
   & p=180 & 36.9/17/19.3 & - & 19.2 & 47.5/67.6 & 38.7/36.4 & 32.4 & 36.5 \\ 
  \midrule\multirow{4}[2]{*}{msnr} & p=14 & 14/14/13.4 & 13.4 & 13.4 & 13.9/13.9 & 13.4/13.9 & 13.6 & 13.7 \\ 
   & p=30 & 26.9/26/21.1 & 20.7 & 20.9 & 25.1/26.3 & 18.8/24.9 & 23.7 & 22.6 \\ 
   & p=60 & 26/14.9/18.4 & - & 18.3 & 32.2/36.4 & 22.7/29.2 & 29.6 & 25 \\ 
   & p=180 & 30.7/7.9/9.9 & - & 9.9 & 33.8/49.1 & 40.6/30.1 & 27.9 & 25.8 \\ 
  \midrule\multirow{4}[2]{*}{lsnr} & p=14 & 12.2/11.8/8.3 & 8.4 & 8.2 & 10.6/11.2 & 7.6/10.4 & 10 & 9.1 \\ 
   & p=30 & 13/7.8/8 & 7.5 & 7.8 & 14/15.1 & 10.3/12.3 & 12.7 & 10.6 \\ 
   & p=60 & 5.4/1/4.2 & - & 4.1 & 15.2/16.6 & 15.3/13.7 & 14.6 & 12.2 \\ 
   & p=180 & 16.6/0.3/1.4 & - & 1.5 & 12.4/15.8 & 41.6/12.2 & 13.5 & 11.3 \\ 
   \bottomrule 
\end{tabular}
}
\end{table}
