# Supplementary material for: On the Use of Information Criteria for Subset Selection in Least Squares Regression
Source: arXiv:1911.10191 source file (2021-03-06)
Supplement: Supplementary file 5 [file Dense_n200_rho_05.tex]

% latex table generated in R 3.6.2 by xtable 1.8-4 package
% Sat Dec 21 23:36:38 2019
\begin{table}[ht]
\centering
\caption{The performance of BOSS compared to other methods, Dense, $\rho$=0.5, n=200} 
\scalebox{0.7}{
\begin{tabular}{|c|c|ccccccc|}
  \toprule 
 \multicolumn{1}{|c}{} &       & BOSS  & BS    & FS    & LASSO & Gamma LASSO & SparseNet & \multicolumn{1}{c|}{rLASSO} \\
 \multicolumn{1}{|c}{} &       & C$_p$-hdf/AICc-hdf/CV & CV    & CV    & AICc/CV & AICc/CV & CV    & \multicolumn{1}{c|}{CV}  \\
 \cmidrule{3-9}\multicolumn{1}{|c}{} &       & \multicolumn{7}{c|}{\% worse than the best possible BOSS}  \\
 \midrule\multirow{4}[2]{*}{hsnr} & p=14 & 0/0/4 & 0 & 0 & 0/0 & 1/2 & 0 & -1 \\ 
   & p=30 & 1/1/8 & 9 & 8 & 2/1 & 6/2 & 5 & 1 \\ 
   & p=60 & 13/13/12 & - & 12 & 10/7 & 5/5 & 7 & 4 \\ 
   & p=180 & 37/14/13 & - & 16 & 47/27 & 10/13 & 8 & 7 \\ 
  \midrule\multirow{4}[2]{*}{msnr} & p=14 & 0/0/5 & 5 & 4 & 0/0 & 2/1 & 2 & 1 \\ 
   & p=30 & 4/5/10 & 11 & 10 & 4/3 & 8/4 & 8 & 3 \\ 
   & p=60 & 16/15/14 & - & 14 & 11/6 & 4/6 & 7 & 4 \\ 
   & p=180 & 43/14/14 & - & 17 & 37/21 & 18/18 & 11 & 14 \\ 
  \midrule\multirow{4}[2]{*}{lsnr} & p=14 & 5/7/17 & 19 & 17 & 9/7 & 16/8 & 14 & 12 \\ 
   & p=30 & 18/18/17 & 16 & 18 & 10/7 & 10/10 & 11 & 7 \\ 
   & p=60 & 17/13/13 & - & 14 & 6/5 & 19/8 & 8 & 5 \\ 
   & p=180 & 47/4/8 & - & 9 & 2/4 & 79/6 & 6 & 4 \\ 
   \midrule 
 \multicolumn{1}{|c}{} &       & \multicolumn{7}{c|}{Relative efficiency} \\
\midrule\multirow{4}[2]{*}{hsnr} & p=14 & 0.99/0.99/0.95 & 0.99 & 0.99 & 0.99/0.99 & 0.99/0.97 & 0.99 & 1 \\ 
   & p=30 & 0.98/0.98/0.93 & 0.91 & 0.93 & 0.98/0.98 & 0.94/0.98 & 0.94 & 0.98 \\ 
   & p=60 & 0.92/0.92/0.93 & - & 0.93 & 0.95/0.98 & 0.99/0.99 & 0.97 & 1 \\ 
   & p=180 & 0.78/0.94/0.95 & - & 0.92 & 0.73/0.84 & 0.97/0.95 & 0.99 & 1 \\ 
  \midrule\multirow{4}[2]{*}{msnr} & p=14 & 1/1/0.95 & 0.95 & 0.96 & 1/1 & 0.98/0.99 & 0.98 & 0.99 \\ 
   & p=30 & 0.98/0.98/0.93 & 0.92 & 0.93 & 0.99/1 & 0.95/0.98 & 0.95 & 0.99 \\ 
   & p=60 & 0.89/0.9/0.91 & - & 0.91 & 0.93/0.98 & 1/0.98 & 0.97 & 1 \\ 
   & p=180 & 0.77/0.97/0.97 & - & 0.95 & 0.81/0.91 & 0.94/0.94 & 1 & 0.97 \\ 
  \midrule\multirow{4}[2]{*}{lsnr} & p=14 & 0.97/0.96/0.87 & 0.86 & 0.87 & 0.93/0.96 & 0.88/0.94 & 0.9 & 0.91 \\ 
   & p=30 & 0.9/0.9/0.92 & 0.92 & 0.91 & 0.97/1 & 0.98/0.97 & 0.96 & 1 \\ 
   & p=60 & 0.9/0.93/0.93 & - & 0.93 & 0.99/1 & 0.88/0.98 & 0.97 & 1 \\ 
   & p=180 & 0.69/0.97/0.94 & - & 0.94 & 1/0.98 & 0.57/0.96 & 0.96 & 0.98 \\ 
   \midrule 
 \multicolumn{1}{|c}{} &       & \multicolumn{7}{c|}{Sparsistency (number of extra variables)} \\
\midrule\multirow{4}[2]{*}{hsnr} & p=14 & 14/14/14 & 14 & 14 & 14/14 & 14/14 & 14 & 14 \\ 
   & p=30 & 29.7/29.6/26.1 & 25.1 & 26 & 29.1/29.7 & 27/29.2 & 27 & 28 \\ 
   & p=60 & 42/29.1/29.4 & - & 28.6 & 44.7/50.7 & 33.7/43.1 & 35 & 42 \\ 
   & p=180 & 43.6/17/20.2 & - & 19.6 & 52.2/87.1 & 40.3/42.5 & 32.4 & 63.5 \\ 
  \midrule\multirow{4}[2]{*}{msnr} & p=14 & 14/14/13.7 & 13.6 & 13.7 & 14/14 & 13.8/14 & 13.8 & 13.9 \\ 
   & p=30 & 28.3/27.8/21.1 & 18.8 & 20.9 & 26.7/28.2 & 20.3/26.2 & 22.6 & 25.1 \\ 
   & p=60 & 34.4/17.9/19.9 & - & 19.6 & 34.7/43.5 & 24.7/33.7 & 27.1 & 35.8 \\ 
   & p=180 & 36.7/8.3/11 & - & 9.7 & 24.5/61.4 & 39.6/28.9 & 22.1 & 47.6 \\ 
  \midrule\multirow{4}[2]{*}{lsnr} & p=14 & 13.1/12.7/9.4 & 8.7 & 9.3 & 10.8/12 & 8.7/11.4 & 10.3 & 10.6 \\ 
   & p=30 & 13.4/5.7/7.5 & 6.6 & 7.1 & 5.3/12.9 & 11.8/11.8 & 10.3 & 11.4 \\ 
   & p=60 & 4.8/0.6/3.5 & - & 3 & 3.7/11.2 & 15.7/9.4 & 8.9 & 8.7 \\ 
   & p=180 & 19/0.2/1.1 & - & 0.9 & 2.7/8.6 & 38.9/7.2 & 6.9 & 5.9 \\ 
   \bottomrule 
\end{tabular}
}
\end{table}
