# Supplementary material for: On the Use of Information Criteria for Subset Selection in Least Squares Regression
Source: arXiv:1911.10191 source file (2021-03-06)
Supplement: Supplementary file 6 [file Dense_n200_rho_09.tex]

% latex table generated in R 3.6.2 by xtable 1.8-4 package
% Sat Dec 21 23:36:44 2019
\begin{table}[ht]
\centering
\caption{The performance of BOSS compared to other methods, Dense, $\rho$=0.9, n=200} 
\scalebox{0.7}{
\begin{tabular}{|c|c|ccccccc|}
  \toprule 
 \multicolumn{1}{|c}{} &       & BOSS  & BS    & FS    & LASSO & Gamma LASSO & SparseNet & \multicolumn{1}{c|}{rLASSO} \\
 \multicolumn{1}{|c}{} &       & C$_p$-hdf/AICc-hdf/CV & CV    & CV    & AICc/CV & AICc/CV & CV    & \multicolumn{1}{c|}{CV}  \\
 \cmidrule{3-9}\multicolumn{1}{|c}{} &       & \multicolumn{7}{c|}{\% worse than the best possible BOSS}  \\
 \midrule\multirow{4}[2]{*}{hsnr} & p=14 & 0/0/5 & 0 & 0 & 0/0 & 6/7 & 1 & 1 \\ 
   & p=30 & 2/2/9 & 10 & 8 & 2/2 & 14/15 & 8 & 3 \\ 
   & p=60 & 15/19/14 & - & 12 & 12/11 & 12/13 & 14 & 6 \\ 
   & p=180 & 46/15/12 & - & 12 & 71/43 & 23/24 & 20 & 23 \\ 
  \midrule\multirow{4}[2]{*}{msnr} & p=14 & 1/1/7 & 8 & 6 & 2/1 & 8/8 & 5 & 5 \\ 
   & p=30 & 4/5/12 & 12 & 10 & 4/3 & 8/5 & 9 & 7 \\ 
   & p=60 & 20/23/16 & - & 13 & 30/17 & 12/15 & 15 & 18 \\ 
   & p=180 & 58/26/15 & - & 17 & 61/46 & 31/37 & 26 & 44 \\ 
  \midrule\multirow{4}[2]{*}{lsnr} & p=14 & 11/13/18 & 19 & 18 & 11/10 & 13/12 & 18 & 16 \\ 
   & p=30 & 19/15/14 & 15 & 13 & 10/11 & 19/12 & 12 & 15 \\ 
   & p=60 & 14/11/12 & - & 12 & 9/12 & 34/13 & 12 & 4 \\ 
   & p=180 & 59/12/10 & - & 10 & 15/17 & 106/12 & 9 & 10 \\ 
   \midrule 
 \multicolumn{1}{|c}{} &       & \multicolumn{7}{c|}{Relative efficiency} \\
\midrule\multirow{4}[2]{*}{hsnr} & p=14 & 0.99/0.99/0.95 & 0.99 & 0.99 & 0.99/0.99 & 0.94/0.93 & 0.99 & 0.99 \\ 
   & p=30 & 0.98/0.98/0.91 & 0.9 & 0.92 & 0.98/0.98 & 0.87/0.87 & 0.93 & 0.97 \\ 
   & p=60 & 0.87/0.84/0.87 & - & 0.89 & 0.89/0.9 & 0.89/0.88 & 0.88 & 0.94 \\ 
   & p=180 & 0.77/0.97/1 & - & 1 & 0.65/0.78 & 0.91/0.9 & 0.93 & 0.91 \\ 
  \midrule\multirow{4}[2]{*}{msnr} & p=14 & 0.99/0.99/0.94 & 0.93 & 0.94 & 0.98/0.99 & 0.93/0.93 & 0.95 & 0.96 \\ 
   & p=30 & 0.99/0.98/0.92 & 0.92 & 0.93 & 0.99/1 & 0.95/0.98 & 0.95 & 0.96 \\ 
   & p=60 & 0.93/0.92/0.97 & - & 0.99 & 0.86/0.96 & 1/0.97 & 0.98 & 0.95 \\ 
   & p=180 & 0.73/0.91/1 & - & 0.98 & 0.71/0.79 & 0.88/0.84 & 0.91 & 0.8 \\ 
  \midrule\multirow{4}[2]{*}{lsnr} & p=14 & 0.93/0.91/0.87 & 0.87 & 0.88 & 0.94/0.94 & 0.91/0.93 & 0.88 & 0.89 \\ 
   & p=30 & 0.92/0.96/0.97 & 0.96 & 0.97 & 1/1 & 0.92/0.98 & 0.98 & 0.96 \\ 
   & p=60 & 0.91/0.94/0.93 & - & 0.93 & 0.96/0.93 & 0.78/0.93 & 0.93 & 1 \\ 
   & p=180 & 0.69/0.97/0.99 & - & 1 & 0.95/0.93 & 0.53/0.98 & 1 & 1 \\ 
   \midrule 
 \multicolumn{1}{|c}{} &       & \multicolumn{7}{c|}{Sparsistency (number of extra variables)} \\
\midrule\multirow{4}[2]{*}{hsnr} & p=14 & 14/14/14 & 14 & 14 & 14/14 & 14/14 & 14 & 14 \\ 
   & p=30 & 29.5/29.3/25.2 & 23 & 24.6 & 28.9/29.5 & 24.4/24.8 & 26.2 & 27.6 \\ 
   & p=60 & 44.3/26.1/27.4 & - & 23.6 & 46.5/49.8 & 31.6/34.4 & 32.9 & 41.2 \\ 
   & p=180 & 46.7/15.6/21.3 & - & 17.2 & 54.4/93.4 & 44.8/46.9 & 37.7 & 67.6 \\ 
  \midrule\multirow{4}[2]{*}{msnr} & p=14 & 14/14/13.5 & 13.2 & 13.4 & 13.9/14 & 13.4/13.7 & 13.5 & 13.6 \\ 
   & p=30 & 28.6/28/20.2 & 16.6 & 19 & 26.4/27.9 & 19.3/24.4 & 22.3 & 24.5 \\ 
   & p=60 & 33/13/18.4 & - & 14.9 & 30.3/42.2 & 24.7/32.3 & 25.8 & 34.3 \\ 
   & p=180 & 41.6/5.8/14.1 & - & 9.3 & 4.8/42.5 & 46.7/30.9 & 26 & 29.2 \\ 
  \midrule\multirow{4}[2]{*}{lsnr} & p=14 & 10.6/9.8/7.1 & 6.4 & 6.6 & 8.9/9.3 & 7.5/8.6 & 7 & 7.6 \\ 
   & p=30 & 8.6/4.1/5.2 & 4.3 & 4.5 & 8.4/9.2 & 10.3/7.6 & 5.9 & 6.8 \\ 
   & p=60 & 3.7/1.4/4 & - & 2.7 & 2.7/8.1 & 14.5/6.2 & 5 & 4.2 \\ 
   & p=180 & 18/1/2.1 & - & 1.6 & 3.9/6.8 & 37.7/4 & 3.3 & 2.7 \\ 
   \bottomrule 
\end{tabular}
}
\end{table}
