# Supplementary material for: On the Use of Information Criteria for Subset Selection in Least Squares Regression
Source: arXiv:1911.10191 source file (2021-03-06)
Supplement: Supplementary file 7 [file Sparse-Ex1_n2000_rho_0.tex]

% latex table generated in R 3.6.2 by xtable 1.8-4 package
% Sat Dec 21 23:35:16 2019
\begin{table}[ht]
\centering
\caption{The performance of BOSS compared to other methods, Sparse-Ex1, $\rho$=0, n=2000} 
\scalebox{0.7}{
\begin{tabular}{|c|c|ccccccc|}
  \toprule 
 \multicolumn{1}{|c}{} &       & BOSS  & BS    & FS    & LASSO & Gamma LASSO & SparseNet & \multicolumn{1}{c|}{rLASSO} \\
 \multicolumn{1}{|c}{} &       & C$_p$-hdf/AICc-hdf/CV & CV    & CV    & AICc/CV & AICc/CV & CV    & \multicolumn{1}{c|}{CV}  \\
 \cmidrule{3-9}\multicolumn{1}{|c}{} &       & \multicolumn{7}{c|}{\% worse than the best possible BOSS}  \\
 \midrule\multirow{4}[2]{*}{hsnr} & p=14 & 6/6/17 & 18 & 17 & 40/40 & 12/14 & 11 & 13 \\ 
   & p=30 & 3/3/20 & 21 & 21 & 72/69 & 19/16 & 12 & 15 \\ 
   & p=60 & 2/2/23 & - & 22 & 100/96 & 30/19 & 15 & 17 \\ 
   & p=180 & 1/1/21 & - & 21 & 136/132 & 53/20 & 14 & 16 \\ 
  \midrule\multirow{4}[2]{*}{msnr} & p=14 & 6/6/17 & 18 & 17 & 41/40 & 14/17 & 12 & 13 \\ 
   & p=30 & 3/3/20 & 21 & 21 & 72/69 & 26/18 & 12 & 15 \\ 
   & p=60 & 2/2/23 & - & 22 & 100/96 & 46/22 & 15 & 18 \\ 
   & p=180 & 1/1/21 & - & 21 & 136/132 & 97/22 & 13 & 17 \\ 
  \midrule\multirow{4}[2]{*}{lsnr} & p=14 & 8/8/17 & 18 & 17 & 41/40 & 21/20 & 12 & 13 \\ 
   & p=30 & 5/4/20 & 21 & 21 & 72/69 & 44/23 & 12 & 15 \\ 
   & p=60 & 5/4/23 & - & 22 & 100/96 & 84/27 & 16 & 17 \\ 
   & p=180 & 5/5/21 & - & 21 & 136/132 & 192/27 & 13 & 17 \\ 
   \midrule 
 \multicolumn{1}{|c}{} &       & \multicolumn{7}{c|}{Relative efficiency} \\
\midrule\multirow{4}[2]{*}{hsnr} & p=14 & 1/1/0.9 & 0.9 & 0.91 & 0.76/0.76 & 0.95/0.92 & 0.95 & 0.94 \\ 
   & p=30 & 1/1/0.86 & 0.85 & 0.85 & 0.6/0.61 & 0.87/0.88 & 0.92 & 0.89 \\ 
   & p=60 & 1/1/0.83 & - & 0.83 & 0.51/0.52 & 0.78/0.85 & 0.89 & 0.87 \\ 
   & p=180 & 1/1/0.84 & - & 0.84 & 0.43/0.44 & 0.66/0.85 & 0.89 & 0.87 \\ 
  \midrule\multirow{4}[2]{*}{msnr} & p=14 & 1/1/0.9 & 0.9 & 0.91 & 0.75/0.76 & 0.93/0.91 & 0.95 & 0.94 \\ 
   & p=30 & 1/1/0.86 & 0.85 & 0.85 & 0.6/0.61 & 0.82/0.87 & 0.92 & 0.89 \\ 
   & p=60 & 1/1/0.83 & - & 0.83 & 0.51/0.52 & 0.7/0.84 & 0.89 & 0.86 \\ 
   & p=180 & 1/1/0.83 & - & 0.83 & 0.43/0.44 & 0.51/0.83 & 0.9 & 0.87 \\ 
  \midrule\multirow{4}[2]{*}{lsnr} & p=14 & 1/1/0.93 & 0.92 & 0.93 & 0.77/0.77 & 0.9/0.9 & 0.97 & 0.96 \\ 
   & p=30 & 1/1/0.87 & 0.86 & 0.87 & 0.61/0.62 & 0.73/0.85 & 0.93 & 0.91 \\ 
   & p=60 & 1/1/0.85 & - & 0.85 & 0.52/0.53 & 0.57/0.82 & 0.9 & 0.89 \\ 
   & p=180 & 1/1/0.86 & - & 0.86 & 0.44/0.45 & 0.36/0.83 & 0.93 & 0.9 \\ 
   \midrule 
 \multicolumn{1}{|c}{} &       & \multicolumn{7}{c|}{Sparsistency (number of extra variables)} \\
\midrule\multirow{4}[2]{*}{hsnr} & p=14 & 6(0.2)/6(0.2)/6(0.6) & 6(0.6) & 6(0.6) & 6(3.8)/6(4.4) & 6(0.9)/6(1.2) & 6(0.6) & 6(0.5) \\ 
   & p=30 & 6(0.1)/6(0.1)/6(0.5) & 6(0.6) & 6(0.6) & 6(8.5)/6(8.8) & 6(1.9)/6(1.7) & 6(1) & 6(0.5) \\ 
   & p=60 & 6(0)/6(0)/6(0.5) & - & 6(0.5) & 6(13.4)/6(12.6) & 6(4)/6(2.2) & 6(1.6) & 6(0.6) \\ 
   & p=180 & 6(0)/6(0)/6(0.4) & - & 6(0.3) & 6(23)/6(20.1) & 6(10.4)/6(2.5) & 6(2.1) & 6(0.4) \\ 
  \midrule\multirow{4}[2]{*}{msnr} & p=14 & 6(0.2)/6(0.2)/6(0.6) & 6(0.6) & 6(0.6) & 6(3.8)/6(4.4) & 6(1)/6(1.3) & 6(0.6) & 6(0.5) \\ 
   & p=30 & 6(0.1)/6(0.1)/6(0.5) & 6(0.6) & 6(0.6) & 6(8.5)/6(8.7) & 6(2.2)/6(1.6) & 6(0.9) & 6(0.5) \\ 
   & p=60 & 6(0)/6(0)/6(0.5) & - & 6(0.5) & 6(13.3)/6(12.6) & 6(5)/6(1.9) & 6(1.5) & 6(0.6) \\ 
   & p=180 & 6(0)/6(0)/6(0.4) & - & 6(0.3) & 6(22.8)/6(20) & 6(15.7)/6(1.9) & 6(1.8) & 6(0.4) \\ 
  \midrule\multirow{4}[2]{*}{lsnr} & p=14 & 6(0.4)/6(0.4)/6(0.6) & 6(0.6) & 6(0.6) & 6(3.8)/6(4.4) & 6(1.1)/6(1.3) & 6(0.5) & 6(0.5) \\ 
   & p=30 & 6(0.1)/6(0.1)/6(0.5) & 6(0.6) & 6(0.6) & 6(8.5)/6(8.7) & 6(2.9)/6(1.4) & 6(0.7) & 6(0.5) \\ 
   & p=60 & 6(0.1)/6(0.1)/6(0.5) & - & 6(0.5) & 6(13.4)/6(12.5) & 6(6.7)/6(1.6) & 6(1) & 6(0.6) \\ 
   & p=180 & 6(0.1)/6(0.1)/6(0.4) & - & 6(0.3) & 6(23)/6(20) & 6(23.6)/6(1.1) & 6(1) & 6(0.4) \\ 
   \bottomrule 
\end{tabular}
}
\end{table}
