# Supplementary material for: On the Use of Information Criteria for Subset Selection in Least Squares Regression
Source: arXiv:1911.10191 source file (2021-03-06)
Supplement: Supplementary file 8 [file Sparse-Ex1_n2000_rho_05.tex]

% latex table generated in R 3.6.2 by xtable 1.8-4 package
% Sat Dec 21 23:35:23 2019
\begin{table}[ht]
\centering
\caption{The performance of BOSS compared to other methods, Sparse-Ex1, $\rho$=0.5, n=2000} 
\scalebox{0.7}{
\begin{tabular}{|c|c|ccccccc|}
  \toprule 
 \multicolumn{1}{|c}{} &       & BOSS  & BS    & FS    & LASSO & Gamma LASSO & SparseNet & \multicolumn{1}{c|}{rLASSO} \\
 \multicolumn{1}{|c}{} &       & C$_p$-hdf/AICc-hdf/CV & CV    & CV    & AICc/CV & AICc/CV & CV    & \multicolumn{1}{c|}{CV}  \\
 \cmidrule{3-9}\multicolumn{1}{|c}{} &       & \multicolumn{7}{c|}{\% worse than the best possible BOSS}  \\
 \midrule\multirow{4}[2]{*}{hsnr} & p=14 & 7/6/17 & 19 & 17 & 38/39 & 12/14 & 12 & 14 \\ 
   & p=30 & 3/3/20 & 23 & 22 & 67/65 & 21/18 & 14 & 19 \\ 
   & p=60 & 2/2/21 & - & 21 & 91/89 & 29/19 & 15 & 20 \\ 
   & p=180 & 2/1/22 & - & 23 & 126/123 & 52/20 & 15 & 17 \\ 
  \midrule\multirow{4}[2]{*}{msnr} & p=14 & 7/6/17 & 19 & 17 & 39/39 & 16/17 & 12 & 14 \\ 
   & p=30 & 3/3/20 & 23 & 22 & 67/66 & 29/20 & 14 & 19 \\ 
   & p=60 & 2/2/21 & - & 21 & 91/89 & 45/21 & 14 & 20 \\ 
   & p=180 & 2/1/22 & - & 23 & 126/123 & 95/22 & 15 & 17 \\ 
  \midrule\multirow{4}[2]{*}{lsnr} & p=14 & 13/13/17 & 18 & 17 & 39/39 & 23/21 & 13 & 19 \\ 
   & p=30 & 6/6/20 & 23 & 22 & 67/65 & 49/25 & 15 & 21 \\ 
   & p=60 & 5/5/21 & - & 21 & 91/89 & 83/26 & 15 & 20 \\ 
   & p=180 & 4/4/22 & - & 23 & 126/123 & 192/28 & 15 & 17 \\ 
   \midrule 
 \multicolumn{1}{|c}{} &       & \multicolumn{7}{c|}{Relative efficiency} \\
\midrule\multirow{4}[2]{*}{hsnr} & p=14 & 1/1/0.91 & 0.9 & 0.91 & 0.77/0.77 & 0.95/0.93 & 0.95 & 0.93 \\ 
   & p=30 & 1/1/0.86 & 0.84 & 0.84 & 0.62/0.62 & 0.85/0.87 & 0.9 & 0.87 \\ 
   & p=60 & 1/1/0.84 & - & 0.84 & 0.54/0.54 & 0.79/0.86 & 0.89 & 0.85 \\ 
   & p=180 & 1/1/0.83 & - & 0.83 & 0.45/0.45 & 0.67/0.85 & 0.88 & 0.87 \\ 
  \midrule\multirow{4}[2]{*}{msnr} & p=14 & 1/1/0.91 & 0.9 & 0.91 & 0.77/0.76 & 0.92/0.91 & 0.95 & 0.93 \\ 
   & p=30 & 1/1/0.86 & 0.84 & 0.84 & 0.62/0.62 & 0.8/0.86 & 0.9 & 0.87 \\ 
   & p=60 & 1/1/0.84 & - & 0.84 & 0.54/0.54 & 0.71/0.84 & 0.89 & 0.85 \\ 
   & p=180 & 1/1/0.83 & - & 0.83 & 0.45/0.45 & 0.52/0.83 & 0.89 & 0.87 \\ 
  \midrule\multirow{4}[2]{*}{lsnr} & p=14 & 1/1/0.96 & 0.95 & 0.96 & 0.81/0.81 & 0.92/0.93 & 1 & 0.95 \\ 
   & p=30 & 1/1/0.88 & 0.86 & 0.87 & 0.63/0.64 & 0.71/0.85 & 0.92 & 0.88 \\ 
   & p=60 & 1/1/0.87 & - & 0.87 & 0.55/0.56 & 0.57/0.84 & 0.91 & 0.87 \\ 
   & p=180 & 1/1/0.85 & - & 0.85 & 0.46/0.47 & 0.36/0.82 & 0.9 & 0.89 \\ 
   \midrule 
 \multicolumn{1}{|c}{} &       & \multicolumn{7}{c|}{Sparsistency (number of extra variables)} \\
\midrule\multirow{4}[2]{*}{hsnr} & p=14 & 6(0.3)/6(0.3)/6(0.6) & 6(0.6) & 6(0.6) & 6(3.8)/6(4.2) & 6(0.9)/6(1) & 6(0.6) & 6(0.6) \\ 
   & p=30 & 6(0.1)/6(0.1)/6(0.6) & 6(0.7) & 6(0.6) & 6(6.6)/6(8.3) & 6(2.1)/6(1.7) & 6(1) & 6(0.8) \\ 
   & p=60 & 6(0)/6(0)/6(0.5) & - & 6(0.4) & 6(10.3)/6(12.1) & 6(3.7)/6(2) & 6(1.3) & 6(0.7) \\ 
   & p=180 & 6(0)/6(0)/6(0.5) & - & 6(0.4) & 6(13.8)/6(18.9) & 6(9.3)/6(2.5) & 6(2.3) & 6(0.4) \\ 
  \midrule\multirow{4}[2]{*}{msnr} & p=14 & 6(0.3)/6(0.3)/6(0.6) & 6(0.6) & 6(0.6) & 6(3.8)/6(4.2) & 6(1)/6(1.2) & 6(0.6) & 6(0.6) \\ 
   & p=30 & 6(0.1)/6(0.1)/6(0.6) & 6(0.7) & 6(0.6) & 6(6.6)/6(8.3) & 6(2.5)/6(1.6) & 6(0.9) & 6(0.8) \\ 
   & p=60 & 6(0)/6(0)/6(0.5) & - & 6(0.4) & 6(10.4)/6(12) & 6(4.6)/6(1.7) & 6(1.2) & 6(0.7) \\ 
   & p=180 & 6(0)/6(0)/6(0.5) & - & 6(0.4) & 6(14)/6(18.7) & 6(14.2)/6(2) & 6(2.1) & 6(0.5) \\ 
  \midrule\multirow{4}[2]{*}{lsnr} & p=14 & 6(0.6)/6(0.6)/6(0.6) & 6(0.6) & 6(0.6) & 6(3.8)/6(4.3) & 6(1.2)/6(1.3) & 6(0.5) & 6(1) \\ 
   & p=30 & 6(0.2)/6(0.1)/6(0.6) & 6(0.7) & 6(0.6) & 6(6.6)/6(8.4) & 6(3.1)/6(1.5) & 6(0.7) & 6(0.8) \\ 
   & p=60 & 6(0.1)/6(0.1)/6(0.5) & - & 6(0.4) & 6(10.3)/6(12) & 6(6.5)/6(1.4) & 6(0.8) & 6(0.8) \\ 
   & p=180 & 6(0.1)/6(0)/6(0.5) & - & 6(0.4) & 6(13.8)/6(18.8) & 6(23)/6(1.4) & 6(1.4) & 6(0.5) \\ 
   \bottomrule 
\end{tabular}
}
\end{table}
