# Supplementary material for: On the Use of Information Criteria for Subset Selection in Least Squares Regression
Source: arXiv:1911.10191 source file (2021-03-06)
Supplement: Supplementary file 9 [file Sparse-Ex1_n2000_rho_09.tex]

% latex table generated in R 3.6.2 by xtable 1.8-4 package
% Sat Dec 21 23:35:31 2019
\begin{table}[ht]
\centering
\caption{The performance of BOSS compared to other methods, Sparse-Ex1, $\rho$=0.9, n=2000} 
\scalebox{0.7}{
\begin{tabular}{|c|c|ccccccc|}
  \toprule 
 \multicolumn{1}{|c}{} &       & BOSS  & BS    & FS    & LASSO & Gamma LASSO & SparseNet & \multicolumn{1}{c|}{rLASSO} \\
 \multicolumn{1}{|c}{} &       & C$_p$-hdf/AICc-hdf/CV & CV    & CV    & AICc/CV & AICc/CV & CV    & \multicolumn{1}{c|}{CV}  \\
 \cmidrule{3-9}\multicolumn{1}{|c}{} &       & \multicolumn{7}{c|}{\% worse than the best possible BOSS}  \\
 \midrule\multirow{4}[2]{*}{hsnr} & p=14 & 7/7/21 & 18 & 22 & 30/30 & 6/8 & 17 & 23 \\ 
   & p=30 & 4/3/22 & 25 & 23 & 58/57 & 14/12 & 21 & 33 \\ 
   & p=60 & 2/2/21 & - & 22 & 81/82 & 34/19 & 18 & 18 \\ 
   & p=180 & 1/1/18 & - & 22 & 114/113 & 68/18 & 15 & 17 \\ 
  \midrule\multirow{4}[2]{*}{msnr} & p=14 & 15/15/21 & 14 & 21 & 22/20 & 14/12 & 14 & 23 \\ 
   & p=30 & 4/4/28 & 23 & 28 & 54/53 & 46/22 & 21 & 50 \\ 
   & p=60 & 2/2/22 & - & 24 & 81/82 & 76/24 & 20 & 24 \\ 
   & p=180 & 1/1/18 & - & 22 & 114/113 & 140/21 & 15 & 18 \\ 
  \midrule\multirow{4}[2]{*}{lsnr} & p=14 & 27/28/17 & 17 & 15 & -7/-9 & 10/2 & 4 & -2 \\ 
   & p=30 & 22/22/20 & 16 & 17 & -7/-7 & 10/-1 & 0 & -4 \\ 
   & p=60 & 9/9/17 & - & 16 & 15/15 & 42/13 & 16 & 12 \\ 
   & p=180 & 3/3/13 & - & 15 & 59/58 & 146/21 & 33 & 18 \\ 
   \midrule 
 \multicolumn{1}{|c}{} &       & \multicolumn{7}{c|}{Relative efficiency} \\
\midrule\multirow{4}[2]{*}{hsnr} & p=14 & 0.99/0.99/0.87 & 0.89 & 0.87 & 0.81/0.81 & 1/0.97 & 0.9 & 0.86 \\ 
   & p=30 & 1/1/0.85 & 0.83 & 0.84 & 0.65/0.66 & 0.9/0.92 & 0.86 & 0.77 \\ 
   & p=60 & 1/1/0.84 & - & 0.83 & 0.56/0.56 & 0.76/0.86 & 0.86 & 0.86 \\ 
   & p=180 & 1/1/0.85 & - & 0.83 & 0.47/0.47 & 0.6/0.85 & 0.88 & 0.86 \\ 
  \midrule\multirow{4}[2]{*}{msnr} & p=14 & 0.98/0.98/0.93 & 0.99 & 0.93 & 0.92/0.93 & 0.99/1 & 0.98 & 0.91 \\ 
   & p=30 & 1/1/0.81 & 0.85 & 0.81 & 0.67/0.68 & 0.71/0.85 & 0.86 & 0.69 \\ 
   & p=60 & 1/1/0.83 & - & 0.82 & 0.56/0.56 & 0.58/0.82 & 0.85 & 0.82 \\ 
   & p=180 & 1/1/0.85 & - & 0.83 & 0.47/0.47 & 0.42/0.84 & 0.87 & 0.86 \\ 
  \midrule\multirow{4}[2]{*}{lsnr} & p=14 & 0.72/0.72/0.78 & 0.78 & 0.79 & 0.98/1 & 0.83/0.9 & 0.88 & 0.93 \\ 
   & p=30 & 0.76/0.76/0.77 & 0.8 & 0.79 & 0.99/1 & 0.84/0.94 & 0.92 & 0.97 \\ 
   & p=60 & 1/1/0.93 & - & 0.93 & 0.94/0.94 & 0.77/0.96 & 0.94 & 0.97 \\ 
   & p=180 & 1/1/0.92 & - & 0.9 & 0.65/0.65 & 0.42/0.85 & 0.78 & 0.88 \\ 
   \midrule 
 \multicolumn{1}{|c}{} &       & \multicolumn{7}{c|}{Sparsistency (number of extra variables)} \\
\midrule\multirow{4}[2]{*}{hsnr} & p=14 & 6(0.3)/6(0.3)/6(0.9) & 6(0.7) & 6(0.9) & 6(3.4)/6(3.4) & 6(0.2)/6(0.3) & 6(0.6) & 6(1.9) \\ 
   & p=30 & 6(0.1)/6(0.1)/6(0.7) & 6(0.7) & 6(0.6) & 6(7.6)/6(8) & 6(0.9)/6(0.7) & 6(1.2) & 6(2.3) \\ 
   & p=60 & 6(0)/6(0)/6(1) & - & 6(0.5) & 6(11.1)/6(12.1) & 6(2.9)/6(1.4) & 6(1.4) & 6(0.8) \\ 
   & p=180 & 6(0)/6(0)/6(1.3) & - & 6(0.4) & 6(15.6)/6(18.5) & 6(9.5)/6(1.7) & 6(1.9) & 6(0.6) \\ 
  \midrule\multirow{4}[2]{*}{msnr} & p=14 & 5.9(1.2)/5.9(1.2)/6(1.7) & 6(1) & 6(1.6) & 6(4)/6(3.9) & 6(1)/6(1.2) & 5.9(1) & 6(3.3) \\ 
   & p=30 & 6(0.2)/6(0.2)/6(1.2) & 6(0.7) & 6(1) & 6(7.8)/6(8.2) & 6(3.1)/6(1.4) & 6(1.2) & 6(4.8) \\ 
   & p=60 & 6(0)/6(0)/6(1.1) & - & 6(0.6) & 6(11.1)/6(12.1) & 6(6.4)/6(1.5) & 6(1.2) & 6(1.1) \\ 
   & p=180 & 6(0)/6(0)/6(1.3) & - & 6(0.4) & 6(15.8)/6(18.5) & 6(18.7)/6(1.4) & 6(1.5) & 6(0.6) \\ 
  \midrule\multirow{4}[2]{*}{lsnr} & p=14 & 3.5(2.1)/3.5(2.1)/4.3(3) & 4(2.4) & 4.2(2.8) & 5.3(3.8)/5.4(3.8) & 3.9(1.8)/4.6(2.7) & 4.5(2.6) & 5(3.5) \\ 
   & p=30 & 4.1(2.7)/4.1(2.7)/4.6(4.5) & 4.5(3.2) & 4.5(3.7) & 5.6(7.7)/5.7(8) & 4.7(4)/5.1(5.3) & 5.1(5) & 5.5(7) \\ 
   & p=60 & 5(1.4)/5(1.4)/5.1(3.1) & - & 5.1(2.2) & 5.9(11.1)/5.9(12) & 5.3(8.2)/5.4(6) & 5.3(5.7) & 5.8(7.4) \\ 
   & p=180 & 5.6(0.6)/5.6(0.6)/5.6(2) & - & 5.6(0.9) & 6(15.7)/6(18.4) & 5.7(26.1)/5.6(3.6) & 5.5(5.3) & 5.9(3.1) \\ 
   \bottomrule 
\end{tabular}
}
\end{table}
