# Supplementary material for: On the Use of Information Criteria for Subset Selection in Least Squares Regression
Source: arXiv:1911.10191 source file (2021-03-06)
Supplement: Supplementary file 10 [file Sparse-Ex1_n200_rho_0.tex]

% latex table generated in R 3.6.2 by xtable 1.8-4 package
% Sat Dec 21 23:35:10 2019
\begin{table}[ht]
\centering
\caption{The performance of BOSS compared to other methods, Sparse-Ex1, $\rho$=0, n=200} 
\scalebox{0.7}{
\begin{tabular}{|c|c|ccccccc|}
  \toprule 
 \multicolumn{1}{|c}{} &       & BOSS  & BS    & FS    & LASSO & Gamma LASSO & SparseNet & \multicolumn{1}{c|}{rLASSO} \\
 \multicolumn{1}{|c}{} &       & C$_p$-hdf/AICc-hdf/CV & CV    & CV    & AICc/CV & AICc/CV & CV    & \multicolumn{1}{c|}{CV}  \\
 \cmidrule{3-9}\multicolumn{1}{|c}{} &       & \multicolumn{7}{c|}{\% worse than the best possible BOSS}  \\
 \midrule\multirow{4}[2]{*}{hsnr} & p=14 & 8/6/18 & 19 & 19 & 42/41 & 16/20 & 13 & 15 \\ 
   & p=30 & 5/3/23 & 25 & 23 & 71/69 & 32/23 & 14 & 19 \\ 
   & p=60 & 4/2/21 & - & 23 & 87/85 & 51/24 & 16 & 19 \\ 
   & p=180 & 34/1/19 & - & 22 & 119/121 & 134/25 & 17 & 19 \\ 
  \midrule\multirow{4}[2]{*}{msnr} & p=14 & 17/14/18 & 19 & 19 & 43/42 & 23/23 & 14 & 16 \\ 
   & p=30 & 15/11/23 & 25 & 23 & 71/69 & 49/28 & 16 & 20 \\ 
   & p=60 & 13/9/22 & - & 24 & 87/85 & 82/28 & 17 & 20 \\ 
   & p=180 & 44/7/20 & - & 22 & 119/121 & 222/30 & 17 & 20 \\ 
  \midrule\multirow{4}[2]{*}{lsnr} & p=14 & 22/24/25 & 26 & 25 & 8/9 & 13/15 & 18 & 15 \\ 
   & p=30 & 32/34/26 & 26 & 26 & 2/2 & 14/9 & 10 & 7 \\ 
   & p=60 & 27/29/24 & - & 24 & -1/-2 & 27/5 & 6 & 3 \\ 
   & p=180 & 32/22/18 & - & 19 & -4/-2 & 83/2 & 1 & 1 \\ 
   \midrule 
 \multicolumn{1}{|c}{} &       & \multicolumn{7}{c|}{Relative efficiency} \\
\midrule\multirow{4}[2]{*}{hsnr} & p=14 & 0.98/1/0.89 & 0.89 & 0.89 & 0.74/0.75 & 0.91/0.88 & 0.93 & 0.92 \\ 
   & p=30 & 0.98/1/0.84 & 0.82 & 0.83 & 0.6/0.61 & 0.78/0.83 & 0.9 & 0.87 \\ 
   & p=60 & 0.99/1/0.84 & - & 0.83 & 0.55/0.55 & 0.68/0.83 & 0.88 & 0.86 \\ 
   & p=180 & 0.75/1/0.85 & - & 0.83 & 0.46/0.46 & 0.43/0.81 & 0.87 & 0.85 \\ 
  \midrule\multirow{4}[2]{*}{msnr} & p=14 & 0.98/1/0.96 & 0.96 & 0.96 & 0.8/0.81 & 0.93/0.93 & 1 & 0.98 \\ 
   & p=30 & 0.96/1/0.9 & 0.89 & 0.9 & 0.65/0.66 & 0.75/0.87 & 0.96 & 0.93 \\ 
   & p=60 & 0.97/1/0.9 & - & 0.88 & 0.58/0.59 & 0.6/0.85 & 0.94 & 0.91 \\ 
   & p=180 & 0.75/1/0.9 & - & 0.88 & 0.49/0.49 & 0.33/0.83 & 0.91 & 0.89 \\ 
  \midrule\multirow{4}[2]{*}{lsnr} & p=14 & 0.89/0.88/0.87 & 0.86 & 0.86 & 1/1 & 0.95/0.94 & 0.92 & 0.95 \\ 
   & p=30 & 0.78/0.76/0.81 & 0.81 & 0.81 & 1/1 & 0.9/0.94 & 0.93 & 0.96 \\ 
   & p=60 & 0.77/0.76/0.79 & - & 0.79 & 1/1 & 0.78/0.94 & 0.93 & 0.96 \\ 
   & p=180 & 0.73/0.79/0.81 & - & 0.81 & 1/0.98 & 0.52/0.94 & 0.95 & 0.95 \\ 
   \midrule 
 \multicolumn{1}{|c}{} &       & \multicolumn{7}{c|}{Sparsistency (number of extra variables)} \\
\midrule\multirow{4}[2]{*}{hsnr} & p=14 & 6(0.4)/6(0.2)/6(0.6) & 6(0.6) & 6(0.6) & 6(3.8)/6(4.6) & 6(0.9)/6(1.4) & 6(0.7) & 6(0.6) \\ 
   & p=30 & 6(0.1)/6(0)/6(0.6) & 6(0.7) & 6(0.6) & 6(7.3)/6(8.4) & 6(2.3)/6(1.7) & 6(1) & 6(0.7) \\ 
   & p=60 & 6(0.1)/6(0)/6(0.5) & - & 6(0.5) & 6(10)/6(11.3) & 6(4.6)/6(1.8) & 6(1.4) & 6(0.7) \\ 
   & p=180 & 6(8.9)/6(0)/6(0.4) & - & 6(0.4) & 6(15.3)/6(20.3) & 6(18.1)/6(2.1) & 6(2.3) & 6(0.7) \\ 
  \midrule\multirow{4}[2]{*}{msnr} & p=14 & 6(0.8)/6(0.6)/6(0.6) & 6(0.6) & 6(0.6) & 6(3.8)/6(4.6) & 6(1.1)/6(1.4) & 6(0.6) & 6(0.6) \\ 
   & p=30 & 6(0.4)/6(0.2)/6(0.6) & 6(0.7) & 6(0.6) & 6(7.4)/6(8.4) & 6(2.9)/6(1.6) & 6(0.7) & 6(0.7) \\ 
   & p=60 & 6(0.2)/6(0.1)/6(0.5) & - & 6(0.5) & 6(10)/6(11.3) & 6(6.2)/6(1.6) & 6(1) & 6(0.8) \\ 
   & p=180 & 6(9.1)/6(0.1)/6(0.4) & - & 6(0.4) & 6(15.3)/6(20.3) & 6(27.7)/6(1.7) & 6(1.4) & 6(0.8) \\ 
  \midrule\multirow{4}[2]{*}{lsnr} & p=14 & 5.4(4.5)/5.2(4.1)/4.6(1.7) & 4.5(1.6) & 4.6(1.7) & 5.5(3.3)/5.5(3.9) & 5(1.5)/5.1(2.9) & 5(2.7) & 5(2.1) \\ 
   & p=30 & 4(4.7)/3.1(2.1)/3.7(2) & 3.7(2) & 3.7(2) & 5.3(6.4)/5.3(7.1) & 4.9(3.8)/4.8(4.9) & 4.8(5.3) & 4.6(3.6) \\ 
   & p=60 & 2.8(1.9)/2(0.3)/2.9(1.4) & - & 3(1.4) & 5.1(8.5)/5.2(9.2) & 4.8(8.1)/4.5(6.3) & 4.5(7) & 4.3(4.4) \\ 
   & p=180 & 2.1(13.8)/1(0.1)/1.8(0.8) & - & 1.8(0.8) & 4.4(11.8)/4.5(15.4) & 4.7(36.6)/3.8(10.1) & 4.1(11.9) & 3.7(7.5) \\ 
   \bottomrule 
\end{tabular}
}
\end{table}
