# Supplementary material for: On the Use of Information Criteria for Subset Selection in Least Squares Regression
Source: arXiv:1911.10191 source file (2021-03-06)
Supplement: Supplementary file 11 [file Sparse-Ex1_n200_rho_05.tex]

% latex table generated in R 3.6.2 by xtable 1.8-4 package
% Sat Dec 21 23:35:17 2019
\begin{table}[ht]
\centering
\caption{The performance of BOSS compared to other methods, Sparse-Ex1, $\rho$=0.5, n=200} 
\scalebox{0.7}{
\begin{tabular}{|c|c|ccccccc|}
  \toprule 
 \multicolumn{1}{|c}{} &       & BOSS  & BS    & FS    & LASSO & Gamma LASSO & SparseNet & \multicolumn{1}{c|}{rLASSO} \\
 \multicolumn{1}{|c}{} &       & C$_p$-hdf/AICc-hdf/CV & CV    & CV    & AICc/CV & AICc/CV & CV    & \multicolumn{1}{c|}{CV}  \\
 \cmidrule{3-9}\multicolumn{1}{|c}{} &       & \multicolumn{7}{c|}{\% worse than the best possible BOSS}  \\
 \midrule\multirow{4}[2]{*}{hsnr} & p=14 & 7/5/20 & 18 & 21 & 39/39 & 16/19 & 13 & 18 \\ 
   & p=30 & 4/2/20 & 22 & 21 & 66/65 & 34/21 & 15 & 18 \\ 
   & p=60 & 3/2/21 & - & 23 & 92/89 & 57/25 & 16 & 18 \\ 
   & p=180 & 65/1/19 & - & 22 & 139/134 & 136/25 & 16 & 16 \\ 
  \midrule\multirow{4}[2]{*}{msnr} & p=14 & 19/17/20 & 15 & 20 & 34/34 & 21/20 & 12 & 21 \\ 
   & p=30 & 13/9/22 & 23 & 23 & 66/65 & 50/26 & 17 & 26 \\ 
   & p=60 & 12/8/22 & - & 25 & 90/88 & 85/30 & 17 & 29 \\ 
   & p=180 & 46/9/21 & - & 25 & 126/125 & 211/31 & 18 & 39 \\ 
  \midrule\multirow{4}[2]{*}{lsnr} & p=14 & 19/22/23 & 23 & 21 & -2/-2 & 12/6 & 7 & 4 \\ 
   & p=30 & 26/27/25 & 24 & 23 & -4/-5 & 9/2 & 2 & -1 \\ 
   & p=60 & 24/26/22 & - & 20 & -4/-6 & 22/1 & 0 & -3 \\ 
   & p=180 & 48/12/14 & - & 14 & -2/-2 & 91/2 & 1 & 0 \\ 
   \midrule 
 \multicolumn{1}{|c}{} &       & \multicolumn{7}{c|}{Relative efficiency} \\
\midrule\multirow{4}[2]{*}{hsnr} & p=14 & 0.98/1/0.87 & 0.89 & 0.87 & 0.75/0.75 & 0.9/0.88 & 0.93 & 0.89 \\ 
   & p=30 & 0.99/1/0.85 & 0.84 & 0.84 & 0.61/0.62 & 0.77/0.85 & 0.89 & 0.87 \\ 
   & p=60 & 0.99/1/0.85 & - & 0.83 & 0.53/0.54 & 0.65/0.82 & 0.88 & 0.87 \\ 
   & p=180 & 0.61/1/0.85 & - & 0.83 & 0.42/0.43 & 0.43/0.81 & 0.87 & 0.87 \\ 
  \midrule\multirow{4}[2]{*}{msnr} & p=14 & 0.95/0.96/0.94 & 0.98 & 0.93 & 0.84/0.84 & 0.93/0.94 & 1 & 0.93 \\ 
   & p=30 & 0.97/1/0.9 & 0.89 & 0.89 & 0.66/0.66 & 0.73/0.87 & 0.93 & 0.87 \\ 
   & p=60 & 0.97/1/0.88 & - & 0.87 & 0.57/0.58 & 0.59/0.83 & 0.93 & 0.84 \\ 
   & p=180 & 0.75/1/0.9 & - & 0.88 & 0.48/0.49 & 0.35/0.83 & 0.93 & 0.79 \\ 
  \midrule\multirow{4}[2]{*}{lsnr} & p=14 & 0.82/0.8/0.8 & 0.8 & 0.81 & 1/1 & 0.88/0.92 & 0.91 & 0.94 \\ 
   & p=30 & 0.75/0.75/0.76 & 0.77 & 0.77 & 0.99/1 & 0.87/0.93 & 0.93 & 0.96 \\ 
   & p=60 & 0.76/0.75/0.77 & - & 0.78 & 0.99/1 & 0.77/0.94 & 0.95 & 0.97 \\ 
   & p=180 & 0.66/0.87/0.86 & - & 0.86 & 1/1 & 0.51/0.96 & 0.97 & 0.98 \\ 
   \midrule 
 \multicolumn{1}{|c}{} &       & \multicolumn{7}{c|}{Sparsistency (number of extra variables)} \\
\midrule\multirow{4}[2]{*}{hsnr} & p=14 & 6(0.3)/6(0.2)/6(0.8) & 6(0.6) & 6(0.8) & 6(3.8)/6(4.2) & 6(0.9)/6(1.3) & 6(0.6) & 6(1) \\ 
   & p=30 & 6(0.1)/6(0)/6(0.6) & 6(0.7) & 6(0.6) & 6(6)/6(8.6) & 6(2.5)/6(1.5) & 6(1.1) & 6(0.8) \\ 
   & p=60 & 6(0)/6(0)/6(0.5) & - & 6(0.6) & 6(8.8)/6(12.5) & 6(4.9)/6(1.7) & 6(1.4) & 6(0.9) \\ 
   & p=180 & 6(9.4)/6(0)/6(0.3) & - & 6(0.4) & 6(11.7)/6(21.3) & 6(16.6)/6(1.7) & 6(1.9) & 6(0.6) \\ 
  \midrule\multirow{4}[2]{*}{msnr} & p=14 & 6(1.2)/6(1)/6(1.1) & 6(0.7) & 6(1.1) & 6(3.8)/6(4.2) & 6(1.1)/6(1.5) & 6(0.7) & 6(1.7) \\ 
   & p=30 & 6(0.4)/6(0.2)/6(0.7) & 6(0.7) & 6(0.7) & 6(6.1)/6(8.6) & 6(3.1)/6(1.6) & 6(1) & 6(1.3) \\ 
   & p=60 & 6(0.2)/6(0.2)/6(0.6) & - & 6(0.6) & 6(8.8)/6(12.4) & 6(6.3)/6(1.8) & 6(1.1) & 6(1.6) \\ 
   & p=180 & 6(10.2)/6(0.1)/6(0.4) & - & 6(0.4) & 6(16)/6(21.1) & 6(26.5)/6(1.6) & 6(1.3) & 6(1.6) \\ 
  \midrule\multirow{4}[2]{*}{lsnr} & p=14 & 4.4(3.5)/4.1(3.2)/3.8(2.4) & 3.7(2) & 3.8(2.2) & 5(3.3)/5.1(3.5) & 4(1.6)/4.6(2.8) & 4.6(2.7) & 4.6(2.6) \\ 
   & p=30 & 3.7(4.4)/2.9(2.1)/3.4(2.7) & 3.3(2.3) & 3.4(2.3) & 4.8(4.8)/5.2(7.4) & 4.5(3.9)/4.7(5.2) & 4.8(5.7) & 4.6(4.5) \\ 
   & p=60 & 2.4(2)/1.6(0.5)/2.5(1.8) & - & 2.5(1.6) & 4.4(6.4)/4.8(10) & 4.4(8.2)/4.2(7) & 4.4(7.9) & 4.1(5.7) \\ 
   & p=180 & 1.3(14.1)/0.3(0.1)/1(0.8) & - & 1.1(0.7) & 2.5(4.9)/3.2(12) & 4.2(35.8)/2.9(9.2) & 3(9.7) & 2.7(7.5) \\ 
   \bottomrule 
\end{tabular}
}
\end{table}
