# Supplementary material for: On the Use of Information Criteria for Subset Selection in Least Squares Regression
Source: arXiv:1911.10191 source file (2021-03-06)
Supplement: Supplementary file 12 [file Sparse-Ex1_n200_rho_09.tex]

% latex table generated in R 3.6.2 by xtable 1.8-4 package
% Sat Dec 21 23:35:24 2019
\begin{table}[ht]
\centering
\caption{The performance of BOSS compared to other methods, Sparse-Ex1, $\rho$=0.9, n=200} 
\scalebox{0.7}{
\begin{tabular}{|c|c|ccccccc|}
  \toprule 
 \multicolumn{1}{|c}{} &       & BOSS  & BS    & FS    & LASSO & Gamma LASSO & SparseNet & \multicolumn{1}{c|}{rLASSO} \\
 \multicolumn{1}{|c}{} &       & C$_p$-hdf/AICc-hdf/CV & CV    & CV    & AICc/CV & AICc/CV & CV    & \multicolumn{1}{c|}{CV}  \\
 \cmidrule{3-9}\multicolumn{1}{|c}{} &       & \multicolumn{7}{c|}{\% worse than the best possible BOSS}  \\
 \midrule\multirow{4}[2]{*}{hsnr} & p=14 & 20/21/19 & 16 & 18 & 6/5 & 10/6 & 12 & 7 \\ 
   & p=30 & 16/16/28 & 15 & 28 & 24/24 & 26/16 & 12 & 25 \\ 
   & p=60 & 15/15/34 & - & 34 & 58/59 & 66/38 & 28 & 23 \\ 
   & p=180 & 59/8/35 & - & 36 & 98/98 & 153/45 & 27 & 23 \\ 
  \midrule\multirow{4}[2]{*}{msnr} & p=14 & 26/27/18 & 17 & 16 & -8/-9 & 11/1 & 3 & -3 \\ 
   & p=30 & 24/27/20 & 19 & 15 & -11/-12 & 5/-5 & -3 & -7 \\ 
   & p=60 & 16/16/19 & - & 16 & 2/3 & 27/6 & 8 & 0 \\ 
   & p=180 & 26/7/15 & - & 16 & 31/31 & 111/17 & 15 & 12 \\ 
  \midrule\multirow{4}[2]{*}{lsnr} & p=14 & 28/27/24 & 22 & 19 & -9/-13 & 9/3 & 3 & -1 \\ 
   & p=30 & 19/18/21 & 19 & 15 & -18/-21 & 5/-7 & -9 & -10 \\ 
   & p=60 & 17/18/20 & - & 14 & -20/-21 & 6/-12 & -14 & -18 \\ 
   & p=180 & 47/21/18 & - & 14 & -13/-14 & 53/-9 & -10 & -12 \\ 
   \midrule 
 \multicolumn{1}{|c}{} &       & \multicolumn{7}{c|}{Relative efficiency} \\
\midrule\multirow{4}[2]{*}{hsnr} & p=14 & 0.87/0.87/0.89 & 0.91 & 0.89 & 0.99/1 & 0.95/0.99 & 0.94 & 0.98 \\ 
   & p=30 & 0.97/0.97/0.87 & 0.98 & 0.88 & 0.91/0.91 & 0.89/0.96 & 1 & 0.89 \\ 
   & p=60 & 1/0.99/0.85 & - & 0.85 & 0.73/0.72 & 0.69/0.83 & 0.9 & 0.93 \\ 
   & p=180 & 0.68/1/0.8 & - & 0.79 & 0.55/0.54 & 0.43/0.74 & 0.85 & 0.88 \\ 
  \midrule\multirow{4}[2]{*}{msnr} & p=14 & 0.72/0.71/0.77 & 0.77 & 0.78 & 0.98/1 & 0.82/0.9 & 0.88 & 0.93 \\ 
   & p=30 & 0.71/0.69/0.74 & 0.74 & 0.76 & 0.99/1 & 0.84/0.93 & 0.91 & 0.95 \\ 
   & p=60 & 0.86/0.85/0.83 & - & 0.86 & 0.98/0.97 & 0.78/0.94 & 0.92 & 1 \\ 
   & p=180 & 0.86/1/0.93 & - & 0.92 & 0.82/0.82 & 0.51/0.92 & 0.93 & 0.96 \\ 
  \midrule\multirow{4}[2]{*}{lsnr} & p=14 & 0.68/0.68/0.7 & 0.71 & 0.73 & 0.95/1 & 0.8/0.85 & 0.85 & 0.88 \\ 
   & p=30 & 0.67/0.67/0.66 & 0.67 & 0.69 & 0.96/1 & 0.76/0.85 & 0.87 & 0.88 \\ 
   & p=60 & 0.68/0.67/0.66 & - & 0.69 & 0.98/1 & 0.74/0.89 & 0.92 & 0.96 \\ 
   & p=180 & 0.59/0.71/0.73 & - & 0.76 & 1/1 & 0.57/0.95 & 0.96 & 0.98 \\ 
   \midrule 
 \multicolumn{1}{|c}{} &       & \multicolumn{7}{c|}{Sparsistency (number of extra variables)} \\
\midrule\multirow{4}[2]{*}{hsnr} & p=14 & 5.6(2.8)/5.5(2.6)/5.7(2.8) & 5.6(1.9) & 5.6(2.6) & 5.9(4)/6(4) & 5.6(1.4)/5.8(2) & 5.6(2.2) & 5.9(3.8) \\ 
   & p=30 & 5.6(1.5)/5.6(1.2)/5.8(3.2) & 5.8(1.5) & 5.8(2.8) & 6(7.5)/6(8.6) & 5.8(3.4)/5.8(3.4) & 5.8(2.3) & 6(7.3) \\ 
   & p=60 & 5.9(1)/5.8(0.9)/5.9(2.8) & - & 5.9(1.9) & 6(10.2)/6(12.1) & 5.9(6.6)/5.9(4) & 5.9(3) & 6(3.1) \\ 
   & p=180 & 6(9.9)/5.9(0.4)/6(2.4) & - & 6(1.2) & 6(13.6)/6(18) & 6(21.6)/6(4.8) & 6(4.3) & 6(2.5) \\ 
  \midrule\multirow{4}[2]{*}{msnr} & p=14 & 2.9(2)/2.7(1.7)/3.7(2.9) & 3.5(2.4) & 3.6(2.7) & 4.9(3.7)/5(3.7) & 3.3(1.6)/4.2(2.6) & 4(2.6) & 4.6(3.4) \\ 
   & p=30 & 3.3(2.9)/3(2.1)/3.9(4.9) & 3.6(3.6) & 3.8(4.1) & 5.1(7.3)/5.3(8.2) & 4.1(3.8)/4.7(5.7) & 4.6(5.5) & 4.9(7.4) \\ 
   & p=60 & 4.3(2.8)/4.1(2.1)/4.4(4.3) & - & 4.4(3.2) & 5.6(10.1)/5.6(11.8) & 4.7(7.4)/5(6.9) & 5(6.8) & 5.5(7.9) \\ 
   & p=180 & 5.1(11.7)/5(1.2)/5(2.3) & - & 5(1.7) & 5.9(14.8)/5.9(17.5) & 5.3(28.6)/5.4(6.8) & 5.4(6.3) & 5.6(5.5) \\ 
  \midrule\multirow{4}[2]{*}{lsnr} & p=14 & 1(1)/0.9(0.9)/1.5(1.7) & 1.4(1.4) & 1.5(1.4) & 2.6(2.5)/2.9(2.7) & 1.5(1.4)/2(1.8) & 2(1.9) & 2.1(2.1) \\ 
   & p=30 & 0.9(1.8)/0.8(1.4)/1.2(2.9) & 1.1(2.4) & 1.2(2.2) & 2.2(4.8)/2.6(6) & 1.6(3.2)/2(4.2) & 2.1(4.5) & 1.9(4.5) \\ 
   & p=60 & 0.9(2)/0.7(1.4)/1.1(3.2) & - & 1.1(2.4) & 2.6(7)/2.9(9) & 2(6.5)/2.3(6.6) & 2.5(7.2) & 2.6(7.3) \\ 
   & p=180 & 1.3(14.7)/0.5(0.6)/1(2.6) & - & 1.2(1.9) & 2.8(9.7)/3.1(13.9) & 2.6(26.4)/2.6(10) & 2.8(11.4) & 2.7(9.4) \\ 
   \bottomrule 
\end{tabular}
}
\end{table}
