# Supplementary material for: On the Use of Information Criteria for Subset Selection in Least Squares Regression
Source: arXiv:1911.10191 source file (2021-03-06)
Supplement: Supplementary file 14 [file Sparse-Ex2_n2000_rho_05.tex]

% latex table generated in R 3.6.2 by xtable 1.8-4 package
% Sat Dec 21 23:35:45 2019
\begin{table}[ht]
\centering
\caption{The performance of BOSS compared to other methods, Sparse-Ex2, $\rho$=0.5, n=2000} 
\scalebox{0.7}{
\begin{tabular}{|c|c|ccccccc|}
  \toprule 
 \multicolumn{1}{|c}{} &       & BOSS  & BS    & FS    & LASSO & Gamma LASSO & SparseNet & \multicolumn{1}{c|}{rLASSO} \\
 \multicolumn{1}{|c}{} &       & C$_p$-hdf/AICc-hdf/CV & CV    & CV    & AICc/CV & AICc/CV & CV    & \multicolumn{1}{c|}{CV}  \\
 \cmidrule{3-9}\multicolumn{1}{|c}{} &       & \multicolumn{7}{c|}{\% worse than the best possible BOSS}  \\
 \midrule\multirow{4}[2]{*}{hsnr} & p=14 & 7/7/18 & 19 & 18 & 48/47 & 14/18 & 13 & 15 \\ 
   & p=30 & 4/3/23 & 22 & 23 & 86/83 & 20/18 & 12 & 16 \\ 
   & p=60 & 2/2/23 & - & 23 & 124/120 & 28/20 & 14 & 15 \\ 
   & p=180 & 1/1/21 & - & 21 & 174/171 & 46/20 & 14 & 15 \\ 
  \midrule\multirow{4}[2]{*}{msnr} & p=14 & 7/7/18 & 19 & 18 & 49/48 & 16/19 & 13 & 14 \\ 
   & p=30 & 4/3/23 & 22 & 23 & 85/83 & 25/20 & 12 & 16 \\ 
   & p=60 & 2/2/23 & - & 23 & 125/120 & 39/22 & 14 & 15 \\ 
   & p=180 & 1/1/21 & - & 21 & 174/171 & 77/23 & 13 & 15 \\ 
  \midrule\multirow{4}[2]{*}{lsnr} & p=14 & 12/12/23 & 19 & 18 & 50/48 & 21/23 & 13 & 14 \\ 
   & p=30 & 9/8/27 & 22 & 23 & 85/83 & 40/25 & 13 & 16 \\ 
   & p=60 & 8/8/26 & - & 23 & 124/120 & 72/28 & 14 & 15 \\ 
   & p=180 & 10/9/24 & - & 21 & 175/170 & 163/29 & 12 & 16 \\ 
   \midrule 
 \multicolumn{1}{|c}{} &       & \multicolumn{7}{c|}{Relative efficiency} \\
\midrule\multirow{4}[2]{*}{hsnr} & p=14 & 1/1/0.91 & 0.9 & 0.91 & 0.72/0.72 & 0.94/0.91 & 0.94 & 0.93 \\ 
   & p=30 & 1/1/0.84 & 0.85 & 0.84 & 0.56/0.56 & 0.86/0.87 & 0.92 & 0.89 \\ 
   & p=60 & 1/1/0.83 & - & 0.83 & 0.45/0.46 & 0.79/0.85 & 0.89 & 0.89 \\ 
   & p=180 & 1/1/0.84 & - & 0.84 & 0.37/0.37 & 0.69/0.84 & 0.89 & 0.88 \\ 
  \midrule\multirow{4}[2]{*}{msnr} & p=14 & 1/1/0.91 & 0.9 & 0.91 & 0.72/0.72 & 0.92/0.89 & 0.94 & 0.93 \\ 
   & p=30 & 1/1/0.84 & 0.85 & 0.84 & 0.56/0.56 & 0.83/0.86 & 0.92 & 0.89 \\ 
   & p=60 & 1/1/0.83 & - & 0.83 & 0.45/0.46 & 0.73/0.83 & 0.89 & 0.88 \\ 
   & p=180 & 1/1/0.84 & - & 0.84 & 0.37/0.37 & 0.57/0.82 & 0.89 & 0.88 \\ 
  \midrule\multirow{4}[2]{*}{lsnr} & p=14 & 1/1/0.91 & 0.94 & 0.95 & 0.75/0.76 & 0.92/0.91 & 0.99 & 0.98 \\ 
   & p=30 & 1/1/0.85 & 0.89 & 0.88 & 0.58/0.59 & 0.77/0.87 & 0.96 & 0.93 \\ 
   & p=60 & 1/1/0.85 & - & 0.88 & 0.48/0.49 & 0.63/0.84 & 0.95 & 0.93 \\ 
   & p=180 & 0.99/1/0.88 & - & 0.9 & 0.4/0.4 & 0.41/0.85 & 0.97 & 0.94 \\ 
   \midrule 
 \multicolumn{1}{|c}{} &       & \multicolumn{7}{c|}{Sparsistency (number of extra variables)} \\
\midrule\multirow{4}[2]{*}{hsnr} & p=14 & 6(0.3)/6(0.3)/6(0.6) & 6(0.7) & 6(0.6) & 6(4.7)/6(5.5) & 6(1)/6(1.4) & 6(0.7) & 6(0.5) \\ 
   & p=30 & 6(0.1)/6(0.1)/6(0.6) & 6(0.6) & 6(0.6) & 6(10.9)/6(11.3) & 6(2.1)/6(1.9) & 6(0.9) & 6(0.5) \\ 
   & p=60 & 6(0)/6(0)/6(0.5) & - & 6(0.5) & 6(18.1)/6(17.7) & 6(3.8)/6(2.1) & 6(1.4) & 6(0.4) \\ 
   & p=180 & 6(0)/6(0)/6(0.3) & - & 6(0.3) & 6(32.2)/6(29.7) & 6(9.2)/6(2.4) & 6(2.1) & 6(0.3) \\ 
  \midrule\multirow{4}[2]{*}{msnr} & p=14 & 6(0.3)/6(0.3)/6(0.6) & 6(0.7) & 6(0.6) & 6(4.8)/6(5.5) & 6(1)/6(1.5) & 6(0.6) & 6(0.5) \\ 
   & p=30 & 6(0.1)/6(0.1)/6(0.6) & 6(0.6) & 6(0.6) & 6(11)/6(11.3) & 6(2.3)/6(1.7) & 6(0.9) & 6(0.5) \\ 
   & p=60 & 6(0)/6(0)/6(0.5) & - & 6(0.5) & 6(18.1)/6(17.7) & 6(4.6)/6(1.8) & 6(1.4) & 6(0.4) \\ 
   & p=180 & 6(0)/6(0)/6(0.3) & - & 6(0.3) & 6(32.3)/6(29.7) & 6(13.4)/6(1.8) & 6(2) & 6(0.3) \\ 
  \midrule\multirow{4}[2]{*}{lsnr} & p=14 & 6(0.6)/6(0.5)/6(0.6) & 6(0.7) & 6(0.6) & 6(4.8)/6(5.5) & 6(1.1)/6(1.5) & 6(0.6) & 6(0.5) \\ 
   & p=30 & 6(0.2)/6(0.2)/6(0.6) & 6(0.6) & 6(0.6) & 6(10.9)/6(11.3) & 6(2.8)/6(1.5) & 6(0.8) & 6(0.5) \\ 
   & p=60 & 6(0.1)/6(0.1)/6(0.5) & - & 6(0.5) & 6(18.1)/6(17.8) & 6(6.4)/6(1.4) & 6(1.1) & 6(0.4) \\ 
   & p=180 & 6(0.1)/6(0.1)/6(0.3) & - & 6(0.3) & 6(32.5)/6(29.7) & 6(21.7)/6(1.1) & 6(1.2) & 6(0.4) \\ 
   \bottomrule 
\end{tabular}
}
\end{table}
