# Supplementary material for: On the Use of Information Criteria for Subset Selection in Least Squares Regression
Source: arXiv:1911.10191 source file (2021-03-06)
Supplement: Supplementary file 15 [file Sparse-Ex2_n2000_rho_09.tex]

% latex table generated in R 3.6.2 by xtable 1.8-4 package
% Sat Dec 21 23:35:52 2019
\begin{table}[ht]
\centering
\caption{The performance of BOSS compared to other methods, Sparse-Ex2, $\rho$=0.9, n=2000} 
\scalebox{0.7}{
\begin{tabular}{|c|c|ccccccc|}
  \toprule 
 \multicolumn{1}{|c}{} &       & BOSS  & BS    & FS    & LASSO & Gamma LASSO & SparseNet & \multicolumn{1}{c|}{rLASSO} \\
 \multicolumn{1}{|c}{} &       & C$_p$-hdf/AICc-hdf/CV & CV    & CV    & AICc/CV & AICc/CV & CV    & \multicolumn{1}{c|}{CV}  \\
 \cmidrule{3-9}\multicolumn{1}{|c}{} &       & \multicolumn{7}{c|}{\% worse than the best possible BOSS}  \\
 \midrule\multirow{4}[2]{*}{hsnr} & p=14 & 7/7/18 & 19 & 18 & 56/55 & 22/28 & 14 & 15 \\ 
   & p=30 & 4/3/23 & 22 & 23 & 118/116 & 29/29 & 14 & 17 \\ 
   & p=60 & 2/2/23 & - & 23 & 186/182 & 37/33 & 15 & 15 \\ 
   & p=180 & 1/1/21 & - & 21 & 299/294 & 51/41 & 15 & 13 \\ 
  \midrule\multirow{4}[2]{*}{msnr} & p=14 & 8/8/18 & 19 & 18 & 56/55 & 23/29 & 14 & 14 \\ 
   & p=30 & 4/4/24 & 22 & 23 & 118/115 & 31/30 & 13 & 17 \\ 
   & p=60 & 3/3/23 & - & 23 & 185/182 & 42/36 & 16 & 15 \\ 
   & p=180 & 3/3/22 & - & 21 & 298/293 & 61/43 & 14 & 13 \\ 
  \midrule\multirow{4}[2]{*}{lsnr} & p=14 & 36/36/42 & 15 & 19 & 52/50 & 22/30 & 12 & 23 \\ 
   & p=30 & 37/36/43 & 12 & 32 & 100/97 & 28/26 & 7 & 40 \\ 
   & p=60 & 39/38/47 & - & 47 & 141/138 & 35/22 & 1 & 61 \\ 
   & p=180 & 38/38/37 & - & 72 & 178/175 & 45/16 & -12 & 100 \\ 
   \midrule 
 \multicolumn{1}{|c}{} &       & \multicolumn{7}{c|}{Relative efficiency} \\
\midrule\multirow{4}[2]{*}{hsnr} & p=14 & 1/1/0.91 & 0.9 & 0.91 & 0.68/0.69 & 0.88/0.84 & 0.94 & 0.93 \\ 
   & p=30 & 1/1/0.84 & 0.85 & 0.84 & 0.47/0.48 & 0.8/0.8 & 0.9 & 0.88 \\ 
   & p=60 & 1/1/0.83 & - & 0.83 & 0.35/0.36 & 0.74/0.76 & 0.88 & 0.88 \\ 
   & p=180 & 1/1/0.84 & - & 0.84 & 0.25/0.26 & 0.67/0.72 & 0.88 & 0.89 \\ 
  \midrule\multirow{4}[2]{*}{msnr} & p=14 & 1/1/0.91 & 0.91 & 0.92 & 0.69/0.7 & 0.88/0.83 & 0.94 & 0.94 \\ 
   & p=30 & 1/1/0.84 & 0.85 & 0.84 & 0.48/0.48 & 0.79/0.8 & 0.91 & 0.89 \\ 
   & p=60 & 1/1/0.84 & - & 0.84 & 0.36/0.36 & 0.72/0.76 & 0.88 & 0.9 \\ 
   & p=180 & 1/1/0.84 & - & 0.85 & 0.26/0.26 & 0.64/0.72 & 0.9 & 0.91 \\ 
  \midrule\multirow{4}[2]{*}{lsnr} & p=14 & 0.83/0.83/0.79 & 0.98 & 0.94 & 0.74/0.75 & 0.92/0.87 & 1 & 0.91 \\ 
   & p=30 & 0.79/0.79/0.75 & 0.96 & 0.81 & 0.54/0.54 & 0.84/0.85 & 1 & 0.76 \\ 
   & p=60 & 0.72/0.73/0.68 & - & 0.69 & 0.42/0.42 & 0.75/0.83 & 1 & 0.63 \\ 
   & p=180 & 0.64/0.64/0.64 & - & 0.51 & 0.32/0.32 & 0.61/0.76 & 1 & 0.44 \\ 
   \midrule 
 \multicolumn{1}{|c}{} &       & \multicolumn{7}{c|}{Sparsistency (number of extra variables)} \\
\midrule\multirow{4}[2]{*}{hsnr} & p=14 & 6(0.3)/6(0.3)/6(0.6) & 6(0.7) & 6(0.6) & 6(6.6)/6(7.2) & 6(1.5)/6(2.1) & 6(0.7) & 6(0.5) \\ 
   & p=30 & 6(0.1)/6(0.1)/6(0.6) & 6(0.6) & 6(0.6) & 6(17.8)/6(18.9) & 6(2.7)/6(2.6) & 6(0.9) & 6(0.5) \\ 
   & p=60 & 6(0)/6(0)/6(0.5) & - & 6(0.5) & 6(34.2)/6(35.3) & 6(4.5)/6(2.9) & 6(1.4) & 6(0.4) \\ 
   & p=180 & 6(0)/6(0)/6(0.3) & - & 6(0.3) & 6(72.8)/6(73.6) & 6(8.7)/6(3.9) & 6(2.2) & 6(0.2) \\ 
  \midrule\multirow{4}[2]{*}{msnr} & p=14 & 6(0.3)/6(0.3)/6(0.6) & 6(0.7) & 6(0.6) & 6(6.6)/6(7.2) & 6(1.5)/6(2.2) & 6(0.7) & 6(0.5) \\ 
   & p=30 & 6(0.1)/6(0.1)/6(0.6) & 6(0.6) & 6(0.6) & 6(17.8)/6(18.8) & 6(2.8)/6(2.3) & 6(0.9) & 6(0.5) \\ 
   & p=60 & 6(0)/6(0)/6(0.5) & - & 6(0.5) & 6(34.2)/6(35.2) & 6(4.8)/6(2.6) & 6(1.4) & 6(0.4) \\ 
   & p=180 & 6(0)/6(0)/6(0.3) & - & 6(0.3) & 6(72.8)/6(73.6) & 6(10.5)/6(3.3) & 6(2.1) & 6(0.2) \\ 
  \midrule\multirow{4}[2]{*}{lsnr} & p=14 & 6(2.7)/6(2.6)/6(0.6) & 6(0.7) & 6(0.9) & 6(6.6)/6(7.2) & 6(1.5)/6(2.5) & 6(0.8) & 6(1.3) \\ 
   & p=30 & 6(2.1)/6(2)/6(0.8) & 6(0.6) & 6(1.5) & 6(17.8)/6(18.8) & 6(3.2)/6(2.7) & 6(1.4) & 6(2.5) \\ 
   & p=60 & 6(1)/6(0.9)/6(0.9) & - & 6(2.2) & 6(34.2)/6(35.1) & 6(6.3)/6(3.7) & 6(2.6) & 6(3.9) \\ 
   & p=180 & 6(1.4)/6(1.4)/6(1.8) & - & 6(4.6) & 6(72.3)/6(73.5) & 6(17.1)/6(8.4) & 6(7.1) & 6(10.4) \\ 
   \bottomrule 
\end{tabular}
}
\end{table}
