# Supplementary material for: On the Use of Information Criteria for Subset Selection in Least Squares Regression
Source: arXiv:1911.10191 source file (2021-03-06)
Supplement: Supplementary file 16 [file Sparse-Ex2_n200_rho_0.tex]

% latex table generated in R 3.6.2 by xtable 1.8-4 package
% Sat Dec 21 23:35:32 2019
\begin{table}[ht]
\centering
\caption{The performance of BOSS compared to other methods, Sparse-Ex2, $\rho$=0, n=200} 
\scalebox{0.7}{
\begin{tabular}{|c|c|ccccccc|}
  \toprule 
 \multicolumn{1}{|c}{} &       & BOSS  & BS    & FS    & LASSO & Gamma LASSO & SparseNet & \multicolumn{1}{c|}{rLASSO} \\
 \multicolumn{1}{|c}{} &       & C$_p$-hdf/AICc-hdf/CV & CV    & CV    & AICc/CV & AICc/CV & CV    & \multicolumn{1}{c|}{CV}  \\
 \cmidrule{3-9}\multicolumn{1}{|c}{} &       & \multicolumn{7}{c|}{\% worse than the best possible BOSS}  \\
 \midrule\multirow{4}[2]{*}{hsnr} & p=14 & 8/6/20 & 21 & 20 & 41/41 & 17/20 & 15 & 16 \\ 
   & p=30 & 5/3/24 & 25 & 25 & 69/68 & 32/22 & 15 & 20 \\ 
   & p=60 & 4/2/21 & - & 23 & 95/94 & 53/23 & 16 & 19 \\ 
   & p=180 & 34/1/19 & - & 21 & 129/130 & 139/27 & 18 & 17 \\ 
  \midrule\multirow{4}[2]{*}{msnr} & p=14 & 17/14/20 & 21 & 20 & 42/41 & 23/23 & 16 & 17 \\ 
   & p=30 & 17/13/24 & 25 & 25 & 69/68 & 48/27 & 16 & 21 \\ 
   & p=60 & 13/9/21 & - & 23 & 95/94 & 84/28 & 16 & 23 \\ 
   & p=180 & 49/10/20 & - & 22 & 129/130 & 224/32 & 18 & 29 \\ 
  \midrule\multirow{4}[2]{*}{lsnr} & p=14 & 21/22/24 & 25 & 24 & 7/7 & 14/14 & 16 & 12 \\ 
   & p=30 & 29/31/26 & 25 & 26 & 1/1 & 13/8 & 8 & 6 \\ 
   & p=60 & 26/28/23 & - & 22 & 0/0 & 25/5 & 6 & 5 \\ 
   & p=180 & 31/18/15 & - & 16 & -2/0 & 85/4 & 3 & 3 \\ 
   \midrule 
 \multicolumn{1}{|c}{} &       & \multicolumn{7}{c|}{Relative efficiency} \\
\midrule\multirow{4}[2]{*}{hsnr} & p=14 & 0.98/1/0.89 & 0.88 & 0.89 & 0.75/0.75 & 0.91/0.89 & 0.92 & 0.91 \\ 
   & p=30 & 0.98/1/0.83 & 0.82 & 0.82 & 0.61/0.61 & 0.78/0.84 & 0.9 & 0.86 \\ 
   & p=60 & 0.99/1/0.85 & - & 0.83 & 0.52/0.53 & 0.67/0.83 & 0.88 & 0.86 \\ 
   & p=180 & 0.75/1/0.85 & - & 0.84 & 0.44/0.44 & 0.42/0.8 & 0.86 & 0.86 \\ 
  \midrule\multirow{4}[2]{*}{msnr} & p=14 & 0.98/1/0.95 & 0.94 & 0.95 & 0.8/0.81 & 0.93/0.93 & 0.98 & 0.98 \\ 
   & p=30 & 0.96/1/0.91 & 0.9 & 0.9 & 0.67/0.67 & 0.76/0.89 & 0.97 & 0.93 \\ 
   & p=60 & 0.97/1/0.9 & - & 0.89 & 0.56/0.56 & 0.59/0.85 & 0.94 & 0.89 \\ 
   & p=180 & 0.74/1/0.92 & - & 0.9 & 0.48/0.48 & 0.34/0.83 & 0.93 & 0.85 \\ 
  \midrule\multirow{4}[2]{*}{lsnr} & p=14 & 0.89/0.88/0.86 & 0.86 & 0.86 & 1/1 & 0.94/0.94 & 0.92 & 0.95 \\ 
   & p=30 & 0.78/0.77/0.8 & 0.8 & 0.8 & 1/1 & 0.89/0.93 & 0.93 & 0.95 \\ 
   & p=60 & 0.79/0.78/0.81 & - & 0.81 & 1/0.99 & 0.8/0.95 & 0.94 & 0.95 \\ 
   & p=180 & 0.75/0.83/0.85 & - & 0.85 & 1/0.98 & 0.53/0.94 & 0.95 & 0.95 \\ 
   \midrule 
 \multicolumn{1}{|c}{} &       & \multicolumn{7}{c|}{Sparsistency (number of extra variables)} \\
\midrule\multirow{4}[2]{*}{hsnr} & p=14 & 6(0.3)/6(0.2)/6(0.6) & 6(0.7) & 6(0.6) & 6(3.6)/6(4.4) & 6(1)/6(1.4) & 6(0.6) & 6(0.6) \\ 
   & p=30 & 6(0.1)/6(0)/6(0.6) & 6(0.7) & 6(0.7) & 6(7.5)/6(8.4) & 6(2.4)/6(1.7) & 6(1.1) & 6(0.8) \\ 
   & p=60 & 6(0.1)/6(0)/6(0.5) & - & 6(0.5) & 6(11.4)/6(13.2) & 6(4.8)/6(1.6) & 6(1.6) & 6(0.7) \\ 
   & p=180 & 6(8.8)/6(0)/6(0.4) & - & 6(0.4) & 6(15.9)/6(22.1) & 6(18.5)/6(2.2) & 6(2.6) & 6(0.7) \\ 
  \midrule\multirow{4}[2]{*}{msnr} & p=14 & 6(0.8)/6(0.6)/6(0.6) & 6(0.7) & 6(0.6) & 6(3.6)/6(4.4) & 6(1.1)/6(1.4) & 6(0.6) & 6(0.6) \\ 
   & p=30 & 6(0.5)/6(0.2)/6(0.6) & 6(0.7) & 6(0.7) & 6(7.4)/6(8.5) & 6(2.9)/6(1.6) & 6(0.8) & 6(0.9) \\ 
   & p=60 & 6(0.2)/6(0.1)/6(0.5) & - & 6(0.5) & 6(11.3)/6(13.2) & 6(6.4)/6(1.5) & 6(1) & 6(0.9) \\ 
   & p=180 & 6(9.8)/6(0.1)/6(0.4) & - & 6(0.4) & 6(15.9)/6(22) & 6(27.5)/6(2) & 6(1.6) & 6(1.3) \\ 
  \midrule\multirow{4}[2]{*}{lsnr} & p=14 & 5.5(4.5)/5.4(4.2)/4.8(1.8) & 4.8(1.7) & 4.8(1.8) & 5.7(3.3)/5.7(4) & 5.1(1.5)/5.3(2.9) & 5.2(2.8) & 5.2(2) \\ 
   & p=30 & 3.9(4.3)/3.1(1.8)/3.6(2.2) & 3.6(2) & 3.6(2.1) & 5.3(6.6)/5.3(7.1) & 4.8(3.8)/4.7(4.9) & 4.8(5.3) & 4.5(3.6) \\ 
   & p=60 & 2.3(1.8)/1.4(0.3)/2.7(1.4) & - & 2.7(1.4) & 4.7(8.8)/4.7(9.9) & 4.9(8.6)/4.2(6.9) & 4.3(7.5) & 4(5.5) \\ 
   & p=180 & 1.7(14.1)/0.5(0.1)/1.4(0.6) & - & 1.4(0.7) & 3.7(10.7)/3.8(13.5) & 4.6(36.7)/3.2(9.4) & 3.3(10.3) & 3.1(8) \\ 
   \bottomrule 
\end{tabular}
}
\end{table}
