# Supplementary material for: On the Use of Information Criteria for Subset Selection in Least Squares Regression
Source: arXiv:1911.10191 source file (2021-03-06)
Supplement: Supplementary file 17 [file Sparse-Ex2_n200_rho_05.tex]

% latex table generated in R 3.6.2 by xtable 1.8-4 package
% Sat Dec 21 23:35:39 2019
\begin{table}[ht]
\centering
\caption{The performance of BOSS compared to other methods, Sparse-Ex2, $\rho$=0.5, n=200} 
\scalebox{0.7}{
\begin{tabular}{|c|c|ccccccc|}
  \toprule 
 \multicolumn{1}{|c}{} &       & BOSS  & BS    & FS    & LASSO & Gamma LASSO & SparseNet & \multicolumn{1}{c|}{rLASSO} \\
 \multicolumn{1}{|c}{} &       & C$_p$-hdf/AICc-hdf/CV & CV    & CV    & AICc/CV & AICc/CV & CV    & \multicolumn{1}{c|}{CV}  \\
 \cmidrule{3-9}\multicolumn{1}{|c}{} &       & \multicolumn{7}{c|}{\% worse than the best possible BOSS}  \\
 \midrule\multirow{4}[2]{*}{hsnr} & p=14 & 8/6/17 & 18 & 17 & 46/44 & 15/20 & 13 & 15 \\ 
   & p=30 & 5/3/24 & 24 & 24 & 91/88 & 28/23 & 14 & 18 \\ 
   & p=60 & 4/2/22 & - & 23 & 123/119 & 43/24 & 16 & 17 \\ 
   & p=180 & 34/1/19 & - & 22 & 168/165 & 100/28 & 17 & 15 \\ 
  \midrule\multirow{4}[2]{*}{msnr} & p=14 & 19/16/26 & 18 & 17 & 46/44 & 21/23 & 14 & 16 \\ 
   & p=30 & 22/18/29 & 23 & 25 & 89/87 & 42/28 & 14 & 41 \\ 
   & p=60 & 16/11/29 & - & 25 & 121/117 & 70/29 & 16 & 42 \\ 
   & p=180 & 48/9/29 & - & 30 & 160/157 & 179/32 & 14 & 52 \\ 
  \midrule\multirow{4}[2]{*}{lsnr} & p=14 & 24/25/28 & 23 & 26 & 18/17 & 15/20 & 22 & 23 \\ 
   & p=30 & 33/34/26 & 20 & 30 & 17/17 & 15/19 & 18 & 22 \\ 
   & p=60 & 28/29/23 & - & 28 & 15/16 & 23/17 & 16 & 19 \\ 
   & p=180 & 28/14/14 & - & 17 & 8/9 & 71/11 & 10 & 12 \\ 
   \midrule 
 \multicolumn{1}{|c}{} &       & \multicolumn{7}{c|}{Relative efficiency} \\
\midrule\multirow{4}[2]{*}{hsnr} & p=14 & 0.98/1/0.91 & 0.9 & 0.91 & 0.73/0.74 & 0.92/0.89 & 0.94 & 0.92 \\ 
   & p=30 & 0.98/1/0.83 & 0.83 & 0.83 & 0.54/0.55 & 0.8/0.84 & 0.9 & 0.87 \\ 
   & p=60 & 0.98/1/0.83 & - & 0.83 & 0.46/0.46 & 0.71/0.82 & 0.88 & 0.87 \\ 
   & p=180 & 0.75/1/0.85 & - & 0.83 & 0.38/0.38 & 0.5/0.79 & 0.86 & 0.88 \\ 
  \midrule\multirow{4}[2]{*}{msnr} & p=14 & 0.96/0.98/0.9 & 0.97 & 0.97 & 0.78/0.79 & 0.94/0.92 & 1 & 0.98 \\ 
   & p=30 & 0.93/0.97/0.88 & 0.92 & 0.91 & 0.6/0.61 & 0.8/0.89 & 1 & 0.81 \\ 
   & p=60 & 0.96/1/0.86 & - & 0.89 & 0.5/0.51 & 0.66/0.87 & 0.96 & 0.78 \\ 
   & p=180 & 0.74/1/0.84 & - & 0.83 & 0.42/0.42 & 0.39/0.83 & 0.95 & 0.71 \\ 
  \midrule\multirow{4}[2]{*}{lsnr} & p=14 & 0.92/0.92/0.9 & 0.94 & 0.91 & 0.97/0.98 & 1/0.96 & 0.94 & 0.94 \\ 
   & p=30 & 0.87/0.86/0.92 & 0.96 & 0.88 & 0.99/0.98 & 1/0.96 & 0.98 & 0.94 \\ 
   & p=60 & 0.89/0.89/0.93 & - & 0.89 & 1/0.99 & 0.93/0.98 & 0.99 & 0.96 \\ 
   & p=180 & 0.84/0.94/0.94 & - & 0.92 & 1/0.99 & 0.63/0.97 & 0.98 & 0.96 \\ 
   \midrule 
 \multicolumn{1}{|c}{} &       & \multicolumn{7}{c|}{Sparsistency (number of extra variables)} \\
\midrule\multirow{4}[2]{*}{hsnr} & p=14 & 6(0.4)/6(0.3)/6(0.6) & 6(0.6) & 6(0.6) & 6(4.6)/6(5.5) & 6(0.9)/6(1.5) & 6(0.7) & 6(0.6) \\ 
   & p=30 & 6(0.1)/6(0)/6(0.7) & 6(0.7) & 6(0.7) & 6(11.2)/6(12.8) & 6(2.2)/6(1.5) & 6(1.1) & 6(0.7) \\ 
   & p=60 & 6(0.1)/6(0)/6(0.5) & - & 6(0.5) & 6(16)/6(19.1) & 6(4.3)/6(1.5) & 6(1.7) & 6(0.6) \\ 
   & p=180 & 6(9.3)/6(0)/6(0.4) & - & 6(0.4) & 6(22.5)/6(31.5) & 6(14.2)/6(2.1) & 6(2.8) & 6(0.6) \\ 
  \midrule\multirow{4}[2]{*}{msnr} & p=14 & 6(0.9)/6(0.8)/6(0.6) & 6(0.6) & 6(0.6) & 6(4.6)/6(5.5) & 6(1.1)/6(1.6) & 6(0.7) & 6(0.6) \\ 
   & p=30 & 6(0.6)/6(0.4)/6(0.7) & 6(0.7) & 6(0.7) & 6(11.2)/6(12.8) & 6(2.7)/6(1.5) & 6(0.9) & 6(2) \\ 
   & p=60 & 6(0.3)/6(0.2)/6(0.5) & - & 6(0.6) & 6(16)/6(19.1) & 6(5.6)/6(1.3) & 6(1.4) & 6(1.9) \\ 
   & p=180 & 6(10.1)/6(0.1)/6(0.5) & - & 6(0.7) & 6(22.3)/6(31.6) & 6(23.9)/6(2) & 6(2.1) & 6(2.5) \\ 
  \midrule\multirow{4}[2]{*}{lsnr} & p=14 & 5.7(4.8)/5.6(4.5)/5.1(1.6) & 5.1(1.4) & 5.1(1.9) & 5.7(4.3)/5.7(5.1) & 5.4(1.6)/5.5(3.7) & 5.3(2.7) & 5.4(3.2) \\ 
   & p=30 & 3.6(5.3)/2.4(2.2)/3.9(2.4) & 3.9(1.9) & 3.5(2.8) & 4.5(8)/4.4(8.9) & 5(4.7)/4.3(6.5) & 4.2(5.3) & 3.9(6.1) \\ 
   & p=60 & 2.3(2.4)/1(0.3)/3.1(2.1) & - & 2.5(1.8) & 3.8(9.8)/3.7(10.9) & 5(9)/3.7(8.1) & 3.7(7) & 3.3(7.8) \\ 
   & p=180 & 1.7(14.9)/0.4(0.1)/1.4(1.1) & - & 0.9(0.8) & 2.4(9.8)/2.4(12.9) & 4.5(35.8)/2.3(11) & 2.3(9.3) & 2.1(9.1) \\ 
   \bottomrule 
\end{tabular}
}
\end{table}
