# Supplementary material for: On the Use of Information Criteria for Subset Selection in Least Squares Regression
Source: arXiv:1911.10191 source file (2021-03-06)
Supplement: Supplementary file 18 [file Sparse-Ex2_n200_rho_09.tex]

% latex table generated in R 3.6.2 by xtable 1.8-4 package
% Sat Dec 21 23:35:46 2019
\begin{table}[ht]
\centering
\caption{The performance of BOSS compared to other methods, Sparse-Ex2, $\rho$=0.9, n=200} 
\scalebox{0.7}{
\begin{tabular}{|c|c|ccccccc|}
  \toprule 
 \multicolumn{1}{|c}{} &       & BOSS  & BS    & FS    & LASSO & Gamma LASSO & SparseNet & \multicolumn{1}{c|}{rLASSO} \\
 \multicolumn{1}{|c}{} &       & C$_p$-hdf/AICc-hdf/CV & CV    & CV    & AICc/CV & AICc/CV & CV    & \multicolumn{1}{c|}{CV}  \\
 \cmidrule{3-9}\multicolumn{1}{|c}{} &       & \multicolumn{7}{c|}{\% worse than the best possible BOSS}  \\
 \midrule\multirow{4}[2]{*}{hsnr} & p=14 & 18/15/25 & 17 & 23 & 53/51 & 20/27 & 14 & 18 \\ 
   & p=30 & 12/9/42 & 9 & 53 & 91/89 & 18/18 & 1 & 40 \\ 
   & p=60 & 9/6/49 & - & 69 & 131/126 & 16/12 & -6 & 48 \\ 
   & p=180 & 22/5/75 & - & 111 & 138/120 & -7/-16 & -30 & 42 \\ 
  \midrule\multirow{4}[2]{*}{msnr} & p=14 & 25/23/29 & 3 & 24 & 35/34 & 10/16 & 3 & 21 \\ 
   & p=30 & 23/20/31 & -15 & 36 & 50/48 & -1/2 & -17 & 34 \\ 
   & p=60 & 21/18/30 & - & 48 & 65/61 & -7/-7 & -26 & 46 \\ 
   & p=180 & 23/22/20 & - & 64 & 48/35 & -16/-1 & -24 & 32 \\ 
  \midrule\multirow{4}[2]{*}{lsnr} & p=14 & 40/41/31 & 32 & 50 & 41/40 & 38/39 & 39 & 43 \\ 
   & p=30 & 42/42/28 & 28 & 61 & 53/53 & 44/51 & 46 & 56 \\ 
   & p=60 & 36/35/25 & - & 50 & 45/45 & 52/47 & 45 & 48 \\ 
   & p=180 & 25/9/11 & - & 15 & 10/11 & 59/12 & 12 & 13 \\ 
   \midrule 
 \multicolumn{1}{|c}{} &       & \multicolumn{7}{c|}{Relative efficiency} \\
\midrule\multirow{4}[2]{*}{hsnr} & p=14 & 0.97/0.99/0.91 & 0.97 & 0.93 & 0.75/0.75 & 0.95/0.89 & 1 & 0.97 \\ 
   & p=30 & 0.9/0.92/0.71 & 0.93 & 0.66 & 0.53/0.53 & 0.86/0.85 & 1 & 0.72 \\ 
   & p=60 & 0.87/0.89/0.63 & - & 0.56 & 0.41/0.42 & 0.81/0.84 & 1 & 0.64 \\ 
   & p=180 & 0.58/0.67/0.4 & - & 0.33 & 0.3/0.32 & 0.76/0.84 & 1 & 0.49 \\ 
  \midrule\multirow{4}[2]{*}{msnr} & p=14 & 0.82/0.83/0.79 & 0.99 & 0.83 & 0.76/0.77 & 0.94/0.88 & 1 & 0.85 \\ 
   & p=30 & 0.68/0.69/0.63 & 0.98 & 0.61 & 0.55/0.56 & 0.84/0.82 & 1 & 0.62 \\ 
   & p=60 & 0.61/0.62/0.57 & - & 0.5 & 0.45/0.46 & 0.79/0.79 & 1 & 0.51 \\ 
   & p=180 & 0.62/0.62/0.63 & - & 0.46 & 0.51/0.56 & 0.9/0.76 & 1 & 0.57 \\ 
  \midrule\multirow{4}[2]{*}{lsnr} & p=14 & 0.94/0.93/1 & 0.99 & 0.87 & 0.92/0.93 & 0.95/0.94 & 0.94 & 0.92 \\ 
   & p=30 & 0.9/0.9/1 & 1 & 0.8 & 0.83/0.84 & 0.89/0.85 & 0.88 & 0.82 \\ 
   & p=60 & 0.92/0.93/1 & - & 0.83 & 0.86/0.86 & 0.83/0.85 & 0.87 & 0.85 \\ 
   & p=180 & 0.87/1/0.98 & - & 0.95 & 0.98/0.98 & 0.68/0.97 & 0.97 & 0.96 \\ 
   \midrule 
 \multicolumn{1}{|c}{} &       & \multicolumn{7}{c|}{Sparsistency (number of extra variables)} \\
\midrule\multirow{4}[2]{*}{hsnr} & p=14 & 6(0.9)/6(0.7)/6(0.7) & 6(0.6) & 6(1) & 6(6.5)/6(7.2) & 6(1.3)/6(2.2) & 6(0.7) & 6(0.8) \\ 
   & p=30 & 6(1.1)/6(0.9)/6(2.5) & 6(0.7) & 6(3.7) & 6(18.3)/6(19.9) & 6(2.9)/6(2.5) & 6(1.1) & 6(5.7) \\ 
   & p=60 & 6(1.7)/6(1.6)/6(3.3) & - & 6(4.9) & 6(31.8)/6(36.4) & 6(4.2)/6(2.7) & 6(1.8) & 6(7.5) \\ 
   & p=180 & 6(14.9)/6(6.8)/6(11.8) & - & 5.9(19.7) & 6(51.3)/6(76.1) & 6(8.6)/6(4.1) & 6(3.2) & 6(17.5) \\ 
  \midrule\multirow{4}[2]{*}{msnr} & p=14 & 6(3)/6(2.7)/6(1.2) & 6(0.6) & 6(2.4) & 6(6.5)/6(7.2) & 6(1.5)/6(3) & 6(1.3) & 6(2.4) \\ 
   & p=30 & 6(5.1)/6(4)/6(3.5) & 6(0.7) & 6(7) & 6(18.2)/6(19.9) & 6(3.6)/6(5.3) & 6(3.4) & 6(9.8) \\ 
   & p=60 & 6(6.1)/6(4.7)/6(5.1) & - & 6(10.3) & 6(31.8)/6(36.3) & 6(6.5)/6(7.7) & 6(6) & 6(16.8) \\ 
   & p=180 & 5.9(38.2)/5.5(14.8)/5.8(18.2) & - & 4.2(16.8) & 5.8(49.6)/6(75.8) & 6(23.5)/5.9(36.2) & 5.9(31.7) & 6(46.5) \\ 
  \midrule\multirow{4}[2]{*}{lsnr} & p=14 & 5.7(4.9)/5.6(4.6)/5.6(2.7) & 5.2(1.2) & 5.3(4) & 5.8(6.3)/5.8(6.9) & 5.4(3.7)/5.7(5.9) & 5.4(4.7) & 5.7(5.6) \\ 
   & p=30 & 4(7.5)/2.9(4.4)/4.6(6.6) & 4.1(1.7) & 2.5(4.5) & 2.7(8.3)/2.8(9.2) & 4.4(9.7)/3.3(9.4) & 3.4(8.7) & 2.6(7.6) \\ 
   & p=60 & 2.6(7.1)/1.4(2.5)/3.8(9.8) & - & 0.8(1.7) & 0.8(4.4)/0.9(5.7) & 3.7(16)/1.3(7.2) & 1.8(9.1) & 0.9(4.9) \\ 
   & p=180 & 1.2(20.1)/0.3(0.5)/0.7(2.7) & - & 0.1(0.5) & 0.3(4.4)/0.3(4.6) & 2(35.8)/0.3(4.5) & 0.3(4.9) & 0.3(3.5) \\ 
   \bottomrule 
\end{tabular}
}
\end{table}
