# Supplementary material for: On the Use of Information Criteria for Subset Selection in Least Squares Regression
Source: arXiv:1911.10191 source file (2021-03-06)
Supplement: Supplementary file 19 [file Sparse-Ex3_n2000_rho_0.tex]

% latex table generated in R 3.6.2 by xtable 1.8-4 package
% Sat Dec 21 23:35:58 2019
\begin{table}[ht]
\centering
\caption{The performance of BOSS compared to other methods, Sparse-Ex3, $\rho$=0, n=2000} 
\scalebox{0.7}{
\begin{tabular}{|c|c|ccccccc|}
  \toprule 
 \multicolumn{1}{|c}{} &       & BOSS  & BS    & FS    & LASSO & Gamma LASSO & SparseNet & \multicolumn{1}{c|}{rLASSO} \\
 \multicolumn{1}{|c}{} &       & C$_p$-hdf/AICc-hdf/CV & CV    & CV    & AICc/CV & AICc/CV & CV    & \multicolumn{1}{c|}{CV}  \\
 \cmidrule{3-9}\multicolumn{1}{|c}{} &       & \multicolumn{7}{c|}{\% worse than the best possible BOSS}  \\
 \midrule\multirow{4}[2]{*}{hsnr} & p=14 & 6/6/17 & 17 & 17 & 41/41 & 12/15 & 11 & 13 \\ 
   & p=30 & 3/3/22 & 22 & 23 & 72/69 & 20/18 & 13 & 16 \\ 
   & p=60 & 2/2/24 & - & 23 & 97/93 & 29/19 & 14 & 17 \\ 
   & p=180 & 1/1/21 & - & 21 & 132/129 & 53/19 & 13 & 17 \\ 
  \midrule\multirow{4}[2]{*}{msnr} & p=14 & 6/6/17 & 17 & 17 & 41/41 & 14/17 & 11 & 13 \\ 
   & p=30 & 3/3/22 & 22 & 23 & 72/69 & 26/20 & 13 & 17 \\ 
   & p=60 & 2/2/24 & - & 23 & 97/93 & 43/21 & 14 & 18 \\ 
   & p=180 & 1/1/21 & - & 21 & 132/129 & 97/22 & 13 & 17 \\ 
  \midrule\multirow{4}[2]{*}{lsnr} & p=14 & 9/9/17 & 17 & 17 & 42/41 & 21/20 & 12 & 13 \\ 
   & p=30 & 5/5/22 & 22 & 23 & 72/69 & 45/25 & 13 & 16 \\ 
   & p=60 & 5/4/24 & - & 23 & 97/93 & 82/26 & 15 & 18 \\ 
   & p=180 & 5/4/21 & - & 21 & 132/129 & 192/26 & 13 & 17 \\ 
   \midrule 
 \multicolumn{1}{|c}{} &       & \multicolumn{7}{c|}{Relative efficiency} \\
\midrule\multirow{4}[2]{*}{hsnr} & p=14 & 1/1/0.91 & 0.91 & 0.91 & 0.76/0.76 & 0.95/0.93 & 0.96 & 0.94 \\ 
   & p=30 & 1/1/0.84 & 0.84 & 0.84 & 0.6/0.61 & 0.86/0.87 & 0.91 & 0.88 \\ 
   & p=60 & 1/1/0.83 & - & 0.83 & 0.52/0.53 & 0.79/0.86 & 0.89 & 0.87 \\ 
   & p=180 & 1/1/0.83 & - & 0.84 & 0.44/0.44 & 0.66/0.85 & 0.89 & 0.86 \\ 
  \midrule\multirow{4}[2]{*}{msnr} & p=14 & 1/1/0.91 & 0.91 & 0.91 & 0.75/0.75 & 0.93/0.91 & 0.96 & 0.94 \\ 
   & p=30 & 1/1/0.84 & 0.84 & 0.84 & 0.6/0.61 & 0.81/0.86 & 0.91 & 0.88 \\ 
   & p=60 & 1/1/0.83 & - & 0.83 & 0.52/0.53 & 0.71/0.84 & 0.89 & 0.87 \\ 
   & p=180 & 1/1/0.83 & - & 0.84 & 0.44/0.44 & 0.51/0.83 & 0.89 & 0.86 \\ 
  \midrule\multirow{4}[2]{*}{lsnr} & p=14 & 1/1/0.93 & 0.93 & 0.93 & 0.77/0.77 & 0.9/0.9 & 0.97 & 0.96 \\ 
   & p=30 & 0.99/1/0.86 & 0.86 & 0.85 & 0.61/0.62 & 0.72/0.84 & 0.93 & 0.9 \\ 
   & p=60 & 1/1/0.84 & - & 0.85 & 0.53/0.54 & 0.57/0.83 & 0.91 & 0.89 \\ 
   & p=180 & 0.99/1/0.86 & - & 0.86 & 0.45/0.46 & 0.36/0.82 & 0.92 & 0.89 \\ 
   \midrule 
 \multicolumn{1}{|c}{} &       & \multicolumn{7}{c|}{Sparsistency (number of extra variables)} \\
\midrule\multirow{4}[2]{*}{hsnr} & p=14 & 6(0.3)/6(0.3)/6(0.6) & 6(0.6) & 6(0.6) & 6(3.8)/6(4.5) & 6(0.9)/6(1.3) & 6(0.6) & 6(0.5) \\ 
   & p=30 & 6(0.1)/6(0.1)/6(0.6) & 6(0.6) & 6(0.6) & 6(8.3)/6(8.5) & 6(2)/6(1.8) & 6(0.9) & 6(0.5) \\ 
   & p=60 & 6(0)/6(0)/6(0.5) & - & 6(0.5) & 6(13)/6(12.2) & 6(3.9)/6(2.1) & 6(1.5) & 6(0.5) \\ 
   & p=180 & 6(0)/6(0)/6(0.3) & - & 6(0.3) & 6(21.7)/6(19.1) & 6(10.3)/6(2.4) & 6(2.1) & 6(0.4) \\ 
  \midrule\multirow{4}[2]{*}{msnr} & p=14 & 6(0.3)/6(0.3)/6(0.6) & 6(0.6) & 6(0.6) & 6(3.9)/6(4.5) & 6(1)/6(1.3) & 6(0.6) & 6(0.5) \\ 
   & p=30 & 6(0.1)/6(0.1)/6(0.6) & 6(0.6) & 6(0.6) & 6(8.3)/6(8.6) & 6(2.2)/6(1.8) & 6(0.9) & 6(0.5) \\ 
   & p=60 & 6(0)/6(0)/6(0.5) & - & 6(0.5) & 6(13)/6(12.2) & 6(4.8)/6(1.8) & 6(1.4) & 6(0.6) \\ 
   & p=180 & 6(0)/6(0)/6(0.3) & - & 6(0.3) & 6(21.6)/6(19.1) & 6(15.6)/6(1.8) & 6(1.8) & 6(0.4) \\ 
  \midrule\multirow{4}[2]{*}{lsnr} & p=14 & 6(0.4)/6(0.4)/6(0.6) & 6(0.6) & 6(0.6) & 6(3.9)/6(4.5) & 6(1.1)/6(1.4) & 6(0.5) & 6(0.5) \\ 
   & p=30 & 6(0.1)/6(0.1)/6(0.6) & 6(0.6) & 6(0.6) & 6(8.3)/6(8.5) & 6(3)/6(1.6) & 6(0.7) & 6(0.5) \\ 
   & p=60 & 6(0.1)/6(0.1)/6(0.5) & - & 6(0.5) & 6(13.2)/6(12.2) & 6(6.8)/6(1.5) & 6(1) & 6(0.6) \\ 
   & p=180 & 6(0.1)/6(0)/6(0.3) & - & 6(0.3) & 6(21.9)/6(19.1) & 6(23.7)/6(1) & 6(1) & 6(0.5) \\ 
   \bottomrule 
\end{tabular}
}
\end{table}
