# Supplementary material for: On the Use of Information Criteria for Subset Selection in Least Squares Regression
Source: arXiv:1911.10191 source file (2021-03-06)
Supplement: Supplementary file 20 [file Sparse-Ex3_n2000_rho_05.tex]

% latex table generated in R 3.6.2 by xtable 1.8-4 package
% Sat Dec 21 23:36:05 2019
\begin{table}[ht]
\centering
\caption{The performance of BOSS compared to other methods, Sparse-Ex3, $\rho$=0.5, n=2000} 
\scalebox{0.7}{
\begin{tabular}{|c|c|ccccccc|}
  \toprule 
 \multicolumn{1}{|c}{} &       & BOSS  & BS    & FS    & LASSO & Gamma LASSO & SparseNet & \multicolumn{1}{c|}{rLASSO} \\
 \multicolumn{1}{|c}{} &       & C$_p$-hdf/AICc-hdf/CV & CV    & CV    & AICc/CV & AICc/CV & CV    & \multicolumn{1}{c|}{CV}  \\
 \cmidrule{3-9}\multicolumn{1}{|c}{} &       & \multicolumn{7}{c|}{\% worse than the best possible BOSS}  \\
 \midrule\multirow{4}[2]{*}{hsnr} & p=14 & 7/6/18 & 19 & 19 & 43/42 & 13/16 & 13 & 15 \\ 
   & p=30 & 3/3/22 & 22 & 21 & 73/71 & 21/18 & 14 & 17 \\ 
   & p=60 & 1/1/21 & - & 20 & 96/92 & 29/18 & 13 & 17 \\ 
   & p=180 & 1/1/22 & - & 22 & 130/126 & 53/20 & 14 & 18 \\ 
  \midrule\multirow{4}[2]{*}{msnr} & p=14 & 7/6/18 & 19 & 19 & 44/43 & 16/18 & 13 & 16 \\ 
   & p=30 & 3/3/22 & 22 & 21 & 73/71 & 28/20 & 14 & 17 \\ 
   & p=60 & 1/1/21 & - & 20 & 96/92 & 43/21 & 13 & 17 \\ 
   & p=180 & 1/1/22 & - & 22 & 130/126 & 98/22 & 13 & 18 \\ 
  \midrule\multirow{4}[2]{*}{lsnr} & p=14 & 9/9/18 & 19 & 19 & 44/43 & 22/22 & 13 & 16 \\ 
   & p=30 & 5/5/22 & 21 & 21 & 73/71 & 47/25 & 14 & 17 \\ 
   & p=60 & 4/4/21 & - & 20 & 96/92 & 80/26 & 14 & 17 \\ 
   & p=180 & 5/5/22 & - & 22 & 129/126 & 192/27 & 13 & 19 \\ 
   \midrule 
 \multicolumn{1}{|c}{} &       & \multicolumn{7}{c|}{Relative efficiency} \\
\midrule\multirow{4}[2]{*}{hsnr} & p=14 & 1/1/0.9 & 0.9 & 0.9 & 0.75/0.75 & 0.94/0.92 & 0.95 & 0.92 \\ 
   & p=30 & 1/1/0.85 & 0.85 & 0.85 & 0.59/0.6 & 0.85/0.87 & 0.91 & 0.88 \\ 
   & p=60 & 1/1/0.84 & - & 0.84 & 0.52/0.53 & 0.79/0.86 & 0.89 & 0.86 \\ 
   & p=180 & 1/1/0.83 & - & 0.83 & 0.44/0.45 & 0.66/0.84 & 0.89 & 0.86 \\ 
  \midrule\multirow{4}[2]{*}{msnr} & p=14 & 1/1/0.9 & 0.9 & 0.9 & 0.74/0.75 & 0.92/0.9 & 0.94 & 0.92 \\ 
   & p=30 & 1/1/0.85 & 0.85 & 0.85 & 0.59/0.6 & 0.8/0.85 & 0.9 & 0.88 \\ 
   & p=60 & 1/1/0.84 & - & 0.84 & 0.52/0.53 & 0.71/0.84 & 0.9 & 0.87 \\ 
   & p=180 & 1/1/0.83 & - & 0.83 & 0.44/0.45 & 0.51/0.83 & 0.89 & 0.86 \\ 
  \midrule\multirow{4}[2]{*}{lsnr} & p=14 & 1/1/0.92 & 0.92 & 0.92 & 0.75/0.76 & 0.89/0.89 & 0.96 & 0.94 \\ 
   & p=30 & 1/1/0.86 & 0.86 & 0.86 & 0.61/0.61 & 0.71/0.84 & 0.92 & 0.9 \\ 
   & p=60 & 1/1/0.86 & - & 0.86 & 0.53/0.54 & 0.58/0.83 & 0.91 & 0.88 \\ 
   & p=180 & 1/1/0.86 & - & 0.86 & 0.46/0.46 & 0.36/0.82 & 0.93 & 0.88 \\ 
   \midrule 
 \multicolumn{1}{|c}{} &       & \multicolumn{7}{c|}{Sparsistency (number of extra variables)} \\
\midrule\multirow{4}[2]{*}{hsnr} & p=14 & 6(0.3)/6(0.3)/6(0.6) & 6(0.6) & 6(0.6) & 6(3.9)/6(4.4) & 6(0.9)/6(1.3) & 6(0.6) & 6(0.6) \\ 
   & p=30 & 6(0.1)/6(0.1)/6(0.6) & 6(0.6) & 6(0.6) & 6(8.4)/6(8.6) & 6(2.1)/6(1.7) & 6(1) & 6(0.6) \\ 
   & p=60 & 6(0)/6(0)/6(0.5) & - & 6(0.5) & 6(13.2)/6(12.3) & 6(3.9)/6(2.1) & 6(1.6) & 6(0.6) \\ 
   & p=180 & 6(0)/6(0)/6(0.4) & - & 6(0.4) & 6(21.5)/6(18.7) & 6(10.4)/6(2.6) & 6(2.3) & 6(0.6) \\ 
  \midrule\multirow{4}[2]{*}{msnr} & p=14 & 6(0.3)/6(0.3)/6(0.6) & 6(0.6) & 6(0.6) & 6(3.9)/6(4.5) & 6(1)/6(1.4) & 6(0.6) & 6(0.6) \\ 
   & p=30 & 6(0.1)/6(0.1)/6(0.6) & 6(0.6) & 6(0.6) & 6(8.3)/6(8.6) & 6(2.4)/6(1.6) & 6(0.9) & 6(0.6) \\ 
   & p=60 & 6(0)/6(0)/6(0.5) & - & 6(0.5) & 6(13)/6(12.3) & 6(4.7)/6(1.8) & 6(1.4) & 6(0.6) \\ 
   & p=180 & 6(0)/6(0)/6(0.4) & - & 6(0.4) & 6(21.5)/6(18.7) & 6(15.7)/6(1.9) & 6(2.1) & 6(0.5) \\ 
  \midrule\multirow{4}[2]{*}{lsnr} & p=14 & 6(0.4)/6(0.4)/6(0.6) & 6(0.6) & 6(0.6) & 6(3.9)/6(4.5) & 6(1.1)/6(1.4) & 6(0.5) & 6(0.6) \\ 
   & p=30 & 6(0.1)/6(0.1)/6(0.6) & 6(0.6) & 6(0.6) & 6(8.3)/6(8.6) & 6(3)/6(1.4) & 6(0.7) & 6(0.6) \\ 
   & p=60 & 6(0.1)/6(0.1)/6(0.5) & - & 6(0.5) & 6(13.1)/6(12.2) & 6(6.5)/6(1.5) & 6(1) & 6(0.6) \\ 
   & p=180 & 6(0.1)/6(0.1)/6(0.4) & - & 6(0.4) & 6(21.2)/6(18.7) & 6(23.5)/6(1.2) & 6(0.9) & 6(0.5) \\ 
   \bottomrule 
\end{tabular}
}
\end{table}
