# Supplementary material for: On the Use of Information Criteria for Subset Selection in Least Squares Regression
Source: arXiv:1911.10191 source file (2021-03-06)
Supplement: Supplementary file 21 [file Sparse-Ex3_n2000_rho_09.tex]

% latex table generated in R 3.6.2 by xtable 1.8-4 package
% Sat Dec 21 23:36:11 2019
\begin{table}[ht]
\centering
\caption{The performance of BOSS compared to other methods, Sparse-Ex3, $\rho$=0.9, n=2000} 
\scalebox{0.7}{
\begin{tabular}{|c|c|ccccccc|}
  \toprule 
 \multicolumn{1}{|c}{} &       & BOSS  & BS    & FS    & LASSO & Gamma LASSO & SparseNet & \multicolumn{1}{c|}{rLASSO} \\
 \multicolumn{1}{|c}{} &       & C$_p$-hdf/AICc-hdf/CV & CV    & CV    & AICc/CV & AICc/CV & CV    & \multicolumn{1}{c|}{CV}  \\
 \cmidrule{3-9}\multicolumn{1}{|c}{} &       & \multicolumn{7}{c|}{\% worse than the best possible BOSS}  \\
 \midrule\multirow{4}[2]{*}{hsnr} & p=14 & 6/6/19 & 19 & 19 & 40/39 & 12/14 & 13 & 15 \\ 
   & p=30 & 2/2/21 & 21 & 22 & 74/72 & 20/18 & 13 & 17 \\ 
   & p=60 & 1/1/22 & - & 22 & 101/97 & 29/19 & 14 & 19 \\ 
   & p=180 & 1/1/21 & - & 22 & 135/131 & 52/18 & 14 & 21 \\ 
  \midrule\multirow{4}[2]{*}{msnr} & p=14 & 6/6/19 & 19 & 19 & 42/40 & 18/18 & 14 & 15 \\ 
   & p=30 & 2/2/21 & 21 & 22 & 74/72 & 27/20 & 14 & 17 \\ 
   & p=60 & 1/1/22 & - & 22 & 101/97 & 43/21 & 14 & 19 \\ 
   & p=180 & 1/1/21 & - & 22 & 135/132 & 96/21 & 13 & 21 \\ 
  \midrule\multirow{4}[2]{*}{lsnr} & p=14 & 9/9/19 & 19 & 19 & 27/26 & 17/18 & 6 & 14 \\ 
   & p=30 & 5/5/21 & 20 & 21 & 53/51 & 34/23 & 3 & 14 \\ 
   & p=60 & 4/4/20 & - & 20 & 75/71 & 62/22 & 1 & 12 \\ 
   & p=180 & 4/4/17 & - & 17 & 92/89 & 145/23 & -5 & 11 \\ 
   \midrule 
 \multicolumn{1}{|c}{} &       & \multicolumn{7}{c|}{Relative efficiency} \\
\midrule\multirow{4}[2]{*}{hsnr} & p=14 & 1/1/0.89 & 0.89 & 0.89 & 0.76/0.76 & 0.95/0.93 & 0.94 & 0.92 \\ 
   & p=30 & 1/1/0.84 & 0.85 & 0.84 & 0.59/0.6 & 0.85/0.87 & 0.9 & 0.87 \\ 
   & p=60 & 1/1/0.83 & - & 0.83 & 0.5/0.51 & 0.79/0.85 & 0.89 & 0.85 \\ 
   & p=180 & 1/1/0.84 & - & 0.83 & 0.43/0.44 & 0.67/0.86 & 0.89 & 0.84 \\ 
  \midrule\multirow{4}[2]{*}{msnr} & p=14 & 1/1/0.89 & 0.89 & 0.89 & 0.75/0.76 & 0.9/0.9 & 0.93 & 0.92 \\ 
   & p=30 & 1/1/0.84 & 0.85 & 0.84 & 0.59/0.6 & 0.81/0.85 & 0.9 & 0.87 \\ 
   & p=60 & 1/1/0.83 & - & 0.83 & 0.5/0.51 & 0.71/0.84 & 0.89 & 0.85 \\ 
   & p=180 & 1/1/0.84 & - & 0.83 & 0.43/0.44 & 0.52/0.83 & 0.9 & 0.84 \\ 
  \midrule\multirow{4}[2]{*}{lsnr} & p=14 & 0.97/0.97/0.89 & 0.89 & 0.89 & 0.83/0.84 & 0.91/0.89 & 1 & 0.93 \\ 
   & p=30 & 0.98/0.98/0.85 & 0.86 & 0.85 & 0.67/0.68 & 0.77/0.83 & 1 & 0.9 \\ 
   & p=60 & 0.97/0.97/0.84 & - & 0.84 & 0.58/0.59 & 0.62/0.82 & 1 & 0.9 \\ 
   & p=180 & 0.91/0.91/0.81 & - & 0.81 & 0.49/0.5 & 0.39/0.77 & 1 & 0.85 \\ 
   \midrule 
 \multicolumn{1}{|c}{} &       & \multicolumn{7}{c|}{Sparsistency (number of extra variables)} \\
\midrule\multirow{4}[2]{*}{hsnr} & p=14 & 6(0.3)/6(0.3)/6(0.7) & 6(0.6) & 6(0.6) & 6(4.1)/6(4.6) & 6(0.8)/6(1) & 6(0.7) & 6(0.6) \\ 
   & p=30 & 6(0)/6(0)/6(0.6) & 6(0.6) & 6(0.6) & 6(9.2)/6(9.5) & 6(2)/6(1.8) & 6(1) & 6(0.7) \\ 
   & p=60 & 6(0)/6(0)/6(0.5) & - & 6(0.5) & 6(14)/6(13.3) & 6(3.7)/6(2.1) & 6(1.5) & 6(0.8) \\ 
   & p=180 & 6(0)/6(0)/6(0.4) & - & 6(0.4) & 6(23.2)/6(20.6) & 6(10.1)/6(2.4) & 6(2.2) & 6(0.7) \\ 
  \midrule\multirow{4}[2]{*}{msnr} & p=14 & 6(0.3)/6(0.3)/6(0.7) & 6(0.6) & 6(0.6) & 6(4.2)/6(4.6) & 6(1.1)/6(1.3) & 6(0.7) & 6(0.6) \\ 
   & p=30 & 6(0)/6(0)/6(0.6) & 6(0.6) & 6(0.6) & 6(9.2)/6(9.5) & 6(2.3)/6(1.7) & 6(1) & 6(0.7) \\ 
   & p=60 & 6(0)/6(0)/6(0.5) & - & 6(0.5) & 6(14.1)/6(13.3) & 6(4.7)/6(1.8) & 6(1.4) & 6(0.7) \\ 
   & p=180 & 6(0)/6(0)/6(0.4) & - & 6(0.4) & 6(23.2)/6(20.5) & 6(15.3)/6(1.9) & 6(1.9) & 6(0.7) \\ 
  \midrule\multirow{4}[2]{*}{lsnr} & p=14 & 5.8(0.4)/5.8(0.4)/5.9(1.4) & 5.9(1.5) & 5.9(1.5) & 6(4.2)/6(4.6) & 5.9(1.2)/5.9(2.1) & 6(0.8) & 6(1.6) \\ 
   & p=30 & 5.8(0.3)/5.8(0.3)/5.8(1.1) & 5.8(1.1) & 5.8(1.1) & 6(9.2)/6(9.5) & 5.8(2.8)/5.9(3) & 6(0.8) & 6(1.6) \\ 
   & p=60 & 5.8(0.3)/5.8(0.3)/5.8(0.8) & - & 5.8(0.8) & 6(14)/6(13.3) & 5.8(6.3)/5.8(2.3) & 6(1.1) & 6(1.4) \\ 
   & p=180 & 5.7(0.3)/5.7(0.3)/5.7(0.7) & - & 5.7(0.7) & 6(23)/6(20.6) & 5.7(23.2)/5.7(2.6) & 6(1) & 5.9(1.7) \\ 
   \bottomrule 
\end{tabular}
}
\end{table}
