# Supplementary material for: On the Use of Information Criteria for Subset Selection in Least Squares Regression
Source: arXiv:1911.10191 source file (2021-03-06)
Supplement: Supplementary file 22 [file Sparse-Ex3_n200_rho_0.tex]

% latex table generated in R 3.6.2 by xtable 1.8-4 package
% Sat Dec 21 23:35:52 2019
\begin{table}[ht]
\centering
\caption{The performance of BOSS compared to other methods, Sparse-Ex3, $\rho$=0, n=200} 
\scalebox{0.7}{
\begin{tabular}{|c|c|ccccccc|}
  \toprule 
 \multicolumn{1}{|c}{} &       & BOSS  & BS    & FS    & LASSO & Gamma LASSO & SparseNet & \multicolumn{1}{c|}{rLASSO} \\
 \multicolumn{1}{|c}{} &       & C$_p$-hdf/AICc-hdf/CV & CV    & CV    & AICc/CV & AICc/CV & CV    & \multicolumn{1}{c|}{CV}  \\
 \cmidrule{3-9}\multicolumn{1}{|c}{} &       & \multicolumn{7}{c|}{\% worse than the best possible BOSS}  \\
 \midrule\multirow{4}[2]{*}{hsnr} & p=14 & 8/6/20 & 21 & 20 & 44/43 & 17/20 & 15 & 16 \\ 
   & p=30 & 5/3/24 & 25 & 25 & 69/67 & 32/23 & 15 & 19 \\ 
   & p=60 & 4/2/21 & - & 23 & 97/96 & 52/24 & 16 & 19 \\ 
   & p=180 & 34/1/19 & - & 21 & 133/133 & 137/28 & 19 & 16 \\ 
  \midrule\multirow{4}[2]{*}{msnr} & p=14 & 17/14/20 & 21 & 20 & 44/43 & 24/24 & 16 & 17 \\ 
   & p=30 & 18/13/24 & 25 & 25 & 69/67 & 48/27 & 16 & 21 \\ 
   & p=60 & 14/9/21 & - & 23 & 97/95 & 84/29 & 16 & 22 \\ 
   & p=180 & 50/11/20 & - & 22 & 132/133 & 224/33 & 19 & 29 \\ 
  \midrule\multirow{4}[2]{*}{lsnr} & p=14 & 22/23/26 & 26 & 26 & 8/8 & 13/15 & 17 & 15 \\ 
   & p=30 & 29/32/26 & 26 & 25 & 1/1 & 14/8 & 8 & 6 \\ 
   & p=60 & 27/29/22 & - & 22 & 0/1 & 24/6 & 6 & 6 \\ 
   & p=180 & 30/16/14 & - & 14 & -2/1 & 84/4 & 3 & 4 \\ 
   \midrule 
 \multicolumn{1}{|c}{} &       & \multicolumn{7}{c|}{Relative efficiency} \\
\midrule\multirow{4}[2]{*}{hsnr} & p=14 & 0.98/1/0.89 & 0.88 & 0.89 & 0.74/0.75 & 0.91/0.88 & 0.93 & 0.91 \\ 
   & p=30 & 0.98/1/0.83 & 0.82 & 0.82 & 0.61/0.61 & 0.78/0.84 & 0.89 & 0.86 \\ 
   & p=60 & 0.99/1/0.85 & - & 0.83 & 0.52/0.52 & 0.67/0.83 & 0.88 & 0.86 \\ 
   & p=180 & 0.75/1/0.85 & - & 0.84 & 0.43/0.43 & 0.43/0.79 & 0.85 & 0.87 \\ 
  \midrule\multirow{4}[2]{*}{msnr} & p=14 & 0.98/1/0.95 & 0.95 & 0.96 & 0.8/0.8 & 0.92/0.92 & 0.99 & 0.98 \\ 
   & p=30 & 0.96/1/0.92 & 0.91 & 0.91 & 0.67/0.68 & 0.76/0.89 & 0.98 & 0.94 \\ 
   & p=60 & 0.96/1/0.9 & - & 0.89 & 0.56/0.56 & 0.59/0.85 & 0.94 & 0.9 \\ 
   & p=180 & 0.74/1/0.92 & - & 0.91 & 0.48/0.47 & 0.34/0.83 & 0.93 & 0.86 \\ 
  \midrule\multirow{4}[2]{*}{lsnr} & p=14 & 0.89/0.88/0.86 & 0.86 & 0.86 & 1/1 & 0.95/0.94 & 0.92 & 0.94 \\ 
   & p=30 & 0.78/0.76/0.8 & 0.8 & 0.81 & 1/1 & 0.88/0.93 & 0.93 & 0.95 \\ 
   & p=60 & 0.79/0.78/0.82 & - & 0.82 & 1/1 & 0.81/0.95 & 0.94 & 0.95 \\ 
   & p=180 & 0.76/0.85/0.86 & - & 0.86 & 1/0.98 & 0.53/0.94 & 0.95 & 0.95 \\ 
   \midrule 
 \multicolumn{1}{|c}{} &       & \multicolumn{7}{c|}{Sparsistency (number of extra variables)} \\
\midrule\multirow{4}[2]{*}{hsnr} & p=14 & 6(0.3)/6(0.2)/6(0.6) & 6(0.7) & 6(0.6) & 6(3.7)/6(4.5) & 6(1)/6(1.3) & 6(0.6) & 6(0.6) \\ 
   & p=30 & 6(0.1)/6(0)/6(0.6) & 6(0.7) & 6(0.7) & 6(7.4)/6(8.2) & 6(2.4)/6(1.7) & 6(1) & 6(0.7) \\ 
   & p=60 & 6(0.1)/6(0)/6(0.5) & - & 6(0.5) & 6(11.3)/6(13.1) & 6(4.8)/6(1.7) & 6(1.5) & 6(0.7) \\ 
   & p=180 & 6(8.8)/6(0)/6(0.4) & - & 6(0.4) & 6(16.5)/6(22.7) & 6(18)/6(2.5) & 6(2.7) & 6(0.6) \\ 
  \midrule\multirow{4}[2]{*}{msnr} & p=14 & 6(0.8)/6(0.6)/6(0.6) & 6(0.7) & 6(0.6) & 6(3.7)/6(4.5) & 6(1.2)/6(1.4) & 6(0.6) & 6(0.6) \\ 
   & p=30 & 6(0.5)/6(0.3)/6(0.6) & 6(0.7) & 6(0.7) & 6(7.4)/6(8.2) & 6(2.9)/6(1.6) & 6(0.8) & 6(0.8) \\ 
   & p=60 & 6(0.3)/6(0.1)/6(0.5) & - & 6(0.5) & 6(11.4)/6(13.1) & 6(6.4)/6(1.5) & 6(1.1) & 6(0.9) \\ 
   & p=180 & 6(9.4)/6(0.1)/6(0.4) & - & 6(0.4) & 6(16.5)/6(22.8) & 6(27.4)/6(2) & 6(1.7) & 6(1.1) \\ 
  \midrule\multirow{4}[2]{*}{lsnr} & p=14 & 5.4(4.4)/5.2(4.1)/4.7(1.8) & 4.7(1.7) & 4.7(1.7) & 5.6(3.3)/5.6(4) & 5.1(1.5)/5.3(3) & 5.1(2.8) & 5(2.1) \\ 
   & p=30 & 4(4.4)/3.1(1.9)/3.7(2.1) & 3.6(2.1) & 3.7(2) & 5.3(6.4)/5.4(7) & 4.9(3.8)/4.8(4.9) & 4.8(5.3) & 4.6(3.6) \\ 
   & p=60 & 2.2(1.8)/1.2(0.2)/2.6(1.4) & - & 2.6(1.3) & 4.6(8.6)/4.6(9.6) & 4.9(8.5)/4.1(6.6) & 4.2(7.2) & 3.9(5.5) \\ 
   & p=180 & 1.6(14.2)/0.5(0.1)/1.3(0.6) & - & 1.3(0.6) & 3.4(10.4)/3.5(13.1) & 4.6(36.9)/3(9) & 3.2(10.5) & 2.9(7.7) \\ 
   \bottomrule 
\end{tabular}
}
\end{table}
