# Supplementary material for: On the Use of Information Criteria for Subset Selection in Least Squares Regression
Source: arXiv:1911.10191 source file (2021-03-06)
Supplement: Supplementary file 23 [file Sparse-Ex3_n200_rho_05.tex]

% latex table generated in R 3.6.2 by xtable 1.8-4 package
% Sat Dec 21 23:35:59 2019
\begin{table}[ht]
\centering
\caption{The performance of BOSS compared to other methods, Sparse-Ex3, $\rho$=0.5, n=200} 
\scalebox{0.7}{
\begin{tabular}{|c|c|ccccccc|}
  \toprule 
 \multicolumn{1}{|c}{} &       & BOSS  & BS    & FS    & LASSO & Gamma LASSO & SparseNet & \multicolumn{1}{c|}{rLASSO} \\
 \multicolumn{1}{|c}{} &       & C$_p$-hdf/AICc-hdf/CV & CV    & CV    & AICc/CV & AICc/CV & CV    & \multicolumn{1}{c|}{CV}  \\
 \cmidrule{3-9}\multicolumn{1}{|c}{} &       & \multicolumn{7}{c|}{\% worse than the best possible BOSS}  \\
 \midrule\multirow{4}[2]{*}{hsnr} & p=14 & 7/6/18 & 19 & 18 & 40/39 & 15/18 & 14 & 15 \\ 
   & p=30 & 5/2/22 & 24 & 22 & 70/68 & 30/21 & 14 & 19 \\ 
   & p=60 & 3/1/22 & - & 23 & 93/92 & 51/22 & 16 & 19 \\ 
   & p=180 & 35/1/18 & - & 21 & 135/135 & 134/26 & 17 & 20 \\ 
  \midrule\multirow{4}[2]{*}{msnr} & p=14 & 15/13/18 & 19 & 18 & 40/39 & 20/21 & 15 & 17 \\ 
   & p=30 & 14/10/22 & 25 & 23 & 69/68 & 45/25 & 15 & 22 \\ 
   & p=60 & 13/9/23 & - & 24 & 91/89 & 78/26 & 15 & 27 \\ 
   & p=180 & 48/11/20 & - & 23 & 132/133 & 218/31 & 18 & 43 \\ 
  \midrule\multirow{4}[2]{*}{lsnr} & p=14 & 19/21/24 & 24 & 24 & 5/4 & 11/11 & 13 & 10 \\ 
   & p=30 & 28/30/25 & 25 & 25 & 0/0 & 12/6 & 7 & 6 \\ 
   & p=60 & 23/25/21 & - & 21 & -3/-3 & 22/3 & 3 & 2 \\ 
   & p=180 & 27/11/13 & - & 13 & -3/-1 & 83/3 & 3 & 3 \\ 
   \midrule 
 \multicolumn{1}{|c}{} &       & \multicolumn{7}{c|}{Relative efficiency} \\
\midrule\multirow{4}[2]{*}{hsnr} & p=14 & 0.98/1/0.9 & 0.89 & 0.9 & 0.75/0.76 & 0.92/0.9 & 0.92 & 0.92 \\ 
   & p=30 & 0.98/1/0.84 & 0.82 & 0.84 & 0.6/0.61 & 0.79/0.85 & 0.9 & 0.86 \\ 
   & p=60 & 0.98/1/0.83 & - & 0.83 & 0.53/0.53 & 0.67/0.83 & 0.88 & 0.85 \\ 
   & p=180 & 0.75/1/0.85 & - & 0.84 & 0.43/0.43 & 0.43/0.8 & 0.86 & 0.84 \\ 
  \midrule\multirow{4}[2]{*}{msnr} & p=14 & 0.98/1/0.95 & 0.95 & 0.95 & 0.8/0.81 & 0.93/0.93 & 0.98 & 0.96 \\ 
   & p=30 & 0.97/1/0.9 & 0.88 & 0.89 & 0.65/0.66 & 0.76/0.88 & 0.96 & 0.9 \\ 
   & p=60 & 0.97/1/0.88 & - & 0.88 & 0.57/0.57 & 0.61/0.86 & 0.94 & 0.86 \\ 
   & p=180 & 0.75/1/0.92 & - & 0.9 & 0.48/0.47 & 0.35/0.84 & 0.94 & 0.77 \\ 
  \midrule\multirow{4}[2]{*}{lsnr} & p=14 & 0.88/0.86/0.84 & 0.84 & 0.84 & 0.99/1 & 0.94/0.94 & 0.93 & 0.95 \\ 
   & p=30 & 0.78/0.77/0.8 & 0.8 & 0.8 & 1/1 & 0.9/0.94 & 0.93 & 0.95 \\ 
   & p=60 & 0.79/0.78/0.8 & - & 0.8 & 1/1 & 0.79/0.94 & 0.94 & 0.95 \\ 
   & p=180 & 0.76/0.87/0.86 & - & 0.86 & 1/0.98 & 0.53/0.94 & 0.94 & 0.94 \\ 
   \midrule 
 \multicolumn{1}{|c}{} &       & \multicolumn{7}{c|}{Sparsistency (number of extra variables)} \\
\midrule\multirow{4}[2]{*}{hsnr} & p=14 & 6(0.4)/6(0.2)/6(0.6) & 6(0.7) & 6(0.6) & 6(3.7)/6(4.5) & 6(0.9)/6(1.3) & 6(0.7) & 6(0.6) \\ 
   & p=30 & 6(0.2)/6(0)/6(0.6) & 6(0.7) & 6(0.6) & 6(7.9)/6(9) & 6(2.4)/6(1.5) & 6(1.1) & 6(0.9) \\ 
   & p=60 & 6(0.1)/6(0)/6(0.5) & - & 6(0.5) & 6(11.5)/6(13.3) & 6(4.9)/6(1.6) & 6(1.6) & 6(0.8) \\ 
   & p=180 & 6(9.6)/6(0)/6(0.3) & - & 6(0.4) & 6(16.6)/6(23.8) & 6(18.1)/6(2.1) & 6(2.4) & 6(0.8) \\ 
  \midrule\multirow{4}[2]{*}{msnr} & p=14 & 6(0.7)/6(0.6)/6(0.6) & 6(0.7) & 6(0.6) & 6(3.7)/6(4.5) & 6(1)/6(1.3) & 6(0.6) & 6(0.8) \\ 
   & p=30 & 6(0.4)/6(0.2)/6(0.7) & 6(0.8) & 6(0.7) & 6(8)/6(9) & 6(2.9)/6(1.5) & 6(0.8) & 6(1) \\ 
   & p=60 & 6(0.3)/6(0.2)/6(0.6) & - & 6(0.6) & 6(11.5)/6(13.3) & 6(6.1)/6(1.5) & 6(1.1) & 6(1.3) \\ 
   & p=180 & 6(10)/6(0.1)/6(0.4) & - & 6(0.5) & 6(17)/6(23.8) & 6(27.9)/6(1.8) & 6(1.7) & 6(1.8) \\ 
  \midrule\multirow{4}[2]{*}{lsnr} & p=14 & 5.3(4.3)/5.2(4)/4.6(2.1) & 4.6(2) & 4.6(2) & 5.5(3.4)/5.6(4) & 4.9(1.4)/5.2(3) & 5.2(2.6) & 5.1(2.4) \\ 
   & p=30 & 3.8(4.3)/2.9(2)/3.6(2.4) & 3.4(2.1) & 3.5(2.3) & 5.1(6.9)/5.2(7.5) & 4.6(3.9)/4.6(5.3) & 4.7(5.3) & 4.5(4.2) \\ 
   & p=60 & 2.1(1.7)/1.3(0.4)/2.3(1.5) & - & 2.3(1.4) & 4.4(8.6)/4.5(9.7) & 4.4(8.3)/3.9(6.7) & 4(7.5) & 3.8(5.8) \\ 
   & p=180 & 1.4(15.1)/0.3(0.1)/1(0.7) & - & 1(0.7) & 3(9.7)/3(12.5) & 4.3(37.2)/2.5(8.3) & 2.6(9.3) & 2.4(7.7) \\ 
   \bottomrule 
\end{tabular}
}
\end{table}
