# Supplementary material for: On the Use of Information Criteria for Subset Selection in Least Squares Regression
Source: arXiv:1911.10191 source file (2021-03-06)
Supplement: Supplementary file 24 [file Sparse-Ex3_n200_rho_09.tex]

% latex table generated in R 3.6.2 by xtable 1.8-4 package
% Sat Dec 21 23:36:06 2019
\begin{table}[ht]
\centering
\caption{The performance of BOSS compared to other methods, Sparse-Ex3, $\rho$=0.9, n=200} 
\scalebox{0.7}{
\begin{tabular}{|c|c|ccccccc|}
  \toprule 
 \multicolumn{1}{|c}{} &       & BOSS  & BS    & FS    & LASSO & Gamma LASSO & SparseNet & \multicolumn{1}{c|}{rLASSO} \\
 \multicolumn{1}{|c}{} &       & C$_p$-hdf/AICc-hdf/CV & CV    & CV    & AICc/CV & AICc/CV & CV    & \multicolumn{1}{c|}{CV}  \\
 \cmidrule{3-9}\multicolumn{1}{|c}{} &       & \multicolumn{7}{c|}{\% worse than the best possible BOSS}  \\
 \midrule\multirow{4}[2]{*}{hsnr} & p=14 & 7/6/24 & 13 & 24 & 33/33 & 14/16 & 12 & 16 \\ 
   & p=30 & 7/5/41 & 17 & 41 & 66/64 & 26/29 & 12 & 23 \\ 
   & p=60 & 6/4/43 & - & 43 & 84/83 & 44/38 & 13 & 19 \\ 
   & p=180 & 35/3/27 & - & 29 & 126/126 & 132/35 & 16 & 18 \\ 
  \midrule\multirow{4}[2]{*}{msnr} & p=14 & 14/13/19 & 16 & 19 & 18/17 & 17/17 & 6 & 9 \\ 
   & p=30 & 15/13/24 & 8 & 25 & 30/29 & 29/24 & 0 & 8 \\ 
   & p=60 & 12/10/20 & - & 20 & 43/42 & 50/25 & -6 & 6 \\ 
   & p=180 & 35/7/16 & - & 18 & 87/87 & 164/23 & 2 & 13 \\ 
  \midrule\multirow{4}[2]{*}{lsnr} & p=14 & 17/20/22 & 22 & 21 & -2/-3 & 5/3 & 5 & 4 \\ 
   & p=30 & 26/28/24 & 23 & 23 & -2/-2 & 8/6 & 5 & 3 \\ 
   & p=60 & 23/26/22 & - & 22 & -3/-3 & 20/3 & 4 & 2 \\ 
   & p=180 & 29/16/16 & - & 15 & -5/-3 & 79/1 & 1 & 0 \\ 
   \midrule 
 \multicolumn{1}{|c}{} &       & \multicolumn{7}{c|}{Relative efficiency} \\
\midrule\multirow{4}[2]{*}{hsnr} & p=14 & 0.99/1/0.85 & 0.93 & 0.85 & 0.79/0.79 & 0.92/0.91 & 0.95 & 0.91 \\ 
   & p=30 & 0.98/1/0.74 & 0.9 & 0.74 & 0.63/0.64 & 0.83/0.81 & 0.93 & 0.86 \\ 
   & p=60 & 0.98/1/0.73 & - & 0.73 & 0.57/0.57 & 0.73/0.75 & 0.92 & 0.87 \\ 
   & p=180 & 0.76/1/0.8 & - & 0.79 & 0.45/0.45 & 0.44/0.76 & 0.88 & 0.87 \\ 
  \midrule\multirow{4}[2]{*}{msnr} & p=14 & 0.93/0.94/0.9 & 0.92 & 0.9 & 0.9/0.91 & 0.91/0.91 & 1 & 0.97 \\ 
   & p=30 & 0.87/0.88/0.8 & 0.93 & 0.8 & 0.77/0.77 & 0.77/0.8 & 1 & 0.92 \\ 
   & p=60 & 0.84/0.85/0.78 & - & 0.78 & 0.66/0.66 & 0.63/0.75 & 1 & 0.89 \\ 
   & p=180 & 0.75/0.95/0.88 & - & 0.87 & 0.55/0.55 & 0.39/0.83 & 1 & 0.9 \\ 
  \midrule\multirow{4}[2]{*}{lsnr} & p=14 & 0.83/0.81/0.8 & 0.8 & 0.81 & 0.99/1 & 0.93/0.94 & 0.93 & 0.94 \\ 
   & p=30 & 0.78/0.76/0.79 & 0.8 & 0.8 & 1/1 & 0.91/0.93 & 0.93 & 0.95 \\ 
   & p=60 & 0.78/0.77/0.79 & - & 0.8 & 1/1 & 0.8/0.94 & 0.93 & 0.95 \\ 
   & p=180 & 0.74/0.82/0.82 & - & 0.83 & 1/0.98 & 0.53/0.94 & 0.95 & 0.95 \\ 
   \midrule 
 \multicolumn{1}{|c}{} &       & \multicolumn{7}{c|}{Sparsistency (number of extra variables)} \\
\midrule\multirow{4}[2]{*}{hsnr} & p=14 & 6(0.6)/6(0.5)/6(1.4) & 6(0.6) & 6(1.4) & 6(3.9)/6(4.5) & 6(1)/6(1.4) & 6(0.7) & 6(1.2) \\ 
   & p=30 & 6(0.7)/6(0.6)/6(2.1) & 6(0.8) & 6(2.1) & 6(9.2)/6(10.3) & 6(2.5)/6(3.4) & 6(1.6) & 6(2.3) \\ 
   & p=60 & 6(0.8)/6(0.7)/6(2) & - & 6(1.9) & 6(12.4)/6(14.2) & 6(5.1)/6(4.7) & 6(2.5) & 6(2.1) \\ 
   & p=180 & 6(9.2)/6(0.1)/6(0.6) & - & 6(0.6) & 6(16.2)/6(22.2) & 6(18.1)/6(3.4) & 6(2.4) & 6(0.8) \\ 
  \midrule\multirow{4}[2]{*}{msnr} & p=14 & 5.6(1.2)/5.6(1.1)/5.8(2.1) & 5.8(1.8) & 5.8(2.1) & 6(4)/6(4.5) & 5.7(1.5)/5.8(2.6) & 5.8(1) & 5.9(1.9) \\ 
   & p=30 & 5.1(1.5)/5.1(1.2)/5.3(2.6) & 5.5(1.4) & 5.3(2.6) & 6(9.1)/6(10.2) & 5.2(4.1)/5.4(5.8) & 5.7(1.8) & 5.7(3.2) \\ 
   & p=60 & 5.2(1.2)/5.2(1)/5.2(1.7) & - & 5.2(1.6) & 5.9(12.4)/6(14.1) & 5.2(7.5)/5.3(5.2) & 5.8(1.7) & 5.7(2.8) \\ 
   & p=180 & 5.6(10)/5.6(0.5)/5.6(0.8) & - & 5.6(0.8) & 6(16.2)/6(22.2) & 5.6(27.5)/5.6(3.1) & 5.9(1.7) & 5.9(1.9) \\ 
  \midrule\multirow{4}[2]{*}{lsnr} & p=14 & 4.4(4)/4.2(3.6)/3.7(2.5) & 3.6(2.4) & 3.7(2.3) & 4.8(3.6)/4.9(4.1) & 3.9(2.1)/4.4(3.2) & 4.5(2.5) & 4.5(3) \\ 
   & p=30 & 2.6(4.4)/1.9(2.3)/2.4(3) & 2.5(2.8) & 2.4(2.9) & 3.9(7.5)/4(8.2) & 3.3(4.9)/3.3(6.3) & 3.7(6.1) & 3.4(5.3) \\ 
   & p=60 & 1.7(2)/1.1(0.8)/1.8(2) & - & 1.8(1.9) & 3.7(9.4)/3.8(10.4) & 3.4(8.9)/3.2(7.6) & 3.4(7.7) & 3.2(6.5) \\ 
   & p=180 & 1.4(14.4)/0.5(0.2)/1.1(1.1) & - & 1.1(1.1) & 3.2(11.1)/3.3(14.7) & 3.5(36.7)/2.8(10.2) & 3(10.8) & 2.8(9.1) \\ 
   \bottomrule 
\end{tabular}
}
\end{table}
