# Supplementary material for: On the Use of Information Criteria for Subset Selection in Least Squares Regression
Source: arXiv:1911.10191 source file (2021-03-06)
Supplement: Supplementary file 25 [file Sparse-Ex4_n2000_rho_0.tex]

% latex table generated in R 3.6.2 by xtable 1.8-4 package
% Sat Dec 21 23:36:18 2019
\begin{table}[ht]
\centering
\caption{The performance of BOSS compared to other methods, Sparse-Ex4, $\rho$=0, n=2000} 
\scalebox{0.7}{
\begin{tabular}{|c|c|ccccccc|}
  \toprule 
 \multicolumn{1}{|c}{} &       & BOSS  & BS    & FS    & LASSO & Gamma LASSO & SparseNet & \multicolumn{1}{c|}{rLASSO} \\
 \multicolumn{1}{|c}{} &       & C$_p$-hdf/AICc-hdf/CV & CV    & CV    & AICc/CV & AICc/CV & CV    & \multicolumn{1}{c|}{CV}  \\
 \cmidrule{3-9}\multicolumn{1}{|c}{} &       & \multicolumn{7}{c|}{\% worse than the best possible BOSS}  \\
 \midrule\multirow{4}[2]{*}{hsnr} & p=14 & 9/9/17 & 17 & 17 & 41/41 & 19/15 & 12 & 13 \\ 
   & p=30 & 5/5/22 & 22 & 23 & 74/71 & 45/22 & 13 & 16 \\ 
   & p=60 & 4/4/24 & - & 23 & 97/93 & 83/23 & 16 & 17 \\ 
   & p=180 & 4/4/21 & - & 21 & 131/127 & 200/23 & 13 & 17 \\ 
  \midrule\multirow{4}[2]{*}{msnr} & p=14 & 31/31/21 & 21 & 22 & 34/33 & 20/20 & 22 & 22 \\ 
   & p=30 & 40/40/29 & 31 & 29 & 52/50 & 42/29 & 28 & 34 \\ 
   & p=60 & 40/40/32 & - & 32 & 64/61 & 76/29 & 29 & 33 \\ 
   & p=180 & 39/40/31 & - & 32 & 67/64 & 157/27 & 27 & 30 \\ 
  \midrule\multirow{4}[2]{*}{lsnr} & p=14 & 19/19/19 & 19 & 19 & 28/28 & 24/18 & 16 & 16 \\ 
   & p=30 & 11/11/21 & 22 & 21 & 49/47 & 57/20 & 14 & 17 \\ 
   & p=60 & 10/9/20 & - & 20 & 64/61 & 102/19 & 13 & 17 \\ 
   & p=180 & 9/8/20 & - & 20 & 91/88 & 235/21 & 14 & 18 \\ 
   \midrule 
 \multicolumn{1}{|c}{} &       & \multicolumn{7}{c|}{Relative efficiency} \\
\midrule\multirow{4}[2]{*}{hsnr} & p=14 & 1/1/0.93 & 0.93 & 0.93 & 0.77/0.77 & 0.91/0.95 & 0.97 & 0.96 \\ 
   & p=30 & 1/1/0.86 & 0.86 & 0.86 & 0.6/0.61 & 0.72/0.86 & 0.93 & 0.91 \\ 
   & p=60 & 1/1/0.84 & - & 0.84 & 0.53/0.54 & 0.57/0.85 & 0.9 & 0.89 \\ 
   & p=180 & 1/1/0.86 & - & 0.86 & 0.45/0.46 & 0.35/0.85 & 0.92 & 0.89 \\ 
  \midrule\multirow{4}[2]{*}{msnr} & p=14 & 0.91/0.91/0.99 & 0.99 & 0.98 & 0.9/0.9 & 1/0.99 & 0.98 & 0.98 \\ 
   & p=30 & 0.91/0.91/0.99 & 0.97 & 0.99 & 0.84/0.85 & 0.9/0.99 & 1 & 0.95 \\ 
   & p=60 & 0.92/0.92/0.97 & - & 0.98 & 0.78/0.8 & 0.73/1 & 1 & 0.97 \\ 
   & p=180 & 0.91/0.91/0.96 & - & 0.96 & 0.76/0.77 & 0.49/1 & 1 & 0.97 \\ 
  \midrule\multirow{4}[2]{*}{lsnr} & p=14 & 0.97/0.97/0.97 & 0.97 & 0.97 & 0.9/0.91 & 0.93/0.98 & 1 & 1 \\ 
   & p=30 & 1/1/0.92 & 0.91 & 0.92 & 0.74/0.76 & 0.71/0.93 & 0.98 & 0.95 \\ 
   & p=60 & 1/1/0.91 & - & 0.91 & 0.67/0.68 & 0.54/0.92 & 0.97 & 0.93 \\ 
   & p=180 & 1/1/0.9 & - & 0.9 & 0.57/0.58 & 0.32/0.9 & 0.95 & 0.92 \\ 
   \midrule 
 \multicolumn{1}{|c}{} &       & \multicolumn{7}{c|}{Sparsistency (number of extra variables)} \\
\midrule\multirow{4}[2]{*}{hsnr} & p=14 & 6(0.4)/6(0.4)/6(0.6) & 6(0.6) & 6(0.6) & 6(3.8)/6(4.5) & 6(1.1)/6(0.8) & 6(0.5) & 6(0.5) \\ 
   & p=30 & 6(0.1)/6(0.1)/6(0.6) & 6(0.6) & 6(0.6) & 6(8.4)/6(8.7) & 6(2.9)/6(1.3) & 6(0.7) & 6(0.5) \\ 
   & p=60 & 6(0.1)/6(0.1)/6(0.5) & - & 6(0.5) & 6(13)/6(12.2) & 6(6.8)/6(1.5) & 6(1.1) & 6(0.6) \\ 
   & p=180 & 6(0)/6(0)/6(0.3) & - & 6(0.3) & 6(21.7)/6(19.4) & 6(24.4)/6(1.5) & 6(1.2) & 6(0.5) \\ 
  \midrule\multirow{4}[2]{*}{msnr} & p=14 & 5.8(1.9)/5.8(1.8)/5.8(0.8) & 5.8(0.8) & 5.8(0.8) & 6(3.8)/6(4.4) & 5.9(1.2)/5.9(1.5) & 5.8(1.1) & 5.8(0.9) \\ 
   & p=30 & 5.4(1)/5.4(0.9)/5.6(0.9) & 5.6(0.9) & 5.6(0.9) & 6(8.5)/6(8.6) & 5.9(3.4)/5.7(2.2) & 5.7(1.9) & 5.6(1.5) \\ 
   & p=60 & 5.2(0.3)/5.2(0.3)/5.6(0.8) & - & 5.6(0.8) & 6(13)/6(12.1) & 5.9(7.8)/5.7(2.6) & 5.7(2.7) & 5.6(1.4) \\ 
   & p=180 & 4.7(0.1)/4.7(0.1)/5.2(0.6) & - & 5.2(0.6) & 5.9(21.7)/5.9(19) & 5.9(26.9)/5.4(2.9) & 5.4(4.5) & 5.2(1.4) \\ 
  \midrule\multirow{4}[2]{*}{lsnr} & p=14 & 4.5(1)/4.5(1)/4.5(0.6) & 4.5(0.6) & 4.5(0.6) & 5.3(3.4)/5.4(3.8) & 4.8(1.3)/4.6(1) & 4.5(0.7) & 4.5(0.6) \\ 
   & p=30 & 4.1(0.3)/4.1(0.3)/4.3(0.6) & 4.3(0.6) & 4.3(0.6) & 5.1(7.2)/5.1(7.3) & 4.8(3.6)/4.3(1.2) & 4.3(1) & 4.2(0.9) \\ 
   & p=60 & 4.1(0.2)/4.1(0.2)/4.2(0.5) & - & 4.2(0.5) & 5(11.2)/4.9(10.1) & 4.8(8)/4.2(1.2) & 4.2(1.2) & 4.2(0.8) \\ 
   & p=180 & 4(0.1)/4(0.1)/4.1(0.4) & - & 4.1(0.4) & 4.7(18.7)/4.6(15.6) & 4.8(27)/4.1(1) & 4.1(1.4) & 4.1(0.8) \\ 
   \bottomrule 
\end{tabular}
}
\end{table}
