# Supplementary material for: On the Use of Information Criteria for Subset Selection in Least Squares Regression
Source: arXiv:1911.10191 source file (2021-03-06)
Supplement: Supplementary file 26 [file Sparse-Ex4_n2000_rho_05.tex]

% latex table generated in R 3.6.2 by xtable 1.8-4 package
% Sat Dec 21 23:36:24 2019
\begin{table}[ht]
\centering
\caption{The performance of BOSS compared to other methods, Sparse-Ex4, $\rho$=0.5, n=2000} 
\scalebox{0.7}{
\begin{tabular}{|c|c|ccccccc|}
  \toprule 
 \multicolumn{1}{|c}{} &       & BOSS  & BS    & FS    & LASSO & Gamma LASSO & SparseNet & \multicolumn{1}{c|}{rLASSO} \\
 \multicolumn{1}{|c}{} &       & C$_p$-hdf/AICc-hdf/CV & CV    & CV    & AICc/CV & AICc/CV & CV    & \multicolumn{1}{c|}{CV}  \\
 \cmidrule{3-9}\multicolumn{1}{|c}{} &       & \multicolumn{7}{c|}{\% worse than the best possible BOSS}  \\
 \midrule\multirow{4}[2]{*}{hsnr} & p=14 & 12/11/25 & 19 & 18 & 48/47 & 19/16 & 13 & 14 \\ 
   & p=30 & 8/7/29 & 21 & 23 & 86/83 & 39/20 & 12 & 16 \\ 
   & p=60 & 7/7/28 & - & 23 & 125/120 & 73/22 & 14 & 15 \\ 
   & p=180 & 7/6/28 & - & 21 & 174/171 & 171/23 & 12 & 18 \\ 
  \midrule\multirow{4}[2]{*}{msnr} & p=14 & 33/33/26 & 18 & 20 & 44/42 & 20/23 & 18 & 34 \\ 
   & p=30 & 40/39/33 & 21 & 31 & 71/69 & 43/35 & 26 & 54 \\ 
   & p=60 & 42/43/35 & - & 42 & 93/90 & 76/44 & 31 & 69 \\ 
   & p=180 & 41/42/33 & - & 46 & 105/102 & 153/48 & 37 & 67 \\ 
  \midrule\multirow{4}[2]{*}{lsnr} & p=14 & 22/22/30 & 21 & 21 & 36/35 & 24/20 & 17 & 19 \\ 
   & p=30 & 14/13/30 & 22 & 23 & 61/59 & 55/20 & 15 & 19 \\ 
   & p=60 & 11/10/28 & - & 21 & 89/85 & 104/21 & 13 & 20 \\ 
   & p=180 & 8/8/27 & - & 20 & 125/121 & 242/19 & 10 & 26 \\ 
   \midrule 
 \multicolumn{1}{|c}{} &       & \multicolumn{7}{c|}{Relative efficiency} \\
\midrule\multirow{4}[2]{*}{hsnr} & p=14 & 1/1/0.89 & 0.94 & 0.95 & 0.75/0.76 & 0.94/0.96 & 0.99 & 0.98 \\ 
   & p=30 & 1/1/0.83 & 0.89 & 0.87 & 0.58/0.59 & 0.77/0.89 & 0.96 & 0.93 \\ 
   & p=60 & 1/1/0.83 & - & 0.87 & 0.47/0.48 & 0.62/0.87 & 0.93 & 0.92 \\ 
   & p=180 & 1/1/0.83 & - & 0.88 & 0.39/0.39 & 0.39/0.87 & 0.95 & 0.9 \\ 
  \midrule\multirow{4}[2]{*}{msnr} & p=14 & 0.88/0.88/0.93 & 1 & 0.98 & 0.82/0.83 & 0.99/0.96 & 1 & 0.88 \\ 
   & p=30 & 0.87/0.87/0.91 & 1 & 0.93 & 0.71/0.72 & 0.85/0.9 & 0.97 & 0.79 \\ 
   & p=60 & 0.92/0.92/0.98 & - & 0.92 & 0.68/0.69 & 0.75/0.91 & 1 & 0.77 \\ 
   & p=180 & 0.94/0.94/1 & - & 0.91 & 0.65/0.66 & 0.53/0.9 & 0.97 & 0.8 \\ 
  \midrule\multirow{4}[2]{*}{lsnr} & p=14 & 0.96/0.96/0.9 & 0.97 & 0.96 & 0.86/0.87 & 0.94/0.98 & 1 & 0.98 \\ 
   & p=30 & 0.99/1/0.87 & 0.93 & 0.92 & 0.7/0.71 & 0.73/0.95 & 0.99 & 0.95 \\ 
   & p=60 & 1/1/0.86 & - & 0.91 & 0.58/0.59 & 0.54/0.91 & 0.98 & 0.92 \\ 
   & p=180 & 0.99/1/0.85 & - & 0.9 & 0.48/0.49 & 0.32/0.91 & 0.98 & 0.86 \\ 
   \midrule 
 \multicolumn{1}{|c}{} &       & \multicolumn{7}{c|}{Sparsistency (number of extra variables)} \\
\midrule\multirow{4}[2]{*}{hsnr} & p=14 & 6(0.6)/6(0.5)/6(0.6) & 6(0.7) & 6(0.6) & 6(4.7)/6(5.5) & 6(1)/6(1) & 6(0.6) & 6(0.5) \\ 
   & p=30 & 6(0.2)/6(0.2)/6(0.6) & 6(0.6) & 6(0.6) & 6(10.9)/6(11.3) & 6(2.7)/6(1.4) & 6(0.8) & 6(0.5) \\ 
   & p=60 & 6(0.1)/6(0.1)/6(0.5) & - & 6(0.5) & 6(18)/6(17.7) & 6(6.4)/6(1.5) & 6(1.1) & 6(0.4) \\ 
   & p=180 & 6(0.1)/6(0.1)/6(0.3) & - & 6(0.3) & 6(32.2)/6(29.8) & 6(22.3)/6(1.3) & 6(1.3) & 6(0.4) \\ 
  \midrule\multirow{4}[2]{*}{msnr} & p=14 & 5.9(2.1)/5.9(2)/6(0.7) & 5.9(0.7) & 5.9(0.9) & 6(4.8)/6(5.5) & 6(1.2)/5.9(1.9) & 5.9(1.1) & 5.9(1.7) \\ 
   & p=30 & 5.6(1.1)/5.6(1)/5.9(0.8) & 5.9(0.7) & 5.8(1) & 6(10.9)/6(11.3) & 6(3.3)/5.8(2.8) & 5.8(2) & 5.6(2.2) \\ 
   & p=60 & 5.4(0.4)/5.3(0.3)/5.8(0.8) & - & 5.6(1.1) & 6(18)/6(17.6) & 6(7.7)/5.6(3.7) & 5.7(3.1) & 5.3(2.3) \\ 
   & p=180 & 4.8(0.2)/4.8(0.2)/5.5(1) & - & 5.1(0.8) & 5.9(31.7)/5.9(29) & 6(26.5)/5.1(4.5) & 5.2(4.7) & 4.7(2) \\ 
  \midrule\multirow{4}[2]{*}{lsnr} & p=14 & 4.6(1.4)/4.6(1.3)/4.6(0.7) & 4.6(0.7) & 4.6(0.8) & 5.5(4.4)/5.5(5) & 4.9(1.3)/4.6(1.2) & 4.5(0.8) & 4.4(0.8) \\ 
   & p=30 & 4.2(0.5)/4.2(0.4)/4.3(0.7) & 4.3(0.6) & 4.2(0.7) & 5.2(9.6)/5.3(9.9) & 4.8(3.6)/4.3(1.1) & 4.3(1) & 4.2(0.8) \\ 
   & p=60 & 4.1(0.2)/4.1(0.2)/4.2(0.5) & - & 4.1(0.5) & 5(15.5)/5(14.7) & 4.8(8.2)/4.1(1.2) & 4.1(1.2) & 4.1(0.9) \\ 
   & p=180 & 4(0.1)/4(0.1)/4(0.4) & - & 4(0.4) & 4.6(26.1)/4.6(23.6) & 4.8(27.9)/4(1) & 4.1(1.3) & 4(0.9) \\ 
   \bottomrule 
\end{tabular}
}
\end{table}
