# Supplementary material for: On the Use of Information Criteria for Subset Selection in Least Squares Regression
Source: arXiv:1911.10191 source file (2021-03-06)
Supplement: Supplementary file 27 [file Sparse-Ex4_n2000_rho_09.tex]

% latex table generated in R 3.6.2 by xtable 1.8-4 package
% Sat Dec 21 23:36:30 2019
\begin{table}[ht]
\centering
\caption{The performance of BOSS compared to other methods, Sparse-Ex4, $\rho$=0.9, n=2000} 
\scalebox{0.7}{
\begin{tabular}{|c|c|ccccccc|}
  \toprule 
 \multicolumn{1}{|c}{} &       & BOSS  & BS    & FS    & LASSO & Gamma LASSO & SparseNet & \multicolumn{1}{c|}{rLASSO} \\
 \multicolumn{1}{|c}{} &       & C$_p$-hdf/AICc-hdf/CV & CV    & CV    & AICc/CV & AICc/CV & CV    & \multicolumn{1}{c|}{CV}  \\
 \cmidrule{3-9}\multicolumn{1}{|c}{} &       & \multicolumn{7}{c|}{\% worse than the best possible BOSS}  \\
 \midrule\multirow{4}[2]{*}{hsnr} & p=14 & 33/33/27 & 16 & 20 & 53/51 & 17/20 & 15 & 27 \\ 
   & p=30 & 33/32/33 & 16 & 33 & 108/106 & 26/22 & 12 & 46 \\ 
   & p=60 & 27/26/30 & - & 48 & 157/154 & 37/22 & 9 & 73 \\ 
   & p=180 & 15/15/25 & - & 90 & 226/223 & 68/33 & 10 & 140 \\ 
  \midrule\multirow{4}[2]{*}{msnr} & p=14 & 28/28/22 & 18 & 45 & 53/51 & 26/39 & 30 & 57 \\ 
   & p=30 & 22/22/26 & 23 & 89 & 108/105 & 56/75 & 55 & 109 \\ 
   & p=60 & 21/21/27 & - & 114 & 166/162 & 100/107 & 92 & 124 \\ 
   & p=180 & 25/25/30 & - & 107 & 253/250 & 190/110 & 105 & 106 \\ 
  \midrule\multirow{4}[2]{*}{lsnr} & p=14 & 33/33/32 & 20 & 29 & 45/44 & 24/28 & 19 & 37 \\ 
   & p=30 & 28/27/34 & 16 & 40 & 85/82 & 44/30 & 12 & 57 \\ 
   & p=60 & 19/19/30 & - & 59 & 122/119 & 75/32 & 9 & 89 \\ 
   & p=180 & 15/14/27 & - & 104 & 179/176 & 167/48 & 20 & 159 \\ 
   \midrule 
 \multicolumn{1}{|c}{} &       & \multicolumn{7}{c|}{Relative efficiency} \\
\midrule\multirow{4}[2]{*}{hsnr} & p=14 & 0.86/0.86/0.9 & 0.99 & 0.96 & 0.75/0.76 & 0.98/0.95 & 1 & 0.91 \\ 
   & p=30 & 0.84/0.84/0.84 & 0.96 & 0.84 & 0.54/0.54 & 0.89/0.92 & 1 & 0.77 \\ 
   & p=60 & 0.86/0.86/0.84 & - & 0.74 & 0.42/0.43 & 0.8/0.89 & 1 & 0.63 \\ 
   & p=180 & 0.95/0.96/0.88 & - & 0.58 & 0.34/0.34 & 0.65/0.82 & 1 & 0.46 \\ 
  \midrule\multirow{4}[2]{*}{msnr} & p=14 & 0.92/0.92/0.97 & 1 & 0.81 & 0.77/0.78 & 0.94/0.85 & 0.91 & 0.76 \\ 
   & p=30 & 0.99/1/0.96 & 0.99 & 0.64 & 0.58/0.59 & 0.78/0.7 & 0.78 & 0.58 \\ 
   & p=60 & 1/1/0.95 & - & 0.56 & 0.45/0.46 & 0.6/0.58 & 0.63 & 0.54 \\ 
   & p=180 & 1/1/0.96 & - & 0.6 & 0.35/0.36 & 0.43/0.6 & 0.61 & 0.61 \\ 
  \midrule\multirow{4}[2]{*}{lsnr} & p=14 & 0.9/0.9/0.9 & 1 & 0.92 & 0.82/0.83 & 0.96/0.93 & 1 & 0.87 \\ 
   & p=30 & 0.87/0.88/0.83 & 0.97 & 0.8 & 0.61/0.61 & 0.78/0.86 & 1 & 0.71 \\ 
   & p=60 & 0.92/0.92/0.84 & - & 0.69 & 0.49/0.5 & 0.62/0.83 & 1 & 0.58 \\ 
   & p=180 & 1/1/0.9 & - & 0.56 & 0.41/0.41 & 0.43/0.77 & 0.95 & 0.44 \\ 
   \midrule 
 \multicolumn{1}{|c}{} &       & \multicolumn{7}{c|}{Sparsistency (number of extra variables)} \\
\midrule\multirow{4}[2]{*}{hsnr} & p=14 & 6(1.4)/6(1.4)/6(0.6) & 6(0.7) & 6(0.9) & 6(6.6)/6(7.2) & 6(1.2)/6(1.8) & 6(0.9) & 6(1.4) \\ 
   & p=30 & 6(0.5)/6(0.4)/6(0.7) & 6(0.6) & 6(1.3) & 6(17.8)/6(18.9) & 6(2.6)/6(2.5) & 6(1.6) & 6(2.4) \\ 
   & p=60 & 6(0.4)/6(0.4)/6(0.8) & - & 6(2) & 6(34.2)/6(35.3) & 6(5.8)/6(3.9) & 6(3.1) & 6(4.1) \\ 
   & p=180 & 6(1.4)/6(1.4)/6(1.7) & - & 5.9(3.8) & 6(72.7)/6(73.8) & 6(17.2)/6(9.4) & 6(8.7) & 5.9(9.4) \\ 
  \midrule\multirow{4}[2]{*}{msnr} & p=14 & 6(2)/6(2)/6(1.3) & 6(0.7) & 5.9(2.4) & 6(6.6)/6(7.2) & 6(2.4)/5.9(4.1) & 5.9(2.9) & 5.8(3.9) \\ 
   & p=30 & 5.9(2.4)/5.9(2.4)/5.9(2.6) & 5.9(0.7) & 5.4(3.4) & 6(17.8)/6(18.8) & 5.9(5.9)/5.6(7.2) & 5.6(6.2) & 5.1(5.6) \\ 
   & p=60 & 5.8(4.8)/5.8(4.8)/5.9(5.6) & - & 4.7(1.9) & 6(34)/6(35.1) & 5.8(12.4)/4.9(7.7) & 5(8.3) & 4.3(2.6) \\ 
   & p=180 & 5.5(12.9)/5.5(12.7)/5.7(16.2) & - & 4.2(0.6) & 5.7(68.6)/5.7(69.3) & 5.4(31.9)/4.2(3.4) & 4.3(5) & 4(0.3) \\ 
  \midrule\multirow{4}[2]{*}{lsnr} & p=14 & 5(2.5)/5(2.4)/4.7(1.1) & 4.6(0.7) & 4.6(1.5) & 5.7(6.4)/5.7(7) & 4.6(1.5)/4.7(2.4) & 4.5(1.5) & 4.7(2.6) \\ 
   & p=30 & 4.5(2.1)/4.4(1.9)/4.4(1.7) & 4.3(0.6) & 4.3(2.2) & 5.4(16.6)/5.4(17.6) & 4.5(3.7)/4.3(3.5) & 4.2(2.5) & 4.4(4.6) \\ 
   & p=60 & 4.2(1.9)/4.2(1.8)/4.3(2.3) & - & 4.2(3.2) & 5.1(30.6)/5.1(31.3) & 4.3(8.1)/4.2(5.8) & 4.2(5) & 4.3(8.8) \\ 
   & p=180 & 4.1(3.7)/4.1(3.6)/4.1(4.4) & - & 3.7(3.7) & 4.6(60.3)/4.6(60.5) & 4.3(26.8)/4.1(14.8) & 4.2(14.2) & 3.6(13.7) \\ 
   \bottomrule 
\end{tabular}
}
\end{table}
