# Supplementary material for: On the Use of Information Criteria for Subset Selection in Least Squares Regression
Source: arXiv:1911.10191 source file (2021-03-06)
Supplement: Supplementary file 28 [file Sparse-Ex4_n200_rho_0.tex]

% latex table generated in R 3.6.2 by xtable 1.8-4 package
% Sat Dec 21 23:36:12 2019
\begin{table}[ht]
\centering
\caption{The performance of BOSS compared to other methods, Sparse-Ex4, $\rho$=0, n=200} 
\scalebox{0.7}{
\begin{tabular}{|c|c|ccccccc|}
  \toprule 
 \multicolumn{1}{|c}{} &       & BOSS  & BS    & FS    & LASSO & Gamma LASSO & SparseNet & \multicolumn{1}{c|}{rLASSO} \\
 \multicolumn{1}{|c}{} &       & C$_p$-hdf/AICc-hdf/CV & CV    & CV    & AICc/CV & AICc/CV & CV    & \multicolumn{1}{c|}{CV}  \\
 \cmidrule{3-9}\multicolumn{1}{|c}{} &       & \multicolumn{7}{c|}{\% worse than the best possible BOSS}  \\
 \midrule\multirow{4}[2]{*}{hsnr} & p=14 & 30/30/22 & 22 & 22 & 19/19 & 16/18 & 20 & 20 \\ 
   & p=30 & 24/21/24 & 25 & 25 & 29/28 & 32/19 & 16 & 20 \\ 
   & p=60 & 16/15/20 & - & 21 & 37/36 & 57/17 & 13 & 21 \\ 
   & p=180 & 29/5/14 & - & 15 & 50/51 & 168/14 & 11 & 16 \\ 
  \midrule\multirow{4}[2]{*}{msnr} & p=14 & 25/22/22 & 23 & 22 & 31/31 & 26/21 & 18 & 18 \\ 
   & p=30 & 26/20/27 & 28 & 28 & 52/51 & 43/24 & 21 & 26 \\ 
   & p=60 & 18/14/24 & - & 25 & 69/68 & 72/25 & 21 & 27 \\ 
   & p=180 & 55/16/26 & - & 27 & 97/99 & 237/29 & 27 & 36 \\ 
  \midrule\multirow{4}[2]{*}{lsnr} & p=14 & 34/34/29 & 30 & 29 & 16/16 & 19/25 & 25 & 19 \\ 
   & p=30 & 37/34/31 & 31 & 31 & 20/18 & 33/25 & 24 & 22 \\ 
   & p=60 & 32/33/29 & - & 29 & 20/20 & 55/24 & 22 & 22 \\ 
   & p=180 & 49/29/27 & - & 26 & 18/20 & 142/23 & 21 & 17 \\ 
   \midrule 
 \multicolumn{1}{|c}{} &       & \multicolumn{7}{c|}{Relative efficiency} \\
\midrule\multirow{4}[2]{*}{hsnr} & p=14 & 0.89/0.89/0.95 & 0.95 & 0.95 & 0.98/0.98 & 1/0.98 & 0.97 & 0.97 \\ 
   & p=30 & 0.94/0.96/0.94 & 0.93 & 0.93 & 0.9/0.91 & 0.88/0.98 & 1 & 0.97 \\ 
   & p=60 & 0.97/0.99/0.94 & - & 0.94 & 0.83/0.83 & 0.72/0.97 & 1 & 0.93 \\ 
   & p=180 & 0.82/1/0.92 & - & 0.92 & 0.7/0.7 & 0.39/0.92 & 0.94 & 0.91 \\ 
  \midrule\multirow{4}[2]{*}{msnr} & p=14 & 0.95/0.96/0.97 & 0.96 & 0.97 & 0.9/0.9 & 0.94/0.98 & 1 & 1 \\ 
   & p=30 & 0.96/1/0.95 & 0.94 & 0.94 & 0.79/0.8 & 0.84/0.97 & 0.99 & 0.95 \\ 
   & p=60 & 0.96/1/0.92 & - & 0.92 & 0.68/0.68 & 0.66/0.91 & 0.95 & 0.9 \\ 
   & p=180 & 0.74/1/0.92 & - & 0.91 & 0.59/0.58 & 0.34/0.9 & 0.91 & 0.85 \\ 
  \midrule\multirow{4}[2]{*}{lsnr} & p=14 & 0.86/0.87/0.9 & 0.89 & 0.9 & 1/1 & 0.97/0.93 & 0.93 & 0.97 \\ 
   & p=30 & 0.87/0.89/0.9 & 0.91 & 0.9 & 0.99/1 & 0.89/0.95 & 0.96 & 0.97 \\ 
   & p=60 & 0.91/0.9/0.93 & - & 0.93 & 1/1 & 0.77/0.97 & 0.98 & 0.98 \\ 
   & p=180 & 0.78/0.91/0.92 & - & 0.92 & 0.99/0.97 & 0.48/0.95 & 0.96 & 1 \\ 
   \midrule 
 \multicolumn{1}{|c}{} &       & \multicolumn{7}{c|}{Sparsistency (number of extra variables)} \\
\midrule\multirow{4}[2]{*}{hsnr} & p=14 & 5(1.7)/4.9(1.3)/5.2(0.9) & 5.2(0.9) & 5.2(0.9) & 5.8(3.4)/5.9(4.2) & 5.5(1.3)/5.3(1.5) & 5.3(1.3) & 5.2(1.1) \\ 
   & p=30 & 4.6(0.7)/4.4(0.2)/4.9(0.9) & 4.9(1.1) & 4.9(1) & 5.7(7)/5.8(8) & 5.4(3.3)/5(1.9) & 5(2) & 5(1.4) \\ 
   & p=60 & 4.3(0.2)/4.2(0)/4.6(0.7) & - & 4.6(0.7) & 5.5(10.4)/5.6(12.1) & 5.4(7.5)/4.8(2.2) & 4.9(2.8) & 4.6(1.6) \\ 
   & p=180 & 4.3(10.2)/4.1(0)/4.2(0.4) & - & 4.3(0.5) & 5.2(14)/5.3(19) & 5.4(35.4)/4.4(2.3) & 4.5(3.9) & 4.3(1.5) \\ 
  \midrule\multirow{4}[2]{*}{msnr} & p=14 & 4.5(1.3)/4.4(1)/4.4(0.6) & 4.4(0.7) & 4.4(0.7) & 5.2(3.1)/5.2(3.6) & 4.6(1.1)/4.5(1) & 4.4(0.8) & 4.4(0.7) \\ 
   & p=30 & 4.2(0.8)/4.1(0.4)/4.2(0.8) & 4.2(0.8) & 4.2(0.8) & 5(6.5)/5(7.1) & 4.6(2.9)/4.3(1.3) & 4.3(1.3) & 4.3(1.2) \\ 
   & p=60 & 4(0.3)/4(0.2)/4.1(0.6) & - & 4.1(0.6) & 4.7(9.5)/4.7(10.7) & 4.5(6.5)/4.1(1.3) & 4.2(1.7) & 4.1(1.2) \\ 
   & p=180 & 4.1(10.4)/3.9(0.1)/4(0.5) & - & 4(0.5) & 4.4(13.1)/4.5(17.1) & 4.6(31.6)/4(1.6) & 4.1(2.6) & 4(1.7) \\ 
  \midrule\multirow{4}[2]{*}{lsnr} & p=14 & 3.9(2.4)/3.7(2)/3.3(0.9) & 3.3(1.1) & 3.2(0.9) & 4.4(2.7)/4.5(3) & 3.7(1.3)/3.6(1.5) & 3.6(1.6) & 3.6(1.2) \\ 
   & p=30 & 2.6(1.8)/2.2(0.7)/2.5(1.1) & 2.5(1.1) & 2.5(1.1) & 3.8(5.3)/3.9(5.5) & 3.4(3.5)/2.9(2.5) & 3(2.9) & 3(2.4) \\ 
   & p=60 & 2(0.8)/1.7(0.2)/2.2(0.8) & - & 2.2(0.8) & 3.4(7.3)/3.5(8.1) & 3.5(7.8)/2.7(3.3) & 2.8(3.9) & 2.7(3.1) \\ 
   & p=180 & 1.8(12)/1.3(0.1)/1.6(0.6) & - & 1.7(0.6) & 2.9(9.7)/2.9(11.2) & 3.7(34)/2.2(5) & 2.4(6.2) & 2.2(3.8) \\ 
   \bottomrule 
\end{tabular}
}
\end{table}
