# Supplementary material for: On the Use of Information Criteria for Subset Selection in Least Squares Regression
Source: arXiv:1911.10191 source file (2021-03-06)
Supplement: Supplementary file 29 [file Sparse-Ex4_n200_rho_05.tex]

% latex table generated in R 3.6.2 by xtable 1.8-4 package
% Sat Dec 21 23:36:18 2019
\begin{table}[ht]
\centering
\caption{The performance of BOSS compared to other methods, Sparse-Ex4, $\rho$=0.5, n=200} 
\scalebox{0.7}{
\begin{tabular}{|c|c|ccccccc|}
  \toprule 
 \multicolumn{1}{|c}{} &       & BOSS  & BS    & FS    & LASSO & Gamma LASSO & SparseNet & \multicolumn{1}{c|}{rLASSO} \\
 \multicolumn{1}{|c}{} &       & C$_p$-hdf/AICc-hdf/CV & CV    & CV    & AICc/CV & AICc/CV & CV    & \multicolumn{1}{c|}{CV}  \\
 \cmidrule{3-9}\multicolumn{1}{|c}{} &       & \multicolumn{7}{c|}{\% worse than the best possible BOSS}  \\
 \midrule\multirow{4}[2]{*}{hsnr} & p=14 & 34/33/25 & 22 & 26 & 29/28 & 17/25 & 25 & 33 \\ 
   & p=30 & 23/19/24 & 23 & 28 & 49/47 & 34/26 & 21 & 32 \\ 
   & p=60 & 18/17/21 & - & 24 & 56/54 & 52/21 & 17 & 28 \\ 
   & p=180 & 29/4/15 & - & 16 & 82/81 & 170/16 & 13 & 15 \\ 
  \midrule\multirow{4}[2]{*}{msnr} & p=14 & 27/25/29 & 20 & 21 & 38/37 & 25/20 & 17 & 24 \\ 
   & p=30 & 24/19/34 & 24 & 30 & 74/72 & 52/26 & 16 & 52 \\ 
   & p=60 & 17/13/33 & - & 28 & 90/89 & 78/26 & 14 & 62 \\ 
   & p=180 & 52/14/37 & - & 29 & 137/137 & 263/29 & 17 & 91 \\ 
  \midrule\multirow{4}[2]{*}{lsnr} & p=14 & 37/35/31 & 24 & 30 & 30/29 & 23/29 & 26 & 33 \\ 
   & p=30 & 37/35/32 & 23 & 34 & 35/35 & 30/31 & 23 & 38 \\ 
   & p=60 & 37/38/32 & - & 36 & 38/40 & 53/34 & 24 & 42 \\ 
   & p=180 & 49/31/26 & - & 34 & 33/35 & 120/31 & 20 & 38 \\ 
   \midrule 
 \multicolumn{1}{|c}{} &       & \multicolumn{7}{c|}{Relative efficiency} \\
\midrule\multirow{4}[2]{*}{hsnr} & p=14 & 0.88/0.88/0.94 & 0.97 & 0.93 & 0.91/0.92 & 1/0.94 & 0.94 & 0.89 \\ 
   & p=30 & 0.97/1/0.96 & 0.97 & 0.93 & 0.8/0.81 & 0.89/0.95 & 0.99 & 0.9 \\ 
   & p=60 & 0.99/1/0.96 & - & 0.94 & 0.75/0.76 & 0.77/0.96 & 1 & 0.91 \\ 
   & p=180 & 0.81/1/0.91 & - & 0.9 & 0.57/0.58 & 0.39/0.9 & 0.92 & 0.91 \\ 
  \midrule\multirow{4}[2]{*}{msnr} & p=14 & 0.92/0.94/0.91 & 0.97 & 0.96 & 0.84/0.85 & 0.93/0.97 & 1 & 0.94 \\ 
   & p=30 & 0.93/0.98/0.87 & 0.93 & 0.89 & 0.66/0.67 & 0.76/0.92 & 1 & 0.76 \\ 
   & p=60 & 0.97/1/0.85 & - & 0.88 & 0.6/0.6 & 0.64/0.9 & 1 & 0.7 \\ 
   & p=180 & 0.74/1/0.83 & - & 0.88 & 0.48/0.48 & 0.31/0.88 & 0.97 & 0.59 \\ 
  \midrule\multirow{4}[2]{*}{lsnr} & p=14 & 0.9/0.91/0.94 & 0.99 & 0.95 & 0.95/0.95 & 1/0.95 & 0.98 & 0.92 \\ 
   & p=30 & 0.9/0.91/0.93 & 1 & 0.92 & 0.91/0.91 & 0.94/0.93 & 1 & 0.89 \\ 
   & p=60 & 0.91/0.9/0.94 & - & 0.91 & 0.9/0.89 & 0.81/0.93 & 1 & 0.87 \\ 
   & p=180 & 0.81/0.92/0.96 & - & 0.9 & 0.91/0.89 & 0.55/0.92 & 1 & 0.87 \\ 
   \midrule 
 \multicolumn{1}{|c}{} &       & \multicolumn{7}{c|}{Sparsistency (number of extra variables)} \\
\midrule\multirow{4}[2]{*}{hsnr} & p=14 & 5.2(1.9)/5.1(1.4)/5.5(0.9) & 5.5(0.9) & 5.4(1) & 5.9(4.6)/6(5.4) & 5.7(1.3)/5.4(1.9) & 5.4(1.4) & 5.2(1.4) \\ 
   & p=30 & 4.5(0.9)/4.4(0.2)/5(1) & 5(1) & 4.8(1.1) & 5.7(10.4)/5.7(12) & 5.4(3.6)/4.8(2.3) & 4.8(2.1) & 4.5(1.8) \\ 
   & p=60 & 4.4(0.3)/4.2(0.1)/4.7(0.8) & - & 4.6(0.8) & 5.6(15)/5.7(17.8) & 5.5(7.4)/4.7(2.3) & 4.8(2.8) & 4.4(1.6) \\ 
   & p=180 & 4.3(11.4)/4(0)/4.2(0.5) & - & 4.1(0.5) & 5.1(20.2)/5.3(27.9) & 5.2(35.3)/4.2(2.1) & 4.2(3.5) & 4.1(0.8) \\ 
  \midrule\multirow{4}[2]{*}{msnr} & p=14 & 4.7(1.6)/4.6(1.3)/4.4(0.6) & 4.5(0.7) & 4.5(0.7) & 5.4(4.2)/5.5(5) & 4.7(1.1)/4.6(1.2) & 4.5(0.8) & 4.6(1.1) \\ 
   & p=30 & 4.2(1)/4.1(0.5)/4.2(0.7) & 4.2(0.7) & 4.2(1) & 5(9.3)/5.1(10.7) & 4.5(3.1)/4.2(1.4) & 4.2(1.2) & 4.3(2.9) \\ 
   & p=60 & 4.1(0.4)/4(0.2)/4.1(0.6) & - & 4.1(0.8) & 4.8(13.6)/4.9(15.9) & 4.5(6.8)/4.1(1.6) & 4.1(1.8) & 4.1(3.8) \\ 
   & p=180 & 4.1(10.7)/4(0.1)/4(0.4) & - & 4(0.6) & 4.5(19.3)/4.6(26.2) & 4.5(35.4)/4(1.7) & 4.1(2.6) & 4(5.2) \\ 
  \midrule\multirow{4}[2]{*}{lsnr} & p=14 & 4(2.7)/3.8(2.2)/3.3(0.8) & 3.3(0.8) & 3.3(1) & 4.5(3.6)/4.7(4.1) & 3.7(1.4)/3.5(1.7) & 3.4(1.4) & 3.7(2) \\ 
   & p=30 & 2.7(2.3)/2.3(1)/2.7(1.3) & 2.6(1) & 2.6(1.5) & 3.6(6.9)/3.6(7.5) & 3.4(3.7)/2.9(3.3) & 2.8(2.9) & 2.9(4) \\ 
   & p=60 & 1.9(1.1)/1.5(0.3)/2.3(1.2) & - & 2(1.1) & 2.9(8.5)/2.9(9.5) & 3.4(7.8)/2.4(4) & 2.5(3.9) & 2.4(5.2) \\ 
   & p=180 & 1.7(12.7)/1(0.2)/1.6(0.9) & - & 1.3(0.8) & 2.2(10.7)/2.1(13.3) & 3.5(32.4)/1.9(6.4) & 2.1(6.5) & 1.9(8) \\ 
   \bottomrule 
\end{tabular}
}
\end{table}
