# Supplementary material for: On the Use of Information Criteria for Subset Selection in Least Squares Regression
Source: arXiv:1911.10191 source file (2021-03-06)
Supplement: Supplementary file 30 [file Sparse-Ex4_n200_rho_09.tex]

% latex table generated in R 3.6.2 by xtable 1.8-4 package
% Sat Dec 21 23:36:25 2019
\begin{table}[ht]
\centering
\caption{The performance of BOSS compared to other methods, Sparse-Ex4, $\rho$=0.9, n=200} 
\scalebox{0.7}{
\begin{tabular}{|c|c|ccccccc|}
  \toprule 
 \multicolumn{1}{|c}{} &       & BOSS  & BS    & FS    & LASSO & Gamma LASSO & SparseNet & \multicolumn{1}{c|}{rLASSO} \\
 \multicolumn{1}{|c}{} &       & C$_p$-hdf/AICc-hdf/CV & CV    & CV    & AICc/CV & AICc/CV & CV    & \multicolumn{1}{c|}{CV}  \\
 \cmidrule{3-9}\multicolumn{1}{|c}{} &       & \multicolumn{7}{c|}{\% worse than the best possible BOSS}  \\
 \midrule\multirow{4}[2]{*}{hsnr} & p=14 & 34/33/29 & 24 & 46 & 45/44 & 33/43 & 40 & 53 \\ 
   & p=30 & 25/21/33 & 21 & 56 & 73/71 & 40/36 & 28 & 58 \\ 
   & p=60 & 23/22/37 & - & 57 & 95/91 & 50/31 & 22 & 64 \\ 
   & p=180 & 27/7/34 & - & 68 & 123/110 & 91/2 & -10 & 62 \\ 
  \midrule\multirow{4}[2]{*}{msnr} & p=14 & 29/27/28 & 15 & 33 & 41/39 & 23/28 & 16 & 39 \\ 
   & p=30 & 25/19/30 & -4 & 52 & 61/60 & 29/23 & 3 & 56 \\ 
   & p=60 & 22/14/24 & - & 83 & 90/86 & 57/38 & 16 & 91 \\ 
   & p=180 & 31/17/26 & - & 66 & 78/66 & 78/26 & 6 & 70 \\ 
  \midrule\multirow{4}[2]{*}{lsnr} & p=14 & 41/39/31 & 27 & 54 & 51/50 & 46/47 & 38 & 55 \\ 
   & p=30 & 39/32/27 & 18 & 78 & 71/72 & 58/66 & 44 & 75 \\ 
   & p=60 & 29/28/23 & - & 81 & 80/80 & 79/79 & 57 & 84 \\ 
   & p=180 & 37/17/18 & - & 36 & 33/33 & 110/37 & 35 & 36 \\ 
   \midrule 
 \multicolumn{1}{|c}{} &       & \multicolumn{7}{c|}{Relative efficiency} \\
\midrule\multirow{4}[2]{*}{hsnr} & p=14 & 0.93/0.94/0.96 & 1 & 0.85 & 0.86/0.86 & 0.94/0.87 & 0.89 & 0.81 \\ 
   & p=30 & 0.97/1/0.91 & 1 & 0.78 & 0.7/0.71 & 0.87/0.9 & 0.95 & 0.77 \\ 
   & p=60 & 0.99/1/0.89 & - & 0.77 & 0.62/0.64 & 0.81/0.93 & 0.99 & 0.74 \\ 
   & p=180 & 0.71/0.84/0.68 & - & 0.54 & 0.41/0.43 & 0.47/0.88 & 1 & 0.56 \\ 
  \midrule\multirow{4}[2]{*}{msnr} & p=14 & 0.89/0.91/0.9 & 1 & 0.87 & 0.82/0.83 & 0.93/0.9 & 0.99 & 0.83 \\ 
   & p=30 & 0.77/0.81/0.74 & 1 & 0.63 & 0.6/0.6 & 0.75/0.78 & 0.93 & 0.62 \\ 
   & p=60 & 0.93/1/0.92 & - & 0.62 & 0.6/0.61 & 0.73/0.83 & 0.99 & 0.6 \\ 
   & p=180 & 0.81/0.9/0.84 & - & 0.64 & 0.59/0.64 & 0.59/0.84 & 1 & 0.62 \\ 
  \midrule\multirow{4}[2]{*}{lsnr} & p=14 & 0.9/0.91/0.97 & 1 & 0.83 & 0.84/0.84 & 0.87/0.86 & 0.92 & 0.82 \\ 
   & p=30 & 0.85/0.89/0.93 & 1 & 0.66 & 0.69/0.69 & 0.75/0.71 & 0.82 & 0.67 \\ 
   & p=60 & 0.95/0.97/1 & - & 0.68 & 0.69/0.68 & 0.69/0.69 & 0.78 & 0.67 \\ 
   & p=180 & 0.86/1/0.99 & - & 0.86 & 0.88/0.88 & 0.56/0.86 & 0.87 & 0.86 \\ 
   \midrule 
 \multicolumn{1}{|c}{} &       & \multicolumn{7}{c|}{Sparsistency (number of extra variables)} \\
\midrule\multirow{4}[2]{*}{hsnr} & p=14 & 5.8(2.9)/5.7(2.5)/5.6(1.6) & 5.6(0.8) & 5.3(2) & 6(6.5)/6(7.2) & 5.5(2.3)/5.4(3.4) & 5.3(2.4) & 5.4(3.2) \\ 
   & p=30 & 5.2(3.7)/5.1(2.8)/5.3(3.8) & 5(1) & 4.8(4.1) & 5.8(17.8)/5.8(19.5) & 4.9(4.5)/4.5(3.4) & 4.4(2.7) & 4.8(6.8) \\ 
   & p=60 & 5(4.2)/4.8(3)/4.9(4.7) & - & 4.5(4.3) & 5.6(30.2)/5.7(35.1) & 4.9(8.8)/4.3(3.6) & 4.3(3.3) & 4.3(8.7) \\ 
   & p=180 & 4.4(13.2)/4.2(2.4)/4.3(4.3) & - & 4.3(8) & 4.6(44.2)/4.8(64.9) & 4.4(29.2)/4.1(4) & 4.1(3.1) & 4.1(15.4) \\ 
  \midrule\multirow{4}[2]{*}{msnr} & p=14 & 5(2.5)/4.9(2.2)/4.7(1.4) & 4.6(0.7) & 4.9(2.4) & 5.6(6.3)/5.7(7) & 4.6(1.8)/4.9(3.3) & 4.6(2.4) & 5(3.9) \\ 
   & p=30 & 4.5(4.5)/4.4(3.6)/4.5(3.7) & 4.2(0.7) & 4.6(6.5) & 5.2(16.9)/5.3(18.5) & 4.4(4.7)/4.5(7) & 4.4(5.8) & 4.8(11.2) \\ 
   & p=60 & 4.3(5.9)/4.2(5.1)/4.3(5.7) & - & 3.7(6.3) & 4.8(28.3)/5(32.8) & 4.4(10.4)/4.2(11.8) & 4.3(11.7) & 4.1(17.8) \\ 
   & p=180 & 4.1(24.5)/3.6(7.6)/3.7(9.2) & - & 3(8.8) & 3.8(37.7)/4.3(59.6) & 4.3(37.5)/3.6(20.4) & 3.8(22.8) & 3.2(26) \\ 
  \midrule\multirow{4}[2]{*}{lsnr} & p=14 & 4.2(3)/4(2.7)/3.8(1.9) & 3.3(0.7) & 3.9(2.9) & 4.9(5.9)/5.1(6.5) & 3.8(2.6)/4.1(4.1) & 3.7(3.2) & 4.4(4.7) \\ 
   & p=30 & 3.1(5.5)/2.7(3.9)/3.2(5) & 2.7(0.9) & 2.2(4.4) & 3(10.1)/3(11) & 3.3(7.6)/2.8(8) & 2.9(8) & 2.6(8.5) \\ 
   & p=60 & 2.2(5.3)/1.9(3.9)/2.6(6.8) & - & 0.9(2) & 1.2(7.4)/1.2(8.4) & 2.8(12.8)/1.3(6.6) & 2(10) & 1.1(6.4) \\ 
   & p=180 & 1.4(18.2)/0.7(1.7)/1.1(5.5) & - & 0.2(0.6) & 0.3(4.8)/0.3(5.4) & 2.3(40.2)/0.3(4.4) & 0.6(9) & 0.3(4.4) \\ 
   \bottomrule 
\end{tabular}
}
\end{table}
