# Supplementary material for: On the Use of Information Criteria for Subset Selection in Least Squares Regression
Source: arXiv:1911.10191 source file (2021-03-06)
Supplement: Supplementary file 31 [file Dense_rho_0.tex]

% latex table generated in R 4.0.3 by xtable 1.8-4 package
% Sun Feb 21 09:14:41 2021
\begin{table}[ht]
\centering
\caption{The performance of BOSS for high dimensional data, Dense, $\rho$=0, n=200} 
\scalebox{0.55}{
\begin{tabular}{|c|c|ccccccccc|}
  \toprule 
 \multicolumn{1}{|c}{} &       & BOSS  & FS    & FSstop & FStrim & FSstoptrim & lasso & Gamma lasso & SparseNet & rlasso \\
 \multicolumn{1}{|c}{} &       & C$_p$/AICc/CV & EBIC/HDBIC/HDHQ/CV & EBIC/HDBIC/HDHQ & HDBIC & HDBIC & AICc/CV & AICc/CV & CV    & CV  \\
 \cmidrule{3-11}\multicolumn{1}{|c}{} &       & \multicolumn{9}{c|}{\% worse than the best possible BOSS}  \\
 \midrule\multirow{4}[2]{*}{hsnr} & p=250 & 11/14/14 & 68/68/68/13 & 35/166/50 & 68 & 166 & 18/9 & 5/9 & 3 & 16 \\ 
   & p=500 & 15/9/12 & 55/55/55/12 & 33/147/74 & 55 & 147 & 25/12 & 23/12 & 3 & 19 \\ 
   & p=1000 & 18/9/10 & 45/45/45/10 & 38/132/101 & 45 & 132 & 32/13 & 27/13 & 1 & 20 \\ 
   & p=1500 & 20/13/10 & 41/41/41/10 & 46/126/109 & 41 & 126 & 36/15 & 26/15 & 1 & 18 \\ 
  \midrule\multirow{4}[2]{*}{msnr} & p=250 & 13/19/16 & 76/76/76/16 & 32/69/35 & 76 & 69 & 5/1 & 27/1 & 3 & 7 \\ 
   & p=500 & 15/11/13 & 60/60/60/13 & 21/68/26 & 60 & 68 & 5/1 & 47/1 & 3 & 7 \\ 
   & p=1000 & 17/10/9 & 49/49/49/9 & 14/66/21 & 49 & 66 & 5/1 & 41/1 & 2 & 7 \\ 
   & p=1500 & 18/13/8 & 44/44/44/8 & 12/64/22 & 44 & 64 & 5/1 & 38/1 & 1 & 6 \\ 
  \midrule\multirow{4}[2]{*}{lsnr} & p=250 & 11/9/9 & 156/156/156/9 & 8/9/9 & 156 & 9 & -3/0 & 112/0 & 2 & 3 \\ 
   & p=500 & 16/7/8 & 150/150/150/8 & 6/6/6 & 150 & 6 & -2/1 & 143/1 & 3 & 3 \\ 
   & p=1000 & 26/11/7 & 145/145/145/7 & 4/4/4 & 145 & 4 & -2/2 & 141/2 & 4 & 5 \\ 
   & p=1500 & 35/21/6 & 143/143/143/6 & 4/3/3 & 143 & 3 & -2/3 & 140/3 & 4 & 6 \\ 
   \midrule 
 \multicolumn{1}{|c}{} &       & \multicolumn{9}{c|}{Relative efficiency} \\
\midrule\multirow{4}[2]{*}{hsnr} & p=250 & 0.93/0.91/0.91 & 0.62/0.62/0.62/0.91 & 0.76/0.39/0.69 & 0.62 & 0.39 & 0.88/0.95 & 0.99/0.95 & 1 & 0.89 \\ 
   & p=500 & 0.89/0.94/0.91 & 0.66/0.66/0.66/0.92 & 0.77/0.42/0.59 & 0.66 & 0.42 & 0.82/0.92 & 0.84/0.92 & 1 & 0.87 \\ 
   & p=1000 & 0.86/0.93/0.92 & 0.7/0.7/0.7/0.92 & 0.74/0.44/0.5 & 0.7 & 0.44 & 0.76/0.89 & 0.8/0.89 & 1 & 0.85 \\ 
   & p=1500 & 0.84/0.89/0.92 & 0.72/0.72/0.72/0.92 & 0.69/0.45/0.48 & 0.72 & 0.45 & 0.74/0.88 & 0.8/0.88 & 1 & 0.85 \\ 
  \midrule\multirow{4}[2]{*}{msnr} & p=250 & 0.9/0.85/0.87 & 0.57/0.57/0.57/0.87 & 0.77/0.6/0.75 & 0.57 & 0.6 & 0.97/1 & 0.8/1 & 0.98 & 0.95 \\ 
   & p=500 & 0.87/0.9/0.89 & 0.63/0.63/0.63/0.89 & 0.83/0.6/0.8 & 0.63 & 0.6 & 0.96/1 & 0.68/1 & 0.98 & 0.94 \\ 
   & p=1000 & 0.86/0.92/0.92 & 0.68/0.68/0.68/0.92 & 0.88/0.61/0.83 & 0.68 & 0.61 & 0.96/1 & 0.72/1 & 0.99 & 0.95 \\ 
   & p=1500 & 0.86/0.89/0.94 & 0.7/0.7/0.7/0.94 & 0.9/0.62/0.83 & 0.7 & 0.62 & 0.96/1 & 0.73/1 & 1 & 0.96 \\ 
  \midrule\multirow{4}[2]{*}{lsnr} & p=250 & 0.88/0.89/0.89 & 0.38/0.38/0.38/0.89 & 0.9/0.89/0.89 & 0.38 & 0.89 & 1/0.97 & 0.46/0.97 & 0.95 & 0.95 \\ 
   & p=500 & 0.85/0.91/0.91 & 0.39/0.39/0.39/0.9 & 0.92/0.92/0.92 & 0.39 & 0.92 & 1/0.97 & 0.4/0.97 & 0.95 & 0.95 \\ 
   & p=1000 & 0.78/0.88/0.92 & 0.4/0.4/0.4/0.92 & 0.94/0.94/0.94 & 0.4 & 0.94 & 1/0.96 & 0.41/0.96 & 0.95 & 0.93 \\ 
   & p=1500 & 0.73/0.81/0.93 & 0.4/0.4/0.4/0.92 & 0.95/0.95/0.95 & 0.4 & 0.95 & 1/0.95 & 0.41/0.95 & 0.94 & 0.93 \\ 
   \midrule 
 \multicolumn{1}{|c}{} &       & \multicolumn{9}{c|}{Sparsistency} \\
\midrule\multirow{4}[2]{*}{hsnr} & p=250 & 21.3/14.8/16.5 & 199/199/199/16.3 & 11.3/3.1/10.1 & 199 & 3.1 & 47.7/74.1 & 47.2/74.1 & 32.1 & 35.5 \\ 
   & p=500 & 26.8/15.6/14.8 & 199/199/199/14.5 & 10.7/3/7.8 & 199 & 3 & 47.2/87.8 & 80.7/87.8 & 30.9 & 34.5 \\ 
   & p=1000 & 29.9/19.2/13.7 & 199/199/199/13.6 & 9.6/3/5.1 & 199 & 3 & 45.9/99 & 96.1/99 & 27.7 & 34 \\ 
   & p=1500 & 29.3/23.6/13.5 & 199/199/199/13.3 & 8.8/3/4.1 & 198.9 & 3 & 45.4/106.3 & 98/106.3 & 27.1 & 36.8 \\ 
  \midrule\multirow{4}[2]{*}{msnr} & p=250 & 12/5.9/7.9 & 199/199/199/7.6 & 3.2/1.5/3 & 199 & 1.5 & 32.7/49.7 & 57.8/49.7 & 27.7 & 27.8 \\ 
   & p=500 & 16.3/6.4/5.7 & 199/199/199/5.6 & 3.1/0.8/2.7 & 199 & 0.8 & 30.5/54.7 & 103.2/54.7 & 26.2 & 25.8 \\ 
   & p=1000 & 18.6/9.8/4.4 & 199/199/199/4.4 & 2.9/0.3/2.5 & 199 & 0.3 & 27.7/57.1 & 106.3/57.1 & 22.8 & 20.7 \\ 
   & p=1500 & 19.6/13.9/3.9 & 199/199/199/3.9 & 2.9/0.2/2.3 & 198.9 & 0.2 & 27.2/59 & 106.4/59 & 20.7 & 19.8 \\ 
  \midrule\multirow{4}[2]{*}{lsnr} & p=250 & 1.1/0.3/1.1 & 199/199/199/1.1 & 0.2/0/0.1 & 199 & 0 & 11.1/14.7 & 72.2/14.7 & 11.3 & 9.5 \\ 
   & p=500 & 2.6/0.4/0.8 & 199/199/199/0.8 & 0.1/0/0.1 & 199 & 0 & 11.1/14.8 & 117.1/14.8 & 12.5 & 9.1 \\ 
   & p=1000 & 5/1.5/0.6 & 199/199/199/0.6 & 0.1/0/0 & 199 & 0 & 10.6/16.6 & 114.9/16.6 & 12.5 & 10.5 \\ 
   & p=1500 & 6.5/3.4/0.5 & 199/199/199/0.5 & 0.1/0/0 & 198.9 & 0 & 10/17.6 & 113.5/17.6 & 12.8 & 11.8 \\ 
   \midrule 
 \multicolumn{1}{|c}{} &       & \multicolumn{9}{c|}{Number of extra variables} \\
\midrule\multirow{4}[2]{*}{hsnr} & p=250 & -/-/- & -/-/-/- & -/-/- & - & - & -/- & -/- & - & - \\ 
   & p=500 & -/-/- & -/-/-/- & -/-/- & - & - & -/- & -/- & - & - \\ 
   & p=1000 & -/-/- & -/-/-/- & -/-/- & - & - & -/- & -/- & - & - \\ 
   & p=1500 & -/-/- & -/-/-/- & -/-/- & - & - & -/- & -/- & - & - \\ 
  \midrule\multirow{4}[2]{*}{msnr} & p=250 & -/-/- & -/-/-/- & -/-/- & - & - & -/- & -/- & - & - \\ 
   & p=500 & -/-/- & -/-/-/- & -/-/- & - & - & -/- & -/- & - & - \\ 
   & p=1000 & -/-/- & -/-/-/- & -/-/- & - & - & -/- & -/- & - & - \\ 
   & p=1500 & -/-/- & -/-/-/- & -/-/- & - & - & -/- & -/- & - & - \\ 
  \midrule\multirow{4}[2]{*}{lsnr} & p=250 & -/-/- & -/-/-/- & -/-/- & - & - & -/- & -/- & - & - \\ 
   & p=500 & -/-/- & -/-/-/- & -/-/- & - & - & -/- & -/- & - & - \\ 
   & p=1000 & -/-/- & -/-/-/- & -/-/- & - & - & -/- & -/- & - & - \\ 
   & p=1500 & -/-/- & -/-/-/- & -/-/- & - & - & -/- & -/- & - & - \\ 
   \bottomrule 
\end{tabular}
}
\end{table}
