# Supplementary material for: On the Use of Information Criteria for Subset Selection in Least Squares Regression
Source: arXiv:1911.10191 source file (2021-03-06)
Supplement: Supplementary file 32 [file Dense_rho_05.tex]

% latex table generated in R 4.0.3 by xtable 1.8-4 package
% Sun Feb 21 09:16:36 2021
\begin{table}[ht]
\centering
\caption{The performance of BOSS for high dimensional data, Dense, $\rho$=0.5, n=200} 
\scalebox{0.55}{
\begin{tabular}{|c|c|ccccccccc|}
  \toprule 
 \multicolumn{1}{|c}{} &       & BOSS  & FS    & FSstop & FStrim & FSstoptrim & lasso & Gamma lasso & SparseNet & rlasso \\
 \multicolumn{1}{|c}{} &       & C$_p$/AICc/CV & EBIC/HDBIC/HDHQ/CV & EBIC/HDBIC/HDHQ & HDBIC & HDBIC & AICc/CV & AICc/CV & CV    & CV  \\
 \cmidrule{3-11}\multicolumn{1}{|c}{} &       & \multicolumn{9}{c|}{\% worse than the best possible BOSS}  \\
 \midrule\multirow{4}[2]{*}{hsnr} & p=250 & 9/11/11 & 62/62/62/13 & 34/147/59 & 62 & 147 & 44/23 & 6/23 & 5 & 27 \\ 
   & p=500 & 10/7/13 & 47/47/47/14 & 45/127/87 & 47 & 127 & 71/29 & 9/29 & 1 & 45 \\ 
   & p=1000 & 15/10/24 & 32/32/32/28 & 51/104/89 & 32 & 104 & 100/52 & 11/52 & 3 & 90 \\ 
   & p=1500 & 18/13/35 & 21/21/21/38 & 53/88/79 & 21 & 88 & 89/57 & 8/57 & 21 & 79 \\ 
  \midrule\multirow{4}[2]{*}{msnr} & p=250 & 13/14/13 & 66/66/66/15 & 19/49/21 & 66 & 49 & 24/17 & 15/17 & 10 & 20 \\ 
   & p=500 & 8/6/8 & 52/52/52/8 & 10/54/13 & 52 & 54 & 21/15 & 32/15 & 6 & 16 \\ 
   & p=1000 & 10/5/5 & 46/46/46/5 & 7/61/11 & 46 & 61 & 22/15 & 34/15 & 3 & 18 \\ 
   & p=1500 & 12/8/4 & 44/44/44/4 & 6/63/13 & 44 & 63 & 24/17 & 34/17 & 2 & 21 \\ 
  \midrule\multirow{4}[2]{*}{lsnr} & p=250 & 10/9/10 & 156/156/156/11 & 9/10/9 & 156 & 10 & 4/6 & 99/6 & 7 & 8 \\ 
   & p=500 & 10/6/7 & 147/147/147/7 & 5/5/5 & 147 & 5 & 2/3 & 135/3 & 5 & 5 \\ 
   & p=1000 & 17/6/6 & 142/142/142/6 & 4/3/4 & 142 & 3 & 1/2 & 135/2 & 4 & 5 \\ 
   & p=1500 & 24/12/5 & 140/140/140/6 & 3/2/2 & 140 & 2 & 0/2 & 134/2 & 4 & 4 \\ 
   \midrule 
 \multicolumn{1}{|c}{} &       & \multicolumn{9}{c|}{Relative efficiency} \\
\midrule\multirow{4}[2]{*}{hsnr} & p=250 & 0.96/0.95/0.95 & 0.65/0.65/0.65/0.93 & 0.78/0.43/0.66 & 0.65 & 0.43 & 0.73/0.86 & 0.99/0.86 & 1 & 0.83 \\ 
   & p=500 & 0.92/0.94/0.89 & 0.69/0.69/0.69/0.88 & 0.7/0.44/0.54 & 0.69 & 0.44 & 0.59/0.78 & 0.92/0.78 & 1 & 0.69 \\ 
   & p=1000 & 0.9/0.94/0.83 & 0.78/0.78/0.78/0.81 & 0.68/0.51/0.55 & 0.78 & 0.51 & 0.52/0.68 & 0.93/0.68 & 1 & 0.54 \\ 
   & p=1500 & 0.92/0.96/0.8 & 0.89/0.89/0.89/0.79 & 0.71/0.58/0.6 & 0.89 & 0.58 & 0.57/0.69 & 1/0.69 & 0.89 & 0.61 \\ 
  \midrule\multirow{4}[2]{*}{msnr} & p=250 & 0.98/0.96/0.98 & 0.66/0.66/0.66/0.96 & 0.92/0.74/0.91 & 0.66 & 0.74 & 0.89/0.94 & 0.96/0.94 & 1 & 0.92 \\ 
   & p=500 & 0.98/0.99/0.98 & 0.7/0.7/0.7/0.98 & 0.96/0.69/0.94 & 0.7 & 0.69 & 0.88/0.92 & 0.8/0.92 & 1 & 0.91 \\ 
   & p=1000 & 0.94/0.98/0.98 & 0.71/0.71/0.71/0.99 & 0.97/0.64/0.93 & 0.71 & 0.64 & 0.85/0.89 & 0.77/0.89 & 1 & 0.88 \\ 
   & p=1500 & 0.91/0.94/0.98 & 0.71/0.71/0.71/0.98 & 0.96/0.63/0.9 & 0.71 & 0.63 & 0.82/0.87 & 0.76/0.87 & 1 & 0.84 \\ 
  \midrule\multirow{4}[2]{*}{lsnr} & p=250 & 0.95/0.96/0.95 & 0.41/0.41/0.41/0.94 & 0.96/0.95/0.95 & 0.41 & 0.95 & 1/0.99 & 0.52/0.99 & 0.98 & 0.97 \\ 
   & p=500 & 0.92/0.96/0.95 & 0.41/0.41/0.41/0.95 & 0.97/0.96/0.96 & 0.41 & 0.96 & 1/0.99 & 0.43/0.99 & 0.97 & 0.97 \\ 
   & p=1000 & 0.86/0.95/0.95 & 0.42/0.42/0.42/0.95 & 0.97/0.97/0.97 & 0.42 & 0.97 & 1/0.98 & 0.43/0.98 & 0.97 & 0.96 \\ 
   & p=1500 & 0.81/0.89/0.95 & 0.42/0.42/0.42/0.95 & 0.97/0.98/0.97 & 0.42 & 0.98 & 1/0.98 & 0.43/0.98 & 0.96 & 0.96 \\ 
   \midrule 
 \multicolumn{1}{|c}{} &       & \multicolumn{9}{c|}{Sparsistency} \\
\midrule\multirow{4}[2]{*}{hsnr} & p=250 & 21.5/15.1/17.4 & 199/199/199/16.5 & 10.9/3.2/9 & 199 & 3.2 & 58.7/96.1 & 44.4/96.1 & 27.1 & 63 \\ 
   & p=500 & 22.6/15.5/15.7 & 199/199/199/15.6 & 9.1/3.1/5.8 & 199 & 3.1 & 52.3/106.6 & 63/106.6 & 30.3 & 66.7 \\ 
   & p=1000 & 20.8/15.7/12.5 & 199/199/199/11.5 & 7.3/3/4.1 & 199 & 3 & 30.2/92.9 & 87/92.9 & 38.3 & 19.8 \\ 
   & p=1500 & 16.1/16.1/9.8 & 199/199/199/8.6 & 6/3/3.6 & 198.9 & 3 & 29.4/71.9 & 94.5/71.9 & 28.8 & 11 \\ 
  \midrule\multirow{4}[2]{*}{msnr} & p=250 & 9.2/5/6.6 & 199/199/199/5.2 & 3.2/1.8/3.1 & 199 & 1.8 & 28.2/49 & 52.3/49 & 15.2 & 25 \\ 
   & p=500 & 7.7/4.8/4.4 & 199/199/199/4.1 & 3.1/1.1/2.9 & 199 & 1.1 & 26.1/43.2 & 93.3/43.2 & 10.4 & 18.5 \\ 
   & p=1000 & 10.2/5.4/3.8 & 199/199/199/3.8 & 3/0.4/2.8 & 199 & 0.4 & 25.9/47 & 103.5/47 & 9.2 & 21.1 \\ 
   & p=1500 & 11.1/8/3.7 & 199/199/199/3.7 & 3/0.3/2.6 & 198.9 & 0.3 & 24.9/48.7 & 103.2/48.7 & 10.1 & 22.5 \\ 
  \midrule\multirow{4}[2]{*}{lsnr} & p=250 & 0.6/0.2/1.1 & 199/199/199/0.9 & 0.1/0/0.1 & 199 & 0 & 8.3/9.2 & 65.2/9.2 & 7.2 & 6.2 \\ 
   & p=500 & 1.4/0.2/0.7 & 199/199/199/0.6 & 0.1/0/0 & 199 & 0 & 8.1/9.6 & 112.3/9.6 & 7.7 & 5.8 \\ 
   & p=1000 & 3.3/0.6/0.5 & 199/199/199/0.5 & 0.1/0/0 & 199 & 0 & 8/10.1 & 112.4/10.1 & 8.4 & 7.2 \\ 
   & p=1500 & 4.2/1.6/0.4 & 199/199/199/0.4 & 0/0/0 & 198.9 & 0 & 8.1/10.6 & 110.5/10.6 & 9.3 & 7.2 \\ 
   \midrule 
 \multicolumn{1}{|c}{} &       & \multicolumn{9}{c|}{Number of extra variables} \\
\midrule\multirow{4}[2]{*}{hsnr} & p=250 & -/-/- & -/-/-/- & -/-/- & - & - & -/- & -/- & - & - \\ 
   & p=500 & -/-/- & -/-/-/- & -/-/- & - & - & -/- & -/- & - & - \\ 
   & p=1000 & -/-/- & -/-/-/- & -/-/- & - & - & -/- & -/- & - & - \\ 
   & p=1500 & -/-/- & -/-/-/- & -/-/- & - & - & -/- & -/- & - & - \\ 
  \midrule\multirow{4}[2]{*}{msnr} & p=250 & -/-/- & -/-/-/- & -/-/- & - & - & -/- & -/- & - & - \\ 
   & p=500 & -/-/- & -/-/-/- & -/-/- & - & - & -/- & -/- & - & - \\ 
   & p=1000 & -/-/- & -/-/-/- & -/-/- & - & - & -/- & -/- & - & - \\ 
   & p=1500 & -/-/- & -/-/-/- & -/-/- & - & - & -/- & -/- & - & - \\ 
  \midrule\multirow{4}[2]{*}{lsnr} & p=250 & -/-/- & -/-/-/- & -/-/- & - & - & -/- & -/- & - & - \\ 
   & p=500 & -/-/- & -/-/-/- & -/-/- & - & - & -/- & -/- & - & - \\ 
   & p=1000 & -/-/- & -/-/-/- & -/-/- & - & - & -/- & -/- & - & - \\ 
   & p=1500 & -/-/- & -/-/-/- & -/-/- & - & - & -/- & -/- & - & - \\ 
   \bottomrule 
\end{tabular}
}
\end{table}
