# Supplementary material for: On the Use of Information Criteria for Subset Selection in Least Squares Regression
Source: arXiv:1911.10191 source file (2021-03-06)
Supplement: Supplementary file 33 [file Dense_rho_09.tex]

% latex table generated in R 4.0.3 by xtable 1.8-4 package
% Sun Feb 21 09:18:22 2021
\begin{table}[ht]
\centering
\caption{The performance of BOSS for high dimensional data, Dense, $\rho$=0.9, n=200} 
\scalebox{0.55}{
\begin{tabular}{|c|c|ccccccccc|}
  \toprule 
 \multicolumn{1}{|c}{} &       & BOSS  & FS    & FSstop & FStrim & FSstoptrim & lasso & Gamma lasso & SparseNet & rlasso \\
 \multicolumn{1}{|c}{} &       & C$_p$/AICc/CV & EBIC/HDBIC/HDHQ/CV & EBIC/HDBIC/HDHQ & HDBIC & HDBIC & AICc/CV & AICc/CV & CV    & CV  \\
 \cmidrule{3-11}\multicolumn{1}{|c}{} &       & \multicolumn{9}{c|}{\% worse than the best possible BOSS}  \\
 \midrule\multirow{4}[2]{*}{hsnr} & p=250 & 10/21/12 & 79/79/79/12 & 68/113/90 & 79 & 113 & 75/39 & 19/39 & 14 & 42 \\ 
   & p=500 & 27/24/18 & 61/61/61/21 & 68/95/82 & 61 & 95 & 113/71 & 32/71 & 52 & 80 \\ 
   & p=1000 & 45/21/26 & 37/37/37/29 & 51/67/58 & 37 & 67 & 129/123 & 30/123 & 55 & 125 \\ 
   & p=1500 & 34/17/25 & 22/22/22/26 & 37/51/42 & 22 & 51 & 101/103 & 17/103 & 36 & 106 \\ 
  \midrule\multirow{4}[2]{*}{msnr} & p=250 & 14/13/9 & 94/94/94/9 & 17/49/23 & 94 & 49 & 46/43 & 33/43 & 15 & 46 \\ 
   & p=500 & 10/9/7 & 85/85/85/7 & 15/46/22 & 85 & 46 & 49/50 & 49/50 & 18 & 48 \\ 
   & p=1000 & 8/7/7 & 79/79/79/7 & 15/43/25 & 79 & 43 & 45/46 & 53/46 & 25 & 44 \\ 
   & p=1500 & 7/7/7 & 76/76/76/7 & 15/41/26 & 76 & 41 & 41/42 & 55/42 & 33 & 41 \\ 
  \midrule\multirow{4}[2]{*}{lsnr} & p=250 & 15/16/11 & 227/227/227/11 & 15/38/20 & 227 & 38 & 14/14 & 143/14 & 10 & 11 \\ 
   & p=500 & 15/15/11 & 220/220/220/11 & 15/37/22 & 220 & 37 & 13/13 & 200/13 & 9 & 10 \\ 
   & p=1000 & 19/15/12 & 213/213/213/12 & 16/36/24 & 213 & 36 & 12/13 & 198/13 & 9 & 10 \\ 
   & p=1500 & 24/17/13 & 209/209/209/13 & 17/34/24 & 209 & 34 & 12/14 & 194/14 & 10 & 10 \\ 
   \midrule 
 \multicolumn{1}{|c}{} &       & \multicolumn{9}{c|}{Relative efficiency} \\
\midrule\multirow{4}[2]{*}{hsnr} & p=250 & 1/0.91/0.99 & 0.62/0.62/0.62/0.99 & 0.66/0.52/0.58 & 0.62 & 0.52 & 0.63/0.8 & 0.92/0.8 & 0.97 & 0.78 \\ 
   & p=500 & 0.93/0.95/1 & 0.73/0.73/0.73/0.98 & 0.71/0.61/0.65 & 0.73 & 0.61 & 0.56/0.69 & 0.9/0.69 & 0.78 & 0.66 \\ 
   & p=1000 & 0.83/1/0.97 & 0.89/0.89/0.89/0.94 & 0.8/0.73/0.77 & 0.89 & 0.73 & 0.53/0.54 & 0.93/0.54 & 0.78 & 0.54 \\ 
   & p=1500 & 0.87/1/0.94 & 0.96/0.96/0.96/0.93 & 0.85/0.77/0.82 & 0.96 & 0.77 & 0.58/0.58 & 1/0.58 & 0.86 & 0.57 \\ 
  \midrule\multirow{4}[2]{*}{msnr} & p=250 & 0.96/0.96/1 & 0.56/0.56/0.56/1 & 0.93/0.73/0.89 & 0.56 & 0.73 & 0.75/0.76 & 0.82/0.76 & 0.95 & 0.75 \\ 
   & p=500 & 0.97/0.98/1 & 0.58/0.58/0.58/1 & 0.93/0.73/0.87 & 0.58 & 0.73 & 0.71/0.71 & 0.72/0.71 & 0.91 & 0.72 \\ 
   & p=1000 & 0.99/1/1 & 0.6/0.6/0.6/1 & 0.93/0.75/0.85 & 0.6 & 0.75 & 0.74/0.73 & 0.7/0.73 & 0.86 & 0.74 \\ 
   & p=1500 & 1/1/1 & 0.61/0.61/0.61/1 & 0.93/0.76/0.85 & 0.61 & 0.76 & 0.76/0.75 & 0.69/0.75 & 0.81 & 0.76 \\ 
  \midrule\multirow{4}[2]{*}{lsnr} & p=250 & 0.96/0.95/0.99 & 0.34/0.34/0.34/0.99 & 0.96/0.8/0.92 & 0.34 & 0.8 & 0.97/0.97 & 0.45/0.97 & 1 & 1 \\ 
   & p=500 & 0.95/0.95/0.98 & 0.34/0.34/0.34/0.99 & 0.95/0.8/0.89 & 0.34 & 0.8 & 0.97/0.96 & 0.36/0.96 & 1 & 0.99 \\ 
   & p=1000 & 0.92/0.95/0.98 & 0.35/0.35/0.35/0.98 & 0.94/0.81/0.89 & 0.35 & 0.81 & 0.97/0.96 & 0.37/0.96 & 1 & 0.99 \\ 
   & p=1500 & 0.88/0.94/0.97 & 0.35/0.35/0.35/0.98 & 0.94/0.82/0.88 & 0.35 & 0.82 & 0.98/0.97 & 0.37/0.97 & 1 & 1 \\ 
   \midrule 
 \multicolumn{1}{|c}{} &       & \multicolumn{9}{c|}{Sparsistency} \\
\midrule\multirow{4}[2]{*}{hsnr} & p=250 & 17.2/13.2/19.3 & 199/199/199/16.3 & 6.4/3.2/4.7 & 199 & 3.2 & 55.8/93.9 & 49.7/93.9 & 42.5 & 77.7 \\ 
   & p=500 & 13.1/11.7/16.3 & 199/199/199/13.6 & 5/3.1/3.8 & 199 & 3.1 & 38.3/79.6 & 71.1/79.6 & 36.1 & 55.5 \\ 
   & p=1000 & 6.6/9.7/10.4 & 199/199/199/8 & 4.2/3/3.6 & 199 & 3 & 9.8/19.2 & 62.7/19.2 & 15.1 & 9.2 \\ 
   & p=1500 & 4.9/7.9/6.9 & 199/199/199/5.8 & 3.9/2.9/3.5 & 199 & 2.9 & 12.5/12.6 & 63.7/12.6 & 20.8 & 3.2 \\ 
  \midrule\multirow{4}[2]{*}{msnr} & p=250 & 5.1/3.8/6.7 & 199/199/199/4.6 & 2.8/1.3/2.5 & 199 & 1.3 & 17/28.6 & 52.8/28.6 & 14.9 & 17.2 \\ 
   & p=500 & 3.6/3.6/4.6 & 199/199/199/4 & 2.7/1.1/2.3 & 199 & 1.1 & 7.4/8.9 & 82/8.9 & 16.8 & 3.5 \\ 
   & p=1000 & 3.6/3.6/3.8 & 199/199/199/3.6 & 2.5/1/1.9 & 199 & 1 & 8.3/8.3 & 93.8/8.3 & 17.8 & 2.3 \\ 
   & p=1500 & 3.9/3.9/3.6 & 199/199/199/3.5 & 2.4/1/1.8 & 199 & 1 & 10.4/10.5 & 97.2/10.5 & 11.8 & 2.6 \\ 
  \midrule\multirow{4}[2]{*}{lsnr} & p=250 & 0.9/0.8/2 & 199/199/199/1.6 & 0.7/0.1/0.6 & 199 & 0.1 & 6.6/6.8 & 64.6/6.8 & 3.8 & 3.1 \\ 
   & p=500 & 1/0.8/1.5 & 199/199/199/1.3 & 0.6/0.1/0.4 & 199 & 0.1 & 7.5/7.3 & 112.2/7.3 & 3.9 & 3.2 \\ 
   & p=1000 & 1.5/0.9/1.2 & 199/199/199/1.2 & 0.5/0/0.3 & 199 & 0 & 9.1/9.2 & 115.1/9.2 & 4.9 & 3.9 \\ 
   & p=1500 & 2.2/1/1.1 & 199/199/199/1.1 & 0.5/0/0.3 & 199 & 0 & 9.3/10.3 & 112.6/10.3 & 5.6 & 4.7 \\ 
   \midrule 
 \multicolumn{1}{|c}{} &       & \multicolumn{9}{c|}{Number of extra variables} \\
\midrule\multirow{4}[2]{*}{hsnr} & p=250 & -/-/- & -/-/-/- & -/-/- & - & - & -/- & -/- & - & - \\ 
   & p=500 & -/-/- & -/-/-/- & -/-/- & - & - & -/- & -/- & - & - \\ 
   & p=1000 & -/-/- & -/-/-/- & -/-/- & - & - & -/- & -/- & - & - \\ 
   & p=1500 & -/-/- & -/-/-/- & -/-/- & - & - & -/- & -/- & - & - \\ 
  \midrule\multirow{4}[2]{*}{msnr} & p=250 & -/-/- & -/-/-/- & -/-/- & - & - & -/- & -/- & - & - \\ 
   & p=500 & -/-/- & -/-/-/- & -/-/- & - & - & -/- & -/- & - & - \\ 
   & p=1000 & -/-/- & -/-/-/- & -/-/- & - & - & -/- & -/- & - & - \\ 
   & p=1500 & -/-/- & -/-/-/- & -/-/- & - & - & -/- & -/- & - & - \\ 
  \midrule\multirow{4}[2]{*}{lsnr} & p=250 & -/-/- & -/-/-/- & -/-/- & - & - & -/- & -/- & - & - \\ 
   & p=500 & -/-/- & -/-/-/- & -/-/- & - & - & -/- & -/- & - & - \\ 
   & p=1000 & -/-/- & -/-/-/- & -/-/- & - & - & -/- & -/- & - & - \\ 
   & p=1500 & -/-/- & -/-/-/- & -/-/- & - & - & -/- & -/- & - & - \\ 
   \bottomrule 
\end{tabular}
}
\end{table}
