# Supplementary material for: On the Use of Information Criteria for Subset Selection in Least Squares Regression
Source: arXiv:1911.10191 source file (2021-03-06)
Supplement: Supplementary file 34 [file Sparse-Ex1_rho_0.tex]

% latex table generated in R 4.0.3 by xtable 1.8-4 package
% Sun Feb 21 09:00:00 2021
\begin{table}[ht]
\centering
\caption{The performance of BOSS for high dimensional data, Sparse-Ex1, $\rho$=0, n=200} 
\scalebox{0.55}{
\begin{tabular}{|c|c|ccccccccc|}
  \toprule 
 \multicolumn{1}{|c}{} &       & BOSS  & FS    & FSstop & FStrim & FSstoptrim & lasso & Gamma lasso & SparseNet & rlasso \\
 \multicolumn{1}{|c}{} &       & C$_p$/AICc/CV & EBIC/HDBIC/HDHQ/CV & EBIC/HDBIC/HDHQ & HDBIC & HDBIC & AICc/CV & AICc/CV & CV    & CV  \\
 \cmidrule{3-11}\multicolumn{1}{|c}{} &       & \multicolumn{9}{c|}{\% worse than the best possible BOSS}  \\
 \midrule\multirow{4}[2]{*}{hsnr} & p=250 & 6/1/17 & 502/502/502/18 & 1/0/1 & 502 & 0 & 141/142 & 183/142 & 17 & 16 \\ 
   & p=500 & 26/3/18 & 511/511/511/19 & 2/0/1 & 511 & 0 & 163/165 & 368/165 & 24 & 18 \\ 
   & p=1000 & 86/13/21 & 512/512/512/22 & 2/0/0 & 512 & 0 & 184/192 & 424/192 & 27 & 17 \\ 
   & p=1500 & 122/44/19 & 505/505/505/21 & 2/0/0 & 505 & 0 & 206/209 & 433/209 & 26 & 15 \\ 
  \midrule\multirow{4}[2]{*}{msnr} & p=250 & 23/12/18 & 501/501/501/19 & 4/269/6 & 501 & 269 & 140/141 & 313/141 & 18 & 28 \\ 
   & p=500 & 61/24/19 & 508/508/508/21 & 6/415/18 & 508 & 416 & 161/164 & 459/164 & 25 & 28 \\ 
   & p=1000 & 135/56/23 & 511/511/511/24 & 7/571/18 & 511 & 571 & 184/191 & 478/191 & 27 & 34 \\ 
   & p=1500 & 190/128/23 & 499/499/499/25 & 10/604/53 & 499 & 604 & 202/206 & 472/206 & 26 & 63 \\ 
  \midrule\multirow{4}[2]{*}{lsnr} & p=250 & 16/15/13 & 166/166/166/13 & 15/16/15 & 166 & 16 & -3/0 & 122/0 & 3 & 3 \\ 
   & p=500 & 22/12/12 & 149/149/149/12 & 12/12/12 & 149 & 12 & -3/0 & 143/0 & 3 & 3 \\ 
   & p=1000 & 33/16/9 & 136/136/136/9 & 9/9/9 & 136 & 9 & -3/2 & 133/2 & 3 & 4 \\ 
   & p=1500 & 34/20/6 & 138/138/138/6 & 3/3/3 & 138 & 3 & -3/1 & 135/1 & 3 & 5 \\ 
   \midrule 
 \multicolumn{1}{|c}{} &       & \multicolumn{9}{c|}{Relative efficiency} \\
\midrule\multirow{4}[2]{*}{hsnr} & p=250 & 0.95/0.99/0.86 & 0.17/0.17/0.17/0.85 & 0.99/1/0.99 & 0.17 & 1 & 0.42/0.41 & 0.35/0.41 & 0.85 & 0.87 \\ 
   & p=500 & 0.79/0.98/0.85 & 0.16/0.16/0.16/0.84 & 0.98/1/0.99 & 0.16 & 1 & 0.38/0.38 & 0.21/0.38 & 0.81 & 0.85 \\ 
   & p=1000 & 0.54/0.89/0.83 & 0.16/0.16/0.16/0.82 & 0.98/1/1 & 0.16 & 1 & 0.35/0.34 & 0.19/0.34 & 0.79 & 0.86 \\ 
   & p=1500 & 0.45/0.7/0.84 & 0.17/0.17/0.17/0.82 & 0.98/1/1 & 0.17 & 1 & 0.33/0.32 & 0.19/0.32 & 0.79 & 0.87 \\ 
  \midrule\multirow{4}[2]{*}{msnr} & p=250 & 0.84/0.93/0.88 & 0.17/0.17/0.17/0.87 & 1/0.28/0.98 & 0.17 & 0.28 & 0.43/0.43 & 0.25/0.43 & 0.88 & 0.81 \\ 
   & p=500 & 0.66/0.85/0.89 & 0.17/0.17/0.17/0.88 & 1/0.21/0.9 & 0.17 & 0.21 & 0.41/0.4 & 0.19/0.4 & 0.85 & 0.83 \\ 
   & p=1000 & 0.46/0.69/0.87 & 0.18/0.18/0.18/0.86 & 1/0.16/0.91 & 0.18 & 0.16 & 0.38/0.37 & 0.18/0.37 & 0.84 & 0.8 \\ 
   & p=1500 & 0.38/0.48/0.89 & 0.18/0.18/0.18/0.88 & 1/0.16/0.72 & 0.18 & 0.16 & 0.36/0.36 & 0.19/0.36 & 0.87 & 0.68 \\ 
  \midrule\multirow{4}[2]{*}{lsnr} & p=250 & 0.84/0.85/0.86 & 0.37/0.37/0.37/0.86 & 0.85/0.84/0.84 & 0.37 & 0.84 & 1/0.97 & 0.44/0.97 & 0.94 & 0.94 \\ 
   & p=500 & 0.79/0.87/0.87 & 0.39/0.39/0.39/0.87 & 0.87/0.86/0.86 & 0.39 & 0.86 & 1/0.97 & 0.4/0.97 & 0.94 & 0.94 \\ 
   & p=1000 & 0.73/0.84/0.89 & 0.41/0.41/0.41/0.89 & 0.89/0.89/0.89 & 0.41 & 0.89 & 1/0.95 & 0.42/0.95 & 0.94 & 0.93 \\ 
   & p=1500 & 0.73/0.81/0.92 & 0.41/0.41/0.41/0.92 & 0.94/0.95/0.95 & 0.41 & 0.95 & 1/0.96 & 0.41/0.96 & 0.94 & 0.93 \\ 
   \midrule 
 \multicolumn{1}{|c}{} &       & \multicolumn{9}{c|}{Sparsistency} \\
\midrule\multirow{4}[2]{*}{hsnr} & p=250 & 6/6/6 & 6/6/6/6 & 6/6/6 & 6 & 6 & 6/6 & 6/6 & 6 & 6 \\ 
   & p=500 & 6/6/6 & 6/6/6/6 & 6/6/6 & 6 & 6 & 6/6 & 6/6 & 6 & 6 \\ 
   & p=1000 & 6/6/6 & 6/6/6/6 & 6/6/6 & 6 & 6 & 6/6 & 6/6 & 6 & 6 \\ 
   & p=1500 & 6/6/6 & 6/6/6/6 & 6/6/6 & 6 & 6 & 6/6 & 6/6 & 6 & 6 \\ 
  \midrule\multirow{4}[2]{*}{msnr} & p=250 & 6/6/6 & 6/6/6/6 & 6/3.6/6 & 6 & 3.6 & 6/6 & 6/6 & 6 & 6 \\ 
   & p=500 & 6/6/6 & 6/6/6/6 & 6/2.4/5.9 & 6 & 2.4 & 6/6 & 6/6 & 6 & 6 \\ 
   & p=1000 & 6/6/6 & 6/6/6/6 & 6/1.1/5.9 & 6 & 1.1 & 6/6 & 6/6 & 6 & 6 \\ 
   & p=1500 & 6/6/6 & 6/6/6/6 & 5.9/0.1/5.6 & 6 & 0.1 & 6/6 & 6/6 & 6 & 5.9 \\ 
  \midrule\multirow{4}[2]{*}{lsnr} & p=250 & 0.8/0.4/1.1 & 5.6/5.6/5.6/1.1 & 0.3/0/0.1 & 5.6 & 0 & 3.3/3.3 & 4.6/3.3 & 2.9 & 2.6 \\ 
   & p=500 & 1.1/0.4/0.8 & 4.3/4.3/4.3/0.8 & 0.2/0/0.1 & 4.3 & 0 & 3/3 & 3.9/3 & 2.6 & 2.4 \\ 
   & p=1000 & 1.3/0.7/0.6 & 3.2/3.2/3.2/0.6 & 0.1/0/0 & 3.2 & 0 & 2.5/2.6 & 3.2/2.6 & 2.2 & 2.1 \\ 
   & p=1500 & 0.8/0.5/0.3 & 2.3/2.3/2.3/0.3 & 0.1/0/0 & 2.3 & 0 & 1.5/1.6 & 2.4/1.6 & 1.4 & 1.3 \\ 
   \midrule 
 \multicolumn{1}{|c}{} &       & \multicolumn{9}{c|}{Number of extra variables} \\
\midrule\multirow{4}[2]{*}{hsnr} & p=250 & 0.2/0/0.3 & 193/193/193/0.3 & 0/0/0 & 193 & 0 & 16.8/24.2 & 27.7/24.2 & 2.4 & 0.5 \\ 
   & p=500 & 1.4/0/0.2 & 193/193/193/0.3 & 0/0/0 & 193 & 0 & 18.1/29.6 & 73.7/29.6 & 3.7 & 0.8 \\ 
   & p=1000 & 4.8/0.5/0.3 & 193/193/193/0.3 & 0/0/0 & 193 & 0 & 18.9/37.9 & 87/37.9 & 4.7 & 0.6 \\ 
   & p=1500 & 6.4/2.1/0.2 & 193/193/193/0.3 & 0/0/0 & 192.9 & 0 & 21.4/43.8 & 89.7/43.8 & 5.1 & 0.5 \\ 
  \midrule\multirow{4}[2]{*}{msnr} & p=250 & 0.5/0.2/0.3 & 193/193/193/0.3 & 0/0/0 & 193 & 0 & 16.9/24.2 & 49.6/24.2 & 1.4 & 1 \\ 
   & p=500 & 2/0.3/0.3 & 193/193/193/0.3 & 0/0/0 & 193 & 0 & 18.2/29.6 & 97.9/29.6 & 2.3 & 1.2 \\ 
   & p=1000 & 5.7/1.1/0.3 & 193/193/193/0.3 & 0/0/0 & 193 & 0 & 19.2/37.9 & 99.9/37.9 & 2.5 & 1.3 \\ 
   & p=1500 & 8.1/4/0.3 & 193/193/193/0.3 & 0/0/0 & 192.9 & 0 & 21.3/44.1 & 99/44.1 & 2.6 & 2.5 \\ 
  \midrule\multirow{4}[2]{*}{lsnr} & p=250 & 0.7/0.1/0.5 & 193.4/193.4/193.4/0.5 & 0/0/0 & 193.4 & 0 & 10.1/13.1 & 70/13.1 & 9.6 & 7.2 \\ 
   & p=500 & 2.8/0.2/0.5 & 194.7/194.7/194.7/0.4 & 0/0/0 & 194.7 & 0 & 11.3/15.9 & 113.7/15.9 & 12.4 & 8.9 \\ 
   & p=1000 & 5.8/1.5/0.4 & 195.8/195.8/195.8/0.3 & 0/0/0 & 195.8 & 0 & 10.7/20 & 113/20 & 14.1 & 11.5 \\ 
   & p=1500 & 6.1/3.2/0.3 & 196.7/196.7/196.7/0.3 & 0/0/0 & 196.6 & 0 & 9.5/15.6 & 111.9/15.6 & 12.8 & 10.7 \\ 
   \bottomrule 
\end{tabular}
}
\end{table}
