# Supplementary material for: On the Use of Information Criteria for Subset Selection in Least Squares Regression
Source: arXiv:1911.10191 source file (2021-03-06)
Supplement: Supplementary file 35 [file Sparse-Ex1_rho_05.tex]

% latex table generated in R 4.0.3 by xtable 1.8-4 package
% Sun Feb 21 09:01:57 2021
\begin{table}[ht]
\centering
\caption{The performance of BOSS for high dimensional data, Sparse-Ex1, $\rho$=0.5, n=200} 
\scalebox{0.55}{
\begin{tabular}{|c|c|ccccccccc|}
  \toprule 
 \multicolumn{1}{|c}{} &       & BOSS  & FS    & FSstop & FStrim & FSstoptrim & lasso & Gamma lasso & SparseNet & rlasso \\
 \multicolumn{1}{|c}{} &       & C$_p$/AICc/CV & EBIC/HDBIC/HDHQ/CV & EBIC/HDBIC/HDHQ & HDBIC & HDBIC & AICc/CV & AICc/CV & CV    & CV  \\
 \cmidrule{3-11}\multicolumn{1}{|c}{} &       & \multicolumn{9}{c|}{\% worse than the best possible BOSS}  \\
 \midrule\multirow{4}[2]{*}{hsnr} & p=250 & 4/1/17 & 495/495/495/20 & 1/0/1 & 495 & 0 & 139/138 & 177/138 & 17 & 16 \\ 
   & p=500 & 21/2/18 & 507/507/507/18 & 3/0/1 & 507 & 0 & 161/161 & 359/161 & 20 & 19 \\ 
   & p=1000 & 70/9/20 & 513/513/513/21 & 3/0/0 & 513 & 0 & 184/186 & 425/186 & 24 & 20 \\ 
   & p=1500 & 113/30/16 & 502/502/502/19 & 3/0/0 & 502 & 0 & 208/209 & 428/209 & 23 & 14 \\ 
  \midrule\multirow{4}[2]{*}{msnr} & p=250 & 22/13/19 & 490/490/490/22 & 4/303/8 & 490 & 304 & 137/136 & 293/136 & 18 & 37 \\ 
   & p=500 & 53/24/20 & 498/498/498/20 & 8/412/20 & 498 & 414 & 157/158 & 450/158 & 21 & 35 \\ 
   & p=1000 & 116/52/23 & 506/506/506/25 & 8/570/26 & 506 & 570 & 180/184 & 475/184 & 24 & 39 \\ 
   & p=1500 & 182/113/22 & 491/491/491/24 & 11/584/61 & 491 & 584 & 203/204 & 465/204 & 26 & 73 \\ 
  \midrule\multirow{4}[2]{*}{lsnr} & p=250 & 13/12/11 & 165/165/165/12 & 12/13/13 & 165 & 13 & -4/-2 & 117/-2 & 1 & 1 \\ 
   & p=500 & 20/12/11 & 150/150/150/11 & 11/12/12 & 150 & 12 & -3/-1 & 144/-1 & 2 & 2 \\ 
   & p=1000 & 30/14/9 & 136/136/136/9 & 8/8/8 & 136 & 8 & -4/0 & 133/0 & 2 & 3 \\ 
   & p=1500 & 31/17/6 & 141/141/141/6 & 3/2/2 & 141 & 2 & -3/0 & 138/0 & 3 & 4 \\ 
   \midrule 
 \multicolumn{1}{|c}{} &       & \multicolumn{9}{c|}{Relative efficiency} \\
\midrule\multirow{4}[2]{*}{hsnr} & p=250 & 0.96/0.99/0.85 & 0.17/0.17/0.17/0.83 & 0.99/1/0.99 & 0.17 & 1 & 0.42/0.42 & 0.36/0.42 & 0.85 & 0.86 \\ 
   & p=500 & 0.83/0.98/0.84 & 0.16/0.16/0.16/0.85 & 0.97/1/0.99 & 0.16 & 1 & 0.38/0.38 & 0.22/0.38 & 0.83 & 0.84 \\ 
   & p=1000 & 0.59/0.92/0.84 & 0.16/0.16/0.16/0.82 & 0.97/1/1 & 0.16 & 1 & 0.35/0.35 & 0.19/0.35 & 0.81 & 0.83 \\ 
   & p=1500 & 0.47/0.77/0.86 & 0.17/0.17/0.17/0.84 & 0.98/1/1 & 0.17 & 1 & 0.32/0.32 & 0.19/0.32 & 0.81 & 0.88 \\ 
  \midrule\multirow{4}[2]{*}{msnr} & p=250 & 0.85/0.92/0.87 & 0.18/0.18/0.18/0.85 & 1/0.26/0.96 & 0.18 & 0.26 & 0.44/0.44 & 0.26/0.44 & 0.88 & 0.76 \\ 
   & p=500 & 0.7/0.87/0.89 & 0.18/0.18/0.18/0.9 & 1/0.21/0.9 & 0.18 & 0.21 & 0.42/0.42 & 0.2/0.42 & 0.89 & 0.8 \\ 
   & p=1000 & 0.5/0.71/0.88 & 0.18/0.18/0.18/0.87 & 1/0.16/0.86 & 0.18 & 0.16 & 0.39/0.38 & 0.19/0.38 & 0.87 & 0.78 \\ 
   & p=1500 & 0.4/0.52/0.91 & 0.19/0.19/0.19/0.9 & 1/0.16/0.69 & 0.19 & 0.16 & 0.37/0.37 & 0.2/0.37 & 0.89 & 0.64 \\ 
  \midrule\multirow{4}[2]{*}{lsnr} & p=250 & 0.85/0.86/0.86 & 0.36/0.36/0.36/0.86 & 0.86/0.85/0.85 & 0.36 & 0.85 & 1/0.98 & 0.44/0.98 & 0.95 & 0.95 \\ 
   & p=500 & 0.8/0.86/0.87 & 0.39/0.39/0.39/0.87 & 0.87/0.86/0.86 & 0.39 & 0.86 & 1/0.97 & 0.4/0.97 & 0.94 & 0.94 \\ 
   & p=1000 & 0.74/0.84/0.88 & 0.41/0.41/0.41/0.88 & 0.89/0.88/0.88 & 0.41 & 0.88 & 1/0.96 & 0.41/0.96 & 0.94 & 0.93 \\ 
   & p=1500 & 0.74/0.83/0.92 & 0.4/0.4/0.4/0.92 & 0.95/0.95/0.95 & 0.4 & 0.95 & 1/0.97 & 0.41/0.97 & 0.94 & 0.94 \\ 
   \midrule 
 \multicolumn{1}{|c}{} &       & \multicolumn{9}{c|}{Sparsistency} \\
\midrule\multirow{4}[2]{*}{hsnr} & p=250 & 6/6/6 & 6/6/6/6 & 6/6/6 & 6 & 6 & 6/6 & 6/6 & 6 & 6 \\ 
   & p=500 & 6/6/6 & 6/6/6/6 & 6/6/6 & 6 & 6 & 6/6 & 6/6 & 6 & 6 \\ 
   & p=1000 & 6/6/6 & 6/6/6/6 & 6/6/6 & 6 & 6 & 6/6 & 6/6 & 6 & 6 \\ 
   & p=1500 & 6/6/6 & 6/6/6/6 & 6/6/6 & 6 & 6 & 6/6 & 6/6 & 6 & 6 \\ 
  \midrule\multirow{4}[2]{*}{msnr} & p=250 & 6/6/6 & 6/6/6/6 & 6/3.1/5.9 & 6 & 3.1 & 6/6 & 6/6 & 6 & 6 \\ 
   & p=500 & 6/6/6 & 6/6/6/6 & 6/2.3/5.9 & 6 & 2.3 & 6/6 & 6/6 & 6 & 6 \\ 
   & p=1000 & 6/6/6 & 6/6/6/6 & 6/1/5.8 & 6 & 1 & 6/6 & 6/6 & 6 & 6 \\ 
   & p=1500 & 6/6/6 & 6/6/6/6 & 5.9/0/5.5 & 6 & 0 & 6/6 & 6/6 & 6 & 5.9 \\ 
  \midrule\multirow{4}[2]{*}{lsnr} & p=250 & 0.7/0.3/1 & 5.5/5.5/5.5/1 & 0.2/0/0.1 & 5.5 & 0 & 3/3.1 & 4.3/3.1 & 2.7 & 2.5 \\ 
   & p=500 & 1/0.4/0.8 & 4.2/4.2/4.2/0.8 & 0.2/0/0.1 & 4.2 & 0 & 2.9/2.9 & 3.7/2.9 & 2.5 & 2.4 \\ 
   & p=1000 & 1.2/0.6/0.6 & 3.1/3.1/3.1/0.6 & 0.1/0/0 & 3.1 & 0 & 2.5/2.5 & 3/2.5 & 2.2 & 2 \\ 
   & p=1500 & 0.7/0.4/0.2 & 2.1/2.1/2.1/0.2 & 0/0/0 & 2.1 & 0 & 1.3/1.3 & 2.1/1.3 & 1.2 & 1.1 \\ 
   \midrule 
 \multicolumn{1}{|c}{} &       & \multicolumn{9}{c|}{Number of extra variables} \\
\midrule\multirow{4}[2]{*}{hsnr} & p=250 & 0.2/0/0.3 & 193/193/193/0.3 & 0/0/0 & 193 & 0 & 17/23.7 & 26.6/23.7 & 2 & 0.5 \\ 
   & p=500 & 1/0/0.3 & 193/193/193/0.3 & 0/0/0 & 193 & 0 & 18.3/28.3 & 71.3/28.3 & 3 & 0.8 \\ 
   & p=1000 & 3.6/0.3/0.2 & 193/193/193/0.3 & 0/0/0 & 193 & 0 & 18.7/35.2 & 87.8/35.2 & 3.6 & 0.6 \\ 
   & p=1500 & 5.9/1.3/0.2 & 193/193/193/0.2 & 0/0/0 & 192.9 & 0 & 22.5/44.6 & 89.1/44.6 & 3.9 & 0.5 \\ 
  \midrule\multirow{4}[2]{*}{msnr} & p=250 & 0.5/0.2/0.3 & 193/193/193/0.4 & 0/0/0 & 193 & 0 & 16.7/23.7 & 46.2/23.7 & 1.2 & 1.2 \\ 
   & p=500 & 1.7/0.3/0.3 & 193/193/193/0.3 & 0/0/0 & 193 & 0 & 18.4/28.3 & 98.4/28.3 & 1.8 & 1.3 \\ 
   & p=1000 & 4.6/1/0.3 & 193/193/193/0.3 & 0/0/0 & 193 & 0 & 18.9/35.2 & 101/35.2 & 2 & 1.4 \\ 
   & p=1500 & 7.6/3.2/0.3 & 193/193/193/0.3 & 0/0/0 & 192.9 & 0 & 22.4/44.6 & 100.2/44.6 & 2.4 & 2.9 \\ 
  \midrule\multirow{4}[2]{*}{lsnr} & p=250 & 0.4/0.1/0.5 & 193.5/193.5/193.5/0.6 & 0/0/0 & 193.5 & 0 & 9.4/12.1 & 67.6/12.1 & 8.7 & 6.7 \\ 
   & p=500 & 2.4/0.2/0.5 & 194.8/194.8/194.8/0.5 & 0/0/0 & 194.8 & 0 & 10.8/15.6 & 114.8/15.6 & 12.2 & 9.3 \\ 
   & p=1000 & 5.2/1.3/0.4 & 195.9/195.9/195.9/0.4 & 0/0/0 & 195.8 & 0 & 10.8/18 & 115.1/18 & 12.8 & 10.6 \\ 
   & p=1500 & 5.2/2.3/0.3 & 196.9/196.9/196.9/0.3 & 0/0/0 & 196.8 & 0 & 9/13.3 & 113.5/13.3 & 11.4 & 9.6 \\ 
   \bottomrule 
\end{tabular}
}
\end{table}
