# Supplementary material for: On the Use of Information Criteria for Subset Selection in Least Squares Regression
Source: arXiv:1911.10191 source file (2021-03-06)
Supplement: Supplementary file 36 [file Sparse-Ex1_rho_09.tex]

% latex table generated in R 4.0.3 by xtable 1.8-4 package
% Sun Feb 21 09:03:44 2021
\begin{table}[ht]
\centering
\caption{The performance of BOSS for high dimensional data, Sparse-Ex1, $\rho$=0.9, n=200} 
\scalebox{0.55}{
\begin{tabular}{|c|c|ccccccccc|}
  \toprule 
 \multicolumn{1}{|c}{} &       & BOSS  & FS    & FSstop & FStrim & FSstoptrim & lasso & Gamma lasso & SparseNet & rlasso \\
 \multicolumn{1}{|c}{} &       & C$_p$/AICc/CV & EBIC/HDBIC/HDHQ/CV & EBIC/HDBIC/HDHQ & HDBIC & HDBIC & AICc/CV & AICc/CV & CV    & CV  \\
 \cmidrule{3-11}\multicolumn{1}{|c}{} &       & \multicolumn{9}{c|}{\% worse than the best possible BOSS}  \\
 \midrule\multirow{4}[2]{*}{hsnr} & p=250 & 5/4/39 & 447/447/447/39 & 3/25/4 & 447 & 22 & 108/107 & 201/107 & 22 & 25 \\ 
   & p=500 & 7/5/40 & 473/473/473/42 & 4/17/6 & 473 & 16 & 135/134 & 341/134 & 31 & 26 \\ 
   & p=1000 & 18/7/50 & 447/447/447/51 & 3/46/6 & 447 & 43 & 143/141 & 360/141 & 30 & 22 \\ 
   & p=1500 & 37/9/48 & 459/459/459/49 & 5/27/7 & 459 & 26 & 176/173 & 389/173 & 54 & 30 \\ 
  \midrule\multirow{4}[2]{*}{msnr} & p=250 & 10/9/19 & 272/272/272/19 & 14/199/18 & 272 & 199 & 41/40 & 170/40 & 25 & 20 \\ 
   & p=500 & 12/8/13 & 262/262/262/14 & 7/232/14 & 262 & 232 & 48/47 & 239/47 & 27 & 11 \\ 
   & p=1000 & 21/12/13 & 242/242/242/15 & 7/291/18 & 242 & 291 & 52/50 & 226/50 & 26 & 5 \\ 
   & p=1500 & 41/21/14 & 237/237/237/15 & 11/273/58 & 237 & 273 & 66/64 & 223/64 & 26 & 31 \\ 
  \midrule\multirow{4}[2]{*}{lsnr} & p=250 & 11/11/11 & 164/164/164/10 & 11/11/11 & 164 & 11 & -13/-12 & 97/-12 & -8 & -8 \\ 
   & p=500 & 14/12/12 & 155/155/155/12 & 13/13/13 & 155 & 13 & -9/-9 & 149/-9 & -5 & -5 \\ 
   & p=1000 & 18/11/10 & 139/139/139/10 & 9/9/9 & 139 & 9 & -9/-8 & 136/-8 & -5 & -4 \\ 
   & p=1500 & 19/7/6 & 151/151/151/6 & 2/2/2 & 151 & 2 & -5/-3 & 147/-3 & -1 & 0 \\ 
   \midrule 
 \multicolumn{1}{|c}{} &       & \multicolumn{9}{c|}{Relative efficiency} \\
\midrule\multirow{4}[2]{*}{hsnr} & p=250 & 0.98/0.99/0.74 & 0.19/0.19/0.19/0.74 & 1/0.82/0.99 & 0.19 & 0.85 & 0.49/0.5 & 0.34/0.5 & 0.84 & 0.83 \\ 
   & p=500 & 0.97/0.99/0.75 & 0.18/0.18/0.18/0.74 & 1/0.89/0.99 & 0.18 & 0.9 & 0.44/0.45 & 0.24/0.45 & 0.8 & 0.83 \\ 
   & p=1000 & 0.87/0.96/0.69 & 0.19/0.19/0.19/0.68 & 1/0.71/0.97 & 0.19 & 0.72 & 0.42/0.43 & 0.22/0.43 & 0.8 & 0.84 \\ 
   & p=1500 & 0.77/0.97/0.71 & 0.19/0.19/0.19/0.71 & 1/0.83/0.99 & 0.19 & 0.83 & 0.38/0.38 & 0.21/0.38 & 0.68 & 0.81 \\ 
  \midrule\multirow{4}[2]{*}{msnr} & p=250 & 0.99/1/0.91 & 0.29/0.29/0.29/0.91 & 0.96/0.36/0.92 & 0.29 & 0.36 & 0.77/0.78 & 0.4/0.78 & 0.87 & 0.9 \\ 
   & p=500 & 0.96/0.99/0.95 & 0.3/0.3/0.3/0.94 & 1/0.32/0.94 & 0.3 & 0.32 & 0.72/0.73 & 0.32/0.73 & 0.85 & 0.97 \\ 
   & p=1000 & 0.87/0.93/0.93 & 0.31/0.31/0.31/0.91 & 0.98/0.27/0.89 & 0.31 & 0.27 & 0.69/0.7 & 0.32/0.7 & 0.83 & 1 \\ 
   & p=1500 & 0.79/0.92/0.98 & 0.33/0.33/0.33/0.97 & 1/0.3/0.71 & 0.33 & 0.3 & 0.67/0.68 & 0.34/0.68 & 0.88 & 0.85 \\ 
  \midrule\multirow{4}[2]{*}{lsnr} & p=250 & 0.78/0.78/0.78 & 0.33/0.33/0.33/0.79 & 0.78/0.78/0.78 & 0.33 & 0.78 & 1/0.99 & 0.44/0.99 & 0.95 & 0.95 \\ 
   & p=500 & 0.79/0.81/0.81 & 0.36/0.36/0.36/0.81 & 0.81/0.8/0.8 & 0.36 & 0.8 & 1/0.99 & 0.36/0.99 & 0.95 & 0.95 \\ 
   & p=1000 & 0.77/0.82/0.83 & 0.38/0.38/0.38/0.82 & 0.83/0.83/0.83 & 0.38 & 0.83 & 1/0.98 & 0.39/0.98 & 0.95 & 0.95 \\ 
   & p=1500 & 0.8/0.89/0.9 & 0.38/0.38/0.38/0.9 & 0.93/0.94/0.94 & 0.38 & 0.94 & 1/0.98 & 0.38/0.98 & 0.96 & 0.95 \\ 
   \midrule 
 \multicolumn{1}{|c}{} &       & \multicolumn{9}{c|}{Sparsistency} \\
\midrule\multirow{4}[2]{*}{hsnr} & p=250 & 6/6/6 & 6/6/6/6 & 6/5.8/6 & 6 & 5.8 & 6/6 & 6/6 & 6 & 6 \\ 
   & p=500 & 6/6/6 & 6/6/6/6 & 6/5.9/6 & 6 & 5.9 & 6/6 & 6/6 & 6 & 6 \\ 
   & p=1000 & 6/6/6 & 6/6/6/6 & 6/5.7/5.9 & 6 & 5.7 & 6/6 & 5.9/6 & 6 & 6 \\ 
   & p=1500 & 6/6/6 & 6/6/6/6 & 6/5.8/5.9 & 6 & 5.8 & 6/6 & 5.9/6 & 5.9 & 6 \\ 
  \midrule\multirow{4}[2]{*}{msnr} & p=250 & 5/5/5 & 5.9/5.9/5.9/5.1 & 4.9/2.1/4.8 & 5.9 & 2.1 & 5.9/5.9 & 5.2/5.9 & 5 & 5.6 \\ 
   & p=500 & 5/5/5 & 5.6/5.6/5.6/5 & 4.9/1.8/4.8 & 5.6 & 1.7 & 5.9/5.9 & 4.9/5.9 & 4.8 & 5.7 \\ 
   & p=1000 & 4.9/4.9/4.9 & 5.4/5.4/5.4/4.9 & 4.8/0.6/4.7 & 5.4 & 0.6 & 5.9/5.9 & 4.9/5.9 & 4.7 & 5.7 \\ 
   & p=1500 & 4.9/4.9/4.8 & 5.2/5.2/5.2/4.8 & 4.7/0/3.9 & 5.2 & 0 & 5.8/5.8 & 4.9/5.8 & 4.6 & 5.4 \\ 
  \midrule\multirow{4}[2]{*}{lsnr} & p=250 & 0.4/0.2/0.6 & 5.3/5.3/5.3/0.7 & 0.1/0/0.1 & 5.3 & 0 & 2.4/2.5 & 2.9/2.5 & 2.2 & 2.1 \\ 
   & p=500 & 0.6/0.3/0.6 & 3.6/3.6/3.6/0.6 & 0.1/0/0.1 & 3.6 & 0 & 2.2/2.4 & 2.6/2.4 & 2 & 1.9 \\ 
   & p=1000 & 0.7/0.3/0.4 & 2.6/2.6/2.6/0.4 & 0.1/0/0 & 2.6 & 0 & 2/2.2 & 2.2/2.2 & 1.8 & 1.7 \\ 
   & p=1500 & 0.4/0.1/0.2 & 1.9/1.9/1.9/0.2 & 0/0/0 & 1.9 & 0 & 1/1 & 1.6/1 & 0.9 & 0.8 \\ 
   \midrule 
 \multicolumn{1}{|c}{} &       & \multicolumn{9}{c|}{Number of extra variables} \\
\midrule\multirow{4}[2]{*}{hsnr} & p=250 & 0.5/0.5/2.8 & 193/193/193/1.3 & 0.5/0.5/0.5 & 193 & 0.2 & 17.9/21.4 & 35.7/21.4 & 3.9 & 2.7 \\ 
   & p=500 & 0.3/0.2/1.4 & 193/193/193/0.9 & 0.2/0.2/0.2 & 193 & 0.1 & 19.5/25.2 & 72.1/25.2 & 5.1 & 1.6 \\ 
   & p=1000 & 1.2/0.6/1.6 & 193/193/193/1.3 & 0.6/0.5/0.5 & 193 & 0.3 & 21.2/29.9 & 85.1/29.9 & 7 & 2.3 \\ 
   & p=1500 & 2/0.3/1.1 & 193/193/193/1 & 0.2/0.2/0.2 & 193 & 0.2 & 25.2/40.1 & 91.9/40.1 & 10 & 1.9 \\ 
  \midrule\multirow{4}[2]{*}{msnr} & p=250 & 1.6/1.4/2.9 & 193.1/193.1/193.1/2 & 1.2/0.5/1.2 & 193.1 & 0.5 & 17.9/21.4 & 57/21.4 & 6.9 & 6.8 \\ 
   & p=500 & 1.7/1.3/1.7 & 193.4/193.4/193.4/1.6 & 1.1/0.3/1 & 193.4 & 0.3 & 19.4/25 & 103.4/25 & 7.3 & 5.3 \\ 
   & p=1000 & 2.5/1.7/1.7 & 193.6/193.6/193.6/1.7 & 1.2/0.2/1.2 & 193.6 & 0.2 & 21.1/29.8 & 107/29.8 & 7.8 & 4.7 \\ 
   & p=1500 & 4.6/2.2/1.7 & 193.7/193.7/193.7/1.7 & 1.2/0/0.9 & 193.7 & 0 & 25.1/39.7 & 107.2/39.7 & 7.5 & 8.5 \\ 
  \midrule\multirow{4}[2]{*}{lsnr} & p=250 & 0.9/0.4/1.6 & 193.7/193.7/193.7/1.5 & 0.2/0/0.1 & 193.7 & 0 & 12.2/13.8 & 62.3/13.8 & 11.5 & 9.6 \\ 
   & p=500 & 1.7/0.5/1.5 & 195.4/195.4/195.4/1.2 & 0.1/0/0 & 195.4 & 0 & 12.7/16 & 119.1/16 & 12.9 & 10.2 \\ 
   & p=1000 & 3.3/0.9/1 & 196.4/196.4/196.4/0.9 & 0.1/0/0 & 196.4 & 0 & 13.8/18 & 120.8/18 & 14 & 10.6 \\ 
   & p=1500 & 3.3/0.8/0.5 & 197.1/197.1/197.1/0.5 & 0/0/0 & 197 & 0 & 10.8/14.5 & 119.7/14.5 & 12.4 & 9.2 \\ 
   \bottomrule 
\end{tabular}
}
\end{table}
