# Supplementary material for: On the Use of Information Criteria for Subset Selection in Least Squares Regression
Source: arXiv:1911.10191 source file (2021-03-06)
Supplement: Supplementary file 37 [file Sparse-Ex2_rho_0.tex]

% latex table generated in R 4.0.3 by xtable 1.8-4 package
% Sun Feb 21 09:04:06 2021
\begin{table}[ht]
\centering
\caption{The performance of BOSS for high dimensional data, Sparse-Ex2, $\rho$=0, n=200} 
\scalebox{0.55}{
\begin{tabular}{|c|c|ccccccccc|}
  \toprule 
 \multicolumn{1}{|c}{} &       & BOSS  & FS    & FSstop & FStrim & FSstoptrim & lasso & Gamma lasso & SparseNet & rlasso \\
 \multicolumn{1}{|c}{} &       & C$_p$/AICc/CV & EBIC/HDBIC/HDHQ/CV & EBIC/HDBIC/HDHQ & HDBIC & HDBIC & AICc/CV & AICc/CV & CV    & CV  \\
 \cmidrule{3-11}\multicolumn{1}{|c}{} &       & \multicolumn{9}{c|}{\% worse than the best possible BOSS}  \\
 \midrule\multirow{4}[2]{*}{hsnr} & p=250 & 5/1/18 & 501/501/501/18 & 2/0/1 & 501 & 0 & 152/152 & 189/152 & 18 & 16 \\ 
   & p=500 & 30/3/18 & 501/501/501/19 & 2/0/1 & 501 & 0 & 178/179 & 366/179 & 23 & 17 \\ 
   & p=1000 & 86/11/20 & 501/501/501/20 & 2/0/0 & 501 & 0 & 203/204 & 420/204 & 25 & 14 \\ 
   & p=1500 & 132/40/19 & 501/501/501/21 & 2/0/0 & 501 & 0 & 218/218 & 432/218 & 26 & 15 \\ 
  \midrule\multirow{4}[2]{*}{msnr} & p=250 & 29/16/19 & 498/498/498/20 & 5/419/13 & 498 & 419 & 151/151 & 311/151 & 18 & 60 \\ 
   & p=500 & 83/38/22 & 495/495/495/23 & 10/514/39 & 495 & 514 & 175/176 & 448/176 & 23 & 87 \\ 
   & p=1000 & 162/88/26 & 491/491/491/27 & 18/538/89 & 491 & 538 & 197/200 & 462/200 & 27 & 117 \\ 
   & p=1500 & 214/151/27 & 485/485/485/29 & 26/536/142 & 485 & 536 & 210/211 & 460/211 & 26 & 140 \\ 
  \midrule\multirow{4}[2]{*}{lsnr} & p=250 & 10/8/9 & 169/169/169/9 & 8/7/8 & 169 & 7 & -3/0 & 125/0 & 3 & 3 \\ 
   & p=500 & 16/6/8 & 162/162/162/8 & 5/4/5 & 162 & 4 & -2/1 & 156/1 & 4 & 4 \\ 
   & p=1000 & 27/9/6 & 158/158/158/6 & 3/3/3 & 158 & 3 & -1/3 & 155/3 & 5 & 5 \\ 
   & p=1500 & 36/20/6 & 156/156/156/6 & 2/2/2 & 156 & 2 & -2/2 & 153/2 & 4 & 6 \\ 
   \midrule 
 \multicolumn{1}{|c}{} &       & \multicolumn{9}{c|}{Relative efficiency} \\
\midrule\multirow{4}[2]{*}{hsnr} & p=250 & 0.95/0.99/0.85 & 0.17/0.17/0.17/0.85 & 0.98/1/0.99 & 0.17 & 1 & 0.4/0.4 & 0.35/0.4 & 0.84 & 0.86 \\ 
   & p=500 & 0.77/0.97/0.85 & 0.17/0.17/0.17/0.84 & 0.98/1/0.99 & 0.17 & 1 & 0.36/0.36 & 0.21/0.36 & 0.81 & 0.86 \\ 
   & p=1000 & 0.54/0.9/0.84 & 0.17/0.17/0.17/0.83 & 0.98/1/1 & 0.17 & 1 & 0.33/0.33 & 0.19/0.33 & 0.8 & 0.87 \\ 
   & p=1500 & 0.43/0.72/0.84 & 0.17/0.17/0.17/0.83 & 0.98/1/1 & 0.17 & 1 & 0.31/0.31 & 0.19/0.31 & 0.79 & 0.87 \\ 
  \midrule\multirow{4}[2]{*}{msnr} & p=250 & 0.81/0.9/0.88 & 0.18/0.18/0.18/0.88 & 1/0.2/0.93 & 0.18 & 0.2 & 0.42/0.42 & 0.26/0.42 & 0.89 & 0.66 \\ 
   & p=500 & 0.6/0.8/0.9 & 0.18/0.18/0.18/0.89 & 1/0.18/0.79 & 0.18 & 0.18 & 0.4/0.4 & 0.2/0.4 & 0.89 & 0.59 \\ 
   & p=1000 & 0.45/0.63/0.94 & 0.2/0.2/0.2/0.93 & 1/0.19/0.63 & 0.2 & 0.19 & 0.4/0.39 & 0.21/0.39 & 0.93 & 0.54 \\ 
   & p=1500 & 0.4/0.5/0.99 & 0.22/0.22/0.22/0.98 & 1/0.2/0.52 & 0.22 & 0.2 & 0.41/0.4 & 0.22/0.4 & 1 & 0.52 \\ 
  \midrule\multirow{4}[2]{*}{lsnr} & p=250 & 0.88/0.9/0.89 & 0.36/0.36/0.36/0.89 & 0.9/0.91/0.9 & 0.36 & 0.91 & 1/0.98 & 0.43/0.98 & 0.95 & 0.95 \\ 
   & p=500 & 0.85/0.93/0.91 & 0.38/0.38/0.38/0.91 & 0.94/0.94/0.94 & 0.38 & 0.94 & 1/0.97 & 0.38/0.97 & 0.94 & 0.94 \\ 
   & p=1000 & 0.78/0.91/0.93 & 0.38/0.38/0.38/0.93 & 0.96/0.96/0.96 & 0.38 & 0.96 & 1/0.96 & 0.39/0.96 & 0.94 & 0.94 \\ 
   & p=1500 & 0.73/0.82/0.93 & 0.38/0.38/0.38/0.93 & 0.96/0.97/0.96 & 0.38 & 0.97 & 1/0.96 & 0.39/0.96 & 0.95 & 0.93 \\ 
   \midrule 
 \multicolumn{1}{|c}{} &       & \multicolumn{9}{c|}{Sparsistency} \\
\midrule\multirow{4}[2]{*}{hsnr} & p=250 & 6/6/6 & 6/6/6/6 & 6/6/6 & 6 & 6 & 6/6 & 6/6 & 6 & 6 \\ 
   & p=500 & 6/6/6 & 6/6/6/6 & 6/6/6 & 6 & 6 & 6/6 & 6/6 & 6 & 6 \\ 
   & p=1000 & 6/6/6 & 6/6/6/6 & 6/6/6 & 6 & 6 & 6/6 & 6/6 & 6 & 6 \\ 
   & p=1500 & 6/6/6 & 6/6/6/6 & 6/6/6 & 6 & 6 & 6/6 & 6/6 & 6 & 6 \\ 
  \midrule\multirow{4}[2]{*}{msnr} & p=250 & 6/6/6 & 6/6/6/6 & 6/1.7/5.9 & 6 & 1.7 & 6/6 & 6/6 & 6 & 6 \\ 
   & p=500 & 6/6/6 & 6/6/6/6 & 5.9/0.5/5.7 & 6 & 0.5 & 6/6 & 6/6 & 6 & 5.9 \\ 
   & p=1000 & 6/6/6 & 6/6/6/6 & 5.8/0.1/5.2 & 6 & 0.1 & 6/6 & 6/6 & 6 & 5.8 \\ 
   & p=1500 & 6/6/6 & 6/6/6/6 & 5.8/0/4.6 & 6 & 0 & 6/6 & 6/6 & 6 & 5.7 \\ 
  \midrule\multirow{4}[2]{*}{lsnr} & p=250 & 0.4/0.2/0.7 & 5.5/5.5/5.5/0.7 & 0.1/0/0.1 & 5.5 & 0 & 2.4/2.3 & 4.3/2.3 & 2.1 & 1.9 \\ 
   & p=500 & 0.5/0.2/0.4 & 4/4/4/0.4 & 0.1/0/0 & 4 & 0 & 1.7/1.8 & 3.5/1.8 & 1.6 & 1.5 \\ 
   & p=1000 & 0.5/0.2/0.3 & 2.7/2.7/2.7/0.3 & 0.1/0/0 & 2.7 & 0 & 1.3/1.3 & 2.6/1.3 & 1.2 & 1.2 \\ 
   & p=1500 & 0.6/0.3/0.2 & 2.1/2.1/2.1/0.2 & 0/0/0 & 2.1 & 0 & 1.1/1.1 & 2.1/1.1 & 1 & 0.9 \\ 
   \midrule 
 \multicolumn{1}{|c}{} &       & \multicolumn{9}{c|}{Number of extra variables} \\
\midrule\multirow{4}[2]{*}{hsnr} & p=250 & 0.2/0/0.3 & 193/193/193/0.3 & 0/0/0 & 193 & 0 & 18.2/26.6 & 29.1/26.6 & 2.5 & 0.6 \\ 
   & p=500 & 1.7/0/0.3 & 193/193/193/0.3 & 0/0/0 & 193 & 0 & 20.5/35 & 75/35 & 3.5 & 0.5 \\ 
   & p=1000 & 4.7/0.3/0.3 & 193/193/193/0.3 & 0/0/0 & 193 & 0 & 22.3/44.2 & 88.9/44.2 & 4.2 & 0.4 \\ 
   & p=1500 & 7.1/1.9/0.2 & 193/193/193/0.3 & 0/0/0 & 192.9 & 0 & 23/48.8 & 90.4/48.8 & 4.4 & 0.4 \\ 
  \midrule\multirow{4}[2]{*}{msnr} & p=250 & 0.5/0.2/0.3 & 193/193/193/0.3 & 0/0/0 & 193 & 0 & 18.2/26.6 & 49.3/26.6 & 1.6 & 2.3 \\ 
   & p=500 & 3/0.6/0.3 & 193/193/193/0.4 & 0/0/0 & 193 & 0 & 20.7/34.9 & 98.2/34.9 & 2.1 & 3.7 \\ 
   & p=1000 & 6.6/1.9/0.4 & 193/193/193/0.4 & 0/0/0 & 193 & 0 & 22.4/44.3 & 100.9/44.3 & 2.6 & 4.6 \\ 
   & p=1500 & 9.3/4.8/0.4 & 193/193/193/0.4 & 0/0/0 & 192.9 & 0 & 23/48.6 & 100/48.6 & 2.5 & 6.2 \\ 
  \midrule\multirow{4}[2]{*}{lsnr} & p=250 & 0.5/0/0.4 & 193.5/193.5/193.5/0.4 & 0/0/0 & 193.5 & 0 & 8.9/11 & 69.1/11 & 8.1 & 6.5 \\ 
   & p=500 & 2.1/0.1/0.3 & 195/195/195/0.3 & 0/0/0 & 195 & 0 & 8.5/11.9 & 114.5/11.9 & 9.6 & 7.6 \\ 
   & p=1000 & 3.9/0.7/0.3 & 196.3/196.3/196.3/0.3 & 0/0/0 & 196.3 & 0 & 8.5/13.5 & 114/13.5 & 10.6 & 8.7 \\ 
   & p=1500 & 5.6/2.6/0.2 & 196.9/196.9/196.9/0.3 & 0/0/0 & 196.9 & 0 & 8.2/12.9 & 112.5/12.9 & 10.4 & 8.9 \\ 
   \bottomrule 
\end{tabular}
}
\end{table}
