# Supplementary material for: On the Use of Information Criteria for Subset Selection in Least Squares Regression
Source: arXiv:1911.10191 source file (2021-03-06)
Supplement: Supplementary file 38 [file Sparse-Ex2_rho_05.tex]

% latex table generated in R 4.0.3 by xtable 1.8-4 package
% Sun Feb 21 09:05:41 2021
\begin{table}[ht]
\centering
\caption{The performance of BOSS for high dimensional data, Sparse-Ex2, $\rho$=0.5, n=200} 
\scalebox{0.55}{
\begin{tabular}{|c|c|ccccccccc|}
  \toprule 
 \multicolumn{1}{|c}{} &       & BOSS  & FS    & FSstop & FStrim & FSstoptrim & lasso & Gamma lasso & SparseNet & rlasso \\
 \multicolumn{1}{|c}{} &       & C$_p$/AICc/CV & EBIC/HDBIC/HDHQ/CV & EBIC/HDBIC/HDHQ & HDBIC & HDBIC & AICc/CV & AICc/CV & CV    & CV  \\
 \cmidrule{3-11}\multicolumn{1}{|c}{} &       & \multicolumn{9}{c|}{\% worse than the best possible BOSS}  \\
 \midrule\multirow{4}[2]{*}{hsnr} & p=250 & 6/1/18 & 501/501/501/18 & 2/0/1 & 501 & 0 & 214/206 & 125/206 & 18 & 27 \\ 
   & p=500 & 40/3/18 & 501/501/501/19 & 2/0/1 & 501 & 0 & 259/245 & 269/245 & 24 & 37 \\ 
   & p=1000 & 110/16/20 & 501/501/501/22 & 2/0/0 & 501 & 0 & 304/285 & 373/285 & 26 & 55 \\ 
   & p=1500 & 154/49/21 & 501/501/501/25 & 2/0/0 & 501 & 0 & 337/306 & 391/306 & 27 & 75 \\ 
  \midrule\multirow{4}[2]{*}{msnr} & p=250 & 30/13/34 & 457/457/457/43 & 3/382/6 & 457 & 382 & 191/184 & 232/184 & 12 & 140 \\ 
   & p=500 & 74/26/41 & 412/412/412/62 & 8/437/27 & 412 & 437 & 206/195 & 347/195 & 9 & 177 \\ 
   & p=1000 & 113/57/44 & 331/331/331/66 & 20/368/73 & 331 & 368 & 195/179 & 298/179 & 3 & 180 \\ 
   & p=1500 & 104/80/42 & 263/263/263/67 & 29/296/96 & 263 & 296 & 172/153 & 240/153 & -2 & 157 \\ 
  \midrule\multirow{4}[2]{*}{lsnr} & p=250 & 7/5/8 & 162/162/162/9 & 5/5/5 & 162 & 5 & 3/4 & 113/4 & 7 & 7 \\ 
   & p=500 & 9/3/6 & 155/155/155/6 & 2/2/2 & 155 & 2 & 1/3 & 147/3 & 5 & 5 \\ 
   & p=1000 & 16/5/5 & 153/153/153/5 & 1/1/1 & 153 & 1 & 1/3 & 148/3 & 4 & 5 \\ 
   & p=1500 & 26/13/4 & 152/152/152/5 & 1/0/0 & 152 & 0 & 0/2 & 148/2 & 3 & 5 \\ 
   \midrule 
 \multicolumn{1}{|c}{} &       & \multicolumn{9}{c|}{Relative efficiency} \\
\midrule\multirow{4}[2]{*}{hsnr} & p=250 & 0.94/0.99/0.85 & 0.17/0.17/0.17/0.85 & 0.98/1/0.99 & 0.17 & 1 & 0.32/0.33 & 0.44/0.33 & 0.85 & 0.79 \\ 
   & p=500 & 0.72/0.97/0.85 & 0.17/0.17/0.17/0.84 & 0.98/1/0.99 & 0.17 & 1 & 0.28/0.29 & 0.27/0.29 & 0.8 & 0.73 \\ 
   & p=1000 & 0.48/0.86/0.83 & 0.17/0.17/0.17/0.82 & 0.98/1/1 & 0.17 & 1 & 0.25/0.26 & 0.21/0.26 & 0.79 & 0.65 \\ 
   & p=1500 & 0.39/0.67/0.83 & 0.17/0.17/0.17/0.8 & 0.98/1/1 & 0.17 & 1 & 0.23/0.25 & 0.2/0.25 & 0.79 & 0.57 \\ 
  \midrule\multirow{4}[2]{*}{msnr} & p=250 & 0.8/0.91/0.77 & 0.19/0.19/0.19/0.72 & 1/0.21/0.97 & 0.19 & 0.21 & 0.36/0.36 & 0.31/0.36 & 0.92 & 0.43 \\ 
   & p=500 & 0.62/0.86/0.76 & 0.21/0.21/0.21/0.67 & 1/0.2/0.85 & 0.21 & 0.2 & 0.35/0.37 & 0.24/0.37 & 0.99 & 0.39 \\ 
   & p=1000 & 0.48/0.66/0.72 & 0.24/0.24/0.24/0.62 & 0.86/0.22/0.6 & 0.24 & 0.22 & 0.35/0.37 & 0.26/0.37 & 1 & 0.37 \\ 
   & p=1500 & 0.48/0.54/0.69 & 0.27/0.27/0.27/0.59 & 0.76/0.25/0.5 & 0.27 & 0.25 & 0.36/0.39 & 0.29/0.39 & 1 & 0.38 \\ 
  \midrule\multirow{4}[2]{*}{lsnr} & p=250 & 0.97/0.98/0.96 & 0.39/0.39/0.39/0.95 & 0.98/0.99/0.98 & 0.39 & 0.99 & 1/0.99 & 0.49/0.99 & 0.97 & 0.97 \\ 
   & p=500 & 0.93/0.99/0.96 & 0.4/0.4/0.4/0.95 & 0.99/0.99/0.99 & 0.4 & 0.99 & 1/0.99 & 0.41/0.99 & 0.96 & 0.96 \\ 
   & p=1000 & 0.87/0.96/0.96 & 0.4/0.4/0.4/0.96 & 1/1/1 & 0.4 & 1 & 1/0.98 & 0.41/0.98 & 0.96 & 0.96 \\ 
   & p=1500 & 0.8/0.89/0.96 & 0.4/0.4/0.4/0.96 & 0.99/1/1 & 0.4 & 1 & 1/0.98 & 0.4/0.98 & 0.97 & 0.95 \\ 
   \midrule 
 \multicolumn{1}{|c}{} &       & \multicolumn{9}{c|}{Sparsistency} \\
\midrule\multirow{4}[2]{*}{hsnr} & p=250 & 6/6/6 & 6/6/6/6 & 6/6/6 & 6 & 6 & 6/6 & 6/6 & 6 & 6 \\ 
   & p=500 & 6/6/6 & 6/6/6/6 & 6/6/6 & 6 & 6 & 6/6 & 6/6 & 6 & 6 \\ 
   & p=1000 & 6/6/6 & 6/6/6/6 & 6/6/6 & 6 & 6 & 6/6 & 6/6 & 6 & 6 \\ 
   & p=1500 & 6/6/6 & 6/6/6/6 & 6/6/6 & 6 & 6 & 6/6 & 6/6 & 6 & 6 \\ 
  \midrule\multirow{4}[2]{*}{msnr} & p=250 & 6/6/6 & 6/6/6/6 & 6/1.5/5.9 & 6 & 1.5 & 6/6 & 6/6 & 6 & 5.9 \\ 
   & p=500 & 6/6/6 & 6/6/6/5.9 & 5.9/0.3/5.6 & 6 & 0.3 & 5.9/6 & 6/6 & 6 & 5.8 \\ 
   & p=1000 & 5.9/5.9/5.9 & 6/6/6/5.7 & 5.6/0/4.7 & 6 & 0 & 5.7/5.9 & 6/5.9 & 6 & 5.6 \\ 
   & p=1500 & 5.8/5.8/5.7 & 5.9/5.9/5.9/5.3 & 5.1/0/3.8 & 5.9 & 0 & 5.3/5.6 & 5.9/5.6 & 6 & 5.2 \\ 
  \midrule\multirow{4}[2]{*}{lsnr} & p=250 & 0.2/0.1/0.5 & 5.5/5.5/5.5/0.3 & 0/0/0 & 5.5 & 0 & 1/1 & 4/1 & 1 & 0.9 \\ 
   & p=500 & 0.2/0.1/0.2 & 3.6/3.6/3.6/0.2 & 0/0/0 & 3.6 & 0 & 0.7/0.7 & 2.8/0.7 & 0.7 & 0.6 \\ 
   & p=1000 & 0.2/0.1/0.1 & 2.1/2.1/2.1/0.1 & 0/0/0 & 2.1 & 0 & 0.5/0.5 & 1.8/0.5 & 0.5 & 0.4 \\ 
   & p=1500 & 0.2/0.1/0.1 & 1.5/1.5/1.5/0.1 & 0/0/0 & 1.5 & 0 & 0.4/0.4 & 1.3/0.4 & 0.4 & 0.3 \\ 
   \midrule 
 \multicolumn{1}{|c}{} &       & \multicolumn{9}{c|}{Number of extra variables} \\
\midrule\multirow{4}[2]{*}{hsnr} & p=250 & 0.2/0/0.3 & 193/193/193/0.3 & 0/0/0 & 193 & 0 & 27.9/43.8 & 19.2/43.8 & 2.7 & 1 \\ 
   & p=500 & 2.5/0/0.3 & 193/193/193/0.3 & 0/0/0 & 193 & 0 & 31.8/58.1 & 53.8/58.1 & 3.9 & 1.3 \\ 
   & p=1000 & 6.9/0.7/0.3 & 193/193/193/0.3 & 0/0/0 & 193 & 0 & 35.4/76.2 & 80.3/76.2 & 4.5 & 2 \\ 
   & p=1500 & 8.6/2.4/0.3 & 193/193/193/0.3 & 0/0/0 & 192.9 & 0 & 36.9/86 & 83.5/86 & 5 & 3.2 \\ 
  \midrule\multirow{4}[2]{*}{msnr} & p=250 & 0.9/0.3/0.6 & 193/193/193/1 & 0.1/0/0.1 & 193 & 0 & 27.7/43.8 & 39.5/43.8 & 2.4 & 10.9 \\ 
   & p=500 & 4.3/0.8/0.9 & 193/193/193/1.6 & 0.2/0/0.1 & 193 & 0 & 31.4/57.4 & 89.5/57.4 & 4.1 & 20.8 \\ 
   & p=1000 & 9.2/3/1.3 & 193/193/193/2.1 & 0.3/0/0.1 & 193 & 0 & 32/71.9 & 97.2/71.9 & 7.6 & 35.4 \\ 
   & p=1500 & 10.9/6.7/1.7 & 193.1/193.1/193.1/2.2 & 0.3/0/0.1 & 193 & 0 & 29.5/74.2 & 97.6/74.2 & 11.5 & 42.2 \\ 
  \midrule\multirow{4}[2]{*}{lsnr} & p=250 & 0.3/0/0.6 & 193.5/193.5/193.5/0.4 & 0/0/0 & 193.5 & 0 & 6.1/7.2 & 65.5/7.2 & 6.3 & 5.1 \\ 
   & p=500 & 1.2/0.1/0.3 & 195.4/195.4/195.4/0.3 & 0/0/0 & 195.4 & 0 & 6.6/7.7 & 111.7/7.7 & 7.1 & 5.6 \\ 
   & p=1000 & 2.5/0.5/0.3 & 196.9/196.9/196.9/0.3 & 0/0/0 & 196.9 & 0 & 6.5/9.2 & 112.7/9.2 & 7.9 & 5.9 \\ 
   & p=1500 & 4/1.7/0.2 & 197.5/197.5/197.5/0.3 & 0/0/0 & 197.4 & 0 & 6.8/9.4 & 111/9.4 & 7.4 & 6.5 \\ 
   \bottomrule 
\end{tabular}
}
\end{table}
