# Supplementary material for: On the Use of Information Criteria for Subset Selection in Least Squares Regression
Source: arXiv:1911.10191 source file (2021-03-06)
Supplement: Supplementary file 39 [file Sparse-Ex2_rho_09.tex]

% latex table generated in R 4.0.3 by xtable 1.8-4 package
% Sun Feb 21 09:07:14 2021
\begin{table}[ht]
\centering
\caption{The performance of BOSS for high dimensional data, Sparse-Ex2, $\rho$=0.9, n=200} 
\scalebox{0.55}{
\begin{tabular}{|c|c|ccccccccc|}
  \toprule 
 \multicolumn{1}{|c}{} &       & BOSS  & FS    & FSstop & FStrim & FSstoptrim & lasso & Gamma lasso & SparseNet & rlasso \\
 \multicolumn{1}{|c}{} &       & C$_p$/AICc/CV & EBIC/HDBIC/HDHQ/CV & EBIC/HDBIC/HDHQ & HDBIC & HDBIC & AICc/CV & AICc/CV & CV    & CV  \\
 \cmidrule{3-11}\multicolumn{1}{|c}{} &       & \multicolumn{9}{c|}{\% worse than the best possible BOSS}  \\
 \midrule\multirow{4}[2]{*}{hsnr} & p=250 & 18/13/68 & 225/225/225/128 & 37/137/49 & 225 & 116 & 186/147 & -7/147 & -36 & 116 \\ 
   & p=500 & 106/69/105 & 70/70/70/141 & 96/180/111 & 70 & 174 & 275/234 & -31/234 & -30 & 221 \\ 
   & p=1000 & 97/68/108 & 22/22/22/129 & 91/159/106 & 22 & 158 & 177/178 & 21/178 & 158 & 176 \\ 
   & p=1500 & 91/84/116 & 7/7/7/132 & 111/147/122 & 7 & 147 & 137/133 & 8/133 & 134 & 131 \\ 
  \midrule\multirow{4}[2]{*}{msnr} & p=250 & 23/21/18 & 68/68/68/61 & 57/82/64 & 68 & 82 & 75/70 & -4/70 & -9 & 70 \\ 
   & p=500 & 14/14/15 & 21/21/21/26 & 24/32/27 & 21 & 32 & 27/27 & 6/27 & 27 & 27 \\ 
   & p=1000 & 11/11/13 & 11/11/11/19 & 18/22/20 & 11 & 22 & 18/18 & 2/18 & 19 & 18 \\ 
   & p=1500 & 10/10/12 & 7/7/7/15 & 15/17/16 & 7 & 17 & 12/12 & -2/12 & 12 & 12 \\ 
  \midrule\multirow{4}[2]{*}{lsnr} & p=250 & 3/3/6 & 157/157/157/7 & 3/3/3 & 157 & 3 & 3/4 & 83/4 & 5 & 6 \\ 
   & p=500 & 5/1/5 & 153/153/153/5 & 1/1/1 & 153 & 1 & 2/2 & 132/2 & 4 & 5 \\ 
   & p=1000 & 12/2/4 & 151/151/151/5 & 0/0/0 & 151 & 0 & 1/2 & 138/2 & 4 & 5 \\ 
   & p=1500 & 21/9/4 & 151/151/151/5 & 0/0/0 & 151 & 0 & 1/2 & 140/2 & 3 & 5 \\ 
   \midrule 
 \multicolumn{1}{|c}{} &       & \multicolumn{9}{c|}{Relative efficiency} \\
\midrule\multirow{4}[2]{*}{hsnr} & p=250 & 0.54/0.56/0.38 & 0.2/0.2/0.2/0.28 & 0.47/0.27/0.43 & 0.2 & 0.3 & 0.22/0.26 & 0.69/0.26 & 1 & 0.3 \\ 
   & p=500 & 0.34/0.41/0.34 & 0.41/0.41/0.41/0.29 & 0.35/0.25/0.33 & 0.41 & 0.25 & 0.18/0.21 & 1/0.21 & 0.98 & 0.21 \\ 
   & p=1000 & 0.61/0.72/0.58 & 0.99/0.99/0.99/0.53 & 0.63/0.47/0.59 & 0.99 & 0.47 & 0.44/0.43 & 1/0.43 & 0.47 & 0.44 \\ 
   & p=1500 & 0.56/0.58/0.49 & 1/1/1/0.46 & 0.51/0.43/0.48 & 1 & 0.43 & 0.45/0.46 & 0.98/0.46 & 0.45 & 0.46 \\ 
  \midrule\multirow{4}[2]{*}{msnr} & p=250 & 0.74/0.76/0.77 & 0.54/0.54/0.54/0.57 & 0.58/0.5/0.56 & 0.54 & 0.5 & 0.52/0.54 & 0.95/0.54 & 1 & 0.54 \\ 
   & p=500 & 0.93/0.93/0.92 & 0.88/0.88/0.88/0.84 & 0.85/0.8/0.83 & 0.88 & 0.8 & 0.83/0.83 & 1/0.83 & 0.84 & 0.83 \\ 
   & p=1000 & 0.92/0.91/0.9 & 0.91/0.91/0.91/0.86 & 0.86/0.83/0.85 & 0.91 & 0.83 & 0.86/0.86 & 1/0.86 & 0.86 & 0.86 \\ 
   & p=1500 & 0.89/0.89/0.87 & 0.92/0.92/0.92/0.85 & 0.85/0.84/0.84 & 0.92 & 0.84 & 0.87/0.87 & 1/0.87 & 0.87 & 0.87 \\ 
  \midrule\multirow{4}[2]{*}{lsnr} & p=250 & 0.99/1/0.97 & 0.4/0.4/0.4/0.96 & 1/1/1 & 0.4 & 1 & 0.99/0.99 & 0.56/0.99 & 0.97 & 0.97 \\ 
   & p=500 & 0.96/1/0.96 & 0.4/0.4/0.4/0.96 & 1/1/1 & 0.4 & 1 & 0.99/0.99 & 0.43/0.99 & 0.97 & 0.96 \\ 
   & p=1000 & 0.9/0.98/0.96 & 0.4/0.4/0.4/0.96 & 1/1/1 & 0.4 & 1 & 0.99/0.98 & 0.42/0.98 & 0.97 & 0.96 \\ 
   & p=1500 & 0.83/0.92/0.96 & 0.4/0.4/0.4/0.96 & 1/1/1 & 0.4 & 1 & 1/0.98 & 0.42/0.98 & 0.97 & 0.95 \\ 
   \midrule 
 \multicolumn{1}{|c}{} &       & \multicolumn{9}{c|}{Sparsistency} \\
\midrule\multirow{4}[2]{*}{hsnr} & p=250 & 6/6/6 & 6/6/6/5.8 & 5.6/4.7/5.5 & 6 & 4.7 & 6/6 & 6/6 & 6 & 6 \\ 
   & p=500 & 4.7/4.7/4.7 & 5.4/5.4/5.4/3.4 & 3.9/2.2/3.6 & 5.4 & 2.2 & 1.4/2.2 & 6/2.2 & 6 & 2.3 \\ 
   & p=1000 & 3.7/3.7/3.5 & 4.3/4.3/4.3/1.9 & 2.9/0.8/2.5 & 4.3 & 0.8 & 0.8/0.7 & 3.1/0.7 & 1.2 & 0.8 \\ 
   & p=1500 & 2.4/2.4/2.1 & 3/3/3/0.8 & 1.5/0.1/1.1 & 3 & 0.1 & 0.8/0.8 & 1.9/0.8 & 0.8 & 0.8 \\ 
  \midrule\multirow{4}[2]{*}{msnr} & p=250 & 4.1/3.9/4.5 & 5.8/5.8/5.8/1.6 & 1.5/0.1/1.1 & 5.8 & 0.1 & 1/1.5 & 5.8/1.5 & 5.7 & 1.5 \\ 
   & p=500 & 1.9/1.8/1.9 & 4/4/4/0.6 & 0.7/0/0.4 & 4 & 0 & 0.7/0.6 & 2.5/0.6 & 0.7 & 0.5 \\ 
   & p=1000 & 1.3/1.2/1.1 & 2.6/2.6/2.6/0.4 & 0.4/0/0.2 & 2.6 & 0 & 0.4/0.4 & 1.7/0.4 & 0.4 & 0.4 \\ 
   & p=1500 & 0.8/0.8/0.6 & 1.8/1.8/1.8/0.2 & 0.2/0/0.1 & 1.8 & 0 & 0.4/0.4 & 1.3/0.4 & 0.3 & 0.3 \\ 
  \midrule\multirow{4}[2]{*}{lsnr} & p=250 & 0.1/0.1/0.2 & 4.9/4.9/4.9/0.1 & 0/0/0 & 4.9 & 0 & 0.2/0.2 & 1.4/0.2 & 0.2 & 0.2 \\ 
   & p=500 & 0.1/0/0 & 2.5/2.5/2.5/0 & 0/0/0 & 2.5 & 0 & 0.2/0.1 & 1.3/0.1 & 0.2 & 0.1 \\ 
   & p=1000 & 0.1/0/0 & 1.3/1.3/1.3/0 & 0/0/0 & 1.3 & 0 & 0.1/0.1 & 0.8/0.1 & 0.1 & 0.1 \\ 
   & p=1500 & 0/0/0 & 0.9/0.9/0.9/0 & 0/0/0 & 0.9 & 0 & 0.1/0.1 & 0.5/0.1 & 0.1 & 0.1 \\ 
   \midrule 
 \multicolumn{1}{|c}{} &       & \multicolumn{9}{c|}{Number of extra variables} \\
\midrule\multirow{4}[2]{*}{hsnr} & p=250 & 9.4/6.3/11.3 & 193/193/193/23.8 & 4/2/3.6 & 193 & 0 & 68.2/108.6 & 9.5/108.6 & 4.2 & 49.7 \\ 
   & p=500 & 12.7/9/11.2 & 193.6/193.6/193.6/10.4 & 3.4/1/2.6 & 193.6 & 0 & 9.6/35.3 & 33.7/35.3 & 56.3 & 36.3 \\ 
   & p=1000 & 6.3/6.8/5.8 & 194.7/194.7/194.7/3.5 & 2.3/0.3/1.5 & 194.6 & 0 & 6.1/6.3 & 89/6.3 & 16.4 & 4.9 \\ 
   & p=1500 & 6.4/5.7/3.7 & 196/196/196/1.1 & 1.1/0/0.6 & 195.9 & 0 & 8.6/13.4 & 94/13.4 & 11.3 & 9.9 \\ 
  \midrule\multirow{4}[2]{*}{msnr} & p=250 & 13.6/10.4/16.5 & 193.2/193.2/193.2/2.9 & 0.5/0/0.2 & 193.2 & 0 & 6.8/19.3 & 52.7/19.3 & 65.4 & 16.7 \\ 
   & p=500 & 3.8/3.2/4.4 & 195/195/195/0.9 & 0.2/0/0.1 & 195 & 0 & 5.9/7.3 & 82.8/7.3 & 7.7 & 5.1 \\ 
   & p=1000 & 2.9/2.1/1.8 & 196.4/196.3/196.4/0.4 & 0.1/0/0 & 196.3 & 0 & 5.5/6.2 & 95.5/6.2 & 5.2 & 4.8 \\ 
   & p=1500 & 3.9/2.7/1 & 197.2/197.2/197.2/0.4 & 0/0/0 & 197.1 & 0 & 6.8/8.8 & 97.8/8.8 & 7.3 & 6.1 \\ 
  \midrule\multirow{4}[2]{*}{lsnr} & p=250 & 0.2/0.1/0.6 & 194.1/194.1/194.1/0.3 & 0/0/0 & 194.1 & 0 & 4.5/4.4 & 51.1/4.4 & 4.2 & 3.3 \\ 
   & p=500 & 0.7/0.1/0.3 & 196.5/196.5/196.5/0.3 & 0/0/0 & 196.5 & 0 & 5.5/5.6 & 102.5/5.6 & 5.4 & 4.5 \\ 
   & p=1000 & 1.9/0.3/0.3 & 197.7/197.7/197.7/0.3 & 0/0/0 & 197.7 & 0 & 5.6/7.5 & 105.8/7.5 & 6 & 5.2 \\ 
   & p=1500 & 3.4/1.3/0.2 & 198.1/198.1/198.1/0.3 & 0/0/0 & 198.1 & 0 & 6.1/7.7 & 105.5/7.7 & 6.3 & 6 \\ 
   \bottomrule 
\end{tabular}
}
\end{table}
