# Supplementary material for: On the Use of Information Criteria for Subset Selection in Least Squares Regression
Source: arXiv:1911.10191 source file (2021-03-06)
Supplement: Supplementary file 40 [file Sparse-Ex3_rho_0.tex]

% latex table generated in R 4.0.3 by xtable 1.8-4 package
% Sun Feb 21 09:07:37 2021
\begin{table}[ht]
\centering
\caption{The performance of BOSS for high dimensional data, Sparse-Ex3, $\rho$=0, n=200} 
\scalebox{0.55}{
\begin{tabular}{|c|c|ccccccccc|}
  \toprule 
 \multicolumn{1}{|c}{} &       & BOSS  & FS    & FSstop & FStrim & FSstoptrim & lasso & Gamma lasso & SparseNet & rlasso \\
 \multicolumn{1}{|c}{} &       & C$_p$/AICc/CV & EBIC/HDBIC/HDHQ/CV & EBIC/HDBIC/HDHQ & HDBIC & HDBIC & AICc/CV & AICc/CV & CV    & CV  \\
 \cmidrule{3-11}\multicolumn{1}{|c}{} &       & \multicolumn{9}{c|}{\% worse than the best possible BOSS}  \\
 \midrule\multirow{4}[2]{*}{hsnr} & p=250 & 6/1/18 & 501/501/501/18 & 2/0/1 & 501 & 0 & 131/134 & 189/134 & 18 & 15 \\ 
   & p=500 & 24/2/18 & 501/501/501/19 & 2/0/1 & 501 & 0 & 151/155 & 364/155 & 23 & 17 \\ 
   & p=1000 & 74/12/20 & 501/501/501/20 & 2/0/0 & 501 & 0 & 173/179 & 417/179 & 24 & 16 \\ 
   & p=1500 & 128/40/19 & 501/501/501/21 & 2/0/0 & 501 & 0 & 185/193 & 430/193 & 27 & 15 \\ 
  \midrule\multirow{4}[2]{*}{msnr} & p=250 & 21/10/19 & 498/498/498/19 & 6/221/10 & 498 & 223 & 130/133 & 313/133 & 20 & 20 \\ 
   & p=500 & 57/24/20 & 496/496/496/21 & 9/383/21 & 496 & 385 & 149/153 & 448/153 & 25 & 26 \\ 
   & p=1000 & 134/63/24 & 494/494/494/24 & 13/509/45 & 494 & 510 & 170/177 & 464/177 & 29 & 36 \\ 
   & p=1500 & 194/121/24 & 493/493/493/26 & 17/553/64 & 493 & 553 & 181/190 & 467/190 & 29 & 42 \\ 
  \midrule\multirow{4}[2]{*}{lsnr} & p=250 & 18/18/15 & 168/168/168/15 & 19/24/21 & 168 & 24 & -4/0 & 124/0 & 3 & 2 \\ 
   & p=500 & 24/14/13 & 154/154/154/12 & 14/18/16 & 154 & 18 & -3/0 & 148/0 & 4 & 3 \\ 
   & p=1000 & 37/18/10 & 144/144/144/10 & 11/13/12 & 144 & 13 & -3/2 & 140/2 & 4 & 4 \\ 
   & p=1500 & 46/29/9 & 139/139/139/10 & 9/11/10 & 139 & 11 & -3/3 & 137/3 & 5 & 5 \\ 
   \midrule 
 \multicolumn{1}{|c}{} &       & \multicolumn{9}{c|}{Relative efficiency} \\
\midrule\multirow{4}[2]{*}{hsnr} & p=250 & 0.95/0.99/0.85 & 0.17/0.17/0.17/0.85 & 0.98/1/0.99 & 0.17 & 1 & 0.43/0.43 & 0.35/0.43 & 0.85 & 0.87 \\ 
   & p=500 & 0.81/0.98/0.85 & 0.17/0.17/0.17/0.84 & 0.98/1/0.99 & 0.17 & 1 & 0.4/0.39 & 0.22/0.39 & 0.81 & 0.86 \\ 
   & p=1000 & 0.58/0.9/0.84 & 0.17/0.17/0.17/0.83 & 0.98/1/1 & 0.17 & 1 & 0.37/0.36 & 0.19/0.36 & 0.8 & 0.86 \\ 
   & p=1500 & 0.44/0.72/0.84 & 0.17/0.17/0.17/0.83 & 0.98/1/1 & 0.17 & 1 & 0.35/0.34 & 0.19/0.34 & 0.79 & 0.87 \\ 
  \midrule\multirow{4}[2]{*}{msnr} & p=250 & 0.88/0.96/0.89 & 0.18/0.18/0.18/0.89 & 1/0.33/0.96 & 0.18 & 0.33 & 0.46/0.46 & 0.26/0.46 & 0.88 & 0.88 \\ 
   & p=500 & 0.69/0.88/0.91 & 0.18/0.18/0.18/0.91 & 1/0.23/0.91 & 0.18 & 0.23 & 0.44/0.43 & 0.2/0.43 & 0.88 & 0.87 \\ 
   & p=1000 & 0.48/0.69/0.91 & 0.19/0.19/0.19/0.91 & 1/0.19/0.78 & 0.19 & 0.19 & 0.42/0.41 & 0.2/0.41 & 0.88 & 0.83 \\ 
   & p=1500 & 0.4/0.53/0.94 & 0.2/0.2/0.2/0.93 & 1/0.18/0.71 & 0.2 & 0.18 & 0.42/0.4 & 0.21/0.4 & 0.91 & 0.83 \\ 
  \midrule\multirow{4}[2]{*}{lsnr} & p=250 & 0.82/0.82/0.84 & 0.36/0.36/0.36/0.84 & 0.81/0.78/0.8 & 0.36 & 0.78 & 1/0.97 & 0.43/0.97 & 0.94 & 0.94 \\ 
   & p=500 & 0.78/0.84/0.86 & 0.38/0.38/0.38/0.86 & 0.84/0.82/0.83 & 0.38 & 0.82 & 1/0.97 & 0.39/0.97 & 0.93 & 0.94 \\ 
   & p=1000 & 0.71/0.82/0.88 & 0.4/0.4/0.4/0.88 & 0.88/0.86/0.87 & 0.4 & 0.86 & 1/0.95 & 0.4/0.95 & 0.94 & 0.94 \\ 
   & p=1500 & 0.67/0.75/0.89 & 0.41/0.41/0.41/0.89 & 0.89/0.88/0.88 & 0.41 & 0.88 & 1/0.95 & 0.41/0.95 & 0.93 & 0.93 \\ 
   \midrule 
 \multicolumn{1}{|c}{} &       & \multicolumn{9}{c|}{Sparsistency} \\
\midrule\multirow{4}[2]{*}{hsnr} & p=250 & 6/6/6 & 6/6/6/6 & 6/6/6 & 6 & 6 & 6/6 & 6/6 & 6 & 6 \\ 
   & p=500 & 6/6/6 & 6/6/6/6 & 6/6/6 & 6 & 6 & 6/6 & 6/6 & 6 & 6 \\ 
   & p=1000 & 6/6/6 & 6/6/6/6 & 6/6/6 & 6 & 6 & 6/6 & 6/6 & 6 & 6 \\ 
   & p=1500 & 6/6/6 & 6/6/6/6 & 6/6/6 & 6 & 6 & 6/6 & 6/6 & 6 & 6 \\ 
  \midrule\multirow{4}[2]{*}{msnr} & p=250 & 6/6/6 & 6/6/6/6 & 6/4.2/5.9 & 6 & 4.2 & 6/6 & 6/6 & 6 & 6 \\ 
   & p=500 & 6/6/6 & 6/6/6/6 & 5.9/2.7/5.9 & 6 & 2.7 & 6/6 & 6/6 & 6 & 6 \\ 
   & p=1000 & 6/6/6 & 6/6/6/6 & 5.9/1.4/5.7 & 6 & 1.4 & 6/6 & 6/6 & 6 & 6 \\ 
   & p=1500 & 6/6/6 & 6/6/6/6 & 5.9/0.9/5.5 & 6 & 0.9 & 6/6 & 6/6 & 6 & 6 \\ 
  \midrule\multirow{4}[2]{*}{lsnr} & p=250 & 1.2/0.7/1.4 & 5.6/5.6/5.6/1.4 & 0.5/0/0.3 & 5.6 & 0 & 3.9/3.9 & 4.5/3.9 & 3.3 & 3.1 \\ 
   & p=500 & 1.3/0.7/1 & 4.4/4.4/4.4/1 & 0.3/0/0.1 & 4.4 & 0 & 3.3/3.4 & 4/3.4 & 2.8 & 2.6 \\ 
   & p=1000 & 1.3/0.8/0.7 & 3.2/3.2/3.2/0.7 & 0.2/0/0.1 & 3.2 & 0 & 2.6/2.8 & 3.1/2.8 & 2.3 & 2.2 \\ 
   & p=1500 & 1.3/0.9/0.6 & 2.6/2.6/2.6/0.6 & 0.2/0/0.1 & 2.6 & 0 & 2.4/2.4 & 2.7/2.4 & 2 & 2 \\ 
   \midrule 
 \multicolumn{1}{|c}{} &       & \multicolumn{9}{c|}{Number of extra variables} \\
\midrule\multirow{4}[2]{*}{hsnr} & p=250 & 0.4/0/0.3 & 193/193/193/0.3 & 0/0/0 & 193 & 0 & 15.1/22.3 & 29.1/22.3 & 2.5 & 0.5 \\ 
   & p=500 & 1.4/0/0.3 & 193/193/193/0.3 & 0/0/0 & 193 & 0 & 17.1/27.7 & 74.4/27.7 & 3.6 & 0.8 \\ 
   & p=1000 & 3.9/0.4/0.3 & 193/193/193/0.3 & 0/0/0 & 193 & 0 & 19.2/35.4 & 87.2/35.4 & 4.2 & 0.8 \\ 
   & p=1500 & 6.8/1.9/0.2 & 193/193/193/0.3 & 0/0/0 & 192.9 & 0 & 19.3/40.1 & 89.7/40.1 & 4.7 & 0.8 \\ 
  \midrule\multirow{4}[2]{*}{msnr} & p=250 & 0.6/0.1/0.3 & 193/193/193/0.3 & 0/0/0 & 193 & 0 & 15.1/22.3 & 49.9/22.3 & 1.7 & 0.6 \\ 
   & p=500 & 2/0.3/0.3 & 193/193/193/0.3 & 0/0/0 & 193 & 0 & 17.2/27.7 & 97.2/27.7 & 2.4 & 1.2 \\ 
   & p=1000 & 5.4/1.4/0.3 & 193/193/193/0.3 & 0/0/0 & 193 & 0 & 18.9/35.8 & 100.1/35.8 & 2.7 & 1.3 \\ 
   & p=1500 & 8.3/3.8/0.3 & 193/193/193/0.3 & 0/0/0 & 192.9 & 0 & 19.4/40.4 & 99.6/40.4 & 2.6 & 1.8 \\ 
  \midrule\multirow{4}[2]{*}{lsnr} & p=250 & 1/0.1/0.5 & 193.4/193.4/193.4/0.5 & 0/0/0 & 193.4 & 0 & 10.8/14.6 & 69.8/14.6 & 10.3 & 7 \\ 
   & p=500 & 2.6/0.2/0.5 & 194.6/194.6/194.6/0.4 & 0/0/0 & 194.6 & 0 & 11.3/15.7 & 113.8/15.7 & 11 & 8.2 \\ 
   & p=1000 & 6.1/1.5/0.3 & 195.8/195.8/195.8/0.3 & 0/0/0 & 195.8 & 0 & 11.2/18.9 & 113.7/18.9 & 13.5 & 10.2 \\ 
   & p=1500 & 8/4/0.3 & 196.3/196.3/196.3/0.3 & 0/0/0 & 196.3 & 0 & 11.1/20 & 111.8/20 & 14.5 & 11.4 \\ 
   \bottomrule 
\end{tabular}
}
\end{table}
