# Supplementary material for: On the Use of Information Criteria for Subset Selection in Least Squares Regression
Source: arXiv:1911.10191 source file (2021-03-06)
Supplement: Supplementary file 41 [file Sparse-Ex3_rho_05.tex]

% latex table generated in R 4.0.3 by xtable 1.8-4 package
% Sun Feb 21 09:09:11 2021
\begin{table}[ht]
\centering
\caption{The performance of BOSS for high dimensional data, Sparse-Ex3, $\rho$=0.5, n=200} 
\scalebox{0.55}{
\begin{tabular}{|c|c|ccccccccc|}
  \toprule 
 \multicolumn{1}{|c}{} &       & BOSS  & FS    & FSstop & FStrim & FSstoptrim & lasso & Gamma lasso & SparseNet & rlasso \\
 \multicolumn{1}{|c}{} &       & C$_p$/AICc/CV & EBIC/HDBIC/HDHQ/CV & EBIC/HDBIC/HDHQ & HDBIC & HDBIC & AICc/CV & AICc/CV & CV    & CV  \\
 \cmidrule{3-11}\multicolumn{1}{|c}{} &       & \multicolumn{9}{c|}{\% worse than the best possible BOSS}  \\
 \midrule\multirow{4}[2]{*}{hsnr} & p=250 & 6/1/16 & 495/495/495/19 & 2/0/1 & 495 & 0 & 135/137 & 182/137 & 19 & 16 \\ 
   & p=500 & 24/2/18 & 495/495/495/20 & 2/0/1 & 495 & 0 & 156/159 & 356/159 & 24 & 16 \\ 
   & p=1000 & 79/11/19 & 495/495/495/20 & 2/0/0 & 495 & 0 & 179/185 & 412/185 & 25 & 15 \\ 
   & p=1500 & 124/44/18 & 495/495/495/20 & 2/0/0 & 495 & 0 & 191/199 & 425/199 & 26 & 14 \\ 
  \midrule\multirow{4}[2]{*}{msnr} & p=250 & 22/11/18 & 492/492/492/20 & 4/234/8 & 492 & 236 & 134/136 & 304/136 & 19 & 24 \\ 
   & p=500 & 61/26/19 & 490/490/490/22 & 7/408/19 & 490 & 409 & 153/157 & 441/157 & 24 & 33 \\ 
   & p=1000 & 133/62/23 & 488/488/488/24 & 11/515/41 & 488 & 515 & 176/182 & 458/182 & 27 & 46 \\ 
   & p=1500 & 190/122/22 & 486/486/486/24 & 15/549/63 & 486 & 549 & 187/195 & 460/195 & 27 & 56 \\ 
  \midrule\multirow{4}[2]{*}{lsnr} & p=250 & 17/17/14 & 166/166/166/14 & 17/21/19 & 166 & 21 & -3/0 & 122/0 & 4 & 3 \\ 
   & p=500 & 23/13/12 & 153/153/153/12 & 13/15/14 & 153 & 15 & -3/1 & 148/1 & 4 & 3 \\ 
   & p=1000 & 35/17/10 & 144/144/144/10 & 9/11/10 & 144 & 11 & -3/2 & 141/2 & 4 & 4 \\ 
   & p=1500 & 44/28/9 & 140/140/140/9 & 8/9/9 & 140 & 9 & -2/3 & 138/3 & 5 & 6 \\ 
   \midrule 
 \multicolumn{1}{|c}{} &       & \multicolumn{9}{c|}{Relative efficiency} \\
\midrule\multirow{4}[2]{*}{hsnr} & p=250 & 0.95/0.99/0.86 & 0.17/0.17/0.17/0.84 & 0.98/1/0.99 & 0.17 & 1 & 0.43/0.42 & 0.35/0.42 & 0.84 & 0.86 \\ 
   & p=500 & 0.8/0.98/0.85 & 0.17/0.17/0.17/0.83 & 0.98/1/0.99 & 0.17 & 1 & 0.39/0.39 & 0.22/0.39 & 0.81 & 0.86 \\ 
   & p=1000 & 0.56/0.9/0.84 & 0.17/0.17/0.17/0.84 & 0.98/1/1 & 0.17 & 1 & 0.36/0.35 & 0.2/0.35 & 0.8 & 0.87 \\ 
   & p=1500 & 0.45/0.7/0.85 & 0.17/0.17/0.17/0.84 & 0.98/1/1 & 0.17 & 1 & 0.34/0.33 & 0.19/0.33 & 0.79 & 0.88 \\ 
  \midrule\multirow{4}[2]{*}{msnr} & p=250 & 0.86/0.94/0.89 & 0.18/0.18/0.18/0.87 & 1/0.31/0.96 & 0.18 & 0.31 & 0.45/0.44 & 0.26/0.44 & 0.87 & 0.84 \\ 
   & p=500 & 0.67/0.85/0.9 & 0.18/0.18/0.18/0.88 & 1/0.21/0.9 & 0.18 & 0.21 & 0.42/0.42 & 0.2/0.42 & 0.87 & 0.81 \\ 
   & p=1000 & 0.48/0.68/0.9 & 0.19/0.19/0.19/0.9 & 1/0.18/0.79 & 0.19 & 0.18 & 0.4/0.39 & 0.2/0.39 & 0.88 & 0.76 \\ 
   & p=1500 & 0.39/0.52/0.94 & 0.2/0.2/0.2/0.92 & 1/0.18/0.7 & 0.2 & 0.18 & 0.4/0.39 & 0.2/0.39 & 0.9 & 0.73 \\ 
  \midrule\multirow{4}[2]{*}{lsnr} & p=250 & 0.83/0.83/0.85 & 0.36/0.36/0.36/0.85 & 0.83/0.8/0.82 & 0.36 & 0.8 & 1/0.97 & 0.44/0.97 & 0.94 & 0.95 \\ 
   & p=500 & 0.79/0.86/0.87 & 0.38/0.38/0.38/0.87 & 0.86/0.84/0.85 & 0.38 & 0.84 & 1/0.96 & 0.39/0.96 & 0.94 & 0.94 \\ 
   & p=1000 & 0.72/0.83/0.89 & 0.4/0.4/0.4/0.89 & 0.89/0.88/0.88 & 0.4 & 0.88 & 1/0.96 & 0.41/0.96 & 0.94 & 0.93 \\ 
   & p=1500 & 0.68/0.76/0.9 & 0.41/0.41/0.41/0.9 & 0.9/0.89/0.9 & 0.41 & 0.89 & 1/0.95 & 0.41/0.95 & 0.93 & 0.92 \\ 
   \midrule 
 \multicolumn{1}{|c}{} &       & \multicolumn{9}{c|}{Sparsistency} \\
\midrule\multirow{4}[2]{*}{hsnr} & p=250 & 6/6/6 & 6/6/6/6 & 6/6/6 & 6 & 6 & 6/6 & 6/6 & 6 & 6 \\ 
   & p=500 & 6/6/6 & 6/6/6/6 & 6/6/6 & 6 & 6 & 6/6 & 6/6 & 6 & 6 \\ 
   & p=1000 & 6/6/6 & 6/6/6/6 & 6/6/6 & 6 & 6 & 6/6 & 6/6 & 6 & 6 \\ 
   & p=1500 & 6/6/6 & 6/6/6/6 & 6/6/6 & 6 & 6 & 6/6 & 6/6 & 6 & 6 \\ 
  \midrule\multirow{4}[2]{*}{msnr} & p=250 & 6/6/6 & 6/6/6/6 & 6/4/5.9 & 6 & 4 & 6/6 & 6/6 & 6 & 6 \\ 
   & p=500 & 6/6/6 & 6/6/6/6 & 6/2.3/5.9 & 6 & 2.3 & 6/6 & 6/6 & 6 & 6 \\ 
   & p=1000 & 6/6/6 & 6/6/6/6 & 5.9/1.2/5.7 & 6 & 1.2 & 6/6 & 6/6 & 6 & 6 \\ 
   & p=1500 & 6/6/6 & 6/6/6/6 & 5.9/0.8/5.5 & 6 & 0.8 & 6/6 & 6/6 & 6 & 5.9 \\ 
  \midrule\multirow{4}[2]{*}{lsnr} & p=250 & 1.1/0.6/1.2 & 5.5/5.5/5.5/1.3 & 0.4/0/0.2 & 5.5 & 0 & 3.6/3.6 & 4.3/3.6 & 3 & 2.9 \\ 
   & p=500 & 1.2/0.5/0.9 & 4.2/4.2/4.2/0.9 & 0.3/0/0.1 & 4.2 & 0 & 3/3 & 3.8/3 & 2.6 & 2.4 \\ 
   & p=1000 & 1.1/0.7/0.6 & 3/3/3/0.6 & 0.2/0/0.1 & 3 & 0 & 2.3/2.4 & 2.9/2.4 & 2.1 & 2 \\ 
   & p=1500 & 1.2/0.8/0.5 & 2.5/2.5/2.5/0.5 & 0.2/0/0 & 2.5 & 0 & 2.1/2.2 & 2.5/2.2 & 1.9 & 1.7 \\ 
   \midrule 
 \multicolumn{1}{|c}{} &       & \multicolumn{9}{c|}{Number of extra variables} \\
\midrule\multirow{4}[2]{*}{hsnr} & p=250 & 0.3/0/0.3 & 193/193/193/0.3 & 0/0/0 & 193 & 0 & 15.8/23.3 & 28.2/23.3 & 2.6 & 0.5 \\ 
   & p=500 & 1.4/0/0.3 & 193/193/193/0.3 & 0/0/0 & 193 & 0 & 17.7/29.6 & 73.4/29.6 & 3.7 & 0.6 \\ 
   & p=1000 & 4.4/0.4/0.3 & 193/193/193/0.3 & 0/0/0 & 193 & 0 & 19.6/37.8 & 87.6/37.8 & 4.1 & 0.6 \\ 
   & p=1500 & 6.7/2.2/0.2 & 193/193/193/0.3 & 0/0/0 & 192.9 & 0 & 20.4/42.7 & 89.5/42.7 & 4.6 & 0.5 \\ 
  \midrule\multirow{4}[2]{*}{msnr} & p=250 & 0.5/0.1/0.3 & 193/193/193/0.3 & 0/0/0 & 193 & 0 & 15.9/23.3 & 48.6/23.3 & 1.6 & 0.8 \\ 
   & p=500 & 2.3/0.4/0.3 & 193/193/193/0.3 & 0/0/0 & 193 & 0 & 18/29.7 & 96.8/29.7 & 2.2 & 1.7 \\ 
   & p=1000 & 5.5/1.4/0.3 & 193/193/193/0.3 & 0/0/0 & 193 & 0 & 19.6/37.9 & 100.4/37.9 & 2.5 & 1.8 \\ 
   & p=1500 & 8.4/3.9/0.3 & 193/193/193/0.3 & 0/0/0 & 192.9 & 0 & 20.6/43 & 99.7/43 & 2.5 & 2.4 \\ 
  \midrule\multirow{4}[2]{*}{lsnr} & p=250 & 0.8/0.1/0.5 & 193.5/193.5/193.5/0.5 & 0/0/0 & 193.5 & 0 & 10.3/14.4 & 69.3/14.4 & 10.3 & 7.1 \\ 
   & p=500 & 2.9/0.2/0.4 & 194.8/194.8/194.8/0.4 & 0/0/0 & 194.8 & 0 & 11.2/15.8 & 114.6/15.8 & 11.2 & 8.6 \\ 
   & p=1000 & 5.7/1.5/0.4 & 196/196/196/0.4 & 0/0/0 & 196 & 0 & 10.9/18.1 & 113.7/18.1 & 13.8 & 10.1 \\ 
   & p=1500 & 7.6/3.8/0.3 & 196.5/196.5/196.5/0.3 & 0/0/0 & 196.4 & 0 & 10.7/18.8 & 112.5/18.8 & 14.1 & 12 \\ 
   \bottomrule 
\end{tabular}
}
\end{table}
