# Supplementary material for: On the Use of Information Criteria for Subset Selection in Least Squares Regression
Source: arXiv:1911.10191 source file (2021-03-06)
Supplement: Supplementary file 42 [file Sparse-Ex3_rho_09.tex]

% latex table generated in R 4.0.3 by xtable 1.8-4 package
% Sun Feb 21 09:10:46 2021
\begin{table}[ht]
\centering
\caption{The performance of BOSS for high dimensional data, Sparse-Ex3, $\rho$=0.9, n=200} 
\scalebox{0.55}{
\begin{tabular}{|c|c|ccccccccc|}
  \toprule 
 \multicolumn{1}{|c}{} &       & BOSS  & FS    & FSstop & FStrim & FSstoptrim & lasso & Gamma lasso & SparseNet & rlasso \\
 \multicolumn{1}{|c}{} &       & C$_p$/AICc/CV & EBIC/HDBIC/HDHQ/CV & EBIC/HDBIC/HDHQ & HDBIC & HDBIC & AICc/CV & AICc/CV & CV    & CV  \\
 \cmidrule{3-11}\multicolumn{1}{|c}{} &       & \multicolumn{9}{c|}{\% worse than the best possible BOSS}  \\
 \midrule\multirow{4}[2]{*}{hsnr} & p=250 & 8/3/30 & 477/477/477/33 & 3/13/4 & 477 & 13 & 135/137 & 167/137 & 17 & 16 \\ 
   & p=500 & 28/6/33 & 476/476/476/34 & 4/13/7 & 476 & 13 & 156/159 & 334/159 & 22 & 17 \\ 
   & p=1000 & 85/17/34 & 475/475/475/35 & 6/13/9 & 475 & 13 & 179/183 & 393/183 & 22 & 17 \\ 
   & p=1500 & 123/52/32 & 474/474/474/34 & 6/13/10 & 474 & 13 & 191/196 & 405/196 & 24 & 18 \\ 
  \midrule\multirow{4}[2]{*}{msnr} & p=250 & 15/7/12 & 367/367/367/13 & 2/172/4 & 367 & 172 & 91/92 & 217/92 & 3 & 13 \\ 
   & p=500 & 44/17/13 & 366/366/366/13 & 4/315/11 & 366 & 315 & 107/110 & 327/110 & 5 & 21 \\ 
   & p=1000 & 103/44/15 & 365/365/365/17 & 7/401/27 & 365 & 401 & 126/130 & 342/130 & 10 & 37 \\ 
   & p=1500 & 140/92/16 & 364/364/364/17 & 9/426/42 & 364 & 426 & 135/139 & 343/139 & 11 & 45 \\ 
  \midrule\multirow{4}[2]{*}{lsnr} & p=250 & 16/15/14 & 164/164/164/14 & 16/18/17 & 164 & 18 & -3/0 & 118/0 & 3 & 3 \\ 
   & p=500 & 21/12/11 & 151/151/151/11 & 11/12/12 & 151 & 12 & -3/0 & 145/0 & 2 & 3 \\ 
   & p=1000 & 33/15/9 & 142/142/142/9 & 8/9/8 & 142 & 9 & -3/2 & 139/2 & 4 & 4 \\ 
   & p=1500 & 41/27/8 & 139/139/139/8 & 7/7/7 & 139 & 7 & -3/2 & 136/2 & 4 & 6 \\ 
   \midrule 
 \multicolumn{1}{|c}{} &       & \multicolumn{9}{c|}{Relative efficiency} \\
\midrule\multirow{4}[2]{*}{hsnr} & p=250 & 0.96/1/0.79 & 0.18/0.18/0.18/0.77 & 1/0.91/0.99 & 0.18 & 0.91 & 0.44/0.43 & 0.39/0.43 & 0.88 & 0.89 \\ 
   & p=500 & 0.81/0.99/0.79 & 0.18/0.18/0.18/0.78 & 1/0.92/0.98 & 0.18 & 0.92 & 0.41/0.4 & 0.24/0.4 & 0.86 & 0.89 \\ 
   & p=1000 & 0.57/0.91/0.79 & 0.18/0.18/0.18/0.78 & 1/0.94/0.97 & 0.18 & 0.94 & 0.38/0.37 & 0.21/0.37 & 0.87 & 0.91 \\ 
   & p=1500 & 0.47/0.7/0.8 & 0.18/0.18/0.18/0.79 & 1/0.94/0.96 & 0.18 & 0.94 & 0.36/0.36 & 0.21/0.36 & 0.85 & 0.9 \\ 
  \midrule\multirow{4}[2]{*}{msnr} & p=250 & 0.89/0.96/0.91 & 0.22/0.22/0.22/0.9 & 1/0.38/0.98 & 0.22 & 0.38 & 0.54/0.53 & 0.32/0.53 & 0.99 & 0.91 \\ 
   & p=500 & 0.72/0.88/0.92 & 0.22/0.22/0.22/0.91 & 1/0.25/0.93 & 0.22 & 0.25 & 0.5/0.49 & 0.24/0.49 & 0.99 & 0.86 \\ 
   & p=1000 & 0.53/0.74/0.93 & 0.23/0.23/0.23/0.92 & 1/0.21/0.84 & 0.23 & 0.21 & 0.47/0.47 & 0.24/0.47 & 0.98 & 0.78 \\ 
   & p=1500 & 0.45/0.57/0.94 & 0.23/0.23/0.23/0.93 & 1/0.21/0.77 & 0.23 & 0.21 & 0.46/0.46 & 0.25/0.46 & 0.98 & 0.75 \\ 
  \midrule\multirow{4}[2]{*}{lsnr} & p=250 & 0.83/0.84/0.85 & 0.37/0.37/0.37/0.85 & 0.84/0.82/0.83 & 0.37 & 0.82 & 1/0.97 & 0.45/0.97 & 0.94 & 0.94 \\ 
   & p=500 & 0.8/0.87/0.87 & 0.38/0.38/0.38/0.87 & 0.87/0.86/0.86 & 0.38 & 0.86 & 1/0.97 & 0.39/0.97 & 0.94 & 0.94 \\ 
   & p=1000 & 0.73/0.84/0.89 & 0.4/0.4/0.4/0.89 & 0.9/0.89/0.89 & 0.4 & 0.89 & 1/0.95 & 0.41/0.95 & 0.93 & 0.93 \\ 
   & p=1500 & 0.69/0.76/0.9 & 0.41/0.41/0.41/0.9 & 0.91/0.91/0.91 & 0.41 & 0.91 & 1/0.95 & 0.41/0.95 & 0.93 & 0.92 \\ 
   \midrule 
 \multicolumn{1}{|c}{} &       & \multicolumn{9}{c|}{Sparsistency} \\
\midrule\multirow{4}[2]{*}{hsnr} & p=250 & 6/6/6 & 6/6/6/6 & 6/5.9/6 & 6 & 5.9 & 6/6 & 6/6 & 6 & 6 \\ 
   & p=500 & 6/6/6 & 6/6/6/6 & 6/5.9/6 & 6 & 5.9 & 6/6 & 6/6 & 6 & 6 \\ 
   & p=1000 & 6/6/6 & 6/6/6/6 & 6/5.9/5.9 & 6 & 5.9 & 6/6 & 5.9/6 & 6 & 6 \\ 
   & p=1500 & 6/6/6 & 6/6/6/6 & 6/5.9/5.9 & 6 & 5.9 & 6/6 & 5.9/6 & 6 & 6 \\ 
  \midrule\multirow{4}[2]{*}{msnr} & p=250 & 5.5/5.5/5.5 & 5.9/5.9/5.9/5.5 & 5.5/3.7/5.5 & 5.9 & 3.7 & 6/6 & 5.6/6 & 5.8 & 5.9 \\ 
   & p=500 & 5.5/5.5/5.5 & 5.8/5.8/5.8/5.5 & 5.5/2/5.4 & 5.8 & 2 & 6/6 & 5.6/6 & 5.8 & 5.9 \\ 
   & p=1000 & 5.5/5.5/5.5 & 5.6/5.6/5.6/5.5 & 5.5/0.9/5.3 & 5.6 & 0.9 & 6/6 & 5.5/6 & 5.8 & 5.8 \\ 
   & p=1500 & 5.5/5.5/5.5 & 5.6/5.6/5.6/5.5 & 5.5/0.6/5.1 & 5.6 & 0.6 & 5.9/6 & 5.5/6 & 5.8 & 5.8 \\ 
  \midrule\multirow{4}[2]{*}{lsnr} & p=250 & 0.8/0.5/1 & 5.2/5.2/5.2/1 & 0.3/0/0.2 & 5.2 & 0 & 3/3 & 3.5/3 & 2.6 & 2.4 \\ 
   & p=500 & 0.9/0.4/0.7 & 3.7/3.7/3.7/0.7 & 0.2/0/0.1 & 3.7 & 0 & 2.4/2.4 & 3.1/2.4 & 2.2 & 2 \\ 
   & p=1000 & 0.9/0.5/0.5 & 2.6/2.6/2.6/0.5 & 0.1/0/0 & 2.6 & 0 & 1.9/1.9 & 2.3/1.9 & 1.8 & 1.6 \\ 
   & p=1500 & 0.9/0.7/0.4 & 2.1/2.1/2.1/0.4 & 0.1/0/0 & 2.1 & 0 & 1.6/1.7 & 2/1.7 & 1.5 & 1.4 \\ 
   \midrule 
 \multicolumn{1}{|c}{} &       & \multicolumn{9}{c|}{Number of extra variables} \\
\midrule\multirow{4}[2]{*}{hsnr} & p=250 & 0.3/0.1/0.6 & 193/193/193/0.7 & 0.1/0.1/0.1 & 193 & 0.1 & 17.2/25.2 & 26.8/25.2 & 2.8 & 0.8 \\ 
   & p=500 & 1.6/0.1/0.7 & 193/193/193/0.6 & 0.1/0.1/0.1 & 193 & 0.1 & 19.1/32.2 & 71.2/32.2 & 4 & 0.8 \\ 
   & p=1000 & 5/0.7/0.6 & 193/193/193/0.6 & 0.1/0.1/0.1 & 193 & 0.1 & 21.2/40.2 & 87.3/40.2 & 4.6 & 0.8 \\ 
   & p=1500 & 7.3/2.8/0.5 & 193/193/193/0.5 & 0.1/0.1/0.1 & 192.9 & 0.1 & 22/45 & 89.8/45 & 5.4 & 1 \\ 
  \midrule\multirow{4}[2]{*}{msnr} & p=250 & 1/0.6/0.8 & 193.1/193.1/193.1/0.8 & 0.5/0.3/0.5 & 193.1 & 0.3 & 17.2/25.1 & 47.5/25.1 & 2 & 2 \\ 
   & p=500 & 2.7/0.8/0.8 & 193.2/193.2/193.2/0.8 & 0.5/0.1/0.5 & 193.2 & 0.1 & 19.1/32.2 & 97.3/32.2 & 2.2 & 2.6 \\ 
   & p=1000 & 6.6/1.9/0.8 & 193.4/193.3/193.4/0.8 & 0.5/0/0.4 & 193.3 & 0 & 21.1/40.6 & 100.4/40.6 & 3 & 3.4 \\ 
   & p=1500 & 9.1/4.8/0.8 & 193.4/193.4/193.4/0.8 & 0.5/0/0.4 & 193.3 & 0 & 21.8/44.9 & 100.5/44.9 & 3.3 & 4 \\ 
  \midrule\multirow{4}[2]{*}{lsnr} & p=250 & 1/0.2/0.8 & 193.8/193.8/193.8/0.9 & 0.1/0/0 & 193.8 & 0 & 11.2/14.5 & 68.1/14.5 & 10.9 & 8.1 \\ 
   & p=500 & 2.9/0.3/0.6 & 195.3/195.3/195.3/0.6 & 0/0/0 & 195.3 & 0 & 11.3/15.9 & 114.2/15.9 & 11.5 & 8.8 \\ 
   & p=1000 & 5.9/1.4/0.5 & 196.4/196.4/196.4/0.5 & 0/0/0 & 196.4 & 0 & 11.2/18.2 & 114.5/18.2 & 14 & 11 \\ 
   & p=1500 & 7.6/4.2/0.4 & 196.9/196.9/196.9/0.4 & 0/0/0 & 196.8 & 0 & 10.9/19.3 & 112.4/19.3 & 14.3 & 12.6 \\ 
   \bottomrule 
\end{tabular}
}
\end{table}
