# Supplementary material for: On the Use of Information Criteria for Subset Selection in Least Squares Regression
Source: arXiv:1911.10191 source file (2021-03-06)
Supplement: Supplementary file 43 [file Sparse-Ex4_rho_0.tex]

% latex table generated in R 4.0.3 by xtable 1.8-4 package
% Sun Feb 21 09:11:08 2021
\begin{table}[ht]
\centering
\caption{The performance of BOSS for high dimensional data, Sparse-Ex4, $\rho$=0, n=200} 
\scalebox{0.55}{
\begin{tabular}{|c|c|ccccccccc|}
  \toprule 
 \multicolumn{1}{|c}{} &       & BOSS  & FS    & FSstop & FStrim & FSstoptrim & lasso & Gamma lasso & SparseNet & rlasso \\
 \multicolumn{1}{|c}{} &       & C$_p$/AICc/CV & EBIC/HDBIC/HDHQ/CV & EBIC/HDBIC/HDHQ & HDBIC & HDBIC & AICc/CV & AICc/CV & CV    & CV  \\
 \cmidrule{3-11}\multicolumn{1}{|c}{} &       & \multicolumn{9}{c|}{\% worse than the best possible BOSS}  \\
 \midrule\multirow{4}[2]{*}{hsnr} & p=250 & 10/6/13 & 302/302/302/13 & 6/5/6 & 302 & 5 & 63/63 & 234/63 & 11 & 16 \\ 
   & p=500 & 23/6/11 & 294/294/294/12 & 4/3/4 & 294 & 3 & 73/75 & 281/75 & 12 & 16 \\ 
   & p=1000 & 56/13/12 & 289/289/289/12 & 3/2/2 & 289 & 2 & 84/87 & 280/87 & 13 & 12 \\ 
   & p=1500 & 78/31/11 & 286/286/286/11 & 3/1/2 & 286 & 1 & 90/93 & 278/93 & 13 & 12 \\ 
  \midrule\multirow{4}[2]{*}{msnr} & p=250 & 33/30/29 & 452/452/452/29 & 39/153/58 & 452 & 153 & 108/109 & 363/109 & 29 & 74 \\ 
   & p=500 & 65/36/31 & 427/427/427/31 & 46/155/75 & 427 & 155 & 115/119 & 421/119 & 35 & 86 \\ 
   & p=1000 & 116/62/36 & 399/399/399/37 & 51/150/89 & 399 & 150 & 119/127 & 396/127 & 38 & 95 \\ 
   & p=1500 & 153/109/38 & 386/386/386/37 & 55/146/95 & 386 & 146 & 122/131 & 383/131 & 41 & 100 \\ 
  \midrule\multirow{4}[2]{*}{lsnr} & p=250 & 35/35/28 & 275/275/275/28 & 38/47/42 & 275 & 47 & 19/22 & 201/22 & 21 & 23 \\ 
   & p=500 & 39/27/23 & 244/244/244/23 & 29/35/32 & 244 & 35 & 14/19 & 242/19 & 19 & 21 \\ 
   & p=1000 & 51/27/19 & 217/217/217/19 & 21/24/23 & 217 & 24 & 10/16 & 217/16 & 16 & 19 \\ 
   & p=1500 & 63/40/17 & 207/207/207/18 & 18/20/20 & 207 & 20 & 9/15 & 206/15 & 14 & 19 \\ 
   \midrule 
 \multicolumn{1}{|c}{} &       & \multicolumn{9}{c|}{Relative efficiency} \\
\midrule\multirow{4}[2]{*}{hsnr} & p=250 & 0.96/0.99/0.93 & 0.26/0.26/0.26/0.93 & 0.99/1/1 & 0.26 & 1 & 0.65/0.65 & 0.32/0.65 & 0.95 & 0.91 \\ 
   & p=500 & 0.84/0.98/0.93 & 0.26/0.26/0.26/0.92 & 0.99/1/1 & 0.26 & 1 & 0.6/0.59 & 0.27/0.59 & 0.92 & 0.89 \\ 
   & p=1000 & 0.65/0.9/0.91 & 0.26/0.26/0.26/0.91 & 0.99/1/1 & 0.26 & 1 & 0.55/0.54 & 0.27/0.54 & 0.9 & 0.91 \\ 
   & p=1500 & 0.57/0.78/0.91 & 0.26/0.26/0.26/0.91 & 0.99/1/1 & 0.26 & 1 & 0.53/0.52 & 0.27/0.52 & 0.89 & 0.91 \\ 
  \midrule\multirow{4}[2]{*}{msnr} & p=250 & 0.97/0.99/1 & 0.23/0.23/0.23/1 & 0.93/0.51/0.81 & 0.23 & 0.51 & 0.62/0.62 & 0.28/0.62 & 0.99 & 0.74 \\ 
   & p=500 & 0.79/0.96/1 & 0.25/0.25/0.25/1 & 0.89/0.51/0.75 & 0.25 & 0.51 & 0.61/0.59 & 0.25/0.59 & 0.97 & 0.7 \\ 
   & p=1000 & 0.63/0.84/1 & 0.27/0.27/0.27/0.99 & 0.9/0.54/0.72 & 0.27 & 0.54 & 0.62/0.6 & 0.27/0.6 & 0.99 & 0.69 \\ 
   & p=1500 & 0.54/0.66/0.99 & 0.28/0.28/0.28/1 & 0.88/0.56/0.7 & 0.28 & 0.56 & 0.62/0.59 & 0.28/0.59 & 0.97 & 0.69 \\ 
  \midrule\multirow{4}[2]{*}{lsnr} & p=250 & 0.88/0.88/0.93 & 0.32/0.32/0.32/0.93 & 0.86/0.81/0.84 & 0.32 & 0.81 & 1/0.97 & 0.39/0.97 & 0.98 & 0.96 \\ 
   & p=500 & 0.82/0.9/0.93 & 0.33/0.33/0.33/0.93 & 0.89/0.85/0.86 & 0.33 & 0.85 & 1/0.96 & 0.33/0.96 & 0.96 & 0.95 \\ 
   & p=1000 & 0.73/0.87/0.93 & 0.35/0.35/0.35/0.93 & 0.91/0.89/0.89 & 0.35 & 0.89 & 1/0.95 & 0.35/0.95 & 0.95 & 0.93 \\ 
   & p=1500 & 0.67/0.78/0.93 & 0.35/0.35/0.35/0.92 & 0.92/0.9/0.91 & 0.35 & 0.9 & 1/0.94 & 0.35/0.94 & 0.95 & 0.91 \\ 
   \midrule 
 \multicolumn{1}{|c}{} &       & \multicolumn{9}{c|}{Sparsistency} \\
\midrule\multirow{4}[2]{*}{hsnr} & p=250 & 4.1/4.1/4.3 & 5.8/5.8/5.8/4.2 & 4.1/4/4 & 5.8 & 4 & 5/5.2 & 5.4/5.2 & 4.5 & 4.2 \\ 
   & p=500 & 4.2/4.1/4.2 & 5.3/5.3/5.3/4.2 & 4/4/4 & 5.3 & 4 & 4.8/4.9 & 5.1/4.9 & 4.4 & 4.1 \\ 
   & p=1000 & 4.2/4.1/4.1 & 4.9/4.9/4.9/4.1 & 4/4/4 & 4.9 & 4 & 4.6/4.8 & 4.8/4.8 & 4.3 & 4 \\ 
   & p=1500 & 4.2/4.1/4.1 & 4.7/4.7/4.7/4.1 & 4/4/4 & 4.7 & 4 & 4.5/4.6 & 4.6/4.6 & 4.3 & 4 \\ 
  \midrule\multirow{4}[2]{*}{msnr} & p=250 & 3.8/3.7/3.9 & 5.6/5.6/5.6/3.9 & 3.6/2.3/3.4 & 5.6 & 2.3 & 4.3/4.3 & 4.8/4.3 & 4 & 3.8 \\ 
   & p=500 & 3.9/3.7/3.8 & 4.9/4.9/4.9/3.8 & 3.4/2.2/3.1 & 4.9 & 2.2 & 4.1/4.2 & 4.6/4.2 & 3.9 & 3.6 \\ 
   & p=1000 & 3.9/3.7/3.7 & 4.5/4.5/4.5/3.7 & 3.3/2/2.8 & 4.5 & 2 & 4/4.1 & 4.3/4.1 & 3.9 & 3.4 \\ 
   & p=1500 & 3.9/3.8/3.6 & 4.3/4.3/4.3/3.6 & 3.2/2/2.7 & 4.3 & 2 & 3.8/4 & 4.1/4 & 3.8 & 3.3 \\ 
  \midrule\multirow{4}[2]{*}{lsnr} & p=250 & 0.8/0.5/1.2 & 5.3/5.3/5.3/1.2 & 0.4/0/0.2 & 5.3 & 0 & 2.2/2.2 & 3.7/2.2 & 2 & 1.8 \\ 
   & p=500 & 0.9/0.5/0.9 & 3.8/3.8/3.8/0.9 & 0.3/0/0.1 & 3.8 & 0 & 1.9/1.8 & 3.3/1.8 & 1.7 & 1.6 \\ 
   & p=1000 & 0.9/0.6/0.6 & 2.7/2.7/2.7/0.6 & 0.2/0/0.1 & 2.7 & 0 & 1.6/1.5 & 2.5/1.5 & 1.4 & 1.3 \\ 
   & p=1500 & 1/0.7/0.5 & 2.3/2.3/2.3/0.5 & 0.2/0/0 & 2.3 & 0 & 1.4/1.4 & 2.1/1.4 & 1.3 & 1.2 \\ 
   \midrule 
 \multicolumn{1}{|c}{} &       & \multicolumn{9}{c|}{Number of extra variables} \\
\midrule\multirow{4}[2]{*}{hsnr} & p=250 & 0.2/0/0.4 & 193.2/193.2/193.2/0.3 & 0/0/0 & 193.2 & 0 & 16.1/22.7 & 67.5/22.7 & 3.2 & 1.1 \\ 
   & p=500 & 2/0.1/0.3 & 193.7/193.7/193.7/0.3 & 0/0/0 & 193.7 & 0 & 17.9/29.1 & 101.9/29.1 & 4.2 & 1.6 \\ 
   & p=1000 & 5.1/0.7/0.3 & 194.1/194.1/194.1/0.3 & 0/0/0 & 194.1 & 0 & 19.2/36.7 & 96.1/36.7 & 5.1 & 0.9 \\ 
   & p=1500 & 7.3/2.4/0.3 & 194.3/194.3/194.3/0.3 & 0/0/0 & 194.2 & 0 & 20.2/40.2 & 92.2/40.2 & 5.7 & 1 \\ 
  \midrule\multirow{4}[2]{*}{msnr} & p=250 & 0.5/0.1/0.4 & 193.4/193.4/193.4/0.4 & 0/0/0 & 193.4 & 0 & 15/20.1 & 73/20.1 & 2.7 & 3.1 \\ 
   & p=500 & 2.4/0.3/0.4 & 194.1/194.1/194.1/0.4 & 0/0/0 & 194.1 & 0 & 16.8/26.3 & 117/26.3 & 4.2 & 4.1 \\ 
   & p=1000 & 5.9/1.5/0.4 & 194.5/194.5/194.5/0.4 & 0/0/0 & 194.5 & 0 & 18.1/32.9 & 111.4/32.9 & 5 & 5.3 \\ 
   & p=1500 & 8.2/4.3/0.4 & 194.7/194.7/194.7/0.4 & 0/0/0 & 194.7 & 0 & 18.2/35.6 & 106.8/35.6 & 6.1 & 5.6 \\ 
  \midrule\multirow{4}[2]{*}{lsnr} & p=250 & 0.4/0.1/0.5 & 193.7/193.7/193.7/0.5 & 0/0/0 & 193.7 & 0 & 9.1/11 & 67/11 & 6.8 & 5.6 \\ 
   & p=500 & 1.9/0.1/0.4 & 195.2/195.2/195.2/0.4 & 0/0/0 & 195.2 & 0 & 10.2/12.8 & 128.2/12.8 & 8.4 & 6.8 \\ 
   & p=1000 & 4.6/1/0.3 & 196.2/196.2/196.2/0.3 & 0/0/0 & 196.2 & 0 & 10.3/15.7 & 126.3/15.7 & 10.6 & 9.1 \\ 
   & p=1500 & 6.6/2.9/0.3 & 196.7/196.7/196.7/0.3 & 0/0/0 & 196.7 & 0 & 10/16.5 & 121.8/16.5 & 11.5 & 10.8 \\ 
   \bottomrule 
\end{tabular}
}
\end{table}
