# Supplementary material for: On the Use of Information Criteria for Subset Selection in Least Squares Regression
Source: arXiv:1911.10191 source file (2021-03-06)
Supplement: Supplementary file 44 [file Sparse-Ex4_rho_05.tex]

% latex table generated in R 4.0.3 by xtable 1.8-4 package
% Sun Feb 21 09:12:43 2021
\begin{table}[ht]
\centering
\caption{The performance of BOSS for high dimensional data, Sparse-Ex4, $\rho$=0.5, n=200} 
\scalebox{0.55}{
\begin{tabular}{|c|c|ccccccccc|}
  \toprule 
 \multicolumn{1}{|c}{} &       & BOSS  & FS    & FSstop & FStrim & FSstoptrim & lasso & Gamma lasso & SparseNet & rlasso \\
 \multicolumn{1}{|c}{} &       & C$_p$/AICc/CV & EBIC/HDBIC/HDHQ/CV & EBIC/HDBIC/HDHQ & HDBIC & HDBIC & AICc/CV & AICc/CV & CV    & CV  \\
 \cmidrule{3-11}\multicolumn{1}{|c}{} &       & \multicolumn{9}{c|}{\% worse than the best possible BOSS}  \\
 \midrule\multirow{4}[2]{*}{hsnr} & p=250 & 9/5/12 & 292/292/292/13 & 5/5/5 & 292 & 5 & 95/93 & 215/93 & 13 & 19 \\ 
   & p=500 & 26/4/11 & 283/283/283/12 & 3/2/2 & 283 & 2 & 112/107 & 268/107 & 12 & 21 \\ 
   & p=1000 & 59/13/11 & 278/278/278/12 & 2/1/1 & 278 & 1 & 132/125 & 268/125 & 12 & 30 \\ 
   & p=1500 & 84/37/11 & 277/277/277/12 & 1/0/1 & 277 & 0 & 145/135 & 268/135 & 12 & 39 \\ 
  \midrule\multirow{4}[2]{*}{msnr} & p=250 & 26/22/31 & 374/374/374/44 & 29/117/44 & 374 & 118 & 123/121 & 306/121 & 15 & 115 \\ 
   & p=500 & 48/22/28 & 314/314/314/47 & 30/100/49 & 314 & 100 & 117/115 & 308/115 & 20 & 102 \\ 
   & p=1000 & 72/36/27 & 267/267/267/45 & 30/83/47 & 267 & 84 & 112/110 & 264/110 & 24 & 87 \\ 
   & p=1500 & 78/56/26 & 235/235/235/39 & 26/72/42 & 235 & 73 & 102/101 & 232/101 & 23 & 72 \\ 
  \midrule\multirow{4}[2]{*}{lsnr} & p=250 & 25/24/21 & 251/251/251/33 & 32/37/35 & 251 & 37 & 30/32 & 180/32 & 25 & 35 \\ 
   & p=500 & 26/17/17 & 216/216/216/24 & 21/24/23 & 216 & 24 & 20/23 & 214/23 & 21 & 26 \\ 
   & p=1000 & 30/14/12 & 187/187/187/15 & 11/12/12 & 187 & 12 & 11/14 & 186/14 & 14 & 17 \\ 
   & p=1500 & 36/22/11 & 177/177/177/12 & 8/9/8 & 177 & 9 & 7/11 & 177/11 & 12 & 15 \\ 
   \midrule 
 \multicolumn{1}{|c}{} &       & \multicolumn{9}{c|}{Relative efficiency} \\
\midrule\multirow{4}[2]{*}{hsnr} & p=250 & 0.96/0.99/0.93 & 0.27/0.27/0.27/0.92 & 0.99/1/1 & 0.27 & 1 & 0.53/0.54 & 0.33/0.54 & 0.93 & 0.88 \\ 
   & p=500 & 0.81/0.98/0.92 & 0.27/0.27/0.27/0.91 & 0.99/1/1 & 0.27 & 1 & 0.48/0.49 & 0.28/0.49 & 0.91 & 0.84 \\ 
   & p=1000 & 0.63/0.89/0.91 & 0.27/0.27/0.27/0.9 & 0.99/1/1 & 0.27 & 1 & 0.43/0.45 & 0.27/0.45 & 0.9 & 0.77 \\ 
   & p=1500 & 0.55/0.73/0.91 & 0.27/0.27/0.27/0.9 & 0.99/1/1 & 0.27 & 1 & 0.41/0.43 & 0.27/0.43 & 0.9 & 0.72 \\ 
  \midrule\multirow{4}[2]{*}{msnr} & p=250 & 0.91/0.94/0.88 & 0.24/0.24/0.24/0.8 & 0.89/0.53/0.8 & 0.24 & 0.53 & 0.52/0.52 & 0.28/0.52 & 1 & 0.54 \\ 
   & p=500 & 0.81/0.98/0.94 & 0.29/0.29/0.29/0.82 & 0.93/0.6/0.81 & 0.29 & 0.6 & 0.55/0.56 & 0.29/0.56 & 1 & 0.6 \\ 
   & p=1000 & 0.72/0.91/0.97 & 0.34/0.34/0.34/0.85 & 0.95/0.67/0.84 & 0.34 & 0.67 & 0.58/0.59 & 0.34/0.59 & 1 & 0.66 \\ 
   & p=1500 & 0.69/0.79/0.98 & 0.37/0.37/0.37/0.88 & 0.98/0.71/0.87 & 0.37 & 0.71 & 0.61/0.61 & 0.37/0.61 & 1 & 0.71 \\ 
  \midrule\multirow{4}[2]{*}{lsnr} & p=250 & 0.97/0.98/1 & 0.35/0.35/0.35/0.91 & 0.92/0.88/0.9 & 0.35 & 0.88 & 0.94/0.92 & 0.43/0.92 & 0.97 & 0.9 \\ 
   & p=500 & 0.93/1/1 & 0.37/0.37/0.37/0.94 & 0.97/0.95/0.95 & 0.37 & 0.95 & 0.97/0.95 & 0.37/0.95 & 0.97 & 0.92 \\ 
   & p=1000 & 0.85/0.97/0.98 & 0.39/0.39/0.39/0.96 & 1/0.99/0.99 & 0.39 & 0.99 & 1/0.97 & 0.39/0.97 & 0.97 & 0.94 \\ 
   & p=1500 & 0.79/0.88/0.97 & 0.39/0.39/0.39/0.96 & 1/0.99/0.99 & 0.39 & 0.99 & 1/0.96 & 0.39/0.96 & 0.96 & 0.93 \\ 
   \midrule 
 \multicolumn{1}{|c}{} &       & \multicolumn{9}{c|}{Sparsistency} \\
\midrule\multirow{4}[2]{*}{hsnr} & p=250 & 4.1/4.1/4.2 & 5.8/5.8/5.8/4.1 & 4/4/4 & 5.8 & 4 & 4.8/5 & 5.3/5 & 4.3 & 4 \\ 
   & p=500 & 4.1/4.1/4.1 & 5.2/5.2/5.2/4.1 & 4/4/4 & 5.2 & 4 & 4.5/4.7 & 5/4.7 & 4.2 & 4 \\ 
   & p=1000 & 4.1/4.1/4 & 4.7/4.7/4.7/4 & 4/4/4 & 4.7 & 4 & 4.3/4.5 & 4.6/4.5 & 4.1 & 4 \\ 
   & p=1500 & 4.1/4.1/4 & 4.5/4.5/4.5/4 & 4/4/4 & 4.5 & 4 & 4.2/4.4 & 4.4/4.4 & 4.1 & 4 \\ 
  \midrule\multirow{4}[2]{*}{msnr} & p=250 & 3.9/3.9/3.9 & 5.6/5.6/5.6/3.7 & 3.5/2.3/3.3 & 5.6 & 2.3 & 4.1/4.3 & 4.8/4.3 & 4 & 3.3 \\ 
   & p=500 & 3.8/3.7/3.7 & 4.8/4.8/4.8/3.3 & 3.2/2.2/2.9 & 4.8 & 2.1 & 3.8/4 & 4.4/4 & 3.8 & 2.9 \\ 
   & p=1000 & 3.7/3.6/3.5 & 4.2/4.2/4.2/3.1 & 3/2.1/2.7 & 4.2 & 2 & 3.4/3.7 & 4.1/3.7 & 3.6 & 2.6 \\ 
   & p=1500 & 3.5/3.5/3.3 & 4/4/4/2.9 & 2.9/2/2.5 & 4 & 2 & 3.2/3.4 & 3.8/3.4 & 3.4 & 2.5 \\ 
  \midrule\multirow{4}[2]{*}{lsnr} & p=250 & 0.8/0.6/1.2 & 5.3/5.3/5.3/0.7 & 0.3/0/0.1 & 5.3 & 0 & 1.4/1.2 & 3.4/1.2 & 1.4 & 1.1 \\ 
   & p=500 & 0.7/0.5/0.7 & 3.6/3.6/3.6/0.4 & 0.1/0/0.1 & 3.6 & 0 & 0.9/0.9 & 2.8/0.9 & 1 & 0.7 \\ 
   & p=1000 & 0.5/0.3/0.3 & 2.3/2.3/2.3/0.2 & 0.1/0/0 & 2.3 & 0 & 0.6/0.6 & 1.7/0.6 & 0.6 & 0.5 \\ 
   & p=1500 & 0.4/0.4/0.2 & 1.7/1.7/1.7/0.2 & 0.1/0/0 & 1.7 & 0 & 0.5/0.5 & 1.3/0.5 & 0.5 & 0.4 \\ 
   \midrule 
 \multicolumn{1}{|c}{} &       & \multicolumn{9}{c|}{Number of extra variables} \\
\midrule\multirow{4}[2]{*}{hsnr} & p=250 & 0.4/0/0.4 & 193.2/193.2/193.2/0.3 & 0/0/0 & 193.2 & 0 & 23.7/36.4 & 63.8/36.4 & 3.4 & 1.1 \\ 
   & p=500 & 2.7/0.1/0.3 & 193.8/193.8/193.8/0.3 & 0/0/0 & 193.8 & 0 & 26.1/46.1 & 104.6/46.1 & 4.1 & 1.4 \\ 
   & p=1000 & 6.2/0.8/0.3 & 194.3/194.3/194.3/0.3 & 0/0/0 & 194.2 & 0 & 28.5/59.2 & 103.1/59.2 & 5.1 & 2.3 \\ 
   & p=1500 & 8.3/3.1/0.3 & 194.5/194.5/194.5/0.3 & 0/0/0 & 194.4 & 0 & 29.8/66 & 100.1/66 & 5.3 & 3.7 \\ 
  \midrule\multirow{4}[2]{*}{msnr} & p=250 & 0.9/0.4/0.8 & 193.4/193.4/193.4/0.9 & 0.1/0/0 & 193.4 & 0 & 21.7/32.8 & 74.5/32.8 & 4.6 & 6.5 \\ 
   & p=500 & 3.4/0.7/0.9 & 194.2/194.2/194.2/0.9 & 0.1/0/0 & 194.2 & 0 & 22.8/39.7 & 116.2/39.7 & 7.4 & 5.5 \\ 
   & p=1000 & 6.6/1.9/1 & 194.8/194.7/194.8/0.8 & 0.1/0/0 & 194.7 & 0 & 22.9/46.5 & 114.4/46.5 & 9.3 & 5.1 \\ 
   & p=1500 & 8.2/4.6/0.9 & 195/195/195/0.7 & 0.1/0/0 & 194.9 & 0 & 22.5/47.9 & 111.5/47.9 & 10.8 & 4.2 \\ 
  \midrule\multirow{4}[2]{*}{lsnr} & p=250 & 0.6/0.2/1.1 & 193.7/193.7/193.7/0.6 & 0/0/0 & 193.7 & 0 & 8.6/10.2 & 68.8/10.2 & 6.8 & 7 \\ 
   & p=500 & 1.7/0.3/0.7 & 195.4/195.4/195.4/0.4 & 0/0/0 & 195.4 & 0 & 7.9/9.8 & 126.8/9.8 & 8.1 & 6.8 \\ 
   & p=1000 & 3.3/0.8/0.4 & 196.7/196.7/196.7/0.3 & 0/0/0 & 196.7 & 0 & 7.6/11.5 & 126.4/11.5 & 8.5 & 7.6 \\ 
   & p=1500 & 4.7/2.3/0.3 & 197.3/197.3/197.3/0.3 & 0/0/0 & 197.3 & 0 & 7.5/12.2 & 122.8/12.2 & 9.4 & 9.2 \\ 
   \bottomrule 
\end{tabular}
}
\end{table}
