# Supplementary material for: On the Use of Information Criteria for Subset Selection in Least Squares Regression
Source: arXiv:1911.10191 source file (2021-03-06)
Supplement: Supplementary file 45 [file Sparse-Ex4_rho_09.tex]

% latex table generated in R 4.0.3 by xtable 1.8-4 package
% Sun Feb 21 09:14:17 2021
\begin{table}[ht]
\centering
\caption{The performance of BOSS for high dimensional data, Sparse-Ex4, $\rho$=0.9, n=200} 
\scalebox{0.55}{
\begin{tabular}{|c|c|ccccccccc|}
  \toprule 
 \multicolumn{1}{|c}{} &       & BOSS  & FS    & FSstop & FStrim & FSstoptrim & lasso & Gamma lasso & SparseNet & rlasso \\
 \multicolumn{1}{|c}{} &       & C$_p$/AICc/CV & EBIC/HDBIC/HDHQ/CV & EBIC/HDBIC/HDHQ & HDBIC & HDBIC & AICc/CV & AICc/CV & CV    & CV  \\
 \cmidrule{3-11}\multicolumn{1}{|c}{} &       & \multicolumn{9}{c|}{\% worse than the best possible BOSS}  \\
 \midrule\multirow{4}[2]{*}{hsnr} & p=250 & 13/5/35 & 249/249/249/75 & 6/10/6 & 249 & 3 & 182/149 & 140/149 & 4 & 151 \\ 
   & p=500 & 26/8/48 & 196/196/196/90 & 8/32/12 & 196 & 22 & 254/169 & 170/169 & 10 & 196 \\ 
   & p=1000 & 15/60/119 & 51/51/51/147 & 105/146/115 & 51 & 144 & 105/58 & 47/58 & 4 & 50 \\ 
   & p=1500 & 26/48/123 & 23/23/23/146 & 114/141/124 & 23 & 140 & 97/39 & 21/39 & 3 & 36 \\ 
  \midrule\multirow{4}[2]{*}{msnr} & p=250 & 19/21/23 & 144/144/144/79 & 51/102/60 & 144 & 101 & 86/72 & 100/72 & 20 & 67 \\ 
   & p=500 & 16/14/17 & 66/66/66/53 & 34/60/40 & 66 & 60 & 60/50 & 62/50 & -11 & 48 \\ 
   & p=1000 & 12/12/15 & 22/22/22/25 & 19/27/22 & 22 & 27 & 24/25 & 21/25 & 15 & 25 \\ 
   & p=1500 & 10/10/13 & 13/13/13/18 & 15/19/16 & 13 & 19 & 15/15 & 12/15 & 14 & 15 \\ 
  \midrule\multirow{4}[2]{*}{lsnr} & p=250 & 11/10/14 & 197/197/197/20 & 16/16/16 & 197 & 16 & 17/17 & 160/17 & 20 & 20 \\ 
   & p=500 & 8/5/9 & 173/173/173/11 & 7/7/7 & 173 & 7 & 8/9 & 170/9 & 10 & 11 \\ 
   & p=1000 & 15/4/6 & 162/162/162/7 & 2/2/2 & 162 & 2 & 3/5 & 160/5 & 6 & 8 \\ 
   & p=1500 & 23/10/5 & 158/158/158/6 & 1/1/1 & 158 & 1 & 2/3 & 157/3 & 5 & 7 \\ 
   \midrule 
 \multicolumn{1}{|c}{} &       & \multicolumn{9}{c|}{Relative efficiency} \\
\midrule\multirow{4}[2]{*}{hsnr} & p=250 & 0.92/0.99/0.77 & 0.3/0.3/0.3/0.59 & 0.98/0.94/0.98 & 0.3 & 1 & 0.37/0.42 & 0.43/0.42 & 1 & 0.41 \\ 
   & p=500 & 0.85/1/0.73 & 0.36/0.36/0.36/0.57 & 1/0.82/0.96 & 0.36 & 0.88 & 0.3/0.4 & 0.4/0.4 & 0.98 & 0.36 \\ 
   & p=1000 & 0.91/0.65/0.48 & 0.69/0.69/0.69/0.42 & 0.51/0.42/0.49 & 0.69 & 0.43 & 0.51/0.66 & 0.71/0.66 & 1 & 0.7 \\ 
   & p=1500 & 0.81/0.69/0.46 & 0.83/0.83/0.83/0.42 & 0.48/0.43/0.46 & 0.83 & 0.43 & 0.52/0.74 & 0.85/0.74 & 1 & 0.76 \\ 
  \midrule\multirow{4}[2]{*}{msnr} & p=250 & 1/0.99/0.97 & 0.49/0.49/0.49/0.67 & 0.79/0.59/0.75 & 0.49 & 0.6 & 0.64/0.69 & 0.6/0.69 & 1 & 0.72 \\ 
   & p=500 & 0.76/0.78/0.76 & 0.53/0.53/0.53/0.58 & 0.66/0.55/0.63 & 0.53 & 0.55 & 0.55/0.59 & 0.55/0.59 & 1 & 0.6 \\ 
   & p=1000 & 1/1/0.97 & 0.92/0.92/0.92/0.89 & 0.94/0.88/0.92 & 0.92 & 0.88 & 0.9/0.9 & 0.93/0.9 & 0.97 & 0.9 \\ 
   & p=1500 & 1/0.99/0.97 & 0.97/0.97/0.97/0.93 & 0.95/0.92/0.94 & 0.97 & 0.92 & 0.95/0.95 & 0.98/0.95 & 0.96 & 0.95 \\ 
  \midrule\multirow{4}[2]{*}{lsnr} & p=250 & 0.99/1/0.97 & 0.37/0.37/0.37/0.91 & 0.95/0.95/0.95 & 0.37 & 0.95 & 0.94/0.94 & 0.42/0.94 & 0.92 & 0.92 \\ 
   & p=500 & 0.98/1/0.96 & 0.39/0.39/0.39/0.95 & 0.98/0.98/0.99 & 0.39 & 0.98 & 0.97/0.97 & 0.39/0.97 & 0.95 & 0.95 \\ 
   & p=1000 & 0.89/0.98/0.97 & 0.39/0.39/0.39/0.96 & 1/1/1 & 0.39 & 1 & 0.99/0.97 & 0.39/0.97 & 0.96 & 0.95 \\ 
   & p=1500 & 0.82/0.92/0.96 & 0.39/0.39/0.39/0.95 & 1/1/1 & 0.39 & 1 & 0.99/0.98 & 0.39/0.98 & 0.96 & 0.95 \\ 
   \midrule 
 \multicolumn{1}{|c}{} &       & \multicolumn{9}{c|}{Sparsistency} \\
\midrule\multirow{4}[2]{*}{hsnr} & p=250 & 4.1/4.1/4.2 & 5.6/5.6/5.6/4.1 & 4/3.9/4 & 5.6 & 3.9 & 4.3/4.6 & 4.5/4.6 & 4.2 & 4.1 \\ 
   & p=500 & 4/4/4 & 4.8/4.8/4.8/4 & 3.9/3.7/3.8 & 4.8 & 3.7 & 3.2/4 & 4.3/4 & 4.2 & 3.1 \\ 
   & p=1000 & 3.1/3/2.8 & 3.6/3.6/3.6/1.9 & 2/1.4/1.8 & 3.6 & 1.4 & 3/3 & 2.5/3 & 3.9 & 3 \\ 
   & p=1500 & 2.2/2.1/1.7 & 2.6/2.6/2.6/0.8 & 1.2/0.7/1 & 2.6 & 0.7 & 2.5/2.8 & 1.9/2.8 & 3.3 & 2.8 \\ 
  \midrule\multirow{4}[2]{*}{msnr} & p=250 & 3.5/3.3/3.5 & 5.4/5.4/5.4/2.3 & 2.2/1/1.9 & 5.4 & 1 & 2.9/3.2 & 3.9/3.2 & 2.9 & 2.9 \\ 
   & p=500 & 2.6/2.4/2.5 & 4/4/4/1 & 1.3/0.4/1 & 4 & 0.4 & 1.3/1.6 & 2.8/1.6 & 2.6 & 1.7 \\ 
   & p=1000 & 1.1/1/1 & 2.4/2.4/2.4/0.4 & 0.5/0.1/0.4 & 2.4 & 0.1 & 0.6/0.6 & 1.5/0.6 & 1 & 0.5 \\ 
   & p=1500 & 0.8/0.7/0.5 & 1.6/1.6/1.6/0.2 & 0.3/0.1/0.2 & 1.6 & 0.1 & 0.5/0.5 & 1/0.5 & 0.5 & 0.4 \\ 
  \midrule\multirow{4}[2]{*}{lsnr} & p=250 & 0.3/0.3/0.4 & 4.7/4.7/4.7/0.1 & 0.1/0/0 & 4.7 & 0 & 0.2/0.2 & 1.9/0.2 & 0.2 & 0.2 \\ 
   & p=500 & 0.2/0.1/0.1 & 2.5/2.5/2.5/0 & 0/0/0 & 2.5 & 0 & 0.2/0.1 & 1.3/0.1 & 0.1 & 0.1 \\ 
   & p=1000 & 0.1/0.1/0 & 1.3/1.3/1.3/0 & 0/0/0 & 1.3 & 0 & 0.1/0.1 & 0.7/0.1 & 0.1 & 0.1 \\ 
   & p=1500 & 0.1/0/0 & 0.8/0.8/0.8/0 & 0/0/0 & 0.8 & 0 & 0.1/0.1 & 0.5/0.1 & 0.1 & 0.1 \\ 
   \midrule 
 \multicolumn{1}{|c}{} &       & \multicolumn{9}{c|}{Number of extra variables} \\
\midrule\multirow{4}[2]{*}{hsnr} & p=250 & 2.9/1.2/3.6 & 193.4/193.4/193.4/7.3 & 0.8/0.7/0.8 & 193.4 & 0 & 55.7/90.9 & 49.1/90.9 & 9.3 & 39.6 \\ 
   & p=500 & 7.8/2.5/4.9 & 194.2/194.2/194.2/11.5 & 1.8/1.2/1.6 & 194.2 & 0 & 44.1/104.6 & 96/104.6 & 33.9 & 18.9 \\ 
   & p=1000 & 24.7/10.1/6.6 & 195.4/195.4/195.4/5.9 & 2.5/0.9/2 & 195.4 & 0 & 50.1/93.8 & 108.1/93.8 & 87.7 & 40.7 \\ 
   & p=1500 & 28.5/18.4/4.5 & 196.4/196.4/196.4/2.1 & 1.7/0.5/1.1 & 196.3 & 0 & 43/101.4 & 109.6/101.4 & 84.5 & 61.6 \\ 
  \midrule\multirow{4}[2]{*}{msnr} & p=250 & 9.9/7.2/9.2 & 193.6/193.6/193.6/6.6 & 1.6/0.2/1.2 & 193.6 & 0 & 33.4/55.5 & 68.7/55.5 & 24.4 & 27.8 \\ 
   & p=500 & 11.9/6.4/7.4 & 195/195/195/2 & 1.1/0.1/0.6 & 195 & 0 & 15.2/36.7 & 112.9/36.7 & 41 & 24.6 \\ 
   & p=1000 & 4.7/2.9/2.7 & 196.6/196.6/196.6/0.8 & 0.4/0/0.2 & 196.5 & 0 & 8.2/11 & 115.1/11 & 25.6 & 7.5 \\ 
   & p=1500 & 5.4/3.3/1.4 & 197.4/197.4/197.4/0.6 & 0.2/0/0.1 & 197.3 & 0 & 8.6/11.9 & 113.4/11.9 & 10.1 & 7.8 \\ 
  \midrule\multirow{4}[2]{*}{lsnr} & p=250 & 0.7/0.6/1.5 & 194.3/194.3/194.3/0.3 & 0/0/0 & 194.3 & 0 & 4.2/3.8 & 79.1/3.8 & 4.2 & 2.8 \\ 
   & p=500 & 0.6/0.2/0.5 & 196.5/196.5/196.5/0.3 & 0/0/0 & 196.5 & 0 & 4.7/5.2 & 123.5/5.2 & 4.7 & 3.9 \\ 
   & p=1000 & 2.1/0.3/0.3 & 197.7/197.7/197.7/0.3 & 0/0/0 & 197.7 & 0 & 5.9/8.1 & 121.3/8.1 & 6.3 & 5.5 \\ 
   & p=1500 & 3.6/1.3/0.3 & 198.2/198.2/198.2/0.3 & 0/0/0 & 198.1 & 0 & 6.5/8.5 & 119.2/8.5 & 7 & 6.6 \\ 
   \bottomrule 
\end{tabular}
}
\end{table}
