# Supplementary material for: On the Use of Information Criteria for Subset Selection in Least Squares Regression
Source: arXiv:1911.10191 source file (2021-03-06)
Supplement: Supplementary file 46 [file Orth-Dense_n200.tex]

% latex table generated in R 3.6.1 by xtable 1.8-4 package
% Sun Nov 10 01:27:06 2019
\begin{table}[ht]
\centering
\caption{The performance of BS using different selection rules, Orth-Dense, n=200} 
\scalebox{0.75}{
\begin{tabular}{|c|c|cc|cc|cc|cc|c|}
  \toprule 
 \multicolumn{1}{|c}{} &       & \multicolumn{2}{c|}{C$_p$} & \multicolumn{2}{c|}{AICc} & \multicolumn{2}{c|}{BIC} & \multicolumn{2}{c|}{GCV} & \multirow{2}[2]{*}{CV} \\
 \multicolumn{1}{|c}{} &       & edf   & ndf/hdf/bdf & edf   & ndf/hdf/bdf & edf   & ndf/hdf/bdf & edf   & ndf/hdf/bdf &       \\
 \cmidrule{3-11}\multicolumn{1}{|c}{} &       & \multicolumn{9}{c|}{\% worse than the best possible BS} \\
 \midrule\multirow{4}[2]{*}{hsnr} & p=14 & 0 & 0/0/0 & 0 & 0/0/0 & 0 & 1/0/0 & 0 & 0/0/0 & 0 \\ 
   & p=30 & 1 & 11/1/2 & 1 & 13/1/2 & 1 & 28/3/5 & 1 & 11/1/2 & 7 \\ 
   & p=60 & 8 & 7/9/9 & 9 & 7/11/11 & 20 & 8/32/33 & 8 & 8/10/10 & - \\ 
   & p=180 & 7 & 45/21/20 & 9 & 52/18/19 & 18 & 26/39/42 & 7 & 64/13/13 & - \\ 
  \midrule\multirow{4}[2]{*}{msnr} & p=14 & 0 & 9/0/1 & 0 & 10/0/1 & 0 & 36/1/2 & 0 & 9/0/1 & 6 \\ 
   & p=30 & 3 & 10/3/4 & 3 & 11/4/5 & 21 & 27/19/25 & 3 & 10/4/4 & 11 \\ 
   & p=60 & 10 & 11/14/13 & 10 & 11/13/13 & 26 & 10/48/48 & 10 & 12/14/13 & - \\ 
   & p=180 & 8 & 52/23/23 & 10 & 62/18/19 & 21 & 25/61/56 & 8 & 74/14/14 & - \\ 
  \midrule\multirow{4}[2]{*}{lsnr} & p=14 & 5 & 22/6/8 & 7 & 23/8/10 & 73 & 50/73/72 & 6 & 22/7/8 & 19 \\ 
   & p=30 & 15 & 10/16/16 & 20 & 10/21/20 & 27 & 16/27/27 & 17 & 10/18/18 & 16 \\ 
   & p=60 & 13 & 25/17/16 & 13 & 25/13/13 & 13 & 11/13/13 & 13 & 26/14/14 & - \\ 
   & p=180 & 8 & 86/22/22 & 7 & 102/7/7 & 7 & 39/7/7 & 7 & 116/7/7 & - \\ 
   \midrule 
 \multicolumn{1}{|c}{} &       & \multicolumn{9}{c|}{Relative efficiency} \\
\midrule\multirow{4}[2]{*}{hsnr} & p=14 & 1 & 1/1/1 & 1 & 1/1/1 & 1 & 0.99/1/1 & 1 & 1/1/1 & 1 \\ 
   & p=30 & 1 & 0.91/1/1 & 1 & 0.9/1/0.99 & 1 & 0.79/0.98/0.96 & 1 & 0.91/1/1 & 0.95 \\ 
   & p=60 & 0.99 & 1/0.98/0.98 & 0.98 & 1/0.97/0.96 & 0.89 & 0.99/0.81/0.8 & 0.99 & 0.99/0.98/0.98 & - \\ 
   & p=180 & 1 & 0.74/0.89/0.89 & 0.99 & 0.71/0.91/0.9 & 0.91 & 0.85/0.77/0.76 & 1 & 0.65/0.95/0.95 & - \\ 
  \midrule\multirow{4}[2]{*}{msnr} & p=14 & 1 & 0.92/1/0.99 & 1 & 0.91/1/0.99 & 1 & 0.74/1/0.99 & 1 & 0.92/1/0.99 & 0.95 \\ 
   & p=30 & 1 & 0.93/0.99/0.99 & 0.99 & 0.92/0.98/0.98 & 0.85 & 0.81/0.87/0.82 & 1 & 0.93/0.99/0.99 & 0.93 \\ 
   & p=60 & 1 & 0.99/0.96/0.97 & 1 & 0.99/0.97/0.97 & 0.87 & 1/0.74/0.74 & 1 & 0.98/0.97/0.97 & - \\ 
   & p=180 & 1 & 0.71/0.88/0.88 & 0.98 & 0.67/0.91/0.91 & 0.89 & 0.87/0.67/0.69 & 1 & 0.62/0.95/0.95 & - \\ 
  \midrule\multirow{4}[2]{*}{lsnr} & p=14 & 0.98 & 0.85/0.97/0.96 & 0.97 & 0.84/0.96/0.94 & 0.6 & 0.69/0.6/0.6 & 0.98 & 0.85/0.97/0.95 & 0.86 \\ 
   & p=30 & 0.95 & 1/0.95/0.95 & 0.91 & 1/0.91/0.91 & 0.86 & 0.94/0.86/0.86 & 0.93 & 1/0.93/0.93 & 0.94 \\ 
   & p=60 & 0.98 & 0.89/0.95/0.96 & 0.99 & 0.89/0.99/0.99 & 0.98 & 1/0.98/0.98 & 0.98 & 0.88/0.97/0.98 & - \\ 
   & p=180 & 1 & 0.58/0.88/0.88 & 1 & 0.53/1/1 & 1 & 0.77/1/1 & 1 & 0.5/1/1 & - \\ 
   \midrule 
 \multicolumn{1}{|c}{} &       & \multicolumn{9}{c|}{Sparsistency (number of extra variables)} \\
\midrule\multirow{4}[2]{*}{hsnr} & p=14 & 14 & 14/14/14 & 14 & 14/14/14 & 14 & 14/14/14 & 14 & 14/14/14 & 14 \\ 
   & p=30 & 30 & 24.7/29.5/29 & 30 & 24.2/29.4/28.8 & 30 & 20.9/28.8/27.5 & 30 & 24.7/29.5/29 & 26.6 \\ 
   & p=60 & 29.8 & 30.5/38.4/35.8 & 22.2 & 29.4/25.6/24.5 & 17.8 & 22.5/16.8/16.5 & 28.6 & 31.3/36.8/34 & - \\ 
   & p=180 & 20.5 & 53.3/37.4/35.5 & 18.3 & 62.3/16.3/16.3 & 16.1 & 35/13.7/13.5 & 19.4 & 89.8/17.8/17.8 & - \\ 
  \midrule\multirow{4}[2]{*}{msnr} & p=14 & 14 & 13.2/14/13.9 & 14 & 13.2/14/13.9 & 14 & 11.8/13.9/13.8 & 14 & 13.2/14/13.9 & 13.4 \\ 
   & p=30 & 27.3 & 18.8/27.4/26.1 & 26.5 & 18.3/26.8/25.3 & 18 & 13.4/20.4/17.6 & 27.3 & 18.8/27.4/26.1 & 20.8 \\ 
   & p=60 & 19.4 & 24.1/29.6/27 & 13.9 & 23.4/15.6/15.2 & 9.3 & 14.5/7.5/7.4 & 18.3 & 25.2/26/24.1 & - \\ 
   & p=180 & 12.6 & 47.1/29.1/28.1 & 10.4 & 59/8.8/8.8 & 8.1 & 24.4/4.8/5 & 11.3 & 86.4/10/10 & - \\ 
  \midrule\multirow{4}[2]{*}{lsnr} & p=14 & 13.6 & 7.7/12.7/11.7 & 13.4 & 7.6/12.3/11.3 & 0.7 & 3.6/0.7/0.8 & 13.5 & 7.8/12.6/11.6 & 8.8 \\ 
   & p=30 & 12.8 & 10.5/14.6/13 & 7.6 & 10.3/8.5/7.6 & 0 & 4/0/0 & 11.3 & 10.8/12.3/11.2 & 7.5 \\ 
   & p=60 & 3.4 & 15.7/6.5/6 & 1 & 15.8/0.8/1 & 0 & 4.9/0/0 & 2 & 17.3/2.4/2.4 & - \\ 
   & p=180 & 0.8 & 39/14.5/13.7 & 0.3 & 55.2/0.2/0.3 & 0 & 11.8/0/0 & 0.4 & 81.7/0.3/0.4 & - \\ 
   \bottomrule 
\end{tabular}
}
\end{table}
