# Supplementary material for: On the Use of Information Criteria for Subset Selection in Least Squares Regression
Source: arXiv:1911.10191 source file (2021-03-06)
Supplement: Supplementary file 47 [file Orth-Dense_n2000.tex]

% latex table generated in R 3.6.1 by xtable 1.8-4 package
% Sun Nov 10 01:27:13 2019
\begin{table}[ht]
\centering
\caption{The performance of BS using different selection rules, Orth-Dense, n=2000} 
\scalebox{0.75}{
\begin{tabular}{|c|c|cc|cc|cc|cc|c|}
  \toprule 
 \multicolumn{1}{|c}{} &       & \multicolumn{2}{c|}{C$_p$} & \multicolumn{2}{c|}{AICc} & \multicolumn{2}{c|}{BIC} & \multicolumn{2}{c|}{GCV} & \multirow{2}[2]{*}{CV} \\
 \multicolumn{1}{|c}{} &       & edf   & ndf/hdf/bdf & edf   & ndf/hdf/bdf & edf   & ndf/hdf/bdf & edf   & ndf/hdf/bdf &       \\
 \cmidrule{3-11}\multicolumn{1}{|c}{} &       & \multicolumn{9}{c|}{\% worse than the best possible BS} \\
 \midrule\multirow{4}[2]{*}{hsnr} & p=14 & 0 & 0/0/0 & 0 & 0/0/0 & 0 & 0/0/0 & 0 & 0/0/0 & 0 \\ 
   & p=30 & 0 & 1/0/0 & 0 & 1/0/0 & 0 & 18/0/1 & 0 & 1/0/0 & 1 \\ 
   & p=60 & 5 & 5/5/5 & 5 & 5/5/5 & 25 & 17/34/37 & 5 & 5/5/5 & - \\ 
   & p=180 & 6 & 34/8/8 & 6 & 34/8/8 & 19 & 7/36/37 & 6 & 35/8/8 & - \\ 
  \midrule\multirow{4}[2]{*}{msnr} & p=14 & 0 & 0/0/0 & 0 & 0/0/0 & 0 & 0/0/0 & 0 & 0/0/0 & 0 \\ 
   & p=30 & 1 & 9/1/1 & 1 & 9/1/1 & 1 & 40/2/5 & 1 & 9/1/1 & 5 \\ 
   & p=60 & 7 & 6/8/8 & 7 & 6/8/8 & 28 & 15/37/40 & 7 & 6/8/8 & - \\ 
   & p=180 & 6 & 39/9/9 & 6 & 39/8/9 & 21 & 7/38/40 & 6 & 40/8/9 & - \\ 
  \midrule\multirow{4}[2]{*}{lsnr} & p=14 & 0 & 5/0/0 & 0 & 5/0/0 & 0 & 49/0/1 & 0 & 5/0/0 & 4 \\ 
   & p=30 & 2 & 11/3/3 & 2 & 11/3/3 & 44 & 41/36/45 & 2 & 11/3/3 & 10 \\ 
   & p=60 & 10 & 10/13/12 & 10 & 10/13/12 & 32 & 16/45/48 & 10 & 10/13/12 & - \\ 
   & p=180 & 8 & 48/10/10 & 8 & 48/10/10 & 24 & 8/45/47 & 8 & 49/10/10 & - \\ 
   \midrule 
 \multicolumn{1}{|c}{} &       & \multicolumn{9}{c|}{Relative efficiency} \\
\midrule\multirow{4}[2]{*}{hsnr} & p=14 & 1 & 1/1/1 & 1 & 1/1/1 & 1 & 1/1/1 & 1 & 1/1/1 & 1 \\ 
   & p=30 & 1 & 0.99/1/1 & 1 & 0.99/1/1 & 1 & 0.85/1/0.99 & 1 & 0.99/1/1 & 0.99 \\ 
   & p=60 & 0.99 & 1/0.99/0.99 & 0.99 & 1/0.99/0.99 & 0.83 & 0.89/0.78/0.76 & 0.99 & 1/0.99/0.99 & - \\ 
   & p=180 & 1 & 0.79/0.98/0.98 & 1 & 0.79/0.98/0.98 & 0.89 & 1/0.78/0.78 & 1 & 0.79/0.98/0.98 & - \\ 
  \midrule\multirow{4}[2]{*}{msnr} & p=14 & 1 & 1/1/1 & 1 & 1/1/1 & 1 & 1/1/1 & 1 & 1/1/1 & 1 \\ 
   & p=30 & 1 & 0.92/1/1 & 1 & 0.92/1/1 & 1 & 0.72/0.99/0.96 & 1 & 0.92/1/1 & 0.96 \\ 
   & p=60 & 0.99 & 1/0.98/0.98 & 0.99 & 1/0.98/0.98 & 0.83 & 0.92/0.77/0.76 & 0.99 & 1/0.98/0.98 & - \\ 
   & p=180 & 1 & 0.76/0.98/0.98 & 1 & 0.76/0.98/0.98 & 0.88 & 1/0.77/0.76 & 1 & 0.76/0.98/0.98 & - \\ 
  \midrule\multirow{4}[2]{*}{lsnr} & p=14 & 1 & 0.95/1/1 & 1 & 0.95/1/1 & 1 & 0.67/1/0.99 & 1 & 0.95/1/1 & 0.96 \\ 
   & p=30 & 1 & 0.92/0.99/0.99 & 1 & 0.92/0.99/0.99 & 0.71 & 0.73/0.75/0.7 & 1 & 0.92/0.99/0.99 & 0.93 \\ 
   & p=60 & 1 & 1/0.97/0.98 & 1 & 1/0.97/0.98 & 0.83 & 0.94/0.75/0.74 & 1 & 1/0.97/0.98 & - \\ 
   & p=180 & 1 & 0.73/0.98/0.98 & 1 & 0.73/0.98/0.98 & 0.87 & 1/0.74/0.73 & 1 & 0.72/0.98/0.98 & - \\ 
   \midrule 
 \multicolumn{1}{|c}{} &       & \multicolumn{9}{c|}{Sparsistency (number of extra variables)} \\
\midrule\multirow{4}[2]{*}{hsnr} & p=14 & 14 & 14/14/14 & 14 & 14/14/14 & 14 & 14/14/14 & 14 & 14/14/14 & 14 \\ 
   & p=30 & 30 & 29.8/30/29.9 & 30 & 29.8/30/29.9 & 30 & 28.6/30/29.9 & 30 & 29.8/30/29.9 & 29.8 \\ 
   & p=60 & 44.9 & 39.8/50.9/48.7 & 44.2 & 39.7/50.4/48.2 & 28.5 & 30.5/27.6/27.4 & 45.1 & 39.8/50.8/48.6 & - \\ 
   & p=180 & 32.1 & 58.9/32.4/32.3 & 31.8 & 58.9/31.6/31.6 & 27 & 31.3/25/24.9 & 32 & 59.9/32.1/32 & - \\ 
  \midrule\multirow{4}[2]{*}{msnr} & p=14 & 14 & 14/14/14 & 14 & 14/14/14 & 14 & 14/14/14 & 14 & 14/14/14 & 14 \\ 
   & p=30 & 30 & 27.1/29.9/29.6 & 30 & 27.1/29.9/29.6 & 30 & 22.5/29.5/28.6 & 30 & 27.1/29.9/29.6 & 28.2 \\ 
   & p=60 & 34.8 & 33.3/42.8/40.1 & 33.9 & 33.2/41.9/39.2 & 20.4 & 22.9/19.4/19.2 & 34.6 & 33.3/42.8/40 & - \\ 
   & p=180 & 24.2 & 52.4/24.4/24.3 & 24 & 52.6/23.6/23.6 & 19.2 & 23.6/17.3/17.2 & 24.1 & 53.5/24.1/24.1 & - \\ 
  \midrule\multirow{4}[2]{*}{lsnr} & p=14 & 14 & 13.6/14/13.9 & 14 & 13.6/14/13.9 & 14 & 11.7/14/13.9 & 14 & 13.6/14/13.9 & 13.7 \\ 
   & p=30 & 28.8 & 19.9/28.2/26.9 & 28.8 & 19.9/28.1/26.8 & 13.5 & 12.5/16.7/14.1 & 28.8 & 19.9/28.2/26.9 & 22.3 \\ 
   & p=60 & 21.6 & 24.8/30.6/27.9 & 20.9 & 24.7/29.2/26.9 & 10 & 12.7/8.7/8.5 & 21.8 & 24.9/30.4/27.7 & - \\ 
   & p=180 & 13.9 & 43.8/14/14 & 13.6 & 44.1/13.3/13.3 & 9.1 & 13.4/7/6.8 & 13.8 & 45/13.7/13.6 & - \\ 
   \bottomrule 
\end{tabular}
}
\end{table}
