# Supplementary material for: On the Use of Information Criteria for Subset Selection in Least Squares Regression
Source: arXiv:1911.10191 source file (2021-03-06)
Supplement: Supplementary file 48 [file Orth-Sparse-Ex1_n200.tex]

% latex table generated in R 3.6.1 by xtable 1.8-4 package
% Sun Nov 10 01:26:49 2019
\begin{table}[ht]
\centering
\caption{The performance of BS using different selection rules, Orth-Sparse-Ex1, n=200} 
\scalebox{0.55}{
\begin{tabular}{|c|c|cc|cc|cc|cc|c|}
  \toprule 
 \multicolumn{1}{|c}{} &       & \multicolumn{2}{c|}{C$_p$} & \multicolumn{2}{c|}{AICc} & \multicolumn{2}{c|}{BIC} & \multicolumn{2}{c|}{GCV} & \multirow{2}[2]{*}{CV} \\
 \multicolumn{1}{|c}{} &       & edf   & ndf/hdf/bdf & edf   & ndf/hdf/bdf & edf   & ndf/hdf/bdf & edf   & ndf/hdf/bdf &       \\
 \cmidrule{3-11}\multicolumn{1}{|c}{} &       & \multicolumn{9}{c|}{\% worse than the best possible BS} \\
 \midrule\multirow{4}[2]{*}{hsnr} & p=14 & 8 & 33/9/11 & 7 & 33/6/9 & 0 & 10/0/1 & 9 & 34/8/10 & 19 \\ 
   & p=30 & 4 & 84/5/7 & 2 & 83/2/5 & 0 & 28/0/0 & 4 & 86/4/7 & 24 \\ 
   & p=60 & 2 & 157/3/5 & 1 & 159/2/3 & 0 & 64/0/0 & 2 & 167/3/4 & - \\ 
   & p=180 & 1 & 338/30/32 & 0 & 392/1/2 & 0 & 206/0/0 & 0 & 431/2/3 & - \\ 
  \midrule\multirow{4}[2]{*}{msnr} & p=14 & 8 & 33/14/12 & 7 & 33/11/10 & 0 & 10/2/1 & 9 & 34/14/12 & 19 \\ 
   & p=30 & 4 & 84/12/11 & 2 & 83/8/7 & 0 & 28/1/2 & 4 & 86/10/10 & 24 \\ 
   & p=60 & 2 & 157/13/10 & 1 & 159/8/7 & 0 & 64/2/2 & 2 & 167/11/9 & - \\ 
   & p=180 & 1 & 338/40/38 & 0 & 392/7/6 & 0 & 206/3/4 & 0 & 431/10/8 & - \\ 
  \midrule\multirow{4}[2]{*}{lsnr} & p=14 & 18 & 16/23/23 & 18 & 17/24/24 & 93 & 43/97/93 & 18 & 16/23/23 & 26 \\ 
   & p=30 & 20 & 25/36/33 & 21 & 24/37/35 & 68 & 23/68/67 & 21 & 26/37/35 & 28 \\ 
   & p=60 & 18 & 44/28/27 & 21 & 45/31/30 & 43 & 17/43/43 & 20 & 48/30/29 & - \\ 
   & p=180 & 15 & 108/35/34 & 18 & 132/22/22 & 25 & 50/25/25 & 17 & 149/22/21 & - \\ 
   \midrule 
 \multicolumn{1}{|c}{} &       & \multicolumn{9}{c|}{Relative efficiency} \\
\midrule\multirow{4}[2]{*}{hsnr} & p=14 & 0.93 & 0.75/0.92/0.9 & 0.94 & 0.75/0.94/0.92 & 1 & 0.91/1/0.99 & 0.92 & 0.75/0.92/0.91 & 0.84 \\ 
   & p=30 & 0.96 & 0.54/0.95/0.93 & 0.98 & 0.55/0.98/0.96 & 1 & 0.78/1/1 & 0.96 & 0.54/0.96/0.94 & 0.81 \\ 
   & p=60 & 0.98 & 0.39/0.97/0.95 & 0.99 & 0.39/0.98/0.97 & 1 & 0.61/1/1 & 0.98 & 0.38/0.97/0.96 & - \\ 
   & p=180 & 0.99 & 0.23/0.77/0.76 & 1 & 0.2/0.99/0.98 & 1 & 0.33/1/1 & 1 & 0.19/0.98/0.97 & - \\ 
  \midrule\multirow{4}[2]{*}{msnr} & p=14 & 0.93 & 0.75/0.88/0.89 & 0.94 & 0.75/0.9/0.91 & 1 & 0.91/0.99/0.99 & 0.92 & 0.75/0.88/0.9 & 0.84 \\ 
   & p=30 & 0.96 & 0.54/0.89/0.9 & 0.98 & 0.55/0.92/0.93 & 1 & 0.78/0.99/0.98 & 0.96 & 0.54/0.91/0.91 & 0.81 \\ 
   & p=60 & 0.98 & 0.39/0.89/0.91 & 0.99 & 0.39/0.92/0.93 & 1 & 0.61/0.98/0.98 & 0.98 & 0.38/0.9/0.92 & - \\ 
   & p=180 & 0.99 & 0.23/0.71/0.72 & 1 & 0.2/0.93/0.94 & 1 & 0.33/0.97/0.96 & 1 & 0.19/0.91/0.92 & - \\ 
  \midrule\multirow{4}[2]{*}{lsnr} & p=14 & 0.99 & 1/0.95/0.95 & 0.98 & 1/0.94/0.94 & 0.6 & 0.82/0.59/0.6 & 0.99 & 1/0.95/0.94 & 0.92 \\ 
   & p=30 & 1 & 0.97/0.89/0.9 & 1 & 0.97/0.88/0.89 & 0.72 & 0.98/0.72/0.72 & 0.99 & 0.96/0.88/0.89 & 0.94 \\ 
   & p=60 & 0.99 & 0.81/0.92/0.92 & 0.97 & 0.81/0.89/0.9 & 0.82 & 1/0.82/0.82 & 0.98 & 0.79/0.9/0.91 & - \\ 
   & p=180 & 1 & 0.55/0.86/0.86 & 0.97 & 0.5/0.95/0.95 & 0.93 & 0.77/0.93/0.93 & 0.98 & 0.46/0.95/0.95 & - \\ 
   \midrule 
 \multicolumn{1}{|c}{} &       & \multicolumn{9}{c|}{Sparsistency (number of extra variables)} \\
\midrule\multirow{4}[2]{*}{hsnr} & p=14 & 6(0.2) & 6(1.3)/6(0.4)/6(0.4) & 6(0.2) & 6(1.2)/6(0.2)/6(0.3) & 6(0) & 6(0.2)/6(0)/6(0) & 6(0.3) & 6(1.3)/6(0.4)/6(0.4) & 6(0.7) \\ 
   & p=30 & 6(0.1) & 6(3.9)/6(0.2)/6(0.2) & 6(0) & 6(3.8)/6(0.1)/6(0.1) & 6(0) & 6(0.6)/6(0)/6(0) & 6(0.1) & 6(4.1)/6(0.1)/6(0.1) & 6(0.7) \\ 
   & p=60 & 6(0) & 6(8.9)/6(0)/6(0.1) & 6(0) & 6(9.2)/6(0)/6(0) & 6(0) & 6(1.6)/6(0)/6(0) & 6(0) & 6(10.5)/6(0)/6(0.1) & - \\ 
   & p=180 & 6(0) & 6(32.2)/6(6.4)/6(6.3) & 6(0) & 6(48.9)/6(0)/6(0) & 6(0) & 6(9.5)/6(0)/6(0) & 6(0) & 6(74.6)/6(0)/6(0) & - \\ 
  \midrule\multirow{4}[2]{*}{msnr} & p=14 & 6(0.2) & 6(1.3)/6(0.7)/6(0.4) & 6(0.2) & 6(1.2)/6(0.5)/6(0.3) & 6(0) & 6(0.2)/6(0)/6(0) & 6(0.3) & 6(1.3)/6(0.6)/6(0.4) & 6(0.7) \\ 
   & p=30 & 6(0.1) & 6(3.9)/6(0.4)/6(0.3) & 6(0) & 6(3.8)/6(0.2)/6(0.1) & 6(0) & 6(0.6)/6(0)/6(0) & 6(0.1) & 6(4.1)/6(0.3)/6(0.2) & 6(0.7) \\ 
   & p=60 & 6(0) & 6(8.9)/6(0.3)/6(0.2) & 6(0) & 6(9.2)/6(0.1)/6(0.1) & 6(0) & 6(1.6)/6(0)/6(0) & 6(0) & 6(10.5)/6(0.2)/6(0.1) & - \\ 
   & p=180 & 6(0) & 6(32.2)/6(6.6)/6(6.6) & 6(0) & 6(48.9)/6(0.1)/6(0.1) & 6(0) & 6(9.5)/6(0)/6(0) & 6(0) & 6(74.6)/6(0.1)/6(0.1) & - \\ 
  \midrule\multirow{4}[2]{*}{lsnr} & p=14 & 5.5(2.3) & 5.2(1.3)/5.6(4.6)/5.4(3.6) & 5.4(2.1) & 5.2(1.2)/5.4(4.2)/5.3(3.2) & 0.9(0.1) & 3.6(0.2)/0.7(0.1)/0.9(0.1) & 5.5(2.4) & 5.3(1.3)/5.6(4.6)/5.4(3.5) & 4.9(1.6) \\ 
   & p=30 & 4.5(1.9) & 5.3(3.9)/4.2(4.9)/4.2(4) & 4.2(1.2) & 5.2(3.8)/3.3(2.2)/3.4(1.8) & 0.1(0) & 3.7(0.6)/0.1(0)/0.2(0) & 4.5(2) & 5.3(4.1)/3.9(4.1)/3.9(3.3) & 4(1.9) \\ 
   & p=60 & 3.4(1.1) & 5.2(8.9)/2.7(1.8)/2.8(1.6) & 2.7(0.6) & 5.3(9.2)/1.5(0.2)/1.7(0.3) & 0(0) & 3.8(1.4)/0.1(0)/0.1(0) & 3.1(0.9) & 5.4(10.4)/2(0.6)/2.1(0.7) & - \\ 
   & p=180 & 1.9(0.5) & 5.3(32.2)/1.8(10.9)/1.9(9.8) & 1.1(0.1) & 5.6(49)/0.5(0)/0.6(0) & 0(0) & 4.2(8.4)/0(0)/0(0) & 1.4(0.2) & 5.8(74.6)/0.7(0.1)/0.8(0.1) & - \\ 
   \bottomrule 
\end{tabular}
}
\end{table}
