# Supplementary material for: On the Use of Information Criteria for Subset Selection in Least Squares Regression
Source: arXiv:1911.10191 source file (2021-03-06)
Supplement: Supplementary file 49 [file Orth-Sparse-Ex1_n2000.tex]

% latex table generated in R 3.6.1 by xtable 1.8-4 package
% Sun Nov 10 01:26:57 2019
\begin{table}[ht]
\centering
\caption{The performance of BS using different selection rules, Orth-Sparse-Ex1, n=2000} 
\scalebox{0.65}{
\begin{tabular}{|c|c|cc|cc|cc|cc|c|}
  \toprule 
 \multicolumn{1}{|c}{} &       & \multicolumn{2}{c|}{C$_p$} & \multicolumn{2}{c|}{AICc} & \multicolumn{2}{c|}{BIC} & \multicolumn{2}{c|}{GCV} & \multirow{2}[2]{*}{CV} \\
 \multicolumn{1}{|c}{} &       & edf   & ndf/hdf/bdf & edf   & ndf/hdf/bdf & edf   & ndf/hdf/bdf & edf   & ndf/hdf/bdf &       \\
 \cmidrule{3-11}\multicolumn{1}{|c}{} &       & \multicolumn{9}{c|}{\% worse than the best possible BS} \\
 \midrule\multirow{4}[2]{*}{hsnr} & p=14 & 8 & 33/7/9 & 8 & 33/7/9 & 0 & 3/0/0 & 8 & 33/7/9 & 18 \\ 
   & p=30 & 3 & 85/3/6 & 3 & 85/3/6 & 0 & 9/0/0 & 3 & 86/3/6 & 23 \\ 
   & p=60 & 2 & 155/2/4 & 2 & 156/2/4 & 0 & 21/0/0 & 2 & 156/2/4 & - \\ 
   & p=180 & 0 & 334/1/3 & 1 & 337/1/3 & 0 & 60/0/0 & 1 & 340/1/3 & - \\ 
  \midrule\multirow{4}[2]{*}{msnr} & p=14 & 8 & 33/7/9 & 8 & 33/7/9 & 0 & 3/0/0 & 8 & 33/7/9 & 18 \\ 
   & p=30 & 3 & 85/3/6 & 3 & 85/3/6 & 0 & 9/0/0 & 3 & 86/3/6 & 23 \\ 
   & p=60 & 2 & 155/2/4 & 2 & 156/2/4 & 0 & 21/0/0 & 2 & 156/2/4 & - \\ 
   & p=180 & 0 & 334/1/3 & 1 & 337/1/3 & 0 & 60/0/0 & 1 & 340/1/3 & - \\ 
  \midrule\multirow{4}[2]{*}{lsnr} & p=14 & 8 & 33/9/9 & 8 & 33/9/9 & 0 & 3/0/0 & 8 & 33/9/9 & 18 \\ 
   & p=30 & 3 & 85/6/7 & 3 & 85/5/6 & 0 & 9/0/0 & 3 & 86/6/7 & 23 \\ 
   & p=60 & 2 & 155/5/5 & 2 & 156/5/5 & 0 & 21/0/0 & 2 & 156/5/5 & - \\ 
   & p=180 & 0 & 334/5/4 & 1 & 337/4/4 & 0 & 60/1/1 & 1 & 340/5/4 & - \\ 
   \midrule 
 \multicolumn{1}{|c}{} &       & \multicolumn{9}{c|}{Relative efficiency} \\
\midrule\multirow{4}[2]{*}{hsnr} & p=14 & 0.93 & 0.75/0.94/0.92 & 0.93 & 0.75/0.94/0.92 & 1 & 0.97/1/1 & 0.92 & 0.75/0.94/0.92 & 0.84 \\ 
   & p=30 & 0.97 & 0.54/0.97/0.94 & 0.97 & 0.54/0.97/0.94 & 1 & 0.92/1/1 & 0.97 & 0.54/0.97/0.94 & 0.81 \\ 
   & p=60 & 0.98 & 0.39/0.98/0.96 & 0.98 & 0.39/0.98/0.96 & 1 & 0.83/1/1 & 0.98 & 0.39/0.98/0.96 & - \\ 
   & p=180 & 1 & 0.23/0.99/0.97 & 0.99 & 0.23/0.99/0.97 & 1 & 0.62/1/1 & 0.99 & 0.23/0.99/0.97 & - \\ 
  \midrule\multirow{4}[2]{*}{msnr} & p=14 & 0.93 & 0.75/0.94/0.92 & 0.93 & 0.75/0.94/0.92 & 1 & 0.97/1/1 & 0.92 & 0.75/0.94/0.92 & 0.84 \\ 
   & p=30 & 0.97 & 0.54/0.97/0.94 & 0.97 & 0.54/0.97/0.94 & 1 & 0.92/1/1 & 0.97 & 0.54/0.97/0.94 & 0.81 \\ 
   & p=60 & 0.98 & 0.39/0.98/0.96 & 0.98 & 0.39/0.98/0.96 & 1 & 0.83/1/1 & 0.98 & 0.39/0.98/0.96 & - \\ 
   & p=180 & 1 & 0.23/0.99/0.97 & 0.99 & 0.23/0.99/0.97 & 1 & 0.62/1/1 & 0.99 & 0.23/0.99/0.97 & - \\ 
  \midrule\multirow{4}[2]{*}{lsnr} & p=14 & 0.93 & 0.75/0.92/0.92 & 0.93 & 0.75/0.92/0.92 & 1 & 0.97/1/1 & 0.92 & 0.75/0.92/0.92 & 0.84 \\ 
   & p=30 & 0.97 & 0.54/0.95/0.94 & 0.97 & 0.54/0.95/0.94 & 1 & 0.92/1/1 & 0.97 & 0.54/0.95/0.94 & 0.81 \\ 
   & p=60 & 0.98 & 0.39/0.95/0.95 & 0.98 & 0.39/0.95/0.95 & 1 & 0.83/1/1 & 0.98 & 0.39/0.95/0.95 & - \\ 
   & p=180 & 1 & 0.23/0.96/0.96 & 0.99 & 0.23/0.96/0.96 & 1 & 0.62/0.99/0.99 & 0.99 & 0.23/0.96/0.96 & - \\ 
   \midrule 
 \multicolumn{1}{|c}{} &       & \multicolumn{9}{c|}{Sparsistency (number of extra variables)} \\
\midrule\multirow{4}[2]{*}{hsnr} & p=14 & 6(0.3) & 6(1.2)/6(0.3)/6(0.3) & 6(0.3) & 6(1.2)/6(0.3)/6(0.3) & 6(0) & 6(0)/6(0)/6(0) & 6(0.3) & 6(1.2)/6(0.3)/6(0.3) & 6(0.6) \\ 
   & p=30 & 6(0.1) & 6(3.8)/6(0.1)/6(0.2) & 6(0.1) & 6(3.8)/6(0.1)/6(0.2) & 6(0) & 6(0.1)/6(0)/6(0) & 6(0.1) & 6(3.9)/6(0.1)/6(0.2) & 6(0.6) \\ 
   & p=60 & 6(0) & 6(8.6)/6(0)/6(0) & 6(0) & 6(8.6)/6(0)/6(0) & 6(0) & 6(0.3)/6(0)/6(0) & 6(0) & 6(8.7)/6(0)/6(0) & - \\ 
   & p=180 & 6(0) & 6(27.5)/6(0)/6(0) & 6(0) & 6(28.2)/6(0)/6(0) & 6(0) & 6(1.1)/6(0)/6(0) & 6(0) & 6(28.9)/6(0)/6(0) & - \\ 
  \midrule\multirow{4}[2]{*}{msnr} & p=14 & 6(0.3) & 6(1.2)/6(0.3)/6(0.3) & 6(0.3) & 6(1.2)/6(0.3)/6(0.3) & 6(0) & 6(0)/6(0)/6(0) & 6(0.3) & 6(1.2)/6(0.3)/6(0.3) & 6(0.6) \\ 
   & p=30 & 6(0.1) & 6(3.8)/6(0.1)/6(0.2) & 6(0.1) & 6(3.8)/6(0.1)/6(0.2) & 6(0) & 6(0.1)/6(0)/6(0) & 6(0.1) & 6(3.9)/6(0.1)/6(0.2) & 6(0.6) \\ 
   & p=60 & 6(0) & 6(8.6)/6(0)/6(0) & 6(0) & 6(8.6)/6(0)/6(0) & 6(0) & 6(0.3)/6(0)/6(0) & 6(0) & 6(8.7)/6(0)/6(0) & - \\ 
   & p=180 & 6(0) & 6(27.5)/6(0)/6(0) & 6(0) & 6(28.2)/6(0)/6(0) & 6(0) & 6(1.1)/6(0)/6(0) & 6(0) & 6(28.9)/6(0)/6(0) & - \\ 
  \midrule\multirow{4}[2]{*}{lsnr} & p=14 & 6(0.3) & 6(1.2)/6(0.4)/6(0.3) & 6(0.3) & 6(1.2)/6(0.4)/6(0.3) & 6(0) & 6(0)/6(0)/6(0) & 6(0.3) & 6(1.2)/6(0.4)/6(0.3) & 6(0.6) \\ 
   & p=30 & 6(0.1) & 6(3.8)/6(0.2)/6(0.2) & 6(0.1) & 6(3.8)/6(0.2)/6(0.2) & 6(0) & 6(0.1)/6(0)/6(0) & 6(0.1) & 6(3.9)/6(0.2)/6(0.2) & 6(0.6) \\ 
   & p=60 & 6(0) & 6(8.6)/6(0.1)/6(0.1) & 6(0) & 6(8.6)/6(0.1)/6(0.1) & 6(0) & 6(0.3)/6(0)/6(0) & 6(0) & 6(8.7)/6(0.1)/6(0.1) & - \\ 
   & p=180 & 6(0) & 6(27.5)/6(0.1)/6(0) & 6(0) & 6(28.2)/6(0.1)/6(0) & 6(0) & 6(1.1)/6(0)/6(0) & 6(0) & 6(28.9)/6(0.1)/6(0) & - \\ 
   \bottomrule 
\end{tabular}
}
\end{table}
