# Supplementary material for: On the Use of Information Criteria for Subset Selection in Least Squares Regression
Source: arXiv:1911.10191 source file (2021-03-06)
Supplement: Supplementary file 50 [file Orth-Sparse-Ex2_n200.tex]

% latex table generated in R 3.6.1 by xtable 1.8-4 package
% Sun Nov 10 01:26:58 2019
\begin{table}[ht]
\centering
\caption{The performance of BS using different selection rules, Orth-Sparse-Ex2, n=200} 
\scalebox{0.55}{
\begin{tabular}{|c|c|cc|cc|cc|cc|c|}
  \toprule 
 \multicolumn{1}{|c}{} &       & \multicolumn{2}{c|}{C$_p$} & \multicolumn{2}{c|}{AICc} & \multicolumn{2}{c|}{BIC} & \multicolumn{2}{c|}{GCV} & \multirow{2}[2]{*}{CV} \\
 \multicolumn{1}{|c}{} &       & edf   & ndf/hdf/bdf & edf   & ndf/hdf/bdf & edf   & ndf/hdf/bdf & edf   & ndf/hdf/bdf &       \\
 \cmidrule{3-11}\multicolumn{1}{|c}{} &       & \multicolumn{9}{c|}{\% worse than the best possible BS} \\
 \midrule\multirow{4}[2]{*}{hsnr} & p=14 & 23 & 21/32/29 & 23 & 21/32/28 & 39 & 20/40/38 & 24 & 21/32/29 & 23 \\ 
   & p=30 & 21 & 48/27/26 & 21 & 47/25/23 & 27 & 20/27/26 & 21 & 49/27/25 & 24 \\ 
   & p=60 & 17 & 89/20/19 & 17 & 91/18/18 & 19 & 33/19/18 & 17 & 96/18/18 & - \\ 
   & p=180 & 12 & 200/32/33 & 11 & 236/11/11 & 11 & 112/11/11 & 11 & 262/11/12 & - \\ 
  \midrule\multirow{4}[2]{*}{msnr} & p=14 & 13 & 33/23/20 & 11 & 33/21/17 & 3 & 14/12/11 & 14 & 34/23/19 & 21 \\ 
   & p=30 & 6 & 78/21/19 & 4 & 78/15/14 & 1 & 28/19/18 & 6 & 80/18/17 & 24 \\ 
   & p=60 & 3 & 146/20/17 & 3 & 148/14/13 & 1 & 59/34/28 & 3 & 155/17/15 & - \\ 
   & p=180 & 3 & 314/50/50 & 2 & 365/15/15 & 2 & 184/65/57 & 3 & 400/16/16 & - \\ 
  \midrule\multirow{4}[2]{*}{lsnr} & p=14 & 25 & 26/34/32 & 25 & 26/34/33 & 52 & 24/91/77 & 26 & 27/34/33 & 27 \\ 
   & p=30 & 21 & 54/37/34 & 20 & 54/34/31 & 48 & 23/90/79 & 22 & 56/35/33 & 29 \\ 
   & p=60 & 19 & 95/34/32 & 17 & 97/33/31 & 49 & 35/84/76 & 18 & 102/33/32 & - \\ 
   & p=180 & 15 & 198/57/54 & 15 & 235/39/35 & 56 & 105/72/68 & 15 & 260/37/34 & - \\ 
   \midrule 
 \multicolumn{1}{|c}{} &       & \multicolumn{9}{c|}{Relative efficiency} \\
\midrule\multirow{4}[2]{*}{hsnr} & p=14 & 0.97 & 0.99/0.91/0.93 & 0.97 & 0.99/0.91/0.93 & 0.86 & 1/0.86/0.87 & 0.97 & 0.99/0.91/0.93 & 0.97 \\ 
   & p=30 & 0.99 & 0.81/0.94/0.95 & 0.99 & 0.81/0.96/0.97 & 0.94 & 1/0.94/0.95 & 0.99 & 0.8/0.95/0.96 & 0.97 \\ 
   & p=60 & 0.99 & 0.62/0.97/0.98 & 1 & 0.61/0.99/0.99 & 0.98 & 0.87/0.98/0.98 & 1 & 0.59/0.98/0.99 & - \\ 
   & p=180 & 0.99 & 0.37/0.84/0.84 & 1 & 0.33/1/1 & 1 & 0.52/1/1 & 1 & 0.31/1/0.99 & - \\ 
  \midrule\multirow{4}[2]{*}{msnr} & p=14 & 0.91 & 0.77/0.83/0.85 & 0.92 & 0.77/0.85/0.87 & 1 & 0.9/0.92/0.93 & 0.9 & 0.77/0.83/0.86 & 0.85 \\ 
   & p=30 & 0.95 & 0.57/0.84/0.85 & 0.97 & 0.57/0.88/0.89 & 1 & 0.79/0.85/0.86 & 0.95 & 0.56/0.86/0.86 & 0.81 \\ 
   & p=60 & 0.98 & 0.41/0.84/0.86 & 0.99 & 0.41/0.88/0.89 & 1 & 0.64/0.76/0.79 & 0.98 & 0.4/0.86/0.88 & - \\ 
   & p=180 & 0.99 & 0.25/0.68/0.68 & 1 & 0.22/0.89/0.89 & 1 & 0.36/0.62/0.65 & 1 & 0.2/0.88/0.88 & - \\ 
  \midrule\multirow{4}[2]{*}{lsnr} & p=14 & 0.99 & 0.98/0.92/0.93 & 0.99 & 0.98/0.92/0.93 & 0.81 & 1/0.65/0.7 & 0.98 & 0.97/0.92/0.93 & 0.97 \\ 
   & p=30 & 0.99 & 0.78/0.88/0.9 & 1 & 0.78/0.9/0.92 & 0.82 & 0.98/0.63/0.67 & 0.98 & 0.77/0.89/0.9 & 0.93 \\ 
   & p=60 & 0.99 & 0.6/0.88/0.89 & 1 & 0.6/0.88/0.9 & 0.79 & 0.87/0.64/0.67 & 0.99 & 0.58/0.88/0.89 & - \\ 
   & p=180 & 1 & 0.39/0.73/0.75 & 1 & 0.34/0.83/0.85 & 0.74 & 0.56/0.67/0.69 & 1 & 0.32/0.84/0.86 & - \\ 
   \midrule 
 \multicolumn{1}{|c}{} &       & \multicolumn{9}{c|}{Sparsistency (number of extra variables)} \\
\midrule\multirow{4}[2]{*}{hsnr} & p=14 & 5.3(0.9) & 5.6(1.3)/5.1(1.7)/5.2(1.2) & 5.2(0.7) & 5.6(1.2)/5(1.3)/5.1(1) & 4.1(0) & 5.1(0.2)/4.1(0)/4.2(0) & 5.3(0.9) & 5.6(1.3)/5.1(1.6)/5.2(1.2) & 5.3(1) \\ 
   & p=30 & 4.8(0.4) & 5.6(3.9)/4.6(0.8)/4.7(0.7) & 4.7(0.2) & 5.6(3.8)/4.5(0.2)/4.6(0.2) & 4(0) & 5.1(0.6)/4(0)/4.1(0) & 4.8(0.4) & 5.7(4.1)/4.5(0.6)/4.6(0.6) & 5(0.9) \\ 
   & p=60 & 4.5(0.2) & 5.6(8.9)/4.3(0.3)/4.4(0.3) & 4.4(0.1) & 5.7(9.2)/4.2(0.1)/4.3(0.1) & 4(0) & 5.1(1.5)/4(0)/4(0) & 4.4(0.1) & 5.7(10.5)/4.3(0.1)/4.4(0.1) & - \\ 
   & p=180 & 4.2(0) & 5.7(32.2)/4.3(7.8)/4.4(7.4) & 4.1(0) & 5.8(48.9)/4.1(0)/4.1(0) & 4(0) & 5.3(9.1)/4(0)/4(0) & 4.2(0) & 5.9(74.6)/4.1(0)/4.2(0.1) & - \\ 
  \midrule\multirow{4}[2]{*}{msnr} & p=14 & 4.2(0.4) & 4.8(1.3)/4.5(1.2)/4.4(0.9) & 4.2(0.3) & 4.8(1.2)/4.4(1)/4.3(0.6) & 4(0) & 4.3(0.2)/4(0)/4(0) & 4.2(0.5) & 4.8(1.3)/4.5(1.2)/4.4(0.8) & 4.4(0.7) \\ 
   & p=30 & 4.1(0.1) & 4.8(3.9)/4.2(0.7)/4.2(0.6) & 4(0.1) & 4.8(3.8)/4.1(0.3)/4.1(0.2) & 4(0) & 4.3(0.6)/3.8(0)/3.9(0) & 4.1(0.2) & 4.8(4.1)/4.2(0.5)/4.1(0.5) & 4.2(0.7) \\ 
   & p=60 & 4(0) & 4.8(8.9)/4.1(0.3)/4.1(0.3) & 4(0) & 4.8(9.3)/4(0.2)/4(0.1) & 4(0) & 4.3(1.5)/3.7(0)/3.8(0) & 4(0) & 4.9(10.5)/4.1(0.2)/4(0.2) & - \\ 
   & p=180 & 4(0) & 4.8(32.2)/4.1(7.3)/4.1(7) & 4(0) & 5.1(49.2)/3.9(0.1)/3.9(0.1) & 4(0) & 4.4(8.9)/3.4(0)/3.5(0) & 4(0) & 5.3(74.7)/3.9(0.1)/3.9(0.1) & - \\ 
  \midrule\multirow{4}[2]{*}{lsnr} & p=14 & 3.4(1) & 3.8(1.3)/3.9(2.4)/3.7(1.8) & 3.3(0.8) & 3.8(1.2)/3.7(2.1)/3.5(1.5) & 1.8(0) & 2.8(0.2)/1.1(0)/1.4(0) & 3.4(1.1) & 3.8(1.3)/3.9(2.4)/3.6(1.7) & 3.2(0.8) \\ 
   & p=30 & 2.7(0.6) & 3.8(3.9)/2.8(2)/2.7(1.5) & 2.6(0.4) & 3.8(3.8)/2.5(0.9)/2.4(0.7) & 1.5(0) & 2.8(0.6)/0.6(0)/0.9(0) & 2.7(0.7) & 3.9(4.1)/2.7(1.4)/2.6(1.2) & 2.8(1) \\ 
   & p=60 & 2.3(0.3) & 3.8(8.9)/2.2(0.9)/2.2(0.8) & 2.2(0.2) & 3.9(9.3)/1.8(0.2)/1.9(0.3) & 1.2(0) & 2.8(1.5)/0.4(0)/0.6(0) & 2.2(0.3) & 4(10.5)/2(0.4)/2(0.4) & - \\ 
   & p=180 & 1.9(0.3) & 3.9(32.2)/1.8(9)/1.9(8.2) & 1.8(0.2) & 4.3(49.6)/1.1(0.1)/1.2(0.1) & 0.6(0) & 3.1(8.4)/0.2(0)/0.3(0) & 1.9(0.2) & 4.7(74.7)/1.2(0.1)/1.3(0.1) & - \\ 
   \bottomrule 
\end{tabular}
}
\end{table}
