# Supplementary material for: On the Use of Information Criteria for Subset Selection in Least Squares Regression
Source: arXiv:1911.10191 source file (2021-03-06)
Supplement: Supplementary file 51 [file Orth-Sparse-Ex2_n2000.tex]

% latex table generated in R 3.6.1 by xtable 1.8-4 package
% Sun Nov 10 01:27:05 2019
\begin{table}[ht]
\centering
\caption{The performance of BS using different selection rules, Orth-Sparse-Ex2, n=2000} 
\scalebox{0.55}{
\begin{tabular}{|c|c|cc|cc|cc|cc|c|}
  \toprule 
 \multicolumn{1}{|c}{} &       & \multicolumn{2}{c|}{C$_p$} & \multicolumn{2}{c|}{AICc} & \multicolumn{2}{c|}{BIC} & \multicolumn{2}{c|}{GCV} & \multirow{2}[2]{*}{CV} \\
 \multicolumn{1}{|c}{} &       & edf   & ndf/hdf/bdf & edf   & ndf/hdf/bdf & edf   & ndf/hdf/bdf & edf   & ndf/hdf/bdf &       \\
 \cmidrule{3-11}\multicolumn{1}{|c}{} &       & \multicolumn{9}{c|}{\% worse than the best possible BS} \\
 \midrule\multirow{4}[2]{*}{hsnr} & p=14 & 8 & 33/10/9 & 8 & 33/9/9 & 0 & 3/0/1 & 8 & 33/9/9 & 18 \\ 
   & p=30 & 3 & 85/6/7 & 3 & 85/5/6 & 0 & 9/0/0 & 3 & 86/6/7 & 23 \\ 
   & p=60 & 2 & 155/4/5 & 2 & 156/4/5 & 0 & 21/1/1 & 2 & 156/4/5 & - \\ 
   & p=180 & 0 & 334/4/4 & 1 & 337/4/3 & 0 & 60/4/3 & 1 & 340/4/4 & - \\ 
  \midrule\multirow{4}[2]{*}{msnr} & p=14 & 13 & 27/31/28 & 13 & 27/32/27 & 47 & 26/95/80 & 13 & 27/32/28 & 22 \\ 
   & p=30 & 14 & 66/39/35 & 13 & 66/39/35 & 74 & 23/93/86 & 13 & 66/39/35 & 31 \\ 
   & p=60 & 15 & 111/39/35 & 14 & 111/38/35 & 80 & 22/82/78 & 15 & 112/39/35 & - \\ 
   & p=180 & 15 & 217/37/35 & 16 & 219/37/35 & 63 & 34/63/62 & 16 & 221/37/35 & - \\ 
  \midrule\multirow{4}[2]{*}{lsnr} & p=14 & 15 & 29/19/17 & 15 & 29/19/17 & 4 & 8/8/7 & 15 & 29/19/17 & 20 \\ 
   & p=30 & 7 & 71/13/12 & 7 & 71/13/12 & 1 & 11/10/7 & 7 & 71/13/12 & 24 \\ 
   & p=60 & 3 & 131/10/9 & 3 & 131/10/9 & 1 & 19/16/11 & 3 & 132/10/9 & - \\ 
   & p=180 & 1 & 288/9/8 & 1 & 291/8/7 & 0 & 51/35/30 & 1 & 293/9/8 & - \\ 
   \midrule 
 \multicolumn{1}{|c}{} &       & \multicolumn{9}{c|}{Relative efficiency} \\
\midrule\multirow{4}[2]{*}{hsnr} & p=14 & 0.93 & 0.75/0.91/0.91 & 0.93 & 0.75/0.92/0.92 & 1 & 0.97/1/0.99 & 0.92 & 0.75/0.91/0.91 & 0.84 \\ 
   & p=30 & 0.97 & 0.54/0.95/0.94 & 0.97 & 0.54/0.95/0.94 & 1 & 0.92/1/1 & 0.97 & 0.54/0.95/0.94 & 0.81 \\ 
   & p=60 & 0.98 & 0.39/0.96/0.95 & 0.98 & 0.39/0.96/0.96 & 1 & 0.83/0.99/0.99 & 0.98 & 0.39/0.96/0.95 & - \\ 
   & p=180 & 1 & 0.23/0.96/0.97 & 0.99 & 0.23/0.97/0.97 & 1 & 0.62/0.96/0.97 & 0.99 & 0.23/0.96/0.97 & - \\ 
  \midrule\multirow{4}[2]{*}{msnr} & p=14 & 1 & 0.89/0.86/0.88 & 1 & 0.89/0.86/0.89 & 0.77 & 0.9/0.58/0.63 & 1 & 0.89/0.86/0.88 & 0.93 \\ 
   & p=30 & 1 & 0.68/0.82/0.84 & 1 & 0.68/0.82/0.84 & 0.65 & 0.92/0.59/0.61 & 1 & 0.68/0.82/0.84 & 0.87 \\ 
   & p=60 & 1 & 0.54/0.83/0.85 & 1 & 0.54/0.83/0.85 & 0.64 & 0.94/0.63/0.64 & 1 & 0.54/0.83/0.85 & - \\ 
   & p=180 & 1 & 0.36/0.84/0.85 & 1 & 0.36/0.84/0.85 & 0.71 & 0.86/0.71/0.71 & 1 & 0.36/0.84/0.85 & - \\ 
  \midrule\multirow{4}[2]{*}{lsnr} & p=14 & 0.9 & 0.81/0.88/0.89 & 0.91 & 0.81/0.88/0.89 & 1 & 0.96/0.97/0.97 & 0.91 & 0.81/0.88/0.89 & 0.87 \\ 
   & p=30 & 0.95 & 0.59/0.9/0.9 & 0.95 & 0.59/0.9/0.91 & 1 & 0.92/0.92/0.95 & 0.95 & 0.59/0.9/0.91 & 0.82 \\ 
   & p=60 & 0.98 & 0.44/0.91/0.92 & 0.98 & 0.43/0.92/0.93 & 1 & 0.84/0.87/0.9 & 0.98 & 0.43/0.91/0.93 & - \\ 
   & p=180 & 0.99 & 0.26/0.92/0.93 & 0.99 & 0.26/0.93/0.93 & 1 & 0.66/0.74/0.77 & 0.99 & 0.26/0.92/0.93 & - \\ 
   \midrule 
 \multicolumn{1}{|c}{} &       & \multicolumn{9}{c|}{Sparsistency (number of extra variables)} \\
\midrule\multirow{4}[2]{*}{hsnr} & p=14 & 6(0.3) & 6(1.2)/6(0.4)/6(0.3) & 6(0.3) & 6(1.2)/6(0.4)/6(0.3) & 6(0) & 6(0)/6(0)/6(0) & 6(0.3) & 6(1.2)/6(0.4)/6(0.3) & 6(0.6) \\ 
   & p=30 & 6(0.1) & 6(3.8)/6(0.2)/6(0.2) & 6(0.1) & 6(3.8)/6(0.2)/6(0.2) & 6(0) & 6(0.1)/6(0)/6(0) & 6(0.1) & 6(3.9)/6(0.2)/6(0.2) & 6(0.6) \\ 
   & p=60 & 6(0) & 6(8.6)/6(0.1)/6(0.1) & 6(0) & 6(8.6)/6(0.1)/6(0.1) & 6(0) & 6(0.3)/6(0)/6(0) & 6(0) & 6(8.7)/6(0.1)/6(0.1) & - \\ 
   & p=180 & 6(0) & 6(27.5)/6(0)/6(0) & 6(0) & 6(28.2)/6(0)/6(0) & 6(0) & 6(1.1)/6(0)/6(0) & 6(0) & 6(28.9)/6(0)/6(0) & - \\ 
  \midrule\multirow{4}[2]{*}{msnr} & p=14 & 5.9(0.6) & 6(1.2)/5.8(1.7)/5.8(1.2) & 5.9(0.6) & 6(1.2)/5.8(1.7)/5.8(1.1) & 5.1(0) & 5.5(0)/4.4(0)/4.6(0) & 5.9(0.6) & 6(1.2)/5.8(1.7)/5.8(1.2) & 5.9(0.8) \\ 
   & p=30 & 5.8(0.4) & 6(3.8)/5.5(1)/5.6(0.8) & 5.8(0.4) & 6(3.8)/5.5(0.9)/5.5(0.8) & 4.5(0) & 5.5(0.1)/4.2(0)/4.3(0) & 5.8(0.4) & 6(3.9)/5.5(1)/5.6(0.8) & 5.7(1) \\ 
   & p=60 & 5.6(0.4) & 6(8.6)/5.2(0.3)/5.3(0.3) & 5.6(0.4) & 6(8.6)/5.2(0.3)/5.3(0.3) & 4.1(0) & 5.5(0.3)/4.1(0)/4.2(0) & 5.6(0.4) & 6(8.7)/5.2(0.3)/5.3(0.3) & - \\ 
   & p=180 & 5.4(0.3) & 6(27.5)/4.8(0.1)/4.8(0.1) & 5.4(0.3) & 6(28.2)/4.8(0.1)/4.8(0.1) & 4(0) & 5.5(1.1)/4(0)/4.1(0) & 5.4(0.3) & 6(28.9)/4.8(0.1)/4.8(0.1) & - \\ 
  \midrule\multirow{4}[2]{*}{lsnr} & p=14 & 4.3(0.5) & 4.9(1.2)/4.5(1)/4.4(0.6) & 4.3(0.5) & 4.9(1.2)/4.5(0.9)/4.4(0.6) & 4(0) & 4.1(0)/4(0)/4(0) & 4.3(0.5) & 4.9(1.2)/4.5(1)/4.4(0.6) & 4.5(0.7) \\ 
   & p=30 & 4.1(0.2) & 4.9(3.8)/4.2(0.4)/4.1(0.4) & 4.1(0.2) & 4.9(3.8)/4.2(0.4)/4.1(0.3) & 4(0) & 4.1(0.1)/3.9(0)/4(0) & 4.1(0.2) & 4.9(3.9)/4.2(0.4)/4.1(0.3) & 4.3(0.8) \\ 
   & p=60 & 4(0) & 4.9(8.6)/4.1(0.2)/4.1(0.1) & 4(0) & 4.9(8.6)/4.1(0.1)/4.1(0.1) & 4(0) & 4.1(0.3)/3.9(0)/3.9(0) & 4(0) & 4.9(8.7)/4.1(0.2)/4.1(0.1) & - \\ 
   & p=180 & 4(0) & 4.9(27.5)/4(0.1)/4(0.1) & 4(0) & 4.9(28.2)/4(0.1)/4(0.1) & 4(0) & 4.1(1.1)/3.7(0)/3.8(0) & 4(0) & 4.9(28.9)/4(0.1)/4(0.1) & - \\ 
   \bottomrule 
\end{tabular}
}
\end{table}
