# Supplementary material for: On the Use of Information Criteria for Subset Selection in Least Squares Regression
Source: arXiv:1911.10191 source file (2021-03-06)
Supplement: Supplementary file 52 [file Orth-Dense_n200.tex]

% latex table generated in R 3.6.2 by xtable 1.8-4 package
% Sat Dec 21 23:17:25 2019
\begin{table}[ht]
\centering
\caption{The performance of BS compared to regularization methods, Orth-Dense, n=200} 
\scalebox{0.75}{
\begin{tabular}{|c|c|ccccc|}
  \toprule 
 \multicolumn{1}{|c}{} &       & BS    & LASSO & Gamma LASSO & SparseNet & \multicolumn{1}{c|}{rLASSO}  \\
 \multicolumn{1}{|c}{} &       & AICc-hdf & AICc/CV & AICc/CV & CV    & \multicolumn{1}{c|}{CV}       \\
 \midrule\multicolumn{1}{|c}{} &       & \multicolumn{5}{c|}{\% worse than the best possible BS} \\
 \midrule\multirow{4}[2]{*}{hsnr} & p=14 & 0 & 0/0 & 0/1 & 0 & 0 \\ 
   & p=30 & 1 & 1/1 & 7/2 & 4 & 4 \\ 
   & p=60 & 11 & 2/0 & -1/0 & 2 & 4 \\ 
   & p=180 & 18 & 23/15 & 4/7 & 7 & 13 \\ 
  \midrule\multirow{4}[2]{*}{msnr} & p=14 & 0 & 1/1 & 6/1 & 3 & 3 \\ 
   & p=30 & 4 & 1/0 & 8/3 & 5 & 5 \\ 
   & p=60 & 13 & 0/-1 & 0/1 & 3 & 3 \\ 
   & p=180 & 18 & 13/10 & 18/7 & 7 & 10 \\ 
  \midrule\multirow{4}[2]{*}{lsnr} & p=14 & 8 & 5/4 & 17/8 & 11 & 11 \\ 
   & p=30 & 21 & -6/-6 & 4/0 & -2 & -1 \\ 
   & p=60 & 13 & -6/-6 & 13/-1 & -3 & -2 \\ 
   & p=180 & 7 & -2/0 & 73/3 & 2 & 2 \\ 
   \midrule 
 \multicolumn{1}{|c}{} &       & \multicolumn{5}{c|}{Relative efficiency} \\
\midrule\multirow{4}[2]{*}{hsnr} & p=14 & 1 & 1/1 & 1/0.99 & 1 & 1 \\ 
   & p=30 & 1 & 1/1 & 0.94/1 & 0.97 & 0.97 \\ 
   & p=60 & 0.9 & 0.97/0.99 & 1/0.99 & 0.97 & 0.96 \\ 
   & p=180 & 0.88 & 0.84/0.9 & 1/0.97 & 0.97 & 0.92 \\ 
  \midrule\multirow{4}[2]{*}{msnr} & p=14 & 1 & 1/1 & 0.95/0.99 & 0.97 & 0.97 \\ 
   & p=30 & 0.96 & 0.99/1 & 0.93/0.97 & 0.95 & 0.95 \\ 
   & p=60 & 0.87 & 0.98/1 & 0.99/0.97 & 0.96 & 0.96 \\ 
   & p=180 & 0.9 & 0.95/0.97 & 0.91/1 & 1 & 0.97 \\ 
  \midrule\multirow{4}[2]{*}{lsnr} & p=14 & 0.96 & 0.99/0.99 & 0.88/0.96 & 0.93 & 0.93 \\ 
   & p=30 & 0.78 & 1/1 & 0.9/0.94 & 0.95 & 0.95 \\ 
   & p=60 & 0.83 & 1/1 & 0.83/0.95 & 0.96 & 0.96 \\ 
   & p=180 & 0.91 & 1/0.98 & 0.56/0.95 & 0.96 & 0.95 \\ 
   \midrule 
 \multicolumn{1}{|c}{} &       & \multicolumn{5}{c|}{Sparsistency (number of extra variables)} \\
\midrule\multirow{4}[2]{*}{hsnr} & p=14 & 14 & 14/14 & 14/14 & 14 & 14 \\ 
   & p=30 & 29.4 & 28.9/29.4 & 26.5/29.1 & 27.8 & 27.5 \\ 
   & p=60 & 25.6 & 41.5/46.2 & 30.7/38.9 & 35.1 & 32.4 \\ 
   & p=180 & 16.3 & 41.1/68.3 & 39.9/34.1 & 32.7 & 24.8 \\ 
  \midrule\multirow{4}[2]{*}{msnr} & p=14 & 14 & 13.9/14 & 13.5/13.9 & 13.6 & 13.6 \\ 
   & p=30 & 26.8 & 25.5/26.9 & 19.1/25 & 23.9 & 22.5 \\ 
   & p=60 & 15.6 & 32.8/37.5 & 23.5/29 & 28.3 & 24.7 \\ 
   & p=180 & 8.8 & 30.7/48.8 & 44/26.6 & 25.3 & 19.8 \\ 
  \midrule\multirow{4}[2]{*}{lsnr} & p=14 & 12.3 & 10.9/11.5 & 8.2/11 & 10.4 & 9.6 \\ 
   & p=30 & 8.5 & 14.1/14.8 & 10.9/13.2 & 13.3 & 11.1 \\ 
   & p=60 & 0.8 & 14.6/16 & 16.1/12.8 & 14.1 & 10.8 \\ 
   & p=180 & 0.2 & 10.5/15.3 & 51.1/12.7 & 13.6 & 9.9 \\ 
   \bottomrule 
\end{tabular}
}
\end{table}
