# Supplementary material for: On the Use of Information Criteria for Subset Selection in Least Squares Regression
Source: arXiv:1911.10191 source file (2021-03-06)
Supplement: Supplementary file 53 [file Orth-Dense_n2000.tex]

% latex table generated in R 3.6.2 by xtable 1.8-4 package
% Sat Dec 21 23:17:32 2019
\begin{table}[ht]
\centering
\caption{The performance of BS compared to regularization methods, Orth-Dense, n=2000} 
\scalebox{0.75}{
\begin{tabular}{|c|c|ccccc|}
  \toprule 
 \multicolumn{1}{|c}{} &       & BS    & LASSO & Gamma LASSO & SparseNet & \multicolumn{1}{c|}{rLASSO}  \\
 \multicolumn{1}{|c}{} &       & AICc-hdf & AICc/CV & AICc/CV & CV    & \multicolumn{1}{c|}{CV}       \\
 \midrule\multicolumn{1}{|c}{} &       & \multicolumn{5}{c|}{\% worse than the best possible BS} \\
 \midrule\multirow{4}[2]{*}{hsnr} & p=14 & 0 & 2/2 & 1/4 & 0 & 0 \\ 
   & p=30 & 0 & 1/1 & 3/6 & 1 & 1 \\ 
   & p=60 & 5 & 1/1 & 0/0 & 2 & 4 \\ 
   & p=180 & 8 & 17/16 & 4/5 & 3 & 9 \\ 
  \midrule\multirow{4}[2]{*}{msnr} & p=14 & 0 & 0/0 & 0/2 & 0 & 0 \\ 
   & p=30 & 1 & 1/1 & 3/2 & 3 & 3 \\ 
   & p=60 & 8 & 2/1 & 0/0 & 3 & 4 \\ 
   & p=180 & 8 & 15/14 & 4/4 & 4 & 9 \\ 
  \midrule\multirow{4}[2]{*}{lsnr} & p=14 & 0 & 0/0 & 3/1 & 3 & 3 \\ 
   & p=30 & 3 & 1/0 & 7/2 & 5 & 5 \\ 
   & p=60 & 13 & 0/-1 & 0/1 & 3 & 3 \\ 
   & p=180 & 10 & 9/8 & 14/5 & 5 & 7 \\ 
   \midrule 
 \multicolumn{1}{|c}{} &       & \multicolumn{5}{c|}{Relative efficiency} \\
\midrule\multirow{4}[2]{*}{hsnr} & p=14 & 1 & 0.98/0.98 & 0.99/0.96 & 1 & 1 \\ 
   & p=30 & 1 & 0.99/0.99 & 0.97/0.94 & 0.99 & 0.99 \\ 
   & p=60 & 0.95 & 0.99/0.99 & 1/1 & 0.97 & 0.96 \\ 
   & p=180 & 0.96 & 0.88/0.89 & 0.99/0.98 & 1 & 0.95 \\ 
  \midrule\multirow{4}[2]{*}{msnr} & p=14 & 1 & 1/1 & 1/0.99 & 1 & 1 \\ 
   & p=30 & 1 & 1/1 & 0.98/0.99 & 0.98 & 0.98 \\ 
   & p=60 & 0.92 & 0.98/0.99 & 1/0.99 & 0.97 & 0.96 \\ 
   & p=180 & 0.96 & 0.9/0.91 & 1/0.99 & 1 & 0.95 \\ 
  \midrule\multirow{4}[2]{*}{lsnr} & p=14 & 1 & 1/1 & 0.98/0.99 & 0.98 & 0.97 \\ 
   & p=30 & 0.98 & 1/1 & 0.94/0.98 & 0.96 & 0.96 \\ 
   & p=60 & 0.88 & 0.99/1 & 0.99/0.99 & 0.97 & 0.96 \\ 
   & p=180 & 0.95 & 0.96/0.97 & 0.92/0.99 & 1 & 0.97 \\ 
   \midrule 
 \multicolumn{1}{|c}{} &       & \multicolumn{5}{c|}{Sparsistency (number of extra variables)} \\
\midrule\multirow{4}[2]{*}{hsnr} & p=14 & 14 & 14/14 & 14/14 & 14 & 14 \\ 
   & p=30 & 30 & 30/30 & 30/30 & 29.9 & 29.9 \\ 
   & p=60 & 50.4 & 53.5/54.6 & 46.8/50.4 & 45.4 & 42.9 \\ 
   & p=180 & 31.6 & 89.1/89.8 & 62.4/60.1 & 46.3 & 35.5 \\ 
  \midrule\multirow{4}[2]{*}{msnr} & p=14 & 14 & 14/14 & 14/14 & 14 & 14 \\ 
   & p=30 & 29.9 & 29.6/29.8 & 29/29.6 & 28.8 & 28.7 \\ 
   & p=60 & 41.9 & 48.7/49.7 & 37.2/44.3 & 38.2 & 35 \\ 
   & p=180 & 23.6 & 75.7/75.6 & 51.1/43.5 & 37.6 & 29.5 \\ 
  \midrule\multirow{4}[2]{*}{lsnr} & p=14 & 14 & 14/14 & 13.8/14 & 13.8 & 13.8 \\ 
   & p=30 & 28.1 & 26.8/27.6 & 21.2/26.3 & 24.8 & 23.5 \\ 
   & p=60 & 29.2 & 38.4/39.1 & 25.8/31 & 29.5 & 25.6 \\ 
   & p=180 & 13.3 & 55.1/53.1 & 42.6/30.7 & 29.3 & 23.2 \\ 
   \bottomrule 
\end{tabular}
}
\end{table}
