# Supplementary material for: On the Use of Information Criteria for Subset Selection in Least Squares Regression
Source: arXiv:1911.10191 source file (2021-03-06)
Supplement: Supplementary file 54 [file Orth-Sparse-Ex1_n200.tex]

% latex table generated in R 3.6.2 by xtable 1.8-4 package
% Sat Dec 21 23:17:11 2019
\begin{table}[ht]
\centering
\caption{The performance of BS compared to regularization methods, Orth-Sparse-Ex1, n=200} 
\scalebox{0.75}{
\begin{tabular}{|c|c|ccccc|}
  \toprule 
 \multicolumn{1}{|c}{} &       & BS    & LASSO & Gamma LASSO & SparseNet & \multicolumn{1}{c|}{rLASSO}  \\
 \multicolumn{1}{|c}{} &       & AICc-hdf & AICc/CV & AICc/CV & CV    & \multicolumn{1}{c|}{CV}       \\
 \midrule\multicolumn{1}{|c}{} &       & \multicolumn{5}{c|}{\% worse than the best possible BS} \\
 \midrule\multirow{4}[2]{*}{hsnr} & p=14 & 6 & 42/41 & 16/19 & 13 & 16 \\ 
   & p=30 & 2 & 70/68 & 28/22 & 14 & 18 \\ 
   & p=60 & 2 & 94/92 & 53/25 & 17 & 21 \\ 
   & p=180 & 1 & 128/132 & 129/28 & 20 & 22 \\ 
  \midrule\multirow{4}[2]{*}{msnr} & p=14 & 11 & 43/41 & 21/22 & 13 & 16 \\ 
   & p=30 & 8 & 70/68 & 44/26 & 16 & 19 \\ 
   & p=60 & 8 & 95/92 & 82/30 & 18 & 22 \\ 
   & p=180 & 7 & 127/132 & 228/32 & 19 & 22 \\ 
  \midrule\multirow{4}[2]{*}{lsnr} & p=14 & 24 & 11/11 & 15/17 & 20 & 17 \\ 
   & p=30 & 37 & 7/7 & 16/13 & 15 & 13 \\ 
   & p=60 & 31 & 3/3 & 27/9 & 9 & 7 \\ 
   & p=180 & 22 & 1/5 & 99/8 & 8 & 8 \\ 
   \midrule 
 \multicolumn{1}{|c}{} &       & \multicolumn{5}{c|}{Relative efficiency} \\
\midrule\multirow{4}[2]{*}{hsnr} & p=14 & 1 & 0.74/0.75 & 0.92/0.89 & 0.94 & 0.92 \\ 
   & p=30 & 1 & 0.6/0.61 & 0.8/0.84 & 0.9 & 0.87 \\ 
   & p=60 & 1 & 0.52/0.53 & 0.66/0.81 & 0.87 & 0.84 \\ 
   & p=180 & 1 & 0.44/0.43 & 0.44/0.79 & 0.84 & 0.83 \\ 
  \midrule\multirow{4}[2]{*}{msnr} & p=14 & 1 & 0.78/0.79 & 0.92/0.91 & 0.98 & 0.96 \\ 
   & p=30 & 1 & 0.64/0.64 & 0.75/0.86 & 0.94 & 0.91 \\ 
   & p=60 & 1 & 0.56/0.56 & 0.6/0.83 & 0.92 & 0.89 \\ 
   & p=180 & 1 & 0.47/0.46 & 0.33/0.81 & 0.9 & 0.88 \\ 
  \midrule\multirow{4}[2]{*}{lsnr} & p=14 & 0.89 & 1/1 & 0.97/0.95 & 0.92 & 0.95 \\ 
   & p=30 & 0.78 & 1/1 & 0.92/0.95 & 0.93 & 0.94 \\ 
   & p=60 & 0.78 & 1/1 & 0.81/0.95 & 0.94 & 0.96 \\ 
   & p=180 & 0.83 & 1/0.96 & 0.51/0.93 & 0.94 & 0.93 \\ 
   \midrule 
 \multicolumn{1}{|c}{} &       & \multicolumn{5}{c|}{Sparsistency (number of extra variables)} \\
\midrule\multirow{4}[2]{*}{hsnr} & p=14 & 6(0.2) & 6(3.8)/6(4.5) & 6(0.9)/6(1.3) & 6(0.6) & 6(0.6) \\ 
   & p=30 & 6(0.1) & 6(7.7)/6(8.6) & 6(2.1)/6(1.6) & 6(1.1) & 6(0.6) \\ 
   & p=60 & 6(0) & 6(11.1)/6(12.7) & 6(5.3)/6(2) & 6(1.7) & 6(0.9) \\ 
   & p=180 & 6(0) & 6(14.3)/6(22.9) & 6(20.5)/6(3.3) & 6(3.7) & 6(1.4) \\ 
  \midrule\multirow{4}[2]{*}{msnr} & p=14 & 6(0.5) & 6(3.8)/6(4.5) & 6(1.1)/6(1.3) & 6(0.5) & 6(0.6) \\ 
   & p=30 & 6(0.2) & 6(7.7)/6(8.6) & 6(2.8)/6(1.4) & 6(0.8) & 6(0.7) \\ 
   & p=60 & 6(0.1) & 6(11.1)/6(12.6) & 6(6.5)/6(1.8) & 6(1.2) & 6(0.9) \\ 
   & p=180 & 6(0.1) & 6(14.3)/6(23) & 6(33.6)/6(2.7) & 6(2.4) & 6(1.4) \\ 
  \midrule\multirow{4}[2]{*}{lsnr} & p=14 & 5.4(4.2) & 5.7(3.5)/5.7(4.1) & 5.2(1.4)/5.3(2.9) & 5.3(2.7) & 5.1(2.1) \\ 
   & p=30 & 3.3(2.2) & 5.3(6.7)/5.4(7.1) & 5.2(3.9)/4.9(4.8) & 4.9(5.1) & 4.6(3.5) \\ 
   & p=60 & 1.5(0.2) & 4.9(9.2)/4.9(9.9) & 5.1(8.6)/4.4(6.7) & 4.4(7.4) & 4.2(5) \\ 
   & p=180 & 0.5(0) & 3.9(9.6)/4(14.8) & 5.5(45.9)/3.5(10.5) & 3.6(11.3) & 3.3(8.1) \\ 
   \bottomrule 
\end{tabular}
}
\end{table}
