# Supplementary material for: On the Use of Information Criteria for Subset Selection in Least Squares Regression
Source: arXiv:1911.10191 source file (2021-03-06)
Supplement: Supplementary file 55 [file Orth-Sparse-Ex1_n2000.tex]

% latex table generated in R 3.6.2 by xtable 1.8-4 package
% Sat Dec 21 23:17:18 2019
\begin{table}[ht]
\centering
\caption{The performance of BS compared to regularization methods, Orth-Sparse-Ex1, n=2000} 
\scalebox{0.75}{
\begin{tabular}{|c|c|ccccc|}
  \toprule 
 \multicolumn{1}{|c}{} &       & BS    & LASSO & Gamma LASSO & SparseNet & \multicolumn{1}{c|}{rLASSO}  \\
 \multicolumn{1}{|c}{} &       & AICc-hdf & AICc/CV & AICc/CV & CV    & \multicolumn{1}{c|}{CV}       \\
 \midrule\multicolumn{1}{|c}{} &       & \multicolumn{5}{c|}{\% worse than the best possible BS} \\
 \midrule\multirow{4}[2]{*}{hsnr} & p=14 & 7 & 40/40 & 13/15 & 13 & 15 \\ 
   & p=30 & 3 & 70/68 & 21/17 & 14 & 18 \\ 
   & p=60 & 2 & 94/91 & 29/18 & 14 & 19 \\ 
   & p=180 & 1 & 130/125 & 52/19 & 14 & 16 \\ 
  \midrule\multirow{4}[2]{*}{msnr} & p=14 & 7 & 41/40 & 15/17 & 13 & 16 \\ 
   & p=30 & 3 & 70/68 & 28/19 & 14 & 18 \\ 
   & p=60 & 2 & 94/90 & 44/21 & 15 & 18 \\ 
   & p=180 & 1 & 130/126 & 95/22 & 14 & 16 \\ 
  \midrule\multirow{4}[2]{*}{lsnr} & p=14 & 9 & 41/40 & 21/21 & 14 & 16 \\ 
   & p=30 & 5 & 70/68 & 45/25 & 15 & 19 \\ 
   & p=60 & 5 & 94/90 & 81/27 & 15 & 18 \\ 
   & p=180 & 4 & 129/126 & 188/26 & 14 & 16 \\ 
   \midrule 
 \multicolumn{1}{|c}{} &       & \multicolumn{5}{c|}{Relative efficiency} \\
\midrule\multirow{4}[2]{*}{hsnr} & p=14 & 1 & 0.76/0.76 & 0.95/0.92 & 0.95 & 0.92 \\ 
   & p=30 & 1 & 0.61/0.62 & 0.86/0.88 & 0.91 & 0.87 \\ 
   & p=60 & 1 & 0.53/0.54 & 0.79/0.86 & 0.9 & 0.86 \\ 
   & p=180 & 1 & 0.44/0.45 & 0.67/0.85 & 0.89 & 0.88 \\ 
  \midrule\multirow{4}[2]{*}{msnr} & p=14 & 1 & 0.76/0.76 & 0.92/0.91 & 0.94 & 0.92 \\ 
   & p=30 & 1 & 0.61/0.62 & 0.81/0.87 & 0.91 & 0.87 \\ 
   & p=60 & 1 & 0.53/0.54 & 0.71/0.84 & 0.89 & 0.87 \\ 
   & p=180 & 1 & 0.44/0.45 & 0.52/0.84 & 0.89 & 0.87 \\ 
  \midrule\multirow{4}[2]{*}{lsnr} & p=14 & 1 & 0.77/0.78 & 0.9/0.9 & 0.96 & 0.94 \\ 
   & p=30 & 1 & 0.62/0.63 & 0.73/0.85 & 0.92 & 0.89 \\ 
   & p=60 & 1 & 0.54/0.55 & 0.58/0.83 & 0.91 & 0.89 \\ 
   & p=180 & 1 & 0.46/0.46 & 0.36/0.83 & 0.91 & 0.9 \\ 
   \midrule 
 \multicolumn{1}{|c}{} &       & \multicolumn{5}{c|}{Sparsistency (number of extra variables)} \\
\midrule\multirow{4}[2]{*}{hsnr} & p=14 & 6(0.3) & 6(3.9)/6(4.4) & 6(0.9)/6(1.3) & 6(0.6) & 6(0.6) \\ 
   & p=30 & 6(0.1) & 6(8.5)/6(8.7) & 6(2.2)/6(1.8) & 6(1.1) & 6(0.7) \\ 
   & p=60 & 6(0) & 6(13.2)/6(12.4) & 6(4)/6(2.1) & 6(1.5) & 6(0.6) \\ 
   & p=180 & 6(0) & 6(21.8)/6(18.7) & 6(10.6)/6(2.7) & 6(2.2) & 6(0.5) \\ 
  \midrule\multirow{4}[2]{*}{msnr} & p=14 & 6(0.3) & 6(3.9)/6(4.4) & 6(1)/6(1.4) & 6(0.6) & 6(0.6) \\ 
   & p=30 & 6(0.1) & 6(8.6)/6(8.7) & 6(2.5)/6(1.7) & 6(1.1) & 6(0.7) \\ 
   & p=60 & 6(0) & 6(13.3)/6(12.4) & 6(5)/6(1.8) & 6(1.4) & 6(0.6) \\ 
   & p=180 & 6(0) & 6(21.8)/6(18.7) & 6(15.6)/6(1.9) & 6(2) & 6(0.5) \\ 
  \midrule\multirow{4}[2]{*}{lsnr} & p=14 & 6(0.4) & 6(3.9)/6(4.4) & 6(1.1)/6(1.4) & 6(0.6) & 6(0.6) \\ 
   & p=30 & 6(0.2) & 6(8.5)/6(8.7) & 6(3)/6(1.5) & 6(0.8) & 6(0.7) \\ 
   & p=60 & 6(0.1) & 6(13.2)/6(12.4) & 6(6.7)/6(1.4) & 6(0.9) & 6(0.7) \\ 
   & p=180 & 6(0.1) & 6(21.2)/6(18.7) & 6(23.6)/6(1.3) & 6(1.3) & 6(0.5) \\ 
   \bottomrule 
\end{tabular}
}
\end{table}
