# Supplementary material for: On the Use of Information Criteria for Subset Selection in Least Squares Regression
Source: arXiv:1911.10191 source file (2021-03-06)
Supplement: Supplementary file 56 [file Orth-Sparse-Ex2_n200.tex]

% latex table generated in R 3.6.2 by xtable 1.8-4 package
% Sat Dec 21 23:17:19 2019
\begin{table}[ht]
\centering
\caption{The performance of BS compared to regularization methods, Orth-Sparse-Ex2, n=200} 
\scalebox{0.75}{
\begin{tabular}{|c|c|ccccc|}
  \toprule 
 \multicolumn{1}{|c}{} &       & BS    & LASSO & Gamma LASSO & SparseNet & \multicolumn{1}{c|}{rLASSO}  \\
 \multicolumn{1}{|c}{} &       & AICc-hdf & AICc/CV & AICc/CV & CV    & \multicolumn{1}{c|}{CV}       \\
 \midrule\multicolumn{1}{|c}{} &       & \multicolumn{5}{c|}{\% worse than the best possible BS} \\
 \midrule\multirow{4}[2]{*}{hsnr} & p=14 & 32 & 23/22 & 16/19 & 22 & 22 \\ 
   & p=30 & 25 & 32/30 & 32/20 & 19 & 24 \\ 
   & p=60 & 18 & 39/38 & 59/20 & 16 & 23 \\ 
   & p=180 & 11 & 51/55 & 189/19 & 14 & 20 \\ 
  \midrule\multirow{4}[2]{*}{msnr} & p=14 & 21 & 32/31 & 25/19 & 17 & 18 \\ 
   & p=30 & 15 & 52/51 & 43/23 & 18 & 21 \\ 
   & p=60 & 14 & 70/69 & 73/27 & 22 & 25 \\ 
   & p=180 & 15 & 93/99 & 293/28 & 26 & 29 \\ 
  \midrule\multirow{4}[2]{*}{lsnr} & p=14 & 34 & 19/18 & 18/24 & 24 & 23 \\ 
   & p=30 & 34 & 21/21 & 30/26 & 25 & 23 \\ 
   & p=60 & 33 & 23/24 & 57/26 & 25 & 24 \\ 
   & p=180 & 39 & 24/30 & 167/26 & 25 & 26 \\ 
   \midrule 
 \multicolumn{1}{|c}{} &       & \multicolumn{5}{c|}{Relative efficiency} \\
\midrule\multirow{4}[2]{*}{hsnr} & p=14 & 0.88 & 0.95/0.95 & 1/0.98 & 0.95 & 0.95 \\ 
   & p=30 & 0.95 & 0.9/0.91 & 0.9/0.99 & 1 & 0.96 \\ 
   & p=60 & 0.99 & 0.84/0.84 & 0.73/0.97 & 1 & 0.95 \\ 
   & p=180 & 1 & 0.74/0.72 & 0.38/0.94 & 0.97 & 0.92 \\ 
  \midrule\multirow{4}[2]{*}{msnr} & p=14 & 0.97 & 0.89/0.89 & 0.93/0.98 & 1 & 0.99 \\ 
   & p=30 & 1 & 0.76/0.76 & 0.81/0.94 & 0.98 & 0.96 \\ 
   & p=60 & 1 & 0.67/0.67 & 0.66/0.9 & 0.94 & 0.91 \\ 
   & p=180 & 1 & 0.59/0.58 & 0.29/0.9 & 0.91 & 0.89 \\ 
  \midrule\multirow{4}[2]{*}{lsnr} & p=14 & 0.88 & 1/1 & 1/0.96 & 0.95 & 0.96 \\ 
   & p=30 & 0.9 & 1/1 & 0.93/0.96 & 0.97 & 0.98 \\ 
   & p=60 & 0.92 & 1/1 & 0.78/0.98 & 0.99 & 0.99 \\ 
   & p=180 & 0.9 & 1/0.96 & 0.47/0.99 & 0.99 & 0.99 \\ 
   \midrule 
 \multicolumn{1}{|c}{} &       & \multicolumn{5}{c|}{Sparsistency (number of extra variables)} \\
\midrule\multirow{4}[2]{*}{hsnr} & p=14 & 5(1.3) & 5.9(3.7)/5.9(4.4) & 5.6(1.3)/5.4(1.5) & 5.3(1.2) & 5.3(1) \\ 
   & p=30 & 4.5(0.2) & 5.7(7.2)/5.8(8.2) & 5.5(3.4)/5.1(2) & 5.1(2) & 5(1.3) \\ 
   & p=60 & 4.2(0.1) & 5.6(10.5)/5.7(11.8) & 5.5(7.8)/4.9(2.6) & 5(3) & 4.8(1.7) \\ 
   & p=180 & 4.1(0) & 5.4(12.9)/5.4(20.3) & 5.8(45.9)/4.6(3.7) & 4.7(5.3) & 4.5(2.2) \\ 
  \midrule\multirow{4}[2]{*}{msnr} & p=14 & 4.4(1) & 5.2(3.2)/5.3(3.8) & 4.7(1.1)/4.5(0.9) & 4.4(0.8) & 4.4(0.7) \\ 
   & p=30 & 4.1(0.3) & 5(6.4)/5(7.1) & 4.6(2.9)/4.3(1.2) & 4.3(1.1) & 4.3(0.9) \\ 
   & p=60 & 4(0.2) & 4.8(9.4)/4.8(10.4) & 4.6(6.7)/4.2(1.4) & 4.2(1.9) & 4.2(1.2) \\ 
   & p=180 & 3.9(0.1) & 4.5(12)/4.5(18.2) & 5(46.3)/4.1(2.1) & 4.1(3.7) & 4.1(2) \\ 
  \midrule\multirow{4}[2]{*}{lsnr} & p=14 & 3.7(2.1) & 4.3(2.7)/4.4(3) & 3.7(1.3)/3.5(1.4) & 3.5(1.4) & 3.4(1.2) \\ 
   & p=30 & 2.5(0.9) & 3.9(5.1)/3.9(5.4) & 3.7(3.4)/3(2.3) & 3.1(2.7) & 3.1(2) \\ 
   & p=60 & 1.8(0.2) & 3.6(7.7)/3.6(8) & 3.7(8)/2.8(3.6) & 3(4.7) & 2.8(3.1) \\ 
   & p=180 & 1.1(0.1) & 3(9.6)/3.1(13.7) & 4.1(43.1)/2.4(6.1) & 2.6(7.7) & 2.4(5.3) \\ 
   \bottomrule 
\end{tabular}
}
\end{table}
