# Supplementary material for: On the Use of Information Criteria for Subset Selection in Least Squares Regression
Source: arXiv:1911.10191 source file (2021-03-06)
Supplement: Supplementary file 57 [file Orth-Sparse-Ex2_n2000.tex]

% latex table generated in R 3.6.2 by xtable 1.8-4 package
% Sat Dec 21 23:17:24 2019
\begin{table}[ht]
\centering
\caption{The performance of BS compared to regularization methods, Orth-Sparse-Ex2, n=2000} 
\scalebox{0.75}{
\begin{tabular}{|c|c|ccccc|}
  \toprule 
 \multicolumn{1}{|c}{} &       & BS    & LASSO & Gamma LASSO & SparseNet & \multicolumn{1}{c|}{rLASSO}  \\
 \multicolumn{1}{|c}{} &       & AICc-hdf & AICc/CV & AICc/CV & CV    & \multicolumn{1}{c|}{CV}       \\
 \midrule\multicolumn{1}{|c}{} &       & \multicolumn{5}{c|}{\% worse than the best possible BS} \\
 \midrule\multirow{4}[2]{*}{hsnr} & p=14 & 9 & 40/40 & 20/16 & 14 & 15 \\ 
   & p=30 & 5 & 71/68 & 45/21 & 15 & 19 \\ 
   & p=60 & 4 & 95/91 & 83/24 & 14 & 18 \\ 
   & p=180 & 4 & 129/125 & 195/23 & 14 & 15 \\ 
  \midrule\multirow{4}[2]{*}{msnr} & p=14 & 32 & 34/33 & 20/21 & 23 & 23 \\ 
   & p=30 & 39 & 52/50 & 44/28 & 29 & 31 \\ 
   & p=60 & 38 & 60/57 & 74/28 & 29 & 32 \\ 
   & p=180 & 37 & 67/64 & 155/26 & 25 & 31 \\ 
  \midrule\multirow{4}[2]{*}{lsnr} & p=14 & 19 & 27/26 & 24/18 & 16 & 17 \\ 
   & p=30 & 13 & 46/44 & 57/20 & 15 & 18 \\ 
   & p=60 & 10 & 63/60 & 102/21 & 15 & 18 \\ 
   & p=180 & 8 & 88/84 & 230/19 & 15 & 16 \\ 
   \midrule 
 \multicolumn{1}{|c}{} &       & \multicolumn{5}{c|}{Relative efficiency} \\
\midrule\multirow{4}[2]{*}{hsnr} & p=14 & 1 & 0.78/0.78 & 0.91/0.94 & 0.96 & 0.94 \\ 
   & p=30 & 1 & 0.62/0.63 & 0.73/0.87 & 0.91 & 0.89 \\ 
   & p=60 & 1 & 0.54/0.55 & 0.57/0.84 & 0.91 & 0.89 \\ 
   & p=180 & 1 & 0.45/0.46 & 0.35/0.84 & 0.91 & 0.9 \\ 
  \midrule\multirow{4}[2]{*}{msnr} & p=14 & 0.91 & 0.9/0.9 & 1/0.99 & 0.98 & 0.98 \\ 
   & p=30 & 0.92 & 0.85/0.86 & 0.89/1 & 1 & 0.98 \\ 
   & p=60 & 0.93 & 0.8/0.82 & 0.74/1 & 1 & 0.97 \\ 
   & p=180 & 0.91 & 0.75/0.76 & 0.49/0.99 & 1 & 0.95 \\ 
  \midrule\multirow{4}[2]{*}{lsnr} & p=14 & 0.97 & 0.91/0.92 & 0.94/0.98 & 1 & 0.99 \\ 
   & p=30 & 1 & 0.77/0.78 & 0.72/0.94 & 0.98 & 0.95 \\ 
   & p=60 & 1 & 0.67/0.69 & 0.54/0.91 & 0.95 & 0.93 \\ 
   & p=180 & 1 & 0.58/0.59 & 0.33/0.91 & 0.95 & 0.93 \\ 
   \midrule 
 \multicolumn{1}{|c}{} &       & \multicolumn{5}{c|}{Sparsistency (number of extra variables)} \\
\midrule\multirow{4}[2]{*}{hsnr} & p=14 & 6(0.4) & 6(3.8)/6(4.4) & 6(1.1)/6(0.9) & 6(0.6) & 6(0.6) \\ 
   & p=30 & 6(0.2) & 6(8.5)/6(8.7) & 6(3)/6(1.3) & 6(0.9) & 6(0.7) \\ 
   & p=60 & 6(0.1) & 6(13.2)/6(12.4) & 6(6.8)/6(1.5) & 6(1) & 6(0.6) \\ 
   & p=180 & 6(0) & 6(21.5)/6(18.7) & 6(24)/6(1.6) & 6(1.4) & 6(0.5) \\ 
  \midrule\multirow{4}[2]{*}{msnr} & p=14 & 5.8(1.7) & 6(3.8)/6(4.4) & 6(1.2)/5.9(1.5) & 5.9(1.1) & 5.8(0.9) \\ 
   & p=30 & 5.5(0.9) & 6(8.5)/6(8.6) & 6(3.6)/5.8(2.3) & 5.8(2.2) & 5.7(1.4) \\ 
   & p=60 & 5.2(0.3) & 6(13.1)/6(12.2) & 5.9(7.9)/5.7(2.5) & 5.7(2.8) & 5.6(1.5) \\ 
   & p=180 & 4.8(0.1) & 5.9(21.2)/5.9(18.3) & 6(27.1)/5.5(3.2) & 5.5(4.3) & 5.3(1.6) \\ 
  \midrule\multirow{4}[2]{*}{lsnr} & p=14 & 4.5(0.9) & 5.4(3.4)/5.4(3.9) & 4.9(1.3)/4.6(1.1) & 4.5(0.7) & 4.5(0.7) \\ 
   & p=30 & 4.2(0.4) & 5.1(7.3)/5.2(7.3) & 4.8(3.8)/4.4(1.2) & 4.3(1.2) & 4.3(1) \\ 
   & p=60 & 4.1(0.1) & 5(11.1)/4.9(10) & 4.8(8.1)/4.2(1.2) & 4.2(1.3) & 4.2(0.9) \\ 
   & p=180 & 4(0.1) & 4.7(18.1)/4.6(15) & 4.9(27.3)/4.1(1) & 4.1(1.5) & 4.1(0.8) \\ 
   \bottomrule 
\end{tabular}
}
\end{table}
